# Supplementary material for: Resonant superalgebras for supergravity
Source: arXiv:2108.10304 source file (2021-11-03)
Supplement: Supplementary file 1 [file supplement.pdf]

# Supplement to Resonant superalgebras for supergravity

Remigiusz Durka [*1] and Krzysztof M. Graczyk [†1]

[1] *Institute for Theoretical Physics, University of Wrocław, pl. M. Borna 9, 50-204 Wrocław, Poland*

November 3, 2021

## Contents

**1 Resonant superalgebras with one fermionic charge 1**
1.1 JP+Q . . . 1
1.2 JPZ+Q . . . 1
1.3 JPZU+Q . . . 2

**2 Resonant superalgebras with two fermionic charges 4**
2.1 JP+QY . . . 4
2.2 JPZ+QY . . . 4
2.3 JZPU+QY . . . 7

## Resonant superalgebras

Following the notion of the resonant algebras, we introduce the enlarged generator content:

$$\begin{aligned}
&\square_{ab} \to J_{ab}, Z_{ab}, \ldots &&(\text{Lorentz}-\text{like})\\
&\boxdot_{a} \to P_a, U_a, \ldots &&(\text{translation}-\text{like})\\
&\bigcirc_{\alpha} \to Q_\alpha, Y_\alpha, \ldots &&(\text{supercharge}-\text{like})\,.
\end{aligned}$$

The superalgebra template

$$\begin{cases}
\left[\square_{ab}, \square_{cd}\right] = \eta_{bc}\square_{ad} - \eta_{ac}\square_{bd} - \eta_{bd}\square_{ac} + \eta_{ad}\square_{bc}\,,\\
\left[\square_{ab}, \boxdot_{c}\right] = \eta_{bc}\boxdot_{a} - \eta_{ac}\boxdot_{b}\\
\left[\boxdot_{a}, \boxdot_{b}\right] = \square_{ab}\\
\left[\square_{ab}, \bigcirc_{\alpha}\right] = \frac{1}{2}\,(\Gamma_{ab})_\alpha^{\ \beta}\bigcirc_\beta\,,\\
\left[\boxdot_{a}, \bigcirc_{\alpha}\right] = \frac{1}{2}\,(\Gamma_{a})_\alpha^{\ \beta}\bigcirc_\beta\,,\\
\left\{\bigcirc_{\alpha}, \bigcirc_{\beta}\right\} = -\left(\Gamma^a C\right)_{\alpha\beta}\boxdot_a + \frac{1}{2}\left(\Gamma^{ab} C\right)_{\alpha\beta}\square_{ab}\,,
\end{cases}$$

resembles the structure constants of supersymmetric extension of the AdS algebra. The generators obey few additional requirements and we allow zero to appear on the right-hand-side.

The presented framework offers the following realizations of the resonant algebras and superalgebras depending on the generator content:

| 1× J | 1× J+Q | 0× J+QY |
|---|---|---|
| 2× JP | 2× JP+Q | 10× JP+QY |
| 6× JPZ | 9× JPZ+Q | 102× JPZ+QY |
| 30× JPZU | 43× JPZU+Q | 667× JPZU+QY |

Further filtering with the condition $\{Q, Q\} = P + \ldots$, leading to the supergravity formulation (SUGRA), shows the following superalgebra configurations:

| 2× JP+Q | 8× JP+QY |
|---|---|
| 6× JPZ+Q | 71× JPZ+QY |
| 17× JPZU+Q | 264× JPZU+QY |

Below we present explicitly all possible superalgebras in the form of tables. Note that each separate line encoding the particular (anti)commutation relations represents unique superalgebra.

# 1 Resonant superalgebras with one fermionic charge

## 1.1 JP+Q

**Total number of cases:** 2.
Total number of resonant SUGRA cases: 2.

| [ , ] | $J$ | $P$ |
|---|---|---|
| $J$ | $J$ | $P$ |
| $P$ | $P$ | 0 |

| [ , ] | $Q$ |
|---|---|
| $J$ | $Q$ |
| $P$ | 0 |

| { , } | $Q$ |
|---|---|
| $Q$ | $P$ |

| [ , ] | $J$ | $P$ |
|---|---|---|
| $J$ | $J$ | $P$ |
| $P$ | $P$ | $J$ |

| [ , ] | $Q$ |
|---|---|
| $J$ | $Q$ |
| $P$ | $Q$ |

| { , } | $Q$ |
|---|---|
| $Q$ | $P+J$ |

Total number of resonant non-standard cases: 0.

## 1.2 JPZ+Q

**Total number of cases:** 9.
Total number of resonant SUGRA cases: 6.

| | $J$ | $Z$ | $P$ |
|---|---|---|---|
| $J$ | $J$ | $Z$ | $P$ |
| $Z$ | $Z$ | 0 | 0 |
| $P$ | $P$ | 0 | 0 |

| | $Q$ |
|---|---|
| $J$ | $Q$ |
| $Z$ | 0 |
| $P$ | 0 |

| | $Q$ |
|---|---|
| $Q$ | $P$ |

| | $J$ | $Z$ | $P$ |
|---|---|---|---|
| $J$ | $J$ | $Z$ | $P$ |
| $Z$ | $Z$ | 0 | 0 |
| $P$ | $P$ | 0 | 0 |

| | $Q$ |
|---|---|
| $J$ | $Q$ |
| $Z$ | 0 |
| $P$ | 0 |

| | $Q$ |
|---|---|
| $Q$ | $P+Z$ |

*remigiusz.durka@uwr.edu.pl
†krzysztof.graczyk@uwr.edu.pl

| | J | Z | P |
|---|---|---|---|
| J | J | Z | P |
| Z | Z | Z | 0 |
| P | P | 0 | 0 |

| | Q |
|---|---|
| J | Q |
| Z | 0 |
| P | 0 |

| | Q |
|---|---|
| Q | P |

| | J | Z | P |
|---|---|---|---|
| J | J | Z | P |
| Z | Z | Z | P |
| P | P | P | 0 |

| | Q |
|---|---|
| J | Q |
| Z | Q |
| P | 0 |

| | Q |
|---|---|
| Q | P |

| | J | Z | P |
|---|---|---|---|
| J | J | Z | P |
| Z | Z | Z | P |
| P | P | P | Z |

| | Q |
|---|---|
| J | Q |
| Z | Q |
| P | Q |

| | Q |
|---|---|
| Q | P + Z |

| | J | Z | P |
|---|---|---|---|
| J | J | Z | P |
| Z | Z | J | P |
| P | P | P | 0 |

| | Q |
|---|---|
| J | Q |
| Z | Q |
| P | 0 |

| | Q |
|---|---|
| Q | P |

Total number of resonant non-standard cases: 3.

| | J | Z | P |
|---|---|---|---|
| J | J | Z | P |
| Z | Z | 0 | 0 |
| P | P | 0 | 0 |

| | Q |
|---|---|
| J | Q |
| Z | 0 |
| P | 0 |

| | Q |
|---|---|
| Q | Z |

| | J | Z | P |
|---|---|---|---|
| J | J | Z | P |
| Z | Z | 0 | 0 |
| P | P | 0 | Z |

| | Q |
|---|---|
| J | Q |
| Z | 0 |
| P | 0 |

| | Q |
|---|---|
| Q | Z |

| | J | Z | P |
|---|---|---|---|
| J | J | Z | P |
| Z | Z | Z | 0 |
| P | P | 0 | 0 |

| | Q |
|---|---|
| J | Q |
| Z | Q |
| P | 0 |

| | Q |
|---|---|
| Q | Z |

## 1.3 JPZU+Q

**Total number of cases:** 43.
Total number of resonant SUGRA cases: 17.

| | J | Z | P | U |
|---|---|---|---|---|
| J | J | Z | P | U |
| Z | Z | 0 | 0 | 0 |
| P | P | 0 | 0 | 0 |
| U | U | 0 | 0 | 0 |

| | Q |
|---|---|
| J | Q |
| Z | 0 |
| P | 0 |
| U | 0 |

| | Q |
|---|---|
| Q | P |

| | J | Z | P | U |
|---|---|---|---|---|
| J | J | Z | P | U |
| Z | Z | 0 | 0 | 0 |
| P | P | 0 | 0 | 0 |
| U | U | 0 | 0 | 0 |

| | Q |
|---|---|
| J | Q |
| Z | 0 |
| P | 0 |
| U | 0 |

| | Q |
|---|---|
| Q | P + Z |

| | J | Z | P | U |
|---|---|---|---|---|
| J | J | Z | P | U |
| Z | Z | 0 | 0 | P |
| P | P | 0 | 0 | 0 |
| U | U | P | 0 | 0 |

| | Q |
|---|---|
| J | Q |
| Z | 0 |
| P | 0 |
| U | 0 |

| | Q |
|---|---|
| Q | P |

| | J | Z | P | U |
|---|---|---|---|---|
| J | J | Z | P | U |
| Z | Z | 0 | 0 | 0 |
| P | P | 0 | 0 | 0 |
| U | U | 0 | 0 | Z |

| | Q |
|---|---|
| J | Q |
| Z | 0 |
| P | 0 |
| U | 0 |

| | Q |
|---|---|
| Q | P |

| | J | Z | P | U |
|---|---|---|---|---|
| J | J | Z | P | U |
| Z | Z | 0 | 0 | 0 |
| P | P | 0 | 0 | 0 |
| U | U | 0 | 0 | Z |

| | Q |
|---|---|
| J | Q |
| Z | 0 |
| P | 0 |
| U | 0 |

| | Q |
|---|---|
| Q | P + Z |

| | J | Z | P | U |
|---|---|---|---|---|
| J | J | Z | P | U |
| Z | Z | 0 | 0 | P |
| P | P | 0 | 0 | 0 |
| U | U | P | 0 | Z |

| | Q |
|---|---|
| J | Q |
| Z | 0 |
| P | 0 |
| U | 0 |

| | Q |
|---|---|
| Q | P |

| | J | Z | P | U |
|---|---|---|---|---|
| J | J | Z | P | U |
| Z | Z | 0 | 0 | P |
| P | P | 0 | 0 | Z |
| U | U | P | Z | J |

| | Q |
|---|---|
| J | Q |
| Z | 0 |
| P | 0 |
| U | Q |

| | Q |
|---|---|
| Q | P + Z |

| | J | Z | P | U |
|---|---|---|---|---|
| J | J | Z | P | U |
| Z | Z | Z | 0 | 0 |
| P | P | 0 | 0 | 0 |
| U | U | 0 | 0 | 0 |

| | Q |
|---|---|
| J | Q |
| Z | 0 |
| P | 0 |
| U | 0 |

| | Q |
|---|---|
| Q | P |

| | J | Z | P | U |
|---|---|---|---|---|
| J | J | Z | P | U |
| Z | Z | Z | 0 | U |
| P | P | 0 | 0 | 0 |
| U | U | U | 0 | 0 |

| | Q |
|---|---|
| J | Q |
| Z | 0 |
| P | 0 |
| U | 0 |

| | Q |
|---|---|
| Q | P |

| | J | Z | P | U |
|---|---|---|---|---|
| J | J | Z | P | U |
| Z | Z | Z | P | 0 |
| P | P | P | 0 | 0 |
| U | U | 0 | 0 | 0 |

| | Q |
|---|---|
| J | Q |
| Z | Q |
| P | 0 |
| U | 0 |

| | Q |
|---|---|
| Q | P |

| | J | Z | P | U |
|---|---|---|---|---|
| J | J | Z | P | U |
| Z | Z | Z | P | P |
| P | P | P | 0 | 0 |
| U | U | P | 0 | 0 |

| | Q |
|---|---|
| J | Q |
| Z | Q |
| P | 0 |
| U | 0 |

| | Q |
|---|---|
| Q | P |

| | J | Z | P | U |
|---|---|---|---|---|
| J | J | Z | P | U |
| Z | Z | Z | P | U |
| P | P | P | 0 | 0 |
| U | U | U | 0 | 0 |

| | Q |
|---|---|
| J | Q |
| Z | Q |
| P | 0 |
| U | 0 |

| | Q |
|---|---|
| Q | P |

| | J | Z | P | U |
|---|---|---|---|---|
| J | J | Z | P | U |
| Z | Z | Z | 0 | U |
| P | P | 0 | 0 | 0 |
| U | U | U | 0 | Z |

| | Q |
|---|---|
| J | Q |
| Z | 0 |
| P | 0 |
| U | 0 |

| | Q |
|---|---|
| Q | P |

| | J | Z | P | U |
|---|---|---|---|---|
| J | J | Z | P | U |
| Z | Z | Z | P | 0 |
| P | P | P | Z | 0 |
| U | U | 0 | 0 | 0 |

| | Q |
|---|---|
| J | Q |
| Z | Q |
| P | Q |
| U | 0 |

| | Q |
|---|---|
| Q | P + Z |

| | J | Z | P | U |
|---|---|---|---|---|
| J | J | Z | P | U |
| Z | Z | Z | P | P |
| P | P | P | Z | Z |
| U | U | P | Z | Z |

| | Q |
|---|---|
| J | Q |
| Z | Q |
| P | Q |
| U | Q |

| | Q |
|---|---|
| Q | P + Z |

| | J | Z | P | U |
|---|---|---|---|---|
| J | J | Z | P | U |
| Z | Z | Z | P | P |
| P | P | P | Z | Z |
| U | U | P | Z | J |

| | Q |
|---|---|
| J | Q |
| Z | Q |
| P | Q |
| U | Q |

| | Q |
|---|---|
| Q | P + Z |

| | J | Z | P | U |
|---|---|---|---|---|
| J | J | Z | P | U |
| Z | Z | J | P | U |
| P | P | P | 0 | 0 |
| U | U | U | 0 | 0 |

| | Q |
|---|---|
| J | Q |
| Z | Q |
| P | 0 |
| U | 0 |

| | Q |
|---|---|
| Q | P |

Total number of resonant non-standard cases: 26.

| | J | Z | P | U |
|---|---|---|---|---|
| J | J | Z | P | U |
| Z | Z | 0 | 0 | 0 |
| P | P | 0 | 0 | 0 |
| U | U | 0 | 0 | 0 |

| | Q |
|---|---|
| J | Q |
| Z | 0 |
| P | 0 |
| U | 0 |

| | Q |
|---|---|
| Q | U |

| | $J$ | $Z$ | $P$ | $U$ |
|---|---|---|---|---|
| $J$ | $J$ | $Z$ | $P$ | $U$ |
| $Z$ | $Z$ | 0 | 0 | 0 |
| $P$ | $P$ | 0 | 0 | 0 |
| $U$ | $U$ | 0 | 0 | 0 |

| | $Q$ |
|---|---|
| $J$ | $Q$ |
| $Z$ | 0 |
| $P$ | 0 |
| $U$ | 0 |

| | $Q$ |
|---|---|
| $Q$ | $Z$ |

| | $J$ | $Z$ | $P$ | $U$ |
|---|---|---|---|---|
| $J$ | $J$ | $Z$ | $P$ | $U$ |
| $Z$ | $Z$ | 0 | 0 | 0 |
| $P$ | $P$ | 0 | 0 | 0 |
| $U$ | $U$ | 0 | 0 | 0 |

| | $Q$ |
|---|---|
| $J$ | $Q$ |
| $Z$ | 0 |
| $P$ | 0 |
| $U$ | 0 |

| | $Q$ |
|---|---|
| $Q$ | $U+Z$ |

| | $J$ | $Z$ | $P$ | $U$ |
|---|---|---|---|---|
| $J$ | $J$ | $Z$ | $P$ | $U$ |
| $Z$ | $Z$ | 0 | $U$ | 0 |
| $P$ | $P$ | $U$ | 0 | 0 |
| $U$ | $U$ | 0 | 0 | 0 |

| | $Q$ |
|---|---|
| $J$ | $Q$ |
| $Z$ | 0 |
| $P$ | 0 |
| $U$ | 0 |

| | $Q$ |
|---|---|
| $Q$ | $U$ |

| | $J$ | $Z$ | $P$ | $U$ |
|---|---|---|---|---|
| $J$ | $J$ | $Z$ | $P$ | $U$ |
| $Z$ | $Z$ | 0 | 0 | 0 |
| $P$ | $P$ | 0 | 0 | 0 |
| $U$ | $U$ | 0 | 0 | $Z$ |

| | $Q$ |
|---|---|
| $J$ | $Q$ |
| $Z$ | 0 |
| $P$ | 0 |
| $U$ | 0 |

| | $Q$ |
|---|---|
| $Q$ | $Z$ |

| | $J$ | $Z$ | $P$ | $U$ |
|---|---|---|---|---|
| $J$ | $J$ | $Z$ | $P$ | $U$ |
| $Z$ | $Z$ | 0 | 0 | 0 |
| $P$ | $P$ | 0 | 0 | $Z$ |
| $U$ | $U$ | 0 | $Z$ | 0 |

| | $Q$ |
|---|---|
| $J$ | $Q$ |
| $Z$ | 0 |
| $P$ | 0 |
| $U$ | 0 |

| | $Q$ |
|---|---|
| $Q$ | $Z$ |

| | $J$ | $Z$ | $P$ | $U$ |
|---|---|---|---|---|
| $J$ | $J$ | $Z$ | $P$ | $U$ |
| $Z$ | $Z$ | 0 | 0 | 0 |
| $P$ | $P$ | 0 | 0 | $Z$ |
| $U$ | $U$ | 0 | $Z$ | $Z$ |

| | $Q$ |
|---|---|
| $J$ | $Q$ |
| $Z$ | 0 |
| $P$ | 0 |
| $U$ | 0 |

| | $Q$ |
|---|---|
| $Q$ | $Z$ |

| | $J$ | $Z$ | $P$ | $U$ |
|---|---|---|---|---|
| $J$ | $J$ | $Z$ | $P$ | $U$ |
| $Z$ | $Z$ | 0 | 0 | 0 |
| $P$ | $P$ | 0 | $Z$ | 0 |
| $U$ | $U$ | 0 | 0 | 0 |

| | $Q$ |
|---|---|
| $J$ | $Q$ |
| $Z$ | 0 |
| $P$ | 0 |
| $U$ | 0 |

| | $Q$ |
|---|---|
| $Q$ | $U$ |

| | $J$ | $Z$ | $P$ | $U$ |
|---|---|---|---|---|
| $J$ | $J$ | $Z$ | $P$ | $U$ |
| $Z$ | $Z$ | 0 | 0 | 0 |
| $P$ | $P$ | 0 | $Z$ | 0 |
| $U$ | $U$ | 0 | 0 | 0 |

| | $Q$ |
|---|---|
| $J$ | $Q$ |
| $Z$ | 0 |
| $P$ | 0 |
| $U$ | 0 |

| | $Q$ |
|---|---|
| $Q$ | $Z$ |

| | $J$ | $Z$ | $P$ | $U$ |
|---|---|---|---|---|
| $J$ | $J$ | $Z$ | $P$ | $U$ |
| $Z$ | $Z$ | 0 | 0 | 0 |
| $P$ | $P$ | 0 | $Z$ | 0 |
| $U$ | $U$ | 0 | 0 | 0 |

| | $Q$ |
|---|---|
| $J$ | $Q$ |
| $Z$ | 0 |
| $P$ | 0 |
| $U$ | 0 |

| | $Q$ |
|---|---|
| $Q$ | $U+Z$ |

| | $J$ | $Z$ | $P$ | $U$ |
|---|---|---|---|---|
| $J$ | $J$ | $Z$ | $P$ | $U$ |
| $Z$ | $Z$ | 0 | $U$ | 0 |
| $P$ | $P$ | $U$ | $Z$ | 0 |
| $U$ | $U$ | 0 | 0 | 0 |

| | $Q$ |
|---|---|
| $J$ | $Q$ |
| $Z$ | 0 |
| $P$ | 0 |
| $U$ | 0 |

| | $Q$ |
|---|---|
| $Q$ | $U$ |

| | $J$ | $Z$ | $P$ | $U$ |
|---|---|---|---|---|
| $J$ | $J$ | $Z$ | $P$ | $U$ |
| $Z$ | $Z$ | 0 | 0 | 0 |
| $P$ | $P$ | 0 | $Z$ | 0 |
| $U$ | $U$ | 0 | 0 | $Z$ |

| | $Q$ |
|---|---|
| $J$ | $Q$ |
| $Z$ | 0 |
| $P$ | 0 |
| $U$ | 0 |

| | $Q$ |
|---|---|
| $Q$ | $Z$ |

| | $J$ | $Z$ | $P$ | $U$ |
|---|---|---|---|---|
| $J$ | $J$ | $Z$ | $P$ | $U$ |
| $Z$ | $Z$ | 0 | 0 | 0 |
| $P$ | $P$ | 0 | $Z$ | $Z$ |
| $U$ | $U$ | 0 | $Z$ | 0 |

| | $Q$ |
|---|---|
| $J$ | $Q$ |
| $Z$ | 0 |
| $P$ | 0 |
| $U$ | 0 |

| | $Q$ |
|---|---|
| $Q$ | $Z$ |

| | $J$ | $Z$ | $P$ | $U$ |
|---|---|---|---|---|
| $J$ | $J$ | $Z$ | $P$ | $U$ |
| $Z$ | $Z$ | 0 | 0 | 0 |
| $P$ | $P$ | 0 | $Z$ | $Z$ |
| $U$ | $U$ | 0 | $Z$ | $Z$ |

| | $Q$ |
|---|---|
| $J$ | $Q$ |
| $Z$ | 0 |
| $P$ | 0 |
| $U$ | 0 |

| | $Q$ |
|---|---|
| $Q$ | $Z$ |

| | $J$ | $Z$ | $P$ | $U$ |
|---|---|---|---|---|
| $J$ | $J$ | $Z$ | $P$ | $U$ |
| $Z$ | $Z$ | 0 | $U$ | 0 |
| $P$ | $P$ | $U$ | $J$ | $Z$ |
| $U$ | $U$ | 0 | $Z$ | 0 |

| | $Q$ |
|---|---|
| $J$ | $Q$ |
| $Z$ | 0 |
| $P$ | $Q$ |
| $U$ | 0 |

| | $Q$ |
|---|---|
| $Q$ | $U+Z$ |

| | $J$ | $Z$ | $P$ | $U$ |
|---|---|---|---|---|
| $J$ | $J$ | $Z$ | $P$ | $U$ |
| $Z$ | $Z$ | $Z$ | 0 | 0 |
| $P$ | $P$ | 0 | 0 | 0 |
| $U$ | $U$ | 0 | 0 | 0 |

| | $Q$ |
|---|---|
| $J$ | $Q$ |
| $Z$ | 0 |
| $P$ | 0 |
| $U$ | 0 |

| | $Q$ |
|---|---|
| $Q$ | $U$ |

| | $J$ | $Z$ | $P$ | $U$ |
|---|---|---|---|---|
| $J$ | $J$ | $Z$ | $P$ | $U$ |
| $Z$ | $Z$ | $Z$ | 0 | 0 |
| $P$ | $P$ | 0 | 0 | 0 |
| $U$ | $U$ | 0 | 0 | 0 |

| | $Q$ |
|---|---|
| $J$ | $Q$ |
| $Z$ | $Q$ |
| $P$ | 0 |
| $U$ | 0 |

| | $Q$ |
|---|---|
| $Q$ | $Z$ |

| | $J$ | $Z$ | $P$ | $U$ |
|---|---|---|---|---|
| $J$ | $J$ | $Z$ | $P$ | $U$ |
| $Z$ | $Z$ | $Z$ | 0 | $U$ |
| $P$ | $P$ | 0 | 0 | 0 |
| $U$ | $U$ | $U$ | 0 | 0 |

| | $Q$ |
|---|---|
| $J$ | $Q$ |
| $Z$ | $Q$ |
| $P$ | 0 |
| $U$ | 0 |

| | $Q$ |
|---|---|
| $Q$ | $U$ |

| | $J$ | $Z$ | $P$ | $U$ |
|---|---|---|---|---|
| $J$ | $J$ | $Z$ | $P$ | $U$ |
| $Z$ | $Z$ | $Z$ | $P$ | 0 |
| $P$ | $P$ | $P$ | 0 | 0 |
| $U$ | $U$ | 0 | 0 | 0 |

| | $Q$ |
|---|---|
| $J$ | $Q$ |
| $Z$ | 0 |
| $P$ | 0 |
| $U$ | 0 |

| | $Q$ |
|---|---|
| $Q$ | $U$ |

| | $J$ | $Z$ | $P$ | $U$ |
|---|---|---|---|---|
| $J$ | $J$ | $Z$ | $P$ | $U$ |
| $Z$ | $Z$ | $Z$ | $P$ | $U$ |
| $P$ | $P$ | $P$ | 0 | 0 |
| $U$ | $U$ | $U$ | 0 | 0 |

| | $Q$ |
|---|---|
| $J$ | $Q$ |
| $Z$ | $Q$ |
| $P$ | 0 |
| $U$ | 0 |

| | $Q$ |
|---|---|
| $Q$ | $U$ |

| | $J$ | $Z$ | $P$ | $U$ |
|---|---|---|---|---|
| $J$ | $J$ | $Z$ | $P$ | $U$ |
| $Z$ | $Z$ | $Z$ | $U$ | $U$ |
| $P$ | $P$ | $U$ | 0 | 0 |
| $U$ | $U$ | $U$ | 0 | 0 |

| | $Q$ |
|---|---|
| $J$ | $Q$ |
| $Z$ | $Q$ |
| $P$ | 0 |
| $U$ | 0 |

| | $Q$ |
|---|---|
| $Q$ | $U$ |

| | $J$ | $Z$ | $P$ | $U$ |
|---|---|---|---|---|
| $J$ | $J$ | $Z$ | $P$ | $U$ |
| $Z$ | $Z$ | $Z$ | 0 | $U$ |
| $P$ | $P$ | 0 | 0 | 0 |
| $U$ | $U$ | $U$ | 0 | $Z$ |

| | $Q$ |
|---|---|
| $J$ | $Q$ |
| $Z$ | $Q$ |
| $P$ | 0 |
| $U$ | $Q$ |

| | $Q$ |
|---|---|
| $Q$ | $U+Z$ |

| | $J$ | $Z$ | $P$ | $U$ |
|---|---|---|---|---|
| $J$ | $J$ | $Z$ | $P$ | $U$ |
| $Z$ | $Z$ | $Z$ | $P$ | 0 |
| $P$ | $P$ | $P$ | $Z$ | 0 |
| $U$ | $U$ | 0 | 0 | 0 |

| | $Q$ |
|---|---|
| $J$ | $Q$ |
| $Z$ | 0 |
| $P$ | 0 |
| $U$ | 0 |

| | $Q$ |
|---|---|
| $Q$ | $U$ |

| | $J$ | $Z$ | $P$ | $U$ |
|---|---|---|---|---|
| $J$ | $J$ | $Z$ | $P$ | $U$ |
| $Z$ | $Z$ | $Z$ | $U$ | $U$ |
| $P$ | $P$ | $U$ | $Z$ | $Z$ |
| $U$ | $U$ | $U$ | $Z$ | $Z$ |

| | $Q$ |
|---|---|
| $J$ | $Q$ |
| $Z$ | $Q$ |
| $P$ | $Q$ |
| $U$ | $Q$ |

| | $Q$ |
|---|---|
| $Q$ | $U+Z$ |

| | $J$ | $Z$ | $P$ | $U$ |
|---|---|---|---|---|
| $J$ | $J$ | $Z$ | $P$ | $U$ |
| $Z$ | $Z$ | $Z$ | $U$ | $U$ |
| $P$ | $P$ | $U$ | $J$ | $Z$ |
| $U$ | $U$ | $U$ | $Z$ | $Z$ |

| | $Q$ |
|---|---|
| $J$ | $Q$ |
| $Z$ | $Q$ |
| $P$ | $Q$ |
| $U$ | $Q$ |

| | $Q$ |
|---|---|
| $Q$ | $U+Z$ |

| | $J$ | $Z$ | $P$ | $U$ |
|---|---|---|---|---|
| $J$ | $J$ | $Z$ | $P$ | $U$ |
| $Z$ | $Z$ | $J$ | $P$ | $U$ |
| $P$ | $P$ | $P$ | 0 | 0 |
| $U$ | $U$ | $U$ | 0 | 0 |

| | $Q$ |
|---|---|
| $J$ | $Q$ |
| $Z$ | $Q$ |
| $P$ | 0 |
| $U$ | 0 |

| | $Q$ |
|---|---|
| $Q$ | $U$ |

# 2 Resonant superalgebras with two fermionic charges

## 2.1 JP+QY

**Total number of cases:** 10.
Total number of resonant SUGRA cases: 8.

| | J | P |
|---|---|---|
| J | J | P |
| P | P | 0 |

| | Q | Y |
|---|---|---|
| J | Q | Y |
| P | 0 | 0 |

| | Q | Y |
|---|---|---|
| Q | P | 0 |
| Y | 0 | 0 |

| | J | P |
|---|---|---|
| J | J | P |
| P | P | 0 |

| | Q | Y |
|---|---|---|
| J | Q | Y |
| P | Y | 0 |

| | Q | Y |
|---|---|---|
| Q | P | 0 |
| Y | 0 | 0 |

| | J | P |
|---|---|---|
| J | J | P |
| P | P | 0 |

| | Q | Y |
|---|---|---|
| J | Q | Y |
| P | 0 | 0 |

| | Q | Y |
|---|---|---|
| Q | P | 0 |
| Y | 0 | P |

| | J | P |
|---|---|---|
| J | J | P |
| P | P | 0 |

| | Q | Y |
|---|---|---|
| J | Q | Y |
| P | 0 | 0 |

| | Q | Y |
|---|---|---|
| Q | P | P |
| Y | P | 0 |

| | J | P |
|---|---|---|
| J | J | P |
| P | P | 0 |

| | Q | Y |
|---|---|---|
| J | Q | Y |
| P | 0 | 0 |

| | Q | Y |
|---|---|---|
| Q | P | P |
| Y | P | P |

| | J | P |
|---|---|---|
| J | J | P |
| P | P | 0 |

| | Q | Y |
|---|---|---|
| J | Q | Y |
| P | Y | 0 |

| | Q | Y |
|---|---|---|
| Q | $J+P$ | P |
| Y | P | 0 |

| | J | P |
|---|---|---|
| J | J | P |
| P | P | J |

| | Q | Y |
|---|---|---|
| J | Q | Y |
| P | Y | Q |

| | Q | Y |
|---|---|---|
| Q | P | J |
| Y | J | P |

| | J | P |
|---|---|---|
| J | J | P |
| P | P | J |

| | Q | Y |
|---|---|---|
| J | Q | Y |
| P | Y | Q |

| | Q | Y |
|---|---|---|
| Q | $J+P$ | $J+P$ |
| Y | $J+P$ | $J+P$ |

Total number of resonant non-standard cases: 2.

| | J | P |
|---|---|---|
| J | J | P |
| P | P | 0 |

| | Q | Y |
|---|---|---|
| J | Q | Y |
| P | Y | 0 |

| | Q | Y |
|---|---|---|
| Q | J | P |
| Y | P | 0 |

| | J | P |
|---|---|---|
| J | J | P |
| P | P | J |

| | Q | Y |
|---|---|---|
| J | Q | Y |
| P | Y | Q |

| | Q | Y |
|---|---|---|
| Q | J | P |
| Y | P | J |

## 2.2 JPZ+QY

**Total number of cases:** 102.
Total number of resonant SUGRA cases: 71.

| | J | Z | P |
|---|---|---|---|
| J | J | Z | P |
| Z | Z | 0 | 0 |
| P | P | 0 | 0 |

| | Q | Y |
|---|---|---|
| J | Q | Y |
| Z | 0 | 0 |
| P | 0 | 0 |

| | Q | Y |
|---|---|---|
| Q | P | 0 |
| Y | 0 | 0 |

| | J | Z | P |
|---|---|---|---|
| J | J | Z | P |
| Z | Z | 0 | 0 |
| P | P | 0 | 0 |

| | Q | Y |
|---|---|---|
| J | Q | Y |
| Z | Y | 0 |
| P | 0 | 0 |

| | Q | Y |
|---|---|---|
| Q | P | 0 |
| Y | 0 | 0 |

| | J | Z | P |
|---|---|---|---|
| J | J | Z | P |
| Z | Z | 0 | 0 |
| P | P | 0 | 0 |

| | Q | Y |
|---|---|---|
| J | Q | Y |
| Z | 0 | 0 |
| P | Y | 0 |

| | Q | Y |
|---|---|---|
| Q | P | 0 |
| Y | 0 | 0 |

| | J | Z | P |
|---|---|---|---|
| J | J | Z | P |
| Z | Z | 0 | 0 |
| P | P | 0 | 0 |

| | Q | Y |
|---|---|---|
| J | Q | Y |
| Z | Y | 0 |
| P | Y | 0 |

| | Q | Y |
|---|---|---|
| Q | P | 0 |
| Y | 0 | 0 |

| | J | Z | P |
|---|---|---|---|
| J | J | Z | P |
| Z | Z | 0 | 0 |
| P | P | 0 | 0 |

| | Q | Y |
|---|---|---|
| J | Q | Y |
| Z | 0 | 0 |
| P | 0 | 0 |

| | Q | Y |
|---|---|---|
| Q | P | 0 |
| Y | 0 | P |

| | J | Z | P |
|---|---|---|---|
| J | J | Z | P |
| Z | Z | 0 | 0 |
| P | P | 0 | 0 |

| | Q | Y |
|---|---|---|
| J | Q | Y |
| Z | 0 | 0 |
| P | 0 | 0 |

| | Q | Y |
|---|---|---|
| Q | P | 0 |
| Y | 0 | Z |

| | J | Z | P |
|---|---|---|---|
| J | J | Z | P |
| Z | Z | 0 | 0 |
| P | P | 0 | 0 |

| | Q | Y |
|---|---|---|
| J | Q | Y |
| Z | 0 | 0 |
| P | 0 | 0 |

| | Q | Y |
|---|---|---|
| Q | P | 0 |
| Y | 0 | $P+Z$ |

| | J | Z | P |
|---|---|---|---|
| J | J | Z | P |
| Z | Z | 0 | 0 |
| P | P | 0 | 0 |

| | Q | Y |
|---|---|---|
| J | Q | Y |
| Z | 0 | 0 |
| P | 0 | 0 |

| | Q | Y |
|---|---|---|
| Q | P | P |
| Y | P | 0 |

| | J | Z | P |
|---|---|---|---|
| J | J | Z | P |
| Z | Z | 0 | 0 |
| P | P | 0 | 0 |

| | Q | Y |
|---|---|---|
| J | Q | Y |
| Z | 0 | 0 |
| P | 0 | 0 |

| | Q | Y |
|---|---|---|
| Q | P | P |
| Y | P | P |

| | J | Z | P |
|---|---|---|---|
| J | J | Z | P |
| Z | Z | 0 | 0 |
| P | P | 0 | 0 |

| | Q | Y |
|---|---|---|
| J | Q | Y |
| Z | 0 | 0 |
| P | 0 | 0 |

| | Q | Y |
|---|---|---|
| Q | P | P |
| Y | P | Z |

| | J | Z | P |
|---|---|---|---|
| J | J | Z | P |
| Z | Z | 0 | 0 |
| P | P | 0 | 0 |

| | Q | Y |
|---|---|---|
| J | Q | Y |
| Z | 0 | 0 |
| P | 0 | 0 |

| | Q | Y |
|---|---|---|
| Q | P | P |
| Y | P | $P+Z$ |

| | J | Z | P |
|---|---|---|---|
| J | J | Z | P |
| Z | Z | 0 | 0 |
| P | P | 0 | 0 |

| | Q | Y |
|---|---|---|
| J | Q | Y |
| Z | 0 | 0 |
| P | 0 | 0 |

| | Q | Y |
|---|---|---|
| Q | P | Z |
| Y | Z | 0 |

| | J | Z | P |
|---|---|---|---|
| J | J | Z | P |
| Z | Z | 0 | 0 |
| P | P | 0 | 0 |

| | Q | Y |
|---|---|---|
| J | Q | Y |
| Z | 0 | 0 |
| P | 0 | 0 |

| | Q | Y |
|---|---|---|
| Q | P | Z |
| Y | Z | P |

| | J | Z | P |
|---|---|---|---|
| J | J | Z | P |
| Z | Z | 0 | 0 |
| P | P | 0 | 0 |

| | Q | Y |
|---|---|---|
| J | Q | Y |
| Z | 0 | 0 |
| P | 0 | 0 |

| | Q | Y |
|---|---|---|
| Q | P | Z |
| Y | Z | Z |

| | J | Z | P |
|---|---|---|---|
| J | J | Z | P |
| Z | Z | 0 | 0 |
| P | P | 0 | 0 |

| | Q | Y |
|---|---|---|
| J | Q | Y |
| Z | 0 | 0 |
| P | 0 | 0 |

| | Q | Y |
|---|---|---|
| Q | P | Z |
| Y | Z | $P+Z$ |

| | J | Z | P |
|---|---|---|---|
| J | J | Z | P |
| Z | Z | 0 | 0 |
| P | P | 0 | 0 |

| | Q | Y |
|---|---|---|
| J | Q | Y |
| Z | 0 | 0 |
| P | 0 | 0 |

| | Q | Y |
|---|---|---|
| Q | P | $P+Z$ |
| Y | $P+Z$ | 0 |

| | J | Z | P |
|---|---|---|---|
| J | J | Z | P |
| Z | Z | 0 | 0 |
| P | P | 0 | 0 |

| | Q | Y |
|---|---|---|
| J | Q | Y |
| Z | 0 | 0 |
| P | 0 | 0 |

| | Q | Y |
|---|---|---|
| Q | P | $P+Z$ |
| Y | $P+Z$ | P |

| | J | Z | P |
|---|---|---|---|
| J | J | Z | P |
| Z | Z | 0 | 0 |
| P | P | 0 | 0 |

| | Q | Y |
|---|---|---|
| J | Q | Y |
| Z | 0 | 0 |
| P | 0 | 0 |

| | Q | Y |
|---|---|---|
| Q | P | $P+Z$ |
| Y | $P+Z$ | Z |

| | J | Z | P |
|---|---|---|---|
| J | J | Z | P |
| Z | Z | 0 | 0 |
| P | P | 0 | 0 |

| | Q | Y |
|---|---|---|
| J | Q | Y |
| Z | 0 | 0 |
| P | 0 | 0 |

| | Q | Y |
|---|---|---|
| Q | P | $P+Z$ |
| Y | $P+Z$ | $P+Z$ |

| | J | Z | P |
|---|---|---|---|
| J | J | Z | P |
| Z | Z | 0 | 0 |
| P | P | 0 | 0 |

| | Q | Y |
|---|---|---|
| J | Q | Y |
| Z | 0 | 0 |
| P | 0 | 0 |

| | Q | Y |
|---|---|---|
| Q | $P+Z$ | 0 |
| Y | 0 | 0 |

| | J | Z | P |
|---|---|---|---|
| J | J | Z | P |
| Z | Z | 0 | 0 |
| P | P | 0 | 0 |

| | Q | Y |
|---|---|---|
| J | Q | Y |
| Z | Y | 0 |
| P | 0 | 0 |

| | Q | Y |
|---|---|---|
| Q | $P+Z$ | 0 |
| Y | 0 | 0 |

| | J | Z | P |
|---|---|---|---|
| J | J | Z | P |
| Z | Z | 0 | 0 |
| P | P | 0 | 0 |

| | Q | Y |
|---|---|---|
| J | Q | Y |
| Z | 0 | 0 |
| P | Y | 0 |

| | Q | Y |
|---|---|---|
| Q | $P+Z$ | 0 |
| Y | 0 | 0 |

| | J | Z | P |
|---|---|---|---|
| J | J | Z | P |
| Z | Z | 0 | 0 |
| P | P | 0 | 0 |

| | Q | Y |
|---|---|---|
| J | Q | Y |
| Z | Y | 0 |
| P | Y | 0 |

| | Q | Y |
|---|---|---|
| Q | $P+Z$ | 0 |
| Y | 0 | 0 |

| | J | Z | P |
|---|---|---|---|
| J | J | Z | P |
| Z | Z | 0 | 0 |
| P | P | 0 | 0 |

| | Q | Y |
|---|---|---|
| J | Q | Y |
| Z | 0 | 0 |
| P | 0 | 0 |

| | Q | Y |
|---|---|---|
| Q | $P+Z$ | 0 |
| Y | 0 | P |

| | J | Z | P |
|---|---|---|---|
| J | J | Z | P |
| Z | Z | 0 | 0 |
| P | P | 0 | 0 |

| | Q | Y |
|---|---|---|
| J | Q | Y |
| Z | 0 | 0 |
| P | 0 | 0 |

| | Q | Y |
|---|---|---|
| Q | $P+Z$ | 0 |
| Y | 0 | Z |

| | J | Z | P |
|---|---|---|---|
| J | J | Z | P |
| Z | Z | 0 | 0 |
| P | P | 0 | 0 |

| | Q | Y |
|---|---|---|
| J | Q | Y |
| Z | 0 | 0 |
| P | 0 | 0 |

| | Q | Y |
|---|---|---|
| Q | $P+Z$ | 0 |
| Y | 0 | $P+Z$ |

| | J | Z | P |
|---|---|---|---|
| J | J | Z | P |
| Z | Z | 0 | 0 |
| P | P | 0 | 0 |

| | Q | Y |
|---|---|---|
| J | Q | Y |
| Z | 0 | 0 |
| P | 0 | 0 |

| | Q | Y |
|---|---|---|
| Q | $P+Z$ | P |
| Y | P | 0 |

| | J | Z | P |
|---|---|---|---|
| J | J | Z | P |
| Z | Z | 0 | 0 |
| P | P | 0 | 0 |

| | Q | Y |
|---|---|---|
| J | Q | Y |
| Z | 0 | 0 |
| P | 0 | 0 |

| | Q | Y |
|---|---|---|
| Q | $P+Z$ | P |
| Y | P | P |

| | J | Z | P |
|---|---|---|---|
| J | J | Z | P |
| Z | Z | 0 | 0 |
| P | P | 0 | 0 |

| | Q | Y |
|---|---|---|
| J | Q | Y |
| Z | 0 | 0 |
| P | 0 | 0 |

| | Q | Y |
|---|---|---|
| Q | $P+Z$ | P |
| Y | P | Z |

| | J | Z | P |
|---|---|---|---|
| J | J | Z | P |
| Z | Z | 0 | 0 |
| P | P | 0 | 0 |

| | Q | Y |
|---|---|---|
| J | Q | Y |
| Z | 0 | 0 |
| P | 0 | 0 |

| | Q | Y |
|---|---|---|
| Q | $P+Z$ | P |
| Y | P | $P+Z$ |

| | J | Z | P |
|---|---|---|---|
| J | J | Z | P |
| Z | Z | 0 | 0 |
| P | P | 0 | 0 |

| | Q | Y |
|---|---|---|
| J | Q | Y |
| Z | 0 | 0 |
| P | 0 | 0 |

| | Q | Y |
|---|---|---|
| Q | $P+Z$ | Z |
| Y | Z | 0 |

| | J | Z | P |
|---|---|---|---|
| J | J | Z | P |
| Z | Z | 0 | 0 |
| P | P | 0 | 0 |

| | Q | Y |
|---|---|---|
| J | Q | Y |
| Z | 0 | 0 |
| P | 0 | 0 |

| | Q | Y |
|---|---|---|
| Q | $P+Z$ | Z |
| Y | Z | P |

| | J | Z | P |
|---|---|---|---|
| J | J | Z | P |
| Z | Z | 0 | 0 |
| P | P | 0 | 0 |

| | Q | Y |
|---|---|---|
| J | Q | Y |
| Z | 0 | 0 |
| P | 0 | 0 |

| | Q | Y |
|---|---|---|
| Q | $P+Z$ | Z |
| Y | Z | Z |

| | J | Z | P |
|---|---|---|---|
| J | J | Z | P |
| Z | Z | 0 | 0 |
| P | P | 0 | 0 |

| | Q | Y |
|---|---|---|
| J | Q | Y |
| Z | 0 | 0 |
| P | 0 | 0 |

| | Q | Y |
|---|---|---|
| Q | $P+Z$ | Z |
| Y | Z | $P+Z$ |

| | J | Z | P |
|---|---|---|---|
| J | J | Z | P |
| Z | Z | 0 | 0 |
| P | P | 0 | 0 |

| | Q | Y |
|---|---|---|
| J | Q | Y |
| Z | 0 | 0 |
| P | 0 | 0 |

| | Q | Y |
|---|---|---|
| Q | $P+Z$ | $P+Z$ |
| Y | $P+Z$ | 0 |

| | J | Z | P |
|---|---|---|---|
| J | J | Z | P |
| Z | Z | 0 | 0 |
| P | P | 0 | 0 |

| | Q | Y |
|---|---|---|
| J | Q | Y |
| Z | 0 | 0 |
| P | 0 | 0 |

| | Q | Y |
|---|---|---|
| Q | $P+Z$ | $P+Z$ |
| Y | $P+Z$ | P |

| | J | Z | P |
|---|---|---|---|
| J | J | Z | P |
| Z | Z | 0 | 0 |
| P | P | 0 | 0 |

| | Q | Y |
|---|---|---|
| J | Q | Y |
| Z | 0 | 0 |
| P | 0 | 0 |

| | Q | Y |
|---|---|---|
| Q | $P+Z$ | $P+Z$ |
| Y | $P+Z$ | Z |

| | J | Z | P |
|---|---|---|---|
| J | J | Z | P |
| Z | Z | 0 | 0 |
| P | P | 0 | 0 |

| | Q | Y |
|---|---|---|
| J | Q | Y |
| Z | 0 | 0 |
| P | 0 | 0 |

| | Q | Y |
|---|---|---|
| Q | $P+Z$ | $P+Z$ |
| Y | $P+Z$ | $P+Z$ |

| | J | Z | P |
|---|---|---|---|
| J | J | Z | P |
| Z | Z | 0 | 0 |
| P | P | 0 | Z |

| | Q | Y |
|---|---|---|
| J | Q | Y |
| Z | 0 | 0 |
| P | Y | 0 |

| | Q | Y |
|---|---|---|
| Q | P | Z |
| Y | Z | 0 |

| | J | Z | P |
|---|---|---|---|
| J | J | Z | P |
| Z | Z | 0 | 0 |
| P | P | 0 | Z |

| | Q | Y |
|---|---|---|
| J | Q | Y |
| Z | 0 | 0 |
| P | Y | 0 |

| | Q | Y |
|---|---|---|
| Q | $P+Z$ | Z |
| Y | Z | 0 |

| | J | Z | P |
|---|---|---|---|
| J | J | Z | P |
| Z | Z | Z | 0 |
| P | P | 0 | 0 |

| | Q | Y |
|---|---|---|
| J | Q | Y |
| Z | 0 | 0 |
| P | 0 | 0 |

| | Q | Y |
|---|---|---|
| Q | P | 0 |
| Y | 0 | 0 |

| | J | Z | P |
|---|---|---|---|
| J | J | Z | P |
| Z | Z | Z | 0 |
| P | P | 0 | 0 |

| | Q | Y |
|---|---|---|
| J | Q | Y |
| Z | 0 | Y |
| P | 0 | 0 |

| | Q | Y |
|---|---|---|
| Q | P | 0 |
| Y | 0 | 0 |

| | J | Z | P |
|---|---|---|---|
| J | J | Z | P |
| Z | Z | Z | 0 |
| P | P | 0 | 0 |

| | Q | Y |
|---|---|---|
| J | Q | Y |
| Z | Y | Y |
| P | 0 | 0 |

| | Q | Y |
|---|---|---|
| Q | P | 0 |
| Y | 0 | 0 |

| | J | Z | P |
|---|---|---|---|
| J | J | Z | P |
| Z | Z | Z | 0 |
| P | P | 0 | 0 |

| | Q | Y |
|---|---|---|
| J | Q | Y |
| Z | 0 | 0 |
| P | Y | 0 |

| | Q | Y |
|---|---|---|
| Q | P | 0 |
| Y | 0 | 0 |

| | J | Z | P |
|---|---|---|---|
| J | J | Z | P |
| Z | Z | Z | 0 |
| P | P | 0 | 0 |

| | Q | Y |
|---|---|---|
| J | Q | Y |
| Z | 0 | 0 |
| P | 0 | 0 |

| | Q | Y |
|---|---|---|
| Q | P | 0 |
| Y | 0 | P |

| | J | Z | P |
|---|---|---|---|
| J | J | Z | P |
| Z | Z | Z | 0 |
| P | P | 0 | 0 |

| | Q | Y |
|---|---|---|
| J | Q | Y |
| Z | 0 | Y |
| P | 0 | 0 |

| | Q | Y |
|---|---|---|
| Q | P | 0 |
| Y | 0 | Z |

| | J | Z | P |
|---|---|---|---|
| J | J | Z | P |
| Z | Z | Z | 0 |
| P | P | 0 | 0 |

| | Q | Y |
|---|---|---|
| J | Q | Y |
| Z | 0 | 0 |
| P | 0 | 0 |

| | Q | Y |
|---|---|---|
| Q | P | P |
| Y | P | 0 |

| | J | Z | P |
|---|---|---|---|
| J | J | Z | P |
| Z | Z | Z | 0 |
| P | P | 0 | 0 |

| | Q | Y |
|---|---|---|
| J | Q | Y |
| Z | 0 | 0 |
| P | 0 | 0 |

| | Q | Y |
|---|---|---|
| Q | P | P |
| Y | P | P |

| | J | Z | P |
|---|---|---|---|
| J | J | Z | P |
| Z | Z | Z | 0 |
| P | P | 0 | 0 |

| | Q | Y |
|---|---|---|
| J | Q | Y |
| Z | Y | Y |
| P | 0 | 0 |

| | Q | Y |
|---|---|---|
| Q | $P+Z$ | Z |
| Y | Z | Z |

| | J | Z | P |
|---|---|---|---|
| J | J | Z | P |
| Z | Z | Z | P |
| P | P | P | 0 |

| | Q | Y |
|---|---|---|
| J | Q | Y |
| Z | Q | 0 |
| P | 0 | 0 |

| | Q | Y |
|---|---|---|
| Q | P | 0 |
| Y | 0 | 0 |

| | J | Z | P |
|---|---|---|---|
| J | J | Z | P |
| Z | Z | Z | P |
| P | P | P | 0 |

| | Q | Y |
|---|---|---|
| J | Q | Y |
| Z | Q | Y |
| P | 0 | 0 |

| | Q | Y |
|---|---|---|
| Q | P | 0 |
| Y | 0 | 0 |

| | J | Z | P |
|---|---|---|---|
| J | J | Z | P |
| Z | Z | Z | P |
| P | P | P | 0 |

| | Q | Y |
|---|---|---|
| J | Q | Y |
| Z | Q | Y |
| P | Y | 0 |

| | Q | Y |
|---|---|---|
| Q | P | 0 |
| Y | 0 | 0 |

| | J | Z | P |
|---|---|---|---|
| J | J | Z | P |
| Z | Z | Z | P |
| P | P | P | 0 |

| | Q | Y |
|---|---|---|
| J | Q | Y |
| Z | Q | Y |
| P | 0 | 0 |

| | Q | Y |
|---|---|---|
| Q | P | 0 |
| Y | 0 | P |

| | J | Z | P |
|---|---|---|---|
| J | J | Z | P |
| Z | Z | Z | P |
| P | P | P | 0 |

| | Q | Y |
|---|---|---|
| J | Q | Y |
| Z | Q | Y |
| P | 0 | 0 |

| | Q | Y |
|---|---|---|
| Q | P | P |
| Y | P | 0 |

| | J | Z | P |
|---|---|---|---|
| J | J | Z | P |
| Z | Z | Z | P |
| P | P | P | 0 |

| | Q | Y |
|---|---|---|
| J | Q | Y |
| Z | Q | Q |
| P | 0 | 0 |

| | Q | Y |
|---|---|---|
| Q | P | P |
| Y | P | P |

| | J | Z | P |
|---|---|---|---|
| J | J | Z | P |
| Z | Z | Z | P |
| P | P | P | 0 |

| | Q | Y |
|---|---|---|
| J | Q | Y |
| Z | Q | Y |
| P | 0 | 0 |

| | Q | Y |
|---|---|---|
| Q | P | P |
| Y | P | P |

| | J | Z | P |
|---|---|---|---|
| J | J | Z | P |
| Z | Z | Z | P |
| P | P | P | 0 |

| | Q | Y |
|---|---|---|
| J | Q | Y |
| Z | Y | Y |
| P | 0 | 0 |

| | Q | Y |
|---|---|---|
| Q | P | P |
| Y | P | P |

| | J | Z | P |
|---|---|---|---|
| J | J | Z | P |
| Z | Z | Z | P |
| P | P | P | 0 |

| | Q | Y |
|---|---|---|
| J | Q | Y |
| Z | Q | Y |
| P | Y | 0 |

| | Q | Y |
|---|---|---|
| Q | $P+Z$ | P |
| Y | P | 0 |

| | J | Z | P |
|---|---|---|---|
| J | J | Z | P |
| Z | Z | Z | P |
| P | P | P | Z |

| | Q | Y |
|---|---|---|
| J | Q | Y |
| Z | Q | Y |
| P | Y | Q |

| | Q | Y |
|---|---|---|
| Q | P | Z |
| Y | Z | P |

| | J | Z | P |
|---|---|---|---|
| J | J | Z | P |
| Z | Z | Z | P |
| P | P | P | Z |

| | Q | Y |
|---|---|---|
| J | Q | Y |
| Z | Q | 0 |
| P | Q | 0 |

| | Q | Y |
|---|---|---|
| Q | $P+Z$ | 0 |
| Y | 0 | 0 |

| | J | Z | P |
|---|---|---|---|
| J | J | Z | P |
| Z | Z | Z | P |
| P | P | P | Z |

| | Q | Y |
|---|---|---|
| J | Q | Y |
| Z | Q | Q |
| P | Q | Q |

| | Q | Y |
|---|---|---|
| Q | $P+Z$ | $P+Z$ |
| Y | $P+Z$ | $P+Z$ |

| | J | Z | P |
|---|---|---|---|
| J | J | Z | P |
| Z | Z | Z | P |
| P | P | P | Z |

| | Q | Y |
|---|---|---|
| J | Q | Y |
| Z | Q | Y |
| P | Y | Q |

| | Q | Y |
|---|---|---|
| Q | $P+Z$ | $P+Z$ |
| Y | $P+Z$ | $P+Z$ |

| | J | Z | P |
|---|---|---|---|
| J | J | Z | P |
| Z | Z | Z | P |
| P | P | P | Z |

| | Q | Y |
|---|---|---|
| J | Q | Y |
| Z | Y | Y |
| P | Y | Y |

| | Q | Y |
|---|---|---|
| Q | $P+Z$ | $P+Z$ |
| Y | $P+Z$ | $P+Z$ |

| | J | Z | P |
|---|---|---|---|
| J | J | Z | P |
| Z | Z | Z | P |
| P | P | P | Z |

| | Q | Y |
|---|---|---|
| J | Q | Y |
| Z | Q | Q |
| P | Q | Q |

| | Q | Y |
|---|---|---|
| Q | $P+Z$ | $P+Z$ |
| Y | $P+Z$ | $J+P$ |

| | J | Z | P |
|---|---|---|---|
| J | J | Z | P |
| Z | Z | Z | P |
| P | P | P | Z |

| | Q | Y |
|---|---|---|
| J | Q | Y |
| Z | Y | Y |
| P | Y | Y |

| | Q | Y |
|---|---|---|
| Q | $J+P$ | $P+Z$ |
| Y | $P+Z$ | $P+Z$ |

| | J | Z | P |
|---|---|---|---|
| J | J | Z | P |
| Z | Z | J | P |
| P | P | P | 0 |

| | Q | Y |
|---|---|---|
| J | Q | Y |
| Z | Q | Y |
| P | 0 | 0 |

| | Q | Y |
|---|---|---|
| Q | P | 0 |
| Y | 0 | 0 |

| | J | Z | P |
|---|---|---|---|
| J | J | Z | P |
| Z | Z | J | P |
| P | P | P | 0 |

| | Q | Y |
|---|---|---|
| J | Q | Y |
| Z | Q | Y |
| P | Y | 0 |

| | Q | Y |
|---|---|---|
| Q | P | 0 |
| Y | 0 | 0 |

| | J | Z | P |
|---|---|---|---|
| J | J | Z | P |
| Z | Z | J | P |
| P | P | P | 0 |

| | Q | Y |
|---|---|---|
| J | Q | Y |
| Z | Q | Y |
| P | 0 | 0 |

| | Q | Y |
|---|---|---|
| Q | P | 0 |
| Y | 0 | P |

| | J | Z | P |
|---|---|---|---|
| J | J | Z | P |
| Z | Z | J | P |
| P | P | P | 0 |

| | Q | Y |
|---|---|---|
| J | Q | Y |
| Z | Q | Y |
| P | 0 | 0 |

| | Q | Y |
|---|---|---|
| Q | P | P |
| Y | P | 0 |

| | J | Z | P |
|---|---|---|---|
| J | J | Z | P |
| Z | Z | J | P |
| P | P | P | 0 |

| | Q | Y |
|---|---|---|
| J | Q | Y |
| Z | Q | Y |
| P | 0 | 0 |

| | Q | Y |
|---|---|---|
| Q | P | P |
| Y | P | P |

| | J | Z | P |
|---|---|---|---|
| J | J | Z | P |
| Z | Z | J | P |
| P | P | P | 0 |

| | Q | Y |
|---|---|---|
| J | Q | Y |
| Z | Y | Q |
| P | 0 | 0 |

| | Q | Y |
|---|---|---|
| Q | P | P |
| Y | P | P |

Total number of resonant non-standard cases: 31.

| | J | Z | P |
|---|---|---|---|
| J | J | Z | P |
| Z | Z | 0 | 0 |
| P | P | 0 | 0 |

| | Q | Y |
|---|---|---|
| J | Q | Y |
| Z | 0 | 0 |
| P | 0 | 0 |

| | Q | Y |
|---|---|---|
| Q | Z | 0 |
| Y | 0 | 0 |

| | J | Z | P |
|---|---|---|---|
| J | J | Z | P |
| Z | Z | 0 | 0 |
| P | P | 0 | 0 |

| | Q | Y |
|---|---|---|
| J | Q | Y |
| Z | Y | 0 |
| P | 0 | 0 |

| | Q | Y |
|---|---|---|
| Q | Z | 0 |
| Y | 0 | 0 |

| | J | Z | P |
|---|---|---|---|
| J | J | Z | P |
| Z | Z | 0 | 0 |
| P | P | 0 | 0 |

| | Q | Y |
|---|---|---|
| J | Q | Y |
| Z | 0 | 0 |
| P | Y | 0 |

| | Q | Y |
|---|---|---|
| Q | Z | 0 |
| Y | 0 | 0 |

| | J | Z | P |
|---|---|---|---|
| J | J | Z | P |
| Z | Z | 0 | 0 |
| P | P | 0 | 0 |

| | Q | Y |
|---|---|---|
| J | Q | Y |
| Z | Y | 0 |
| P | Y | 0 |

| | Q | Y |
|---|---|---|
| Q | Z | 0 |
| Y | 0 | 0 |

| | J | Z | P |
|---|---|---|---|
| J | J | Z | P |
| Z | Z | 0 | 0 |
| P | P | 0 | 0 |

| | Q | Y |
|---|---|---|
| J | Q | Y |
| Z | 0 | 0 |
| P | 0 | 0 |

| | Q | Y |
|---|---|---|
| Q | Z | 0 |
| Y | 0 | P |

| | J | Z | P |
|---|---|---|---|
| J | J | Z | P |
| Z | Z | 0 | 0 |
| P | P | 0 | 0 |

| | Q | Y |
|---|---|---|
| J | Q | Y |
| Z | 0 | 0 |
| P | 0 | 0 |

| | Q | Y |
|---|---|---|
| Q | Z | 0 |
| Y | 0 | Z |

| | J | Z | P |
|---|---|---|---|
| J | J | Z | P |
| Z | Z | 0 | 0 |
| P | P | 0 | 0 |

| | Q | Y |
|---|---|---|
| J | Q | Y |
| Z | 0 | 0 |
| P | 0 | 0 |

| | Q | Y |
|---|---|---|
| Q | Z | 0 |
| Y | 0 | $P+Z$ |

| | J | Z | P |
|---|---|---|---|
| J | J | Z | P |
| Z | Z | 0 | 0 |
| P | P | 0 | 0 |

| | Q | Y |
|---|---|---|
| J | Q | Y |
| Z | 0 | 0 |
| P | 0 | 0 |

| | Q | Y |
|---|---|---|
| Q | Z | P |
| Y | P | 0 |

| | $J$ | $Z$ | $P$ |
|---|---|---|---|
| $J$ | $J$ | $Z$ | $P$ |
| $Z$ | $Z$ | 0 | 0 |
| $P$ | $P$ | 0 | 0 |

| | $Q$ | $Y$ |
|---|---|---|
| $J$ | $Q$ | $Y$ |
| $Z$ | 0 | 0 |
| $P$ | 0 | 0 |

| | $Q$ | $Y$ |
|---|---|---|
| $Q$ | $Z$ | $P$ |
| $Y$ | $P$ | $P$ |

| | $J$ | $Z$ | $P$ |
|---|---|---|---|
| $J$ | $J$ | $Z$ | $P$ |
| $Z$ | $Z$ | 0 | 0 |
| $P$ | $P$ | 0 | 0 |

| | $Q$ | $Y$ |
|---|---|---|
| $J$ | $Q$ | $Y$ |
| $Z$ | 0 | 0 |
| $P$ | 0 | 0 |

| | $Q$ | $Y$ |
|---|---|---|
| $Q$ | $Z$ | $P$ |
| $Y$ | $P$ | $Z$ |

| | $J$ | $Z$ | $P$ |
|---|---|---|---|
| $J$ | $J$ | $Z$ | $P$ |
| $Z$ | $Z$ | 0 | 0 |
| $P$ | $P$ | 0 | 0 |

| | $Q$ | $Y$ |
|---|---|---|
| $J$ | $Q$ | $Y$ |
| $Z$ | 0 | 0 |
| $P$ | 0 | 0 |

| | $Q$ | $Y$ |
|---|---|---|
| $Q$ | $Z$ | $P$ |
| $Y$ | $P$ | $P+Z$ |

| | $J$ | $Z$ | $P$ |
|---|---|---|---|
| $J$ | $J$ | $Z$ | $P$ |
| $Z$ | $Z$ | 0 | 0 |
| $P$ | $P$ | 0 | 0 |

| | $Q$ | $Y$ |
|---|---|---|
| $J$ | $Q$ | $Y$ |
| $Z$ | 0 | 0 |
| $P$ | 0 | 0 |

| | $Q$ | $Y$ |
|---|---|---|
| $Q$ | $Z$ | $Z$ |
| $Y$ | $Z$ | 0 |

| | $J$ | $Z$ | $P$ |
|---|---|---|---|
| $J$ | $J$ | $Z$ | $P$ |
| $Z$ | $Z$ | 0 | 0 |
| $P$ | $P$ | 0 | 0 |

| | $Q$ | $Y$ |
|---|---|---|
| $J$ | $Q$ | $Y$ |
| $Z$ | 0 | 0 |
| $P$ | 0 | 0 |

| | $Q$ | $Y$ |
|---|---|---|
| $Q$ | $Z$ | $Z$ |
| $Y$ | $Z$ | $P$ |

| | $J$ | $Z$ | $P$ |
|---|---|---|---|
| $J$ | $J$ | $Z$ | $P$ |
| $Z$ | $Z$ | 0 | 0 |
| $P$ | $P$ | 0 | 0 |

| | $Q$ | $Y$ |
|---|---|---|
| $J$ | $Q$ | $Y$ |
| $Z$ | 0 | 0 |
| $P$ | 0 | 0 |

| | $Q$ | $Y$ |
|---|---|---|
| $Q$ | $Z$ | $Z$ |
| $Y$ | $Z$ | $Z$ |

| | $J$ | $Z$ | $P$ |
|---|---|---|---|
| $J$ | $J$ | $Z$ | $P$ |
| $Z$ | $Z$ | 0 | 0 |
| $P$ | $P$ | 0 | 0 |

| | $Q$ | $Y$ |
|---|---|---|
| $J$ | $Q$ | $Y$ |
| $Z$ | 0 | 0 |
| $P$ | 0 | 0 |

| | $Q$ | $Y$ |
|---|---|---|
| $Q$ | $Z$ | $Z$ |
| $Y$ | $Z$ | $P+Z$ |

| | $J$ | $Z$ | $P$ |
|---|---|---|---|
| $J$ | $J$ | $Z$ | $P$ |
| $Z$ | $Z$ | 0 | 0 |
| $P$ | $P$ | 0 | 0 |

| | $Q$ | $Y$ |
|---|---|---|
| $J$ | $Q$ | $Y$ |
| $Z$ | 0 | 0 |
| $P$ | 0 | 0 |

| | $Q$ | $Y$ |
|---|---|---|
| $Q$ | $Z$ | $P+Z$ |
| $Y$ | $P+Z$ | 0 |

| | $J$ | $Z$ | $P$ |
|---|---|---|---|
| $J$ | $J$ | $Z$ | $P$ |
| $Z$ | $Z$ | 0 | 0 |
| $P$ | $P$ | 0 | 0 |

| | $Q$ | $Y$ |
|---|---|---|
| $J$ | $Q$ | $Y$ |
| $Z$ | 0 | 0 |
| $P$ | 0 | 0 |

| | $Q$ | $Y$ |
|---|---|---|
| $Q$ | $Z$ | $P+Z$ |
| $Y$ | $P+Z$ | $P$ |

| | $J$ | $Z$ | $P$ |
|---|---|---|---|
| $J$ | $J$ | $Z$ | $P$ |
| $Z$ | $Z$ | 0 | 0 |
| $P$ | $P$ | 0 | 0 |

| | $Q$ | $Y$ |
|---|---|---|
| $J$ | $Q$ | $Y$ |
| $Z$ | 0 | 0 |
| $P$ | 0 | 0 |

| | $Q$ | $Y$ |
|---|---|---|
| $Q$ | $Z$ | $P+Z$ |
| $Y$ | $P+Z$ | $Z$ |

| | $J$ | $Z$ | $P$ |
|---|---|---|---|
| $J$ | $J$ | $Z$ | $P$ |
| $Z$ | $Z$ | 0 | 0 |
| $P$ | $P$ | 0 | 0 |

| | $Q$ | $Y$ |
|---|---|---|
| $J$ | $Q$ | $Y$ |
| $Z$ | 0 | 0 |
| $P$ | 0 | 0 |

| | $Q$ | $Y$ |
|---|---|---|
| $Q$ | $Z$ | $P+Z$ |
| $Y$ | $P+Z$ | $P+Z$ |

| | $J$ | $Z$ | $P$ |
|---|---|---|---|
| $J$ | $J$ | $Z$ | $P$ |
| $Z$ | $Z$ | 0 | 0 |
| $P$ | $P$ | 0 | $Z$ |

| | $Q$ | $Y$ |
|---|---|---|
| $J$ | $Q$ | $Y$ |
| $Z$ | 0 | 0 |
| $P$ | 0 | 0 |

| | $Q$ | $Y$ |
|---|---|---|
| $Q$ | $Z$ | 0 |
| $Y$ | 0 | 0 |

| | $J$ | $Z$ | $P$ |
|---|---|---|---|
| $J$ | $J$ | $Z$ | $P$ |
| $Z$ | $Z$ | 0 | 0 |
| $P$ | $P$ | 0 | $Z$ |

| | $Q$ | $Y$ |
|---|---|---|
| $J$ | $Q$ | $Y$ |
| $Z$ | 0 | 0 |
| $P$ | $Y$ | 0 |

| | $Q$ | $Y$ |
|---|---|---|
| $Q$ | $Z$ | 0 |
| $Y$ | 0 | 0 |

| | $J$ | $Z$ | $P$ |
|---|---|---|---|
| $J$ | $J$ | $Z$ | $P$ |
| $Z$ | $Z$ | 0 | 0 |
| $P$ | $P$ | 0 | $Z$ |

| | $Q$ | $Y$ |
|---|---|---|
| $J$ | $Q$ | $Y$ |
| $Z$ | 0 | 0 |
| $P$ | 0 | 0 |

| | $Q$ | $Y$ |
|---|---|---|
| $Q$ | $Z$ | 0 |
| $Y$ | 0 | $Z$ |

| | $J$ | $Z$ | $P$ |
|---|---|---|---|
| $J$ | $J$ | $Z$ | $P$ |
| $Z$ | $Z$ | 0 | 0 |
| $P$ | $P$ | 0 | $Z$ |

| | $Q$ | $Y$ |
|---|---|---|
| $J$ | $Q$ | $Y$ |
| $Z$ | 0 | 0 |
| $P$ | 0 | 0 |

| | $Q$ | $Y$ |
|---|---|---|
| $Q$ | $Z$ | $Z$ |
| $Y$ | $Z$ | 0 |

| | $J$ | $Z$ | $P$ |
|---|---|---|---|
| $J$ | $J$ | $Z$ | $P$ |
| $Z$ | $Z$ | 0 | 0 |
| $P$ | $P$ | 0 | $Z$ |

| | $Q$ | $Y$ |
|---|---|---|
| $J$ | $Q$ | $Y$ |
| $Z$ | 0 | 0 |
| $P$ | 0 | 0 |

| | $Q$ | $Y$ |
|---|---|---|
| $Q$ | $Z$ | $Z$ |
| $Y$ | $Z$ | $Z$ |

| | $J$ | $Z$ | $P$ |
|---|---|---|---|
| $J$ | $J$ | $Z$ | $P$ |
| $Z$ | $Z$ | $Z$ | 0 |
| $P$ | $P$ | 0 | 0 |

| | $Q$ | $Y$ |
|---|---|---|
| $J$ | $Q$ | $Y$ |
| $Z$ | $Q$ | 0 |
| $P$ | 0 | 0 |

| | $Q$ | $Y$ |
|---|---|---|
| $Q$ | $Z$ | 0 |
| $Y$ | 0 | 0 |

| | $J$ | $Z$ | $P$ |
|---|---|---|---|
| $J$ | $J$ | $Z$ | $P$ |
| $Z$ | $Z$ | $Z$ | 0 |
| $P$ | $P$ | 0 | 0 |

| | $Q$ | $Y$ |
|---|---|---|
| $J$ | $Q$ | $Y$ |
| $Z$ | $Q$ | 0 |
| $P$ | 0 | 0 |

| | $Q$ | $Y$ |
|---|---|---|
| $Q$ | $Z$ | 0 |
| $Y$ | 0 | $P$ |

| | $J$ | $Z$ | $P$ |
|---|---|---|---|
| $J$ | $J$ | $Z$ | $P$ |
| $Z$ | $Z$ | $Z$ | 0 |
| $P$ | $P$ | 0 | 0 |

| | $Q$ | $Y$ |
|---|---|---|
| $J$ | $Q$ | $Y$ |
| $Z$ | $Q$ | $Q$ |
| $P$ | 0 | 0 |

| | $Q$ | $Y$ |
|---|---|---|
| $Q$ | $Z$ | $Z$ |
| $Y$ | $Z$ | $Z$ |

| | $J$ | $Z$ | $P$ |
|---|---|---|---|
| $J$ | $J$ | $Z$ | $P$ |
| $Z$ | $Z$ | $Z$ | 0 |
| $P$ | $P$ | 0 | 0 |

| | $Q$ | $Y$ |
|---|---|---|
| $J$ | $Q$ | $Y$ |
| $Z$ | $Y$ | $Y$ |
| $P$ | 0 | 0 |

| | $Q$ | $Y$ |
|---|---|---|
| $Q$ | $Z$ | $Z$ |
| $Y$ | $Z$ | $Z$ |

| | $J$ | $Z$ | $P$ |
|---|---|---|---|
| $J$ | $J$ | $Z$ | $P$ |
| $Z$ | $Z$ | $Z$ | 0 |
| $P$ | $P$ | 0 | 0 |

| | $Q$ | $Y$ |
|---|---|---|
| $J$ | $Q$ | $Y$ |
| $Z$ | $Q$ | $Q$ |
| $P$ | 0 | 0 |

| | $Q$ | $Y$ |
|---|---|---|
| $Q$ | $Z$ | $Z$ |
| $Y$ | $Z$ | $P+Z$ |

| | $J$ | $Z$ | $P$ |
|---|---|---|---|
| $J$ | $J$ | $Z$ | $P$ |
| $Z$ | $Z$ | $Z$ | $P$ |
| $P$ | $P$ | $P$ | 0 |

| | $Q$ | $Y$ |
|---|---|---|
| $J$ | $Q$ | $Y$ |
| $Z$ | $Q$ | $Y$ |
| $P$ | $Y$ | 0 |

| | $Q$ | $Y$ |
|---|---|---|
| $Q$ | $Z$ | $P$ |
| $Y$ | $P$ | 0 |

| | $J$ | $Z$ | $P$ |
|---|---|---|---|
| $J$ | $J$ | $Z$ | $P$ |
| $Z$ | $Z$ | $Z$ | $P$ |
| $P$ | $P$ | $P$ | $Z$ |

| | $Q$ | $Y$ |
|---|---|---|
| $J$ | $Q$ | $Y$ |
| $Z$ | $Q$ | $Y$ |
| $P$ | $Y$ | $Q$ |

| | $Q$ | $Y$ |
|---|---|---|
| $Q$ | $Z$ | $P$ |
| $Y$ | $P$ | $Z$ |

## 2.3 JZPU+QY

**Total number of cases:** 667.
Total number of resonant SUGRA cases: 264.

| | $J$ | $Z$ | $P$ | $U$ |
|---|---|---|---|---|
| $J$ | $J$ | $Z$ | $P$ | $U$ |
| $Z$ | $Z$ | 0 | 0 | 0 |
| $P$ | $P$ | 0 | 0 | 0 |
| $U$ | $U$ | 0 | 0 | 0 |

| | $Q$ | $Y$ |
|---|---|---|
| $J$ | $Q$ | $Y$ |
| $Z$ | 0 | 0 |
| $P$ | 0 | 0 |
| $U$ | 0 | 0 |

| | $Q$ | $Y$ |
|---|---|---|
| $Q$ | $P$ | 0 |
| $Y$ | 0 | 0 |

| | $J$ | $Z$ | $P$ | $U$ |
|---|---|---|---|---|
| $J$ | $J$ | $Z$ | $P$ | $U$ |
| $Z$ | $Z$ | 0 | 0 | 0 |
| $P$ | $P$ | 0 | 0 | 0 |
| $U$ | $U$ | 0 | 0 | 0 |

| | $Q$ | $Y$ |
|---|---|---|
| $J$ | $Q$ | $Y$ |
| $Z$ | $Y$ | 0 |
| $P$ | 0 | 0 |
| $U$ | 0 | 0 |

| | $Q$ | $Y$ |
|---|---|---|
| $Q$ | $P$ | 0 |
| $Y$ | 0 | 0 |

| | $J$ | $Z$ | $P$ | $U$ |
|---|---|---|---|---|
| $J$ | $J$ | $Z$ | $P$ | $U$ |
| $Z$ | $Z$ | 0 | 0 | 0 |
| $P$ | $P$ | 0 | 0 | 0 |
| $U$ | $U$ | 0 | 0 | 0 |

| | $Q$ | $Y$ |
|---|---|---|
| $J$ | $Q$ | $Y$ |
| $Z$ | 0 | 0 |
| $P$ | 0 | 0 |
| $U$ | $Y$ | 0 |

| | $Q$ | $Y$ |
|---|---|---|
| $Q$ | $P$ | 0 |
| $Y$ | 0 | 0 |

| | $J$ | $Z$ | $P$ | $U$ |
|---|---|---|---|---|
| $J$ | $J$ | $Z$ | $P$ | $U$ |
| $Z$ | $Z$ | 0 | 0 | 0 |
| $P$ | $P$ | 0 | 0 | 0 |
| $U$ | $U$ | 0 | 0 | 0 |

| | $Q$ | $Y$ |
|---|---|---|
| $J$ | $Q$ | $Y$ |
| $Z$ | $Y$ | 0 |
| $P$ | 0 | 0 |
| $U$ | $Y$ | 0 |

| | $Q$ | $Y$ |
|---|---|---|
| $Q$ | $P$ | 0 |
| $Y$ | 0 | 0 |

| | $J$ | $Z$ | $P$ | $U$ |
|---|---|---|---|---|
| $J$ | $J$ | $Z$ | $P$ | $U$ |
| $Z$ | $Z$ | 0 | 0 | 0 |
| $P$ | $P$ | 0 | 0 | 0 |
| $U$ | $U$ | 0 | 0 | 0 |

| | $Q$ | $Y$ |
|---|---|---|
| $J$ | $Q$ | $Y$ |
| $Z$ | 0 | 0 |
| $P$ | $Y$ | 0 |
| $U$ | 0 | 0 |

| | $Q$ | $Y$ |
|---|---|---|
| $Q$ | $P$ | 0 |
| $Y$ | 0 | 0 |

| | $J$ | $Z$ | $P$ | $U$ |
|---|---|---|---|---|
| $J$ | $J$ | $Z$ | $P$ | $U$ |
| $Z$ | $Z$ | 0 | 0 | 0 |
| $P$ | $P$ | 0 | 0 | 0 |
| $U$ | $U$ | 0 | 0 | 0 |

| | $Q$ | $Y$ |
|---|---|---|
| $J$ | $Q$ | $Y$ |
| $Z$ | $Y$ | 0 |
| $P$ | $Y$ | 0 |
| $U$ | 0 | 0 |

| | $Q$ | $Y$ |
|---|---|---|
| $Q$ | $P$ | 0 |
| $Y$ | 0 | 0 |

| | $J$ | $Z$ | $P$ | $U$ |
|---|---|---|---|---|
| $J$ | $J$ | $Z$ | $P$ | $U$ |
| $Z$ | $Z$ | 0 | 0 | 0 |
| $P$ | $P$ | 0 | 0 | 0 |
| $U$ | $U$ | 0 | 0 | 0 |

| | $Q$ | $Y$ |
|---|---|---|
| $J$ | $Q$ | $Y$ |
| $Z$ | 0 | 0 |
| $P$ | 0 | 0 |
| $U$ | 0 | 0 |

| | $Q$ | $Y$ |
|---|---|---|
| $Q$ | $P$ | $P$ |
| $Y$ | $P$ | $U+Z$ |

| | $J$ | $Z$ | $P$ | $U$ |
|---|---|---|---|---|
| $J$ | $J$ | $Z$ | $P$ | $U$ |
| $Z$ | $Z$ | 0 | 0 | 0 |
| $P$ | $P$ | 0 | 0 | 0 |
| $U$ | $U$ | 0 | 0 | 0 |

| | $Q$ | $Y$ |
|---|---|---|
| $J$ | $Q$ | $Y$ |
| $Z$ | 0 | 0 |
| $P$ | $Y$ | 0 |
| $U$ | $Y$ | 0 |

| | $Q$ | $Y$ |
|---|---|---|
| $Q$ | $P$ | 0 |
| $Y$ | 0 | 0 |

| | $J$ | $Z$ | $P$ | $U$ |
|---|---|---|---|---|
| $J$ | $J$ | $Z$ | $P$ | $U$ |
| $Z$ | $Z$ | 0 | 0 | 0 |
| $P$ | $P$ | 0 | 0 | 0 |
| $U$ | $U$ | 0 | 0 | 0 |

| | $Q$ | $Y$ |
|---|---|---|
| $J$ | $Q$ | $Y$ |
| $Z$ | 0 | 0 |
| $P$ | 0 | 0 |
| $U$ | 0 | 0 |

| | $Q$ | $Y$ |
|---|---|---|
| $Q$ | $P$ | $U$ |
| $Y$ | $U$ | 0 |

| | $J$ | $Z$ | $P$ | $U$ |
|---|---|---|---|---|
| $J$ | $J$ | $Z$ | $P$ | $U$ |
| $Z$ | $Z$ | 0 | 0 | 0 |
| $P$ | $P$ | 0 | 0 | 0 |
| $U$ | $U$ | 0 | 0 | 0 |

| | $Q$ | $Y$ |
|---|---|---|
| $J$ | $Q$ | $Y$ |
| $Z$ | $Y$ | 0 |
| $P$ | $Y$ | 0 |
| $U$ | $Y$ | 0 |

| | $Q$ | $Y$ |
|---|---|---|
| $Q$ | $P$ | 0 |
| $Y$ | 0 | 0 |

| | $J$ | $Z$ | $P$ | $U$ |
|---|---|---|---|---|
| $J$ | $J$ | $Z$ | $P$ | $U$ |
| $Z$ | $Z$ | 0 | 0 | 0 |
| $P$ | $P$ | 0 | 0 | 0 |
| $U$ | $U$ | 0 | 0 | 0 |

| | $Q$ | $Y$ |
|---|---|---|
| $J$ | $Q$ | $Y$ |
| $Z$ | 0 | 0 |
| $P$ | 0 | 0 |
| $U$ | 0 | 0 |

| | $Q$ | $Y$ |
|---|---|---|
| $Q$ | $P$ | $U$ |
| $Y$ | $U$ | $P$ |

| | $J$ | $Z$ | $P$ | $U$ |
|---|---|---|---|---|
| $J$ | $J$ | $Z$ | $P$ | $U$ |
| $Z$ | $Z$ | 0 | 0 | 0 |
| $P$ | $P$ | 0 | 0 | 0 |
| $U$ | $U$ | 0 | 0 | 0 |

| | $Q$ | $Y$ |
|---|---|---|
| $J$ | $Q$ | $Y$ |
| $Z$ | 0 | 0 |
| $P$ | 0 | 0 |
| $U$ | 0 | 0 |

| | $Q$ | $Y$ |
|---|---|---|
| $Q$ | $P$ | 0 |
| $Y$ | 0 | $P$ |

| | $J$ | $Z$ | $P$ | $U$ |
|---|---|---|---|---|
| $J$ | $J$ | $Z$ | $P$ | $U$ |
| $Z$ | $Z$ | 0 | 0 | 0 |
| $P$ | $P$ | 0 | 0 | 0 |
| $U$ | $U$ | 0 | 0 | 0 |

| | $Q$ | $Y$ |
|---|---|---|
| $J$ | $Q$ | $Y$ |
| $Z$ | 0 | 0 |
| $P$ | 0 | 0 |
| $U$ | 0 | 0 |

| | $Q$ | $Y$ |
|---|---|---|
| $Q$ | $P$ | $U$ |
| $Y$ | $U$ | $U$ |

| | $J$ | $Z$ | $P$ | $U$ |
|---|---|---|---|---|
| $J$ | $J$ | $Z$ | $P$ | $U$ |
| $Z$ | $Z$ | 0 | 0 | 0 |
| $P$ | $P$ | 0 | 0 | 0 |
| $U$ | $U$ | 0 | 0 | 0 |

| | $Q$ | $Y$ |
|---|---|---|
| $J$ | $Q$ | $Y$ |
| $Z$ | 0 | 0 |
| $P$ | 0 | 0 |
| $U$ | 0 | 0 |

| | $Q$ | $Y$ |
|---|---|---|
| $Q$ | $P$ | 0 |
| $Y$ | 0 | $U$ |

| | $J$ | $Z$ | $P$ | $U$ |
|---|---|---|---|---|
| $J$ | $J$ | $Z$ | $P$ | $U$ |
| $Z$ | $Z$ | 0 | 0 | 0 |
| $P$ | $P$ | 0 | 0 | 0 |
| $U$ | $U$ | 0 | 0 | 0 |

| | $Q$ | $Y$ |
|---|---|---|
| $J$ | $Q$ | $Y$ |
| $Z$ | 0 | 0 |
| $P$ | 0 | 0 |
| $U$ | 0 | 0 |

| | $Q$ | $Y$ |
|---|---|---|
| $Q$ | $P$ | $U$ |
| $Y$ | $U$ | $Z$ |

| | $J$ | $Z$ | $P$ | $U$ |
|---|---|---|---|---|
| $J$ | $J$ | $Z$ | $P$ | $U$ |
| $Z$ | $Z$ | 0 | 0 | 0 |
| $P$ | $P$ | 0 | 0 | 0 |
| $U$ | $U$ | 0 | 0 | 0 |

| | $Q$ | $Y$ |
|---|---|---|
| $J$ | $Q$ | $Y$ |
| $Z$ | 0 | 0 |
| $P$ | 0 | 0 |
| $U$ | 0 | 0 |

| | $Q$ | $Y$ |
|---|---|---|
| $Q$ | $P$ | 0 |
| $Y$ | 0 | $Z$ |

| | $J$ | $Z$ | $P$ | $U$ |
|---|---|---|---|---|
| $J$ | $J$ | $Z$ | $P$ | $U$ |
| $Z$ | $Z$ | 0 | 0 | 0 |
| $P$ | $P$ | 0 | 0 | 0 |
| $U$ | $U$ | 0 | 0 | 0 |

| | $Q$ | $Y$ |
|---|---|---|
| $J$ | $Q$ | $Y$ |
| $Z$ | 0 | 0 |
| $P$ | 0 | 0 |
| $U$ | 0 | 0 |

| | $Q$ | $Y$ |
|---|---|---|
| $Q$ | $P$ | $U$ |
| $Y$ | $U$ | $P+Z$ |

| | $J$ | $Z$ | $P$ | $U$ |
|---|---|---|---|---|
| $J$ | $J$ | $Z$ | $P$ | $U$ |
| $Z$ | $Z$ | 0 | 0 | 0 |
| $P$ | $P$ | 0 | 0 | 0 |
| $U$ | $U$ | 0 | 0 | 0 |

| | $Q$ | $Y$ |
|---|---|---|
| $J$ | $Q$ | $Y$ |
| $Z$ | 0 | 0 |
| $P$ | 0 | 0 |
| $U$ | 0 | 0 |

| | $Q$ | $Y$ |
|---|---|---|
| $Q$ | $P$ | 0 |
| $Y$ | 0 | $P+Z$ |

| | $J$ | $Z$ | $P$ | $U$ |
|---|---|---|---|---|
| $J$ | $J$ | $Z$ | $P$ | $U$ |
| $Z$ | $Z$ | 0 | 0 | 0 |
| $P$ | $P$ | 0 | 0 | 0 |
| $U$ | $U$ | 0 | 0 | 0 |

| | $Q$ | $Y$ |
|---|---|---|
| $J$ | $Q$ | $Y$ |
| $Z$ | 0 | 0 |
| $P$ | 0 | 0 |
| $U$ | 0 | 0 |

| | $Q$ | $Y$ |
|---|---|---|
| $Q$ | $P$ | $U$ |
| $Y$ | $U$ | $U+Z$ |

| | $J$ | $Z$ | $P$ | $U$ |
|---|---|---|---|---|
| $J$ | $J$ | $Z$ | $P$ | $U$ |
| $Z$ | $Z$ | 0 | 0 | 0 |
| $P$ | $P$ | 0 | 0 | 0 |
| $U$ | $U$ | 0 | 0 | 0 |

| | $Q$ | $Y$ |
|---|---|---|
| $J$ | $Q$ | $Y$ |
| $Z$ | 0 | 0 |
| $P$ | 0 | 0 |
| $U$ | 0 | 0 |

| | $Q$ | $Y$ |
|---|---|---|
| $Q$ | $P$ | 0 |
| $Y$ | 0 | $U+Z$ |

| | $J$ | $Z$ | $P$ | $U$ |
|---|---|---|---|---|
| $J$ | $J$ | $Z$ | $P$ | $U$ |
| $Z$ | $Z$ | 0 | 0 | 0 |
| $P$ | $P$ | 0 | 0 | 0 |
| $U$ | $U$ | 0 | 0 | 0 |

| | $Q$ | $Y$ |
|---|---|---|
| $J$ | $Q$ | $Y$ |
| $Z$ | 0 | 0 |
| $P$ | 0 | 0 |
| $U$ | 0 | 0 |

| | $Q$ | $Y$ |
|---|---|---|
| $Q$ | $P$ | $Z$ |
| $Y$ | $Z$ | 0 |

| | $J$ | $Z$ | $P$ | $U$ |
|---|---|---|---|---|
| $J$ | $J$ | $Z$ | $P$ | $U$ |
| $Z$ | $Z$ | 0 | 0 | 0 |
| $P$ | $P$ | 0 | 0 | 0 |
| $U$ | $U$ | 0 | 0 | 0 |

| | $Q$ | $Y$ |
|---|---|---|
| $J$ | $Q$ | $Y$ |
| $Z$ | 0 | 0 |
| $P$ | 0 | 0 |
| $U$ | 0 | 0 |

| | $Q$ | $Y$ |
|---|---|---|
| $Q$ | $P$ | $P$ |
| $Y$ | $P$ | 0 |

| | $J$ | $Z$ | $P$ | $U$ |
|---|---|---|---|---|
| $J$ | $J$ | $Z$ | $P$ | $U$ |
| $Z$ | $Z$ | 0 | 0 | 0 |
| $P$ | $P$ | 0 | 0 | 0 |
| $U$ | $U$ | 0 | 0 | 0 |

| | $Q$ | $Y$ |
|---|---|---|
| $J$ | $Q$ | $Y$ |
| $Z$ | 0 | 0 |
| $P$ | 0 | 0 |
| $U$ | 0 | 0 |

| | $Q$ | $Y$ |
|---|---|---|
| $Q$ | $P$ | $Z$ |
| $Y$ | $Z$ | $P$ |

| | $J$ | $Z$ | $P$ | $U$ |
|---|---|---|---|---|
| $J$ | $J$ | $Z$ | $P$ | $U$ |
| $Z$ | $Z$ | 0 | 0 | 0 |
| $P$ | $P$ | 0 | 0 | 0 |
| $U$ | $U$ | 0 | 0 | 0 |

| | $Q$ | $Y$ |
|---|---|---|
| $J$ | $Q$ | $Y$ |
| $Z$ | 0 | 0 |
| $P$ | 0 | 0 |
| $U$ | 0 | 0 |

| | $Q$ | $Y$ |
|---|---|---|
| $Q$ | $P$ | $P$ |
| $Y$ | $P$ | $P$ |

| | $J$ | $Z$ | $P$ | $U$ |
|---|---|---|---|---|
| $J$ | $J$ | $Z$ | $P$ | $U$ |
| $Z$ | $Z$ | 0 | 0 | 0 |
| $P$ | $P$ | 0 | 0 | 0 |
| $U$ | $U$ | 0 | 0 | 0 |

| | $Q$ | $Y$ |
|---|---|---|
| $J$ | $Q$ | $Y$ |
| $Z$ | 0 | 0 |
| $P$ | 0 | 0 |
| $U$ | 0 | 0 |

| | $Q$ | $Y$ |
|---|---|---|
| $Q$ | $P$ | $Z$ |
| $Y$ | $Z$ | $U$ |

| | $J$ | $Z$ | $P$ | $U$ |
|---|---|---|---|---|
| $J$ | $J$ | $Z$ | $P$ | $U$ |
| $Z$ | $Z$ | 0 | 0 | 0 |
| $P$ | $P$ | 0 | 0 | 0 |
| $U$ | $U$ | 0 | 0 | 0 |

| | $Q$ | $Y$ |
|---|---|---|
| $J$ | $Q$ | $Y$ |
| $Z$ | 0 | 0 |
| $P$ | 0 | 0 |
| $U$ | 0 | 0 |

| | $Q$ | $Y$ |
|---|---|---|
| $Q$ | $P$ | $P$ |
| $Y$ | $P$ | $U$ |

| | $J$ | $Z$ | $P$ | $U$ |
|---|---|---|---|---|
| $J$ | $J$ | $Z$ | $P$ | $U$ |
| $Z$ | $Z$ | 0 | 0 | 0 |
| $P$ | $P$ | 0 | 0 | 0 |
| $U$ | $U$ | 0 | 0 | 0 |

| | $Q$ | $Y$ |
|---|---|---|
| $J$ | $Q$ | $Y$ |
| $Z$ | 0 | 0 |
| $P$ | 0 | 0 |
| $U$ | 0 | 0 |

| | $Q$ | $Y$ |
|---|---|---|
| $Q$ | $P$ | $Z$ |
| $Y$ | $Z$ | $Z$ |

| | $J$ | $Z$ | $P$ | $U$ |
|---|---|---|---|---|
| $J$ | $J$ | $Z$ | $P$ | $U$ |
| $Z$ | $Z$ | 0 | 0 | 0 |
| $P$ | $P$ | 0 | 0 | 0 |
| $U$ | $U$ | 0 | 0 | 0 |

| | $Q$ | $Y$ |
|---|---|---|
| $J$ | $Q$ | $Y$ |
| $Z$ | 0 | 0 |
| $P$ | 0 | 0 |
| $U$ | 0 | 0 |

| | $Q$ | $Y$ |
|---|---|---|
| $Q$ | $P$ | $P$ |
| $Y$ | $P$ | $Z$ |

| | $J$ | $Z$ | $P$ | $U$ |
|---|---|---|---|---|
| $J$ | $J$ | $Z$ | $P$ | $U$ |
| $Z$ | $Z$ | 0 | 0 | 0 |
| $P$ | $P$ | 0 | 0 | 0 |
| $U$ | $U$ | 0 | 0 | 0 |

| | $Q$ | $Y$ |
|---|---|---|
| $J$ | $Q$ | $Y$ |
| $Z$ | 0 | 0 |
| $P$ | 0 | 0 |
| $U$ | 0 | 0 |

| | $Q$ | $Y$ |
|---|---|---|
| $Q$ | $P$ | $Z$ |
| $Y$ | $Z$ | $P+Z$ |

| | $J$ | $Z$ | $P$ | $U$ |
|---|---|---|---|---|
| $J$ | $J$ | $Z$ | $P$ | $U$ |
| $Z$ | $Z$ | 0 | 0 | 0 |
| $P$ | $P$ | 0 | 0 | 0 |
| $U$ | $U$ | 0 | 0 | 0 |

| | $Q$ | $Y$ |
|---|---|---|
| $J$ | $Q$ | $Y$ |
| $Z$ | 0 | 0 |
| $P$ | 0 | 0 |
| $U$ | 0 | 0 |

| | $Q$ | $Y$ |
|---|---|---|
| $Q$ | $P$ | $P$ |
| $Y$ | $P$ | $P+Z$ |

| | $J$ | $Z$ | $P$ | $U$ |
|---|---|---|---|---|
| $J$ | $J$ | $Z$ | $P$ | $U$ |
| $Z$ | $Z$ | 0 | 0 | 0 |
| $P$ | $P$ | 0 | 0 | 0 |
| $U$ | $U$ | 0 | 0 | 0 |

| | $Q$ | $Y$ |
|---|---|---|
| $J$ | $Q$ | $Y$ |
| $Z$ | 0 | 0 |
| $P$ | 0 | 0 |
| $U$ | 0 | 0 |

| | $Q$ | $Y$ |
|---|---|---|
| $Q$ | $P$ | $Z$ |
| $Y$ | $Z$ | $U+Z$ |

| | $J$ | $Z$ | $P$ | $U$ |
|---|---|---|---|---|
| $J$ | $J$ | $Z$ | $P$ | $U$ |
| $Z$ | $Z$ | 0 | 0 | 0 |
| $P$ | $P$ | 0 | 0 | 0 |
| $U$ | $U$ | 0 | 0 | 0 |

| | $Q$ | $Y$ |
|---|---|---|
| $J$ | $Q$ | $Y$ |
| $Z$ | 0 | 0 |
| $P$ | 0 | 0 |
| $U$ | 0 | 0 |

| | $Q$ | $Y$ |
|---|---|---|
| $Q$ | $P$ | $P+Z$ |
| $Y$ | $P+Z$ | 0 |

| | $J$ | $Z$ | $P$ | $U$ |
|---|---|---|---|---|
| $J$ | $J$ | $Z$ | $P$ | $U$ |
| $Z$ | $Z$ | 0 | 0 | 0 |
| $P$ | $P$ | 0 | 0 | 0 |
| $U$ | $U$ | 0 | 0 | 0 |

| | $Q$ | $Y$ |
|---|---|---|
| $J$ | $Q$ | $Y$ |
| $Z$ | $Y$ | 0 |
| $P$ | 0 | 0 |
| $U$ | 0 | 0 |

| | $Q$ | $Y$ |
|---|---|---|
| $Q$ | $P+Z$ | 0 |
| $Y$ | 0 | 0 |

| | $J$ | $Z$ | $P$ | $U$ |
|---|---|---|---|---|
| $J$ | $J$ | $Z$ | $P$ | $U$ |
| $Z$ | $Z$ | 0 | 0 | 0 |
| $P$ | $P$ | 0 | 0 | 0 |
| $U$ | $U$ | 0 | 0 | 0 |

| | $Q$ | $Y$ |
|---|---|---|
| $J$ | $Q$ | $Y$ |
| $Z$ | 0 | 0 |
| $P$ | 0 | 0 |
| $U$ | 0 | 0 |

| | $Q$ | $Y$ |
|---|---|---|
| $Q$ | $P$ | $P+Z$ |
| $Y$ | $P+Z$ | $P$ |

| | $J$ | $Z$ | $P$ | $U$ |
|---|---|---|---|---|
| $J$ | $J$ | $Z$ | $P$ | $U$ |
| $Z$ | $Z$ | 0 | 0 | 0 |
| $P$ | $P$ | 0 | 0 | 0 |
| $U$ | $U$ | 0 | 0 | 0 |

| | $Q$ | $Y$ |
|---|---|---|
| $J$ | $Q$ | $Y$ |
| $Z$ | 0 | 0 |
| $P$ | 0 | 0 |
| $U$ | $Y$ | 0 |

| | $Q$ | $Y$ |
|---|---|---|
| $Q$ | $P+Z$ | 0 |
| $Y$ | 0 | 0 |

| | $J$ | $Z$ | $P$ | $U$ |
|---|---|---|---|---|
| $J$ | $J$ | $Z$ | $P$ | $U$ |
| $Z$ | $Z$ | 0 | 0 | 0 |
| $P$ | $P$ | 0 | 0 | 0 |
| $U$ | $U$ | 0 | 0 | 0 |

| | $Q$ | $Y$ |
|---|---|---|
| $J$ | $Q$ | $Y$ |
| $Z$ | 0 | 0 |
| $P$ | 0 | 0 |
| $U$ | 0 | 0 |

| | $Q$ | $Y$ |
|---|---|---|
| $Q$ | $P$ | $P+Z$ |
| $Y$ | $P+Z$ | $U$ |

| | $J$ | $Z$ | $P$ | $U$ |
|---|---|---|---|---|
| $J$ | $J$ | $Z$ | $P$ | $U$ |
| $Z$ | $Z$ | 0 | 0 | 0 |
| $P$ | $P$ | 0 | 0 | 0 |
| $U$ | $U$ | 0 | 0 | 0 |

| | $Q$ | $Y$ |
|---|---|---|
| $J$ | $Q$ | $Y$ |
| $Z$ | $Y$ | 0 |
| $P$ | 0 | 0 |
| $U$ | $Y$ | 0 |

| | $Q$ | $Y$ |
|---|---|---|
| $Q$ | $P+Z$ | 0 |
| $Y$ | 0 | 0 |

| | $J$ | $Z$ | $P$ | $U$ |
|---|---|---|---|---|
| $J$ | $J$ | $Z$ | $P$ | $U$ |
| $Z$ | $Z$ | 0 | 0 | 0 |
| $P$ | $P$ | 0 | 0 | 0 |
| $U$ | $U$ | 0 | 0 | 0 |

| | $Q$ | $Y$ |
|---|---|---|
| $J$ | $Q$ | $Y$ |
| $Z$ | 0 | 0 |
| $P$ | 0 | 0 |
| $U$ | 0 | 0 |

| | $Q$ | $Y$ |
|---|---|---|
| $Q$ | $P$ | $P+Z$ |
| $Y$ | $P+Z$ | $Z$ |

| | $J$ | $Z$ | $P$ | $U$ |
|---|---|---|---|---|
| $J$ | $J$ | $Z$ | $P$ | $U$ |
| $Z$ | $Z$ | 0 | 0 | 0 |
| $P$ | $P$ | 0 | 0 | 0 |
| $U$ | $U$ | 0 | 0 | 0 |

| | $Q$ | $Y$ |
|---|---|---|
| $J$ | $Q$ | $Y$ |
| $Z$ | 0 | 0 |
| $P$ | $Y$ | 0 |
| $U$ | 0 | 0 |

| | $Q$ | $Y$ |
|---|---|---|
| $Q$ | $P+Z$ | 0 |
| $Y$ | 0 | 0 |

| | $J$ | $Z$ | $P$ | $U$ |
|---|---|---|---|---|
| $J$ | $J$ | $Z$ | $P$ | $U$ |
| $Z$ | $Z$ | 0 | 0 | 0 |
| $P$ | $P$ | 0 | 0 | 0 |
| $U$ | $U$ | 0 | 0 | 0 |

| | $Q$ | $Y$ |
|---|---|---|
| $J$ | $Q$ | $Y$ |
| $Z$ | 0 | 0 |
| $P$ | 0 | 0 |
| $U$ | 0 | 0 |

| | $Q$ | $Y$ |
|---|---|---|
| $Q$ | $P$ | $P+Z$ |
| $Y$ | $P+Z$ | $P+Z$ |

| | $J$ | $Z$ | $P$ | $U$ |
|---|---|---|---|---|
| $J$ | $J$ | $Z$ | $P$ | $U$ |
| $Z$ | $Z$ | 0 | 0 | 0 |
| $P$ | $P$ | 0 | 0 | 0 |
| $U$ | $U$ | 0 | 0 | 0 |

| | $Q$ | $Y$ |
|---|---|---|
| $J$ | $Q$ | $Y$ |
| $Z$ | $Y$ | 0 |
| $P$ | $Y$ | 0 |
| $U$ | 0 | 0 |

| | $Q$ | $Y$ |
|---|---|---|
| $Q$ | $P+Z$ | 0 |
| $Y$ | 0 | 0 |

| | $J$ | $Z$ | $P$ | $U$ |
|---|---|---|---|---|
| $J$ | $J$ | $Z$ | $P$ | $U$ |
| $Z$ | $Z$ | 0 | 0 | 0 |
| $P$ | $P$ | 0 | 0 | 0 |
| $U$ | $U$ | 0 | 0 | 0 |

| | $Q$ | $Y$ |
|---|---|---|
| $J$ | $Q$ | $Y$ |
| $Z$ | 0 | 0 |
| $P$ | 0 | 0 |
| $U$ | 0 | 0 |

| | $Q$ | $Y$ |
|---|---|---|
| $Q$ | $P$ | $P+Z$ |
| $Y$ | $P+Z$ | $U+Z$ |

| | $J$ | $Z$ | $P$ | $U$ |
|---|---|---|---|---|
| $J$ | $J$ | $Z$ | $P$ | $U$ |
| $Z$ | $Z$ | 0 | 0 | 0 |
| $P$ | $P$ | 0 | 0 | 0 |
| $U$ | $U$ | 0 | 0 | 0 |

| | $Q$ | $Y$ |
|---|---|---|
| $J$ | $Q$ | $Y$ |
| $Z$ | 0 | 0 |
| $P$ | $Y$ | 0 |
| $U$ | $Y$ | 0 |

| | $Q$ | $Y$ |
|---|---|---|
| $Q$ | $P+Z$ | 0 |
| $Y$ | 0 | 0 |

| | $J$ | $Z$ | $P$ | $U$ |
|---|---|---|---|---|
| $J$ | $J$ | $Z$ | $P$ | $U$ |
| $Z$ | $Z$ | 0 | 0 | 0 |
| $P$ | $P$ | 0 | 0 | 0 |
| $U$ | $U$ | 0 | 0 | 0 |

| | $Q$ | $Y$ |
|---|---|---|
| $J$ | $Q$ | $Y$ |
| $Z$ | 0 | 0 |
| $P$ | 0 | 0 |
| $U$ | 0 | 0 |

| | $Q$ | $Y$ |
|---|---|---|
| $Q$ | $P$ | $U+Z$ |
| $Y$ | $U+Z$ | 0 |

| | $J$ | $Z$ | $P$ | $U$ |
|---|---|---|---|---|
| $J$ | $J$ | $Z$ | $P$ | $U$ |
| $Z$ | $Z$ | 0 | 0 | 0 |
| $P$ | $P$ | 0 | 0 | 0 |
| $U$ | $U$ | 0 | 0 | 0 |

| | $Q$ | $Y$ |
|---|---|---|
| $J$ | $Q$ | $Y$ |
| $Z$ | $Y$ | 0 |
| $P$ | $Y$ | 0 |
| $U$ | $Y$ | 0 |

| | $Q$ | $Y$ |
|---|---|---|
| $Q$ | $P+Z$ | 0 |
| $Y$ | 0 | 0 |

| | $J$ | $Z$ | $P$ | $U$ |
|---|---|---|---|---|
| $J$ | $J$ | $Z$ | $P$ | $U$ |
| $Z$ | $Z$ | 0 | 0 | 0 |
| $P$ | $P$ | 0 | 0 | 0 |
| $U$ | $U$ | 0 | 0 | 0 |

| | $Q$ | $Y$ |
|---|---|---|
| $J$ | $Q$ | $Y$ |
| $Z$ | 0 | 0 |
| $P$ | 0 | 0 |
| $U$ | 0 | 0 |

| | $Q$ | $Y$ |
|---|---|---|
| $Q$ | $P$ | $U+Z$ |
| $Y$ | $U+Z$ | $P$ |

| | $J$ | $Z$ | $P$ | $U$ |
|---|---|---|---|---|
| $J$ | $J$ | $Z$ | $P$ | $U$ |
| $Z$ | $Z$ | 0 | 0 | 0 |
| $P$ | $P$ | 0 | 0 | 0 |
| $U$ | $U$ | 0 | 0 | 0 |

| | $Q$ | $Y$ |
|---|---|---|
| $J$ | $Q$ | $Y$ |
| $Z$ | 0 | 0 |
| $P$ | 0 | 0 |
| $U$ | 0 | 0 |

| | $Q$ | $Y$ |
|---|---|---|
| $Q$ | $P+Z$ | 0 |
| $Y$ | 0 | $P$ |

| | $J$ | $Z$ | $P$ | $U$ |
|---|---|---|---|---|
| $J$ | $J$ | $Z$ | $P$ | $U$ |
| $Z$ | $Z$ | 0 | 0 | 0 |
| $P$ | $P$ | 0 | 0 | 0 |
| $U$ | $U$ | 0 | 0 | 0 |

| | $Q$ | $Y$ |
|---|---|---|
| $J$ | $Q$ | $Y$ |
| $Z$ | 0 | 0 |
| $P$ | 0 | 0 |
| $U$ | 0 | 0 |

| | $Q$ | $Y$ |
|---|---|---|
| $Q$ | $P$ | $U+Z$ |
| $Y$ | $U+Z$ | $U$ |

| | $J$ | $Z$ | $P$ | $U$ |
|---|---|---|---|---|
| $J$ | $J$ | $Z$ | $P$ | $U$ |
| $Z$ | $Z$ | 0 | 0 | 0 |
| $P$ | $P$ | 0 | 0 | 0 |
| $U$ | $U$ | 0 | 0 | 0 |

| | $Q$ | $Y$ |
|---|---|---|
| $J$ | $Q$ | $Y$ |
| $Z$ | 0 | 0 |
| $P$ | 0 | 0 |
| $U$ | 0 | 0 |

| | $Q$ | $Y$ |
|---|---|---|
| $Q$ | $P+Z$ | 0 |
| $Y$ | 0 | $U$ |

| | $J$ | $Z$ | $P$ | $U$ |
|---|---|---|---|---|
| $J$ | $J$ | $Z$ | $P$ | $U$ |
| $Z$ | $Z$ | 0 | 0 | 0 |
| $P$ | $P$ | 0 | 0 | 0 |
| $U$ | $U$ | 0 | 0 | 0 |

| | $Q$ | $Y$ |
|---|---|---|
| $J$ | $Q$ | $Y$ |
| $Z$ | 0 | 0 |
| $P$ | 0 | 0 |
| $U$ | 0 | 0 |

| | $Q$ | $Y$ |
|---|---|---|
| $Q$ | $P$ | $U+Z$ |
| $Y$ | $U+Z$ | $Z$ |

| | $J$ | $Z$ | $P$ | $U$ |
|---|---|---|---|---|
| $J$ | $J$ | $Z$ | $P$ | $U$ |
| $Z$ | $Z$ | 0 | 0 | 0 |
| $P$ | $P$ | 0 | 0 | 0 |
| $U$ | $U$ | 0 | 0 | 0 |

| | $Q$ | $Y$ |
|---|---|---|
| $J$ | $Q$ | $Y$ |
| $Z$ | 0 | 0 |
| $P$ | 0 | 0 |
| $U$ | 0 | 0 |

| | $Q$ | $Y$ |
|---|---|---|
| $Q$ | $P+Z$ | 0 |
| $Y$ | 0 | $Z$ |

| | $J$ | $Z$ | $P$ | $U$ |
|---|---|---|---|---|
| $J$ | $J$ | $Z$ | $P$ | $U$ |
| $Z$ | $Z$ | 0 | 0 | 0 |
| $P$ | $P$ | 0 | 0 | 0 |
| $U$ | $U$ | 0 | 0 | 0 |

| | $Q$ | $Y$ |
|---|---|---|
| $J$ | $Q$ | $Y$ |
| $Z$ | 0 | 0 |
| $P$ | 0 | 0 |
| $U$ | 0 | 0 |

| | $Q$ | $Y$ |
|---|---|---|
| $Q$ | $P$ | $U+Z$ |
| $Y$ | $U+Z$ | $P+Z$ |

| | $J$ | $Z$ | $P$ | $U$ |
|---|---|---|---|---|
| $J$ | $J$ | $Z$ | $P$ | $U$ |
| $Z$ | $Z$ | 0 | 0 | 0 |
| $P$ | $P$ | 0 | 0 | 0 |
| $U$ | $U$ | 0 | 0 | 0 |

| | $Q$ | $Y$ |
|---|---|---|
| $J$ | $Q$ | $Y$ |
| $Z$ | 0 | 0 |
| $P$ | 0 | 0 |
| $U$ | 0 | 0 |

| | $Q$ | $Y$ |
|---|---|---|
| $Q$ | $P+Z$ | 0 |
| $Y$ | 0 | $P+Z$ |

| | $J$ | $Z$ | $P$ | $U$ |
|---|---|---|---|---|
| $J$ | $J$ | $Z$ | $P$ | $U$ |
| $Z$ | $Z$ | 0 | 0 | 0 |
| $P$ | $P$ | 0 | 0 | 0 |
| $U$ | $U$ | 0 | 0 | 0 |

| | $Q$ | $Y$ |
|---|---|---|
| $J$ | $Q$ | $Y$ |
| $Z$ | 0 | 0 |
| $P$ | 0 | 0 |
| $U$ | 0 | 0 |

| | $Q$ | $Y$ |
|---|---|---|
| $Q$ | $P$ | $U+Z$ |
| $Y$ | $U+Z$ | $U+Z$ |

| | $J$ | $Z$ | $P$ | $U$ |
|---|---|---|---|---|
| $J$ | $J$ | $Z$ | $P$ | $U$ |
| $Z$ | $Z$ | 0 | 0 | 0 |
| $P$ | $P$ | 0 | 0 | 0 |
| $U$ | $U$ | 0 | 0 | 0 |

| | $Q$ | $Y$ |
|---|---|---|
| $J$ | $Q$ | $Y$ |
| $Z$ | 0 | 0 |
| $P$ | 0 | 0 |
| $U$ | 0 | 0 |

| | $Q$ | $Y$ |
|---|---|---|
| $Q$ | $P+Z$ | 0 |
| $Y$ | 0 | $U+Z$ |

| | $J$ | $Z$ | $P$ | $U$ |
|---|---|---|---|---|
| $J$ | $J$ | $Z$ | $P$ | $U$ |
| $Z$ | $Z$ | 0 | 0 | 0 |
| $P$ | $P$ | 0 | 0 | 0 |
| $U$ | $U$ | 0 | 0 | 0 |

| | $Q$ | $Y$ |
|---|---|---|
| $J$ | $Q$ | $Y$ |
| $Z$ | 0 | 0 |
| $P$ | 0 | 0 |
| $U$ | 0 | 0 |

| | $Q$ | $Y$ |
|---|---|---|
| $Q$ | $P+Z$ | 0 |
| $Y$ | 0 | 0 |

| | $J$ | $Z$ | $P$ | $U$ |
|---|---|---|---|---|
| $J$ | $J$ | $Z$ | $P$ | $U$ |
| $Z$ | $Z$ | 0 | 0 | 0 |
| $P$ | $P$ | 0 | 0 | 0 |
| $U$ | $U$ | 0 | 0 | 0 |

| | $Q$ | $Y$ |
|---|---|---|
| $J$ | $Q$ | $Y$ |
| $Z$ | 0 | 0 |
| $P$ | 0 | 0 |
| $U$ | 0 | 0 |

| | $Q$ | $Y$ |
|---|---|---|
| $Q$ | $P+Z$ | $P$ |
| $Y$ | $P$ | 0 |

| | $J$ | $Z$ | $P$ | $U$ |
|---|---|---|---|---|
| $J$ | $J$ | $Z$ | $P$ | $U$ |
| $Z$ | $Z$ | 0 | 0 | 0 |
| $P$ | $P$ | 0 | 0 | 0 |
| $U$ | $U$ | 0 | 0 | 0 |

| | $Q$ | $Y$ |
|---|---|---|
| $J$ | $Q$ | $Y$ |
| $Z$ | 0 | 0 |
| $P$ | 0 | 0 |
| $U$ | 0 | 0 |

| | $Q$ | $Y$ |
|---|---|---|
| $Q$ | $P+Z$ | $P$ |
| $Y$ | $P$ | $P$ |

| | $J$ | $Z$ | $P$ | $U$ |
|---|---|---|---|---|
| $J$ | $J$ | $Z$ | $P$ | $U$ |
| $Z$ | $Z$ | 0 | 0 | 0 |
| $P$ | $P$ | 0 | 0 | 0 |
| $U$ | $U$ | 0 | 0 | 0 |

| | $Q$ | $Y$ |
|---|---|---|
| $J$ | $Q$ | $Y$ |
| $Z$ | 0 | 0 |
| $P$ | 0 | 0 |
| $U$ | 0 | 0 |

| | $Q$ | $Y$ |
|---|---|---|
| $Q$ | $P+Z$ | $Z$ |
| $Y$ | $Z$ | $U$ |

| | $J$ | $Z$ | $P$ | $U$ |
|---|---|---|---|---|
| $J$ | $J$ | $Z$ | $P$ | $U$ |
| $Z$ | $Z$ | 0 | 0 | 0 |
| $P$ | $P$ | 0 | 0 | 0 |
| $U$ | $U$ | 0 | 0 | 0 |

| | $Q$ | $Y$ |
|---|---|---|
| $J$ | $Q$ | $Y$ |
| $Z$ | 0 | 0 |
| $P$ | 0 | 0 |
| $U$ | 0 | 0 |

| | $Q$ | $Y$ |
|---|---|---|
| $Q$ | $P+Z$ | $P$ |
| $Y$ | $P$ | $U$ |

| | $J$ | $Z$ | $P$ | $U$ |
|---|---|---|---|---|
| $J$ | $J$ | $Z$ | $P$ | $U$ |
| $Z$ | $Z$ | 0 | 0 | 0 |
| $P$ | $P$ | 0 | 0 | 0 |
| $U$ | $U$ | 0 | 0 | 0 |

| | $Q$ | $Y$ |
|---|---|---|
| $J$ | $Q$ | $Y$ |
| $Z$ | 0 | 0 |
| $P$ | 0 | 0 |
| $U$ | 0 | 0 |

| | $Q$ | $Y$ |
|---|---|---|
| $Q$ | $P+Z$ | $Z$ |
| $Y$ | $Z$ | $Z$ |

| | $J$ | $Z$ | $P$ | $U$ |
|---|---|---|---|---|
| $J$ | $J$ | $Z$ | $P$ | $U$ |
| $Z$ | $Z$ | 0 | 0 | 0 |
| $P$ | $P$ | 0 | 0 | 0 |
| $U$ | $U$ | 0 | 0 | 0 |

| | $Q$ | $Y$ |
|---|---|---|
| $J$ | $Q$ | $Y$ |
| $Z$ | 0 | 0 |
| $P$ | 0 | 0 |
| $U$ | 0 | 0 |

| | $Q$ | $Y$ |
|---|---|---|
| $Q$ | $P+Z$ | $P$ |
| $Y$ | $P$ | $Z$ |

| | $J$ | $Z$ | $P$ | $U$ |
|---|---|---|---|---|
| $J$ | $J$ | $Z$ | $P$ | $U$ |
| $Z$ | $Z$ | 0 | 0 | 0 |
| $P$ | $P$ | 0 | 0 | 0 |
| $U$ | $U$ | 0 | 0 | 0 |

| | $Q$ | $Y$ |
|---|---|---|
| $J$ | $Q$ | $Y$ |
| $Z$ | 0 | 0 |
| $P$ | 0 | 0 |
| $U$ | 0 | 0 |

| | $Q$ | $Y$ |
|---|---|---|
| $Q$ | $P+Z$ | $Z$ |
| $Y$ | $Z$ | $P+Z$ |

| | $J$ | $Z$ | $P$ | $U$ |
|---|---|---|---|---|
| $J$ | $J$ | $Z$ | $P$ | $U$ |
| $Z$ | $Z$ | 0 | 0 | 0 |
| $P$ | $P$ | 0 | 0 | 0 |
| $U$ | $U$ | 0 | 0 | 0 |

| | $Q$ | $Y$ |
|---|---|---|
| $J$ | $Q$ | $Y$ |
| $Z$ | 0 | 0 |
| $P$ | 0 | 0 |
| $U$ | 0 | 0 |

| | $Q$ | $Y$ |
|---|---|---|
| $Q$ | $P+Z$ | $P$ |
| $Y$ | $P$ | $P+Z$ |

| | $J$ | $Z$ | $P$ | $U$ |
|---|---|---|---|---|
| $J$ | $J$ | $Z$ | $P$ | $U$ |
| $Z$ | $Z$ | 0 | 0 | 0 |
| $P$ | $P$ | 0 | 0 | 0 |
| $U$ | $U$ | 0 | 0 | 0 |

| | $Q$ | $Y$ |
|---|---|---|
| $J$ | $Q$ | $Y$ |
| $Z$ | 0 | 0 |
| $P$ | 0 | 0 |
| $U$ | 0 | 0 |

| | $Q$ | $Y$ |
|---|---|---|
| $Q$ | $P+Z$ | $Z$ |
| $Y$ | $Z$ | $U+Z$ |

| | $J$ | $Z$ | $P$ | $U$ |
|---|---|---|---|---|
| $J$ | $J$ | $Z$ | $P$ | $U$ |
| $Z$ | $Z$ | 0 | 0 | 0 |
| $P$ | $P$ | 0 | 0 | 0 |
| $U$ | $U$ | 0 | 0 | 0 |

| | $Q$ | $Y$ |
|---|---|---|
| $J$ | $Q$ | $Y$ |
| $Z$ | 0 | 0 |
| $P$ | 0 | 0 |
| $U$ | 0 | 0 |

| | $Q$ | $Y$ |
|---|---|---|
| $Q$ | $P+Z$ | $P$ |
| $Y$ | $P$ | $U+Z$ |

| | $J$ | $Z$ | $P$ | $U$ |
|---|---|---|---|---|
| $J$ | $J$ | $Z$ | $P$ | $U$ |
| $Z$ | $Z$ | 0 | 0 | 0 |
| $P$ | $P$ | 0 | 0 | 0 |
| $U$ | $U$ | 0 | 0 | 0 |

| | $Q$ | $Y$ |
|---|---|---|
| $J$ | $Q$ | $Y$ |
| $Z$ | 0 | 0 |
| $P$ | 0 | 0 |
| $U$ | 0 | 0 |

| | $Q$ | $Y$ |
|---|---|---|
| $Q$ | $P+Z$ | $P+Z$ |
| $Y$ | $P+Z$ | 0 |

| | $J$ | $Z$ | $P$ | $U$ |
|---|---|---|---|---|
| $J$ | $J$ | $Z$ | $P$ | $U$ |
| $Z$ | $Z$ | 0 | 0 | 0 |
| $P$ | $P$ | 0 | 0 | 0 |
| $U$ | $U$ | 0 | 0 | 0 |

| | $Q$ | $Y$ |
|---|---|---|
| $J$ | $Q$ | $Y$ |
| $Z$ | 0 | 0 |
| $P$ | 0 | 0 |
| $U$ | 0 | 0 |

| | $Q$ | $Y$ |
|---|---|---|
| $Q$ | $P+Z$ | $U$ |
| $Y$ | $U$ | 0 |

| | $J$ | $Z$ | $P$ | $U$ |
|---|---|---|---|---|
| $J$ | $J$ | $Z$ | $P$ | $U$ |
| $Z$ | $Z$ | 0 | 0 | 0 |
| $P$ | $P$ | 0 | 0 | 0 |
| $U$ | $U$ | 0 | 0 | 0 |

| | $Q$ | $Y$ |
|---|---|---|
| $J$ | $Q$ | $Y$ |
| $Z$ | 0 | 0 |
| $P$ | 0 | 0 |
| $U$ | 0 | 0 |

| | $Q$ | $Y$ |
|---|---|---|
| $Q$ | $P+Z$ | $P+Z$ |
| $Y$ | $P+Z$ | $P$ |

| | $J$ | $Z$ | $P$ | $U$ |
|---|---|---|---|---|
| $J$ | $J$ | $Z$ | $P$ | $U$ |
| $Z$ | $Z$ | 0 | 0 | 0 |
| $P$ | $P$ | 0 | 0 | 0 |
| $U$ | $U$ | 0 | 0 | 0 |

| | $Q$ | $Y$ |
|---|---|---|
| $J$ | $Q$ | $Y$ |
| $Z$ | 0 | 0 |
| $P$ | 0 | 0 |
| $U$ | 0 | 0 |

| | $Q$ | $Y$ |
|---|---|---|
| $Q$ | $P+Z$ | $U$ |
| $Y$ | $U$ | $P$ |

| | $J$ | $Z$ | $P$ | $U$ |
|---|---|---|---|---|
| $J$ | $J$ | $Z$ | $P$ | $U$ |
| $Z$ | $Z$ | 0 | 0 | 0 |
| $P$ | $P$ | 0 | 0 | 0 |
| $U$ | $U$ | 0 | 0 | 0 |

| | $Q$ | $Y$ |
|---|---|---|
| $J$ | $Q$ | $Y$ |
| $Z$ | 0 | 0 |
| $P$ | 0 | 0 |
| $U$ | 0 | 0 |

| | $Q$ | $Y$ |
|---|---|---|
| $Q$ | $P+Z$ | $P+Z$ |
| $Y$ | $P+Z$ | $U$ |

| | $J$ | $Z$ | $P$ | $U$ |
|---|---|---|---|---|
| $J$ | $J$ | $Z$ | $P$ | $U$ |
| $Z$ | $Z$ | 0 | 0 | 0 |
| $P$ | $P$ | 0 | 0 | 0 |
| $U$ | $U$ | 0 | 0 | 0 |

| | $Q$ | $Y$ |
|---|---|---|
| $J$ | $Q$ | $Y$ |
| $Z$ | 0 | 0 |
| $P$ | 0 | 0 |
| $U$ | 0 | 0 |

| | $Q$ | $Y$ |
|---|---|---|
| $Q$ | $P+Z$ | $U$ |
| $Y$ | $U$ | $U$ |

| | $J$ | $Z$ | $P$ | $U$ |
|---|---|---|---|---|
| $J$ | $J$ | $Z$ | $P$ | $U$ |
| $Z$ | $Z$ | 0 | 0 | 0 |
| $P$ | $P$ | 0 | 0 | 0 |
| $U$ | $U$ | 0 | 0 | 0 |

| | $Q$ | $Y$ |
|---|---|---|
| $J$ | $Q$ | $Y$ |
| $Z$ | 0 | 0 |
| $P$ | 0 | 0 |
| $U$ | 0 | 0 |

| | $Q$ | $Y$ |
|---|---|---|
| $Q$ | $P+Z$ | $P+Z$ |
| $Y$ | $P+Z$ | $Z$ |

| | $J$ | $Z$ | $P$ | $U$ |
|---|---|---|---|---|
| $J$ | $J$ | $Z$ | $P$ | $U$ |
| $Z$ | $Z$ | 0 | 0 | 0 |
| $P$ | $P$ | 0 | 0 | 0 |
| $U$ | $U$ | 0 | 0 | 0 |

| | $Q$ | $Y$ |
|---|---|---|
| $J$ | $Q$ | $Y$ |
| $Z$ | 0 | 0 |
| $P$ | 0 | 0 |
| $U$ | 0 | 0 |

| | $Q$ | $Y$ |
|---|---|---|
| $Q$ | $P+Z$ | $U$ |
| $Y$ | $U$ | $Z$ |

| | $J$ | $Z$ | $P$ | $U$ |
|---|---|---|---|---|
| $J$ | $J$ | $Z$ | $P$ | $U$ |
| $Z$ | $Z$ | 0 | 0 | 0 |
| $P$ | $P$ | 0 | 0 | 0 |
| $U$ | $U$ | 0 | 0 | 0 |

| | $Q$ | $Y$ |
|---|---|---|
| $J$ | $Q$ | $Y$ |
| $Z$ | 0 | 0 |
| $P$ | 0 | 0 |
| $U$ | 0 | 0 |

| | $Q$ | $Y$ |
|---|---|---|
| $Q$ | $P+Z$ | $P+Z$ |
| $Y$ | $P+Z$ | $P+Z$ |

| | $J$ | $Z$ | $P$ | $U$ |
|---|---|---|---|---|
| $J$ | $J$ | $Z$ | $P$ | $U$ |
| $Z$ | $Z$ | 0 | 0 | 0 |
| $P$ | $P$ | 0 | 0 | 0 |
| $U$ | $U$ | 0 | 0 | 0 |

| | $Q$ | $Y$ |
|---|---|---|
| $J$ | $Q$ | $Y$ |
| $Z$ | 0 | 0 |
| $P$ | 0 | 0 |
| $U$ | 0 | 0 |

| | $Q$ | $Y$ |
|---|---|---|
| $Q$ | $P+Z$ | $U$ |
| $Y$ | $U$ | $P+Z$ |

| | $J$ | $Z$ | $P$ | $U$ |
|---|---|---|---|---|
| $J$ | $J$ | $Z$ | $P$ | $U$ |
| $Z$ | $Z$ | 0 | 0 | 0 |
| $P$ | $P$ | 0 | 0 | 0 |
| $U$ | $U$ | 0 | 0 | 0 |

| | $Q$ | $Y$ |
|---|---|---|
| $J$ | $Q$ | $Y$ |
| $Z$ | 0 | 0 |
| $P$ | 0 | 0 |
| $U$ | 0 | 0 |

| | $Q$ | $Y$ |
|---|---|---|
| $Q$ | $P+Z$ | $P+Z$ |
| $Y$ | $P+Z$ | $U+Z$ |

| | $J$ | $Z$ | $P$ | $U$ |
|---|---|---|---|---|
| $J$ | $J$ | $Z$ | $P$ | $U$ |
| $Z$ | $Z$ | 0 | 0 | 0 |
| $P$ | $P$ | 0 | 0 | 0 |
| $U$ | $U$ | 0 | 0 | 0 |

| | $Q$ | $Y$ |
|---|---|---|
| $J$ | $Q$ | $Y$ |
| $Z$ | 0 | 0 |
| $P$ | 0 | 0 |
| $U$ | 0 | 0 |

| | $Q$ | $Y$ |
|---|---|---|
| $Q$ | $P+Z$ | $U$ |
| $Y$ | $U$ | $U+Z$ |

| | $J$ | $Z$ | $P$ | $U$ |
|---|---|---|---|---|
| $J$ | $J$ | $Z$ | $P$ | $U$ |
| $Z$ | $Z$ | 0 | 0 | 0 |
| $P$ | $P$ | 0 | 0 | 0 |
| $U$ | $U$ | 0 | 0 | 0 |

| | $Q$ | $Y$ |
|---|---|---|
| $J$ | $Q$ | $Y$ |
| $Z$ | 0 | 0 |
| $P$ | 0 | 0 |
| $U$ | 0 | 0 |

| | $Q$ | $Y$ |
|---|---|---|
| $Q$ | $P+Z$ | $U+Z$ |
| $Y$ | $U+Z$ | 0 |

| | $J$ | $Z$ | $P$ | $U$ |
|---|---|---|---|---|
| $J$ | $J$ | $Z$ | $P$ | $U$ |
| $Z$ | $Z$ | 0 | 0 | 0 |
| $P$ | $P$ | 0 | 0 | 0 |
| $U$ | $U$ | 0 | 0 | 0 |

| | $Q$ | $Y$ |
|---|---|---|
| $J$ | $Q$ | $Y$ |
| $Z$ | 0 | 0 |
| $P$ | 0 | 0 |
| $U$ | 0 | 0 |

| | $Q$ | $Y$ |
|---|---|---|
| $Q$ | $P+Z$ | $Z$ |
| $Y$ | $Z$ | 0 |

| | $J$ | $Z$ | $P$ | $U$ |
|---|---|---|---|---|
| $J$ | $J$ | $Z$ | $P$ | $U$ |
| $Z$ | $Z$ | 0 | 0 | 0 |
| $P$ | $P$ | 0 | 0 | 0 |
| $U$ | $U$ | 0 | 0 | 0 |

| | $Q$ | $Y$ |
|---|---|---|
| $J$ | $Q$ | $Y$ |
| $Z$ | 0 | 0 |
| $P$ | 0 | 0 |
| $U$ | 0 | 0 |

| | $Q$ | $Y$ |
|---|---|---|
| $Q$ | $P+Z$ | $U+Z$ |
| $Y$ | $U+Z$ | $P$ |

| | $J$ | $Z$ | $P$ | $U$ |
|---|---|---|---|---|
| $J$ | $J$ | $Z$ | $P$ | $U$ |
| $Z$ | $Z$ | 0 | 0 | 0 |
| $P$ | $P$ | 0 | 0 | 0 |
| $U$ | $U$ | 0 | 0 | 0 |

| | $Q$ | $Y$ |
|---|---|---|
| $J$ | $Q$ | $Y$ |
| $Z$ | 0 | 0 |
| $P$ | 0 | 0 |
| $U$ | 0 | 0 |

| | $Q$ | $Y$ |
|---|---|---|
| $Q$ | $P+Z$ | $Z$ |
| $Y$ | $Z$ | $P$ |

| | $J$ | $Z$ | $P$ | $U$ |
|---|---|---|---|---|
| $J$ | $J$ | $Z$ | $P$ | $U$ |
| $Z$ | $Z$ | 0 | 0 | 0 |
| $P$ | $P$ | 0 | 0 | 0 |
| $U$ | $U$ | 0 | 0 | 0 |

| | $Q$ | $Y$ |
|---|---|---|
| $J$ | $Q$ | $Y$ |
| $Z$ | 0 | 0 |
| $P$ | 0 | 0 |
| $U$ | 0 | 0 |

| | $Q$ | $Y$ |
|---|---|---|
| $Q$ | $P+Z$ | $U+Z$ |
| $Y$ | $U+Z$ | $U$ |

| | J | Z | P | U |
|---|---|---|---|---|
| J | J | Z | P | U |
| Z | Z | 0 | 0 | 0 |
| P | P | 0 | 0 | 0 |
| U | U | 0 | 0 | 0 |

| | Q | Y |
|---|---|---|
| J | Q | Y |
| Z | 0 | 0 |
| P | 0 | 0 |
| U | 0 | 0 |

| | Q | Y |
|---|---|---|
| Q | P + Z | U + Z |
| Y | U + Z | Z |

| | J | Z | P | U |
|---|---|---|---|---|
| J | J | Z | P | U |
| Z | Z | 0 | 0 | 0 |
| P | P | 0 | 0 | 0 |
| U | U | 0 | 0 | Z |

| | Q | Y |
|---|---|---|
| J | Q | Y |
| Z | 0 | 0 |
| P | 0 | 0 |
| U | 0 | 0 |

| | Q | Y |
|---|---|---|
| Q | P | 0 |
| Y | 0 | 0 |

| | J | Z | P | U |
|---|---|---|---|---|
| J | J | Z | P | U |
| Z | Z | 0 | 0 | 0 |
| P | P | 0 | 0 | 0 |
| U | U | 0 | 0 | 0 |

| | Q | Y |
|---|---|---|
| J | Q | Y |
| Z | 0 | 0 |
| P | 0 | 0 |
| U | 0 | 0 |

| | Q | Y |
|---|---|---|
| Q | P + Z | U + Z |
| Y | U + Z | P + Z |

| | J | Z | P | U |
|---|---|---|---|---|
| J | J | Z | P | U |
| Z | Z | 0 | 0 | 0 |
| P | P | 0 | 0 | 0 |
| U | U | 0 | 0 | Z |

| | Q | Y |
|---|---|---|
| J | Q | Y |
| Z | 0 | 0 |
| P | 0 | 0 |
| U | Y | 0 |

| | Q | Y |
|---|---|---|
| Q | P | 0 |
| Y | 0 | 0 |

| | J | Z | P | U |
|---|---|---|---|---|
| J | J | Z | P | U |
| Z | Z | 0 | 0 | 0 |
| P | P | 0 | 0 | 0 |
| U | U | 0 | 0 | 0 |

| | Q | Y |
|---|---|---|
| J | Q | Y |
| Z | 0 | 0 |
| P | 0 | 0 |
| U | 0 | 0 |

| | Q | Y |
|---|---|---|
| Q | P + Z | U + Z |
| Y | U + Z | U + Z |

| | J | Z | P | U |
|---|---|---|---|---|
| J | J | Z | P | U |
| Z | Z | 0 | 0 | 0 |
| P | P | 0 | 0 | 0 |
| U | U | 0 | 0 | Z |

| | Q | Y |
|---|---|---|
| J | Q | Y |
| Z | 0 | 0 |
| P | Y | 0 |
| U | 0 | 0 |

| | Q | Y |
|---|---|---|
| Q | P | 0 |
| Y | 0 | 0 |

| | J | Z | P | U |
|---|---|---|---|---|
| J | J | Z | P | U |
| Z | Z | 0 | 0 | P |
| P | P | 0 | 0 | 0 |
| U | U | P | 0 | 0 |

| | Q | Y |
|---|---|---|
| J | Q | Y |
| Z | 0 | 0 |
| P | 0 | 0 |
| U | 0 | 0 |

| | Q | Y |
|---|---|---|
| Q | P | 0 |
| Y | 0 | 0 |

| | J | Z | P | U |
|---|---|---|---|---|
| J | J | Z | P | U |
| Z | Z | 0 | 0 | 0 |
| P | P | 0 | 0 | 0 |
| U | U | 0 | 0 | Z |

| | Q | Y |
|---|---|---|
| J | Q | Y |
| Z | 0 | 0 |
| P | Y | 0 |
| U | Y | 0 |

| | Q | Y |
|---|---|---|
| Q | P | 0 |
| Y | 0 | 0 |

| | J | Z | P | U |
|---|---|---|---|---|
| J | J | Z | P | U |
| Z | Z | 0 | 0 | P |
| P | P | 0 | 0 | 0 |
| U | U | P | 0 | 0 |

| | Q | Y |
|---|---|---|
| J | Q | Y |
| Z | Y | 0 |
| P | 0 | 0 |
| U | 0 | 0 |

| | Q | Y |
|---|---|---|
| Q | P | 0 |
| Y | 0 | 0 |

| | J | Z | P | U |
|---|---|---|---|---|
| J | J | Z | P | U |
| Z | Z | 0 | 0 | 0 |
| P | P | 0 | 0 | 0 |
| U | U | 0 | 0 | Z |

| | Q | Y |
|---|---|---|
| J | Q | Y |
| Z | 0 | 0 |
| P | 0 | 0 |
| U | 0 | 0 |

| | Q | Y |
|---|---|---|
| Q | P | 0 |
| Y | 0 | P |

| | J | Z | P | U |
|---|---|---|---|---|
| J | J | Z | P | U |
| Z | Z | 0 | 0 | P |
| P | P | 0 | 0 | 0 |
| U | U | P | 0 | 0 |

| | Q | Y |
|---|---|---|
| J | Q | Y |
| Z | 0 | 0 |
| P | 0 | 0 |
| U | Y | 0 |

| | Q | Y |
|---|---|---|
| Q | P | 0 |
| Y | 0 | 0 |

| | J | Z | P | U |
|---|---|---|---|---|
| J | J | Z | P | U |
| Z | Z | 0 | 0 | 0 |
| P | P | 0 | 0 | 0 |
| U | U | 0 | 0 | Z |

| | Q | Y |
|---|---|---|
| J | Q | Y |
| Z | 0 | 0 |
| P | 0 | 0 |
| U | 0 | 0 |

| | Q | Y |
|---|---|---|
| Q | P | 0 |
| Y | 0 | Z |

| | J | Z | P | U |
|---|---|---|---|---|
| J | J | Z | P | U |
| Z | Z | 0 | 0 | P |
| P | P | 0 | 0 | 0 |
| U | U | P | 0 | 0 |

| | Q | Y |
|---|---|---|
| J | Q | Y |
| Z | Y | 0 |
| P | 0 | 0 |
| U | Y | 0 |

| | Q | Y |
|---|---|---|
| Q | P | 0 |
| Y | 0 | 0 |

| | J | Z | P | U |
|---|---|---|---|---|
| J | J | Z | P | U |
| Z | Z | 0 | 0 | 0 |
| P | P | 0 | 0 | 0 |
| U | U | 0 | 0 | Z |

| | Q | Y |
|---|---|---|
| J | Q | Y |
| Z | 0 | 0 |
| P | 0 | 0 |
| U | 0 | 0 |

| | Q | Y |
|---|---|---|
| Q | P | 0 |
| Y | 0 | P + Z |

| | J | Z | P | U |
|---|---|---|---|---|
| J | J | Z | P | U |
| Z | Z | 0 | 0 | P |
| P | P | 0 | 0 | 0 |
| U | U | P | 0 | 0 |

| | Q | Y |
|---|---|---|
| J | Q | Y |
| Z | 0 | 0 |
| P | 0 | 0 |
| U | 0 | 0 |

| | Q | Y |
|---|---|---|
| Q | P | 0 |
| Y | 0 | P |

| | J | Z | P | U |
|---|---|---|---|---|
| J | J | Z | P | U |
| Z | Z | 0 | 0 | 0 |
| P | P | 0 | 0 | 0 |
| U | U | 0 | 0 | Z |

| | Q | Y |
|---|---|---|
| J | Q | Y |
| Z | 0 | 0 |
| P | 0 | 0 |
| U | 0 | 0 |

| | Q | Y |
|---|---|---|
| Q | P | P |
| Y | P | 0 |

| | J | Z | P | U |
|---|---|---|---|---|
| J | J | Z | P | U |
| Z | Z | 0 | 0 | P |
| P | P | 0 | 0 | 0 |
| U | U | P | 0 | 0 |

| | Q | Y |
|---|---|---|
| J | Q | Y |
| Z | 0 | 0 |
| P | 0 | 0 |
| U | 0 | 0 |

| | Q | Y |
|---|---|---|
| Q | P | P |
| Y | P | 0 |

| | J | Z | P | U |
|---|---|---|---|---|
| J | J | Z | P | U |
| Z | Z | 0 | 0 | 0 |
| P | P | 0 | 0 | 0 |
| U | U | 0 | 0 | Z |

| | Q | Y |
|---|---|---|
| J | Q | Y |
| Z | 0 | 0 |
| P | 0 | 0 |
| U | 0 | 0 |

| | Q | Y |
|---|---|---|
| Q | P | P |
| Y | P | P |

| | J | Z | P | U |
|---|---|---|---|---|
| J | J | Z | P | U |
| Z | Z | 0 | 0 | P |
| P | P | 0 | 0 | 0 |
| U | U | P | 0 | 0 |

| | Q | Y |
|---|---|---|
| J | Q | Y |
| Z | 0 | 0 |
| P | 0 | 0 |
| U | 0 | 0 |

| | Q | Y |
|---|---|---|
| Q | P | P |
| Y | P | P |

| | J | Z | P | U |
|---|---|---|---|---|
| J | J | Z | P | U |
| Z | Z | 0 | 0 | 0 |
| P | P | 0 | 0 | 0 |
| U | U | 0 | 0 | Z |

| | Q | Y |
|---|---|---|
| J | Q | Y |
| Z | 0 | 0 |
| P | 0 | 0 |
| U | 0 | 0 |

| | Q | Y |
|---|---|---|
| Q | P | P |
| Y | P | Z |

| | J | Z | P | U |
|---|---|---|---|---|
| J | J | Z | P | U |
| Z | Z | 0 | 0 | P |
| P | P | 0 | 0 | 0 |
| U | U | P | 0 | 0 |

| | Q | Y |
|---|---|---|
| J | Q | Y |
| Z | 0 | 0 |
| P | 0 | 0 |
| U | Y | 0 |

| | Q | Y |
|---|---|---|
| Q | P + Z | P |
| Y | P | 0 |

| | J | Z | P | U |
|---|---|---|---|---|
| J | J | Z | P | U |
| Z | Z | 0 | 0 | 0 |
| P | P | 0 | 0 | 0 |
| U | U | 0 | 0 | Z |

| | Q | Y |
|---|---|---|
| J | Q | Y |
| Z | 0 | 0 |
| P | 0 | 0 |
| U | 0 | 0 |

| | Q | Y |
|---|---|---|
| Q | P | P |
| Y | P | P + Z |

| | J | Z | P | U |
|---|---|---|---|---|
| J | J | Z | P | U |
| Z | Z | 0 | U | 0 |
| P | P | U | 0 | 0 |
| U | U | 0 | 0 | 0 |

| | Q | Y |
|---|---|---|
| J | Q | Y |
| Z | Y | 0 |
| P | 0 | 0 |
| U | 0 | 0 |

| | Q | Y |
|---|---|---|
| Q | P | U |
| Y | U | 0 |

| | J | Z | P | U |
|---|---|---|---|---|
| J | J | Z | P | U |
| Z | Z | 0 | 0 | 0 |
| P | P | 0 | 0 | 0 |
| U | U | 0 | 0 | Z |

| | Q | Y |
|---|---|---|
| J | Q | Y |
| Z | 0 | 0 |
| P | 0 | 0 |
| U | 0 | 0 |

| | Q | Y |
|---|---|---|
| Q | P | Z |
| Y | Z | 0 |

| | J | Z | P | U |
|---|---|---|---|---|
| J | J | Z | P | U |
| Z | Z | 0 | U | 0 |
| P | P | U | 0 | 0 |
| U | U | 0 | 0 | 0 |

| | Q | Y |
|---|---|---|
| J | Q | Y |
| Z | Y | 0 |
| P | Y | 0 |
| U | 0 | 0 |

| | Q | Y |
|---|---|---|
| Q | P + Z | U |
| Y | U | 0 |

| | J | Z | P | U |
|---|---|---|---|---|
| J | J | Z | P | U |
| Z | Z | 0 | 0 | 0 |
| P | P | 0 | 0 | 0 |
| U | U | 0 | 0 | Z |

| | Q | Y |
|---|---|---|
| J | Q | Y |
| Z | 0 | 0 |
| P | 0 | 0 |
| U | 0 | 0 |

| | Q | Y |
|---|---|---|
| Q | P | Z |
| Y | Z | P |

| | $J$ | $Z$ | $P$ | $U$ |
|---|---|---|---|---|
| $J$ | $J$ | $Z$ | $P$ | $U$ |
| $Z$ | $Z$ | 0 | 0 | 0 |
| $P$ | $P$ | 0 | 0 | 0 |
| $U$ | $U$ | 0 | 0 | $Z$ |

| | $Q$ | $Y$ |
|---|---|---|
| $J$ | $Q$ | $Y$ |
| $Z$ | 0 | 0 |
| $P$ | 0 | 0 |
| $U$ | 0 | 0 |

| | $Q$ | $Y$ |
|---|---|---|
| $Q$ | $P$ | $Z$ |
| $Y$ | $Z$ | $Z$ |

| | $J$ | $Z$ | $P$ | $U$ |
|---|---|---|---|---|
| $J$ | $J$ | $Z$ | $P$ | $U$ |
| $Z$ | $Z$ | 0 | 0 | 0 |
| $P$ | $P$ | 0 | 0 | 0 |
| $U$ | $U$ | 0 | 0 | $Z$ |

| | $Q$ | $Y$ |
|---|---|---|
| $J$ | $Q$ | $Y$ |
| $Z$ | 0 | 0 |
| $P$ | 0 | 0 |
| $U$ | 0 | 0 |

| | $Q$ | $Y$ |
|---|---|---|
| $Q$ | $P+Z$ | $P$ |
| $Y$ | $P$ | 0 |

| | $J$ | $Z$ | $P$ | $U$ |
|---|---|---|---|---|
| $J$ | $J$ | $Z$ | $P$ | $U$ |
| $Z$ | $Z$ | 0 | 0 | 0 |
| $P$ | $P$ | 0 | 0 | 0 |
| $U$ | $U$ | 0 | 0 | $Z$ |

| | $Q$ | $Y$ |
|---|---|---|
| $J$ | $Q$ | $Y$ |
| $Z$ | 0 | 0 |
| $P$ | 0 | 0 |
| $U$ | 0 | 0 |

| | $Q$ | $Y$ |
|---|---|---|
| $Q$ | $P$ | $Z$ |
| $Y$ | $Z$ | $P+Z$ |

| | $J$ | $Z$ | $P$ | $U$ |
|---|---|---|---|---|
| $J$ | $J$ | $Z$ | $P$ | $U$ |
| $Z$ | $Z$ | 0 | 0 | 0 |
| $P$ | $P$ | 0 | 0 | 0 |
| $U$ | $U$ | 0 | 0 | $Z$ |

| | $Q$ | $Y$ |
|---|---|---|
| $J$ | $Q$ | $Y$ |
| $Z$ | 0 | 0 |
| $P$ | 0 | 0 |
| $U$ | 0 | 0 |

| | $Q$ | $Y$ |
|---|---|---|
| $Q$ | $P+Z$ | $P$ |
| $Y$ | $P$ | $P$ |

| | $J$ | $Z$ | $P$ | $U$ |
|---|---|---|---|---|
| $J$ | $J$ | $Z$ | $P$ | $U$ |
| $Z$ | $Z$ | 0 | 0 | 0 |
| $P$ | $P$ | 0 | 0 | 0 |
| $U$ | $U$ | 0 | 0 | $Z$ |

| | $Q$ | $Y$ |
|---|---|---|
| $J$ | $Q$ | $Y$ |
| $Z$ | 0 | 0 |
| $P$ | 0 | 0 |
| $U$ | 0 | 0 |

| | $Q$ | $Y$ |
|---|---|---|
| $Q$ | $P$ | $P+Z$ |
| $Y$ | $P+Z$ | 0 |

| | $J$ | $Z$ | $P$ | $U$ |
|---|---|---|---|---|
| $J$ | $J$ | $Z$ | $P$ | $U$ |
| $Z$ | $Z$ | 0 | 0 | 0 |
| $P$ | $P$ | 0 | 0 | 0 |
| $U$ | $U$ | 0 | 0 | $Z$ |

| | $Q$ | $Y$ |
|---|---|---|
| $J$ | $Q$ | $Y$ |
| $Z$ | 0 | 0 |
| $P$ | 0 | 0 |
| $U$ | 0 | 0 |

| | $Q$ | $Y$ |
|---|---|---|
| $Q$ | $P+Z$ | $P$ |
| $Y$ | $P$ | $Z$ |

| | $J$ | $Z$ | $P$ | $U$ |
|---|---|---|---|---|
| $J$ | $J$ | $Z$ | $P$ | $U$ |
| $Z$ | $Z$ | 0 | 0 | 0 |
| $P$ | $P$ | 0 | 0 | 0 |
| $U$ | $U$ | 0 | 0 | $Z$ |

| | $Q$ | $Y$ |
|---|---|---|
| $J$ | $Q$ | $Y$ |
| $Z$ | 0 | 0 |
| $P$ | 0 | 0 |
| $U$ | 0 | 0 |

| | $Q$ | $Y$ |
|---|---|---|
| $Q$ | $P$ | $P+Z$ |
| $Y$ | $P+Z$ | $P$ |

| | $J$ | $Z$ | $P$ | $U$ |
|---|---|---|---|---|
| $J$ | $J$ | $Z$ | $P$ | $U$ |
| $Z$ | $Z$ | 0 | 0 | 0 |
| $P$ | $P$ | 0 | 0 | 0 |
| $U$ | $U$ | 0 | 0 | $Z$ |

| | $Q$ | $Y$ |
|---|---|---|
| $J$ | $Q$ | $Y$ |
| $Z$ | 0 | 0 |
| $P$ | 0 | 0 |
| $U$ | 0 | 0 |

| | $Q$ | $Y$ |
|---|---|---|
| $Q$ | $P+Z$ | $P$ |
| $Y$ | $P$ | $P+Z$ |

| | $J$ | $Z$ | $P$ | $U$ |
|---|---|---|---|---|
| $J$ | $J$ | $Z$ | $P$ | $U$ |
| $Z$ | $Z$ | 0 | 0 | 0 |
| $P$ | $P$ | 0 | 0 | 0 |
| $U$ | $U$ | 0 | 0 | $Z$ |

| | $Q$ | $Y$ |
|---|---|---|
| $J$ | $Q$ | $Y$ |
| $Z$ | 0 | 0 |
| $P$ | 0 | 0 |
| $U$ | 0 | 0 |

| | $Q$ | $Y$ |
|---|---|---|
| $Q$ | $P$ | $P+Z$ |
| $Y$ | $P+Z$ | $Z$ |

| | $J$ | $Z$ | $P$ | $U$ |
|---|---|---|---|---|
| $J$ | $J$ | $Z$ | $P$ | $U$ |
| $Z$ | $Z$ | 0 | 0 | 0 |
| $P$ | $P$ | 0 | 0 | 0 |
| $U$ | $U$ | 0 | 0 | $Z$ |

| | $Q$ | $Y$ |
|---|---|---|
| $J$ | $Q$ | $Y$ |
| $Z$ | 0 | 0 |
| $P$ | 0 | 0 |
| $U$ | 0 | 0 |

| | $Q$ | $Y$ |
|---|---|---|
| $Q$ | $P+Z$ | $Z$ |
| $Y$ | $Z$ | 0 |

| | $J$ | $Z$ | $P$ | $U$ |
|---|---|---|---|---|
| $J$ | $J$ | $Z$ | $P$ | $U$ |
| $Z$ | $Z$ | 0 | 0 | 0 |
| $P$ | $P$ | 0 | 0 | 0 |
| $U$ | $U$ | 0 | 0 | $Z$ |

| | $Q$ | $Y$ |
|---|---|---|
| $J$ | $Q$ | $Y$ |
| $Z$ | 0 | 0 |
| $P$ | 0 | 0 |
| $U$ | 0 | 0 |

| | $Q$ | $Y$ |
|---|---|---|
| $Q$ | $P$ | $P+Z$ |
| $Y$ | $P+Z$ | $P+Z$ |

| | $J$ | $Z$ | $P$ | $U$ |
|---|---|---|---|---|
| $J$ | $J$ | $Z$ | $P$ | $U$ |
| $Z$ | $Z$ | 0 | 0 | 0 |
| $P$ | $P$ | 0 | 0 | 0 |
| $U$ | $U$ | 0 | 0 | $Z$ |

| | $Q$ | $Y$ |
|---|---|---|
| $J$ | $Q$ | $Y$ |
| $Z$ | 0 | 0 |
| $P$ | 0 | 0 |
| $U$ | 0 | 0 |

| | $Q$ | $Y$ |
|---|---|---|
| $Q$ | $P+Z$ | $Z$ |
| $Y$ | $Z$ | $P$ |

| | $J$ | $Z$ | $P$ | $U$ |
|---|---|---|---|---|
| $J$ | $J$ | $Z$ | $P$ | $U$ |
| $Z$ | $Z$ | 0 | 0 | 0 |
| $P$ | $P$ | 0 | 0 | 0 |
| $U$ | $U$ | 0 | 0 | $Z$ |

| | $Q$ | $Y$ |
|---|---|---|
| $J$ | $Q$ | $Y$ |
| $Z$ | 0 | 0 |
| $P$ | 0 | 0 |
| $U$ | 0 | 0 |

| | $Q$ | $Y$ |
|---|---|---|
| $Q$ | $P+Z$ | 0 |
| $Y$ | 0 | 0 |

| | $J$ | $Z$ | $P$ | $U$ |
|---|---|---|---|---|
| $J$ | $J$ | $Z$ | $P$ | $U$ |
| $Z$ | $Z$ | 0 | 0 | 0 |
| $P$ | $P$ | 0 | 0 | 0 |
| $U$ | $U$ | 0 | 0 | $Z$ |

| | $Q$ | $Y$ |
|---|---|---|
| $J$ | $Q$ | $Y$ |
| $Z$ | 0 | 0 |
| $P$ | 0 | 0 |
| $U$ | 0 | 0 |

| | $Q$ | $Y$ |
|---|---|---|
| $Q$ | $P+Z$ | $Z$ |
| $Y$ | $Z$ | $Z$ |

| | $J$ | $Z$ | $P$ | $U$ |
|---|---|---|---|---|
| $J$ | $J$ | $Z$ | $P$ | $U$ |
| $Z$ | $Z$ | 0 | 0 | 0 |
| $P$ | $P$ | 0 | 0 | 0 |
| $U$ | $U$ | 0 | 0 | $Z$ |

| | $Q$ | $Y$ |
|---|---|---|
| $J$ | $Q$ | $Y$ |
| $Z$ | 0 | 0 |
| $P$ | 0 | 0 |
| $U$ | $Y$ | 0 |

| | $Q$ | $Y$ |
|---|---|---|
| $Q$ | $P+Z$ | 0 |
| $Y$ | 0 | 0 |

| | $J$ | $Z$ | $P$ | $U$ |
|---|---|---|---|---|
| $J$ | $J$ | $Z$ | $P$ | $U$ |
| $Z$ | $Z$ | 0 | 0 | 0 |
| $P$ | $P$ | 0 | 0 | 0 |
| $U$ | $U$ | 0 | 0 | $Z$ |

| | $Q$ | $Y$ |
|---|---|---|
| $J$ | $Q$ | $Y$ |
| $Z$ | 0 | 0 |
| $P$ | 0 | 0 |
| $U$ | 0 | 0 |

| | $Q$ | $Y$ |
|---|---|---|
| $Q$ | $P+Z$ | $Z$ |
| $Y$ | $Z$ | $P+Z$ |

| | $J$ | $Z$ | $P$ | $U$ |
|---|---|---|---|---|
| $J$ | $J$ | $Z$ | $P$ | $U$ |
| $Z$ | $Z$ | 0 | 0 | 0 |
| $P$ | $P$ | 0 | 0 | 0 |
| $U$ | $U$ | 0 | 0 | $Z$ |

| | $Q$ | $Y$ |
|---|---|---|
| $J$ | $Q$ | $Y$ |
| $Z$ | 0 | 0 |
| $P$ | $Y$ | 0 |
| $U$ | 0 | 0 |

| | $Q$ | $Y$ |
|---|---|---|
| $Q$ | $P+Z$ | 0 |
| $Y$ | 0 | 0 |

| | $J$ | $Z$ | $P$ | $U$ |
|---|---|---|---|---|
| $J$ | $J$ | $Z$ | $P$ | $U$ |
| $Z$ | $Z$ | 0 | 0 | 0 |
| $P$ | $P$ | 0 | 0 | 0 |
| $U$ | $U$ | 0 | 0 | $Z$ |

| | $Q$ | $Y$ |
|---|---|---|
| $J$ | $Q$ | $Y$ |
| $Z$ | 0 | 0 |
| $P$ | 0 | 0 |
| $U$ | 0 | 0 |

| | $Q$ | $Y$ |
|---|---|---|
| $Q$ | $P+Z$ | $P+Z$ |
| $Y$ | $P+Z$ | 0 |

| | $J$ | $Z$ | $P$ | $U$ |
|---|---|---|---|---|
| $J$ | $J$ | $Z$ | $P$ | $U$ |
| $Z$ | $Z$ | 0 | 0 | 0 |
| $P$ | $P$ | 0 | 0 | 0 |
| $U$ | $U$ | 0 | 0 | $Z$ |

| | $Q$ | $Y$ |
|---|---|---|
| $J$ | $Q$ | $Y$ |
| $Z$ | 0 | 0 |
| $P$ | $Y$ | 0 |
| $U$ | $Y$ | 0 |

| | $Q$ | $Y$ |
|---|---|---|
| $Q$ | $P+Z$ | 0 |
| $Y$ | 0 | 0 |

| | $J$ | $Z$ | $P$ | $U$ |
|---|---|---|---|---|
| $J$ | $J$ | $Z$ | $P$ | $U$ |
| $Z$ | $Z$ | 0 | 0 | 0 |
| $P$ | $P$ | 0 | 0 | 0 |
| $U$ | $U$ | 0 | 0 | $Z$ |

| | $Q$ | $Y$ |
|---|---|---|
| $J$ | $Q$ | $Y$ |
| $Z$ | 0 | 0 |
| $P$ | 0 | 0 |
| $U$ | 0 | 0 |

| | $Q$ | $Y$ |
|---|---|---|
| $Q$ | $P+Z$ | $P+Z$ |
| $Y$ | $P+Z$ | $P$ |

| | $J$ | $Z$ | $P$ | $U$ |
|---|---|---|---|---|
| $J$ | $J$ | $Z$ | $P$ | $U$ |
| $Z$ | $Z$ | 0 | 0 | 0 |
| $P$ | $P$ | 0 | 0 | 0 |
| $U$ | $U$ | 0 | 0 | $Z$ |

| | $Q$ | $Y$ |
|---|---|---|
| $J$ | $Q$ | $Y$ |
| $Z$ | 0 | 0 |
| $P$ | 0 | 0 |
| $U$ | 0 | 0 |

| | $Q$ | $Y$ |
|---|---|---|
| $Q$ | $P+Z$ | 0 |
| $Y$ | 0 | $P$ |

| | $J$ | $Z$ | $P$ | $U$ |
|---|---|---|---|---|
| $J$ | $J$ | $Z$ | $P$ | $U$ |
| $Z$ | $Z$ | 0 | 0 | 0 |
| $P$ | $P$ | 0 | 0 | 0 |
| $U$ | $U$ | 0 | 0 | $Z$ |

| | $Q$ | $Y$ |
|---|---|---|
| $J$ | $Q$ | $Y$ |
| $Z$ | 0 | 0 |
| $P$ | 0 | 0 |
| $U$ | 0 | 0 |

| | $Q$ | $Y$ |
|---|---|---|
| $Q$ | $P+Z$ | $P+Z$ |
| $Y$ | $P+Z$ | $Z$ |

| | $J$ | $Z$ | $P$ | $U$ |
|---|---|---|---|---|
| $J$ | $J$ | $Z$ | $P$ | $U$ |
| $Z$ | $Z$ | 0 | 0 | 0 |
| $P$ | $P$ | 0 | 0 | 0 |
| $U$ | $U$ | 0 | 0 | $Z$ |

| | $Q$ | $Y$ |
|---|---|---|
| $J$ | $Q$ | $Y$ |
| $Z$ | 0 | 0 |
| $P$ | 0 | 0 |
| $U$ | 0 | 0 |

| | $Q$ | $Y$ |
|---|---|---|
| $Q$ | $P+Z$ | 0 |
| $Y$ | 0 | $Z$ |

| | $J$ | $Z$ | $P$ | $U$ |
|---|---|---|---|---|
| $J$ | $J$ | $Z$ | $P$ | $U$ |
| $Z$ | $Z$ | 0 | 0 | 0 |
| $P$ | $P$ | 0 | 0 | 0 |
| $U$ | $U$ | 0 | 0 | $Z$ |

| | $Q$ | $Y$ |
|---|---|---|
| $J$ | $Q$ | $Y$ |
| $Z$ | 0 | 0 |
| $P$ | 0 | 0 |
| $U$ | 0 | 0 |

| | $Q$ | $Y$ |
|---|---|---|
| $Q$ | $P+Z$ | $P+Z$ |
| $Y$ | $P+Z$ | $P+Z$ |

| | $J$ | $Z$ | $P$ | $U$ |
|---|---|---|---|---|
| $J$ | $J$ | $Z$ | $P$ | $U$ |
| $Z$ | $Z$ | 0 | 0 | 0 |
| $P$ | $P$ | 0 | 0 | 0 |
| $U$ | $U$ | 0 | 0 | $Z$ |

| | $Q$ | $Y$ |
|---|---|---|
| $J$ | $Q$ | $Y$ |
| $Z$ | 0 | 0 |
| $P$ | 0 | 0 |
| $U$ | 0 | 0 |

| | $Q$ | $Y$ |
|---|---|---|
| $Q$ | $P+Z$ | 0 |
| $Y$ | 0 | $P+Z$ |

| | $J$ | $Z$ | $P$ | $U$ |
|---|---|---|---|---|
| $J$ | $J$ | $Z$ | $P$ | $U$ |
| $Z$ | $Z$ | 0 | 0 | $P$ |
| $P$ | $P$ | 0 | 0 | 0 |
| $U$ | $U$ | $P$ | 0 | $Z$ |

| | $Q$ | $Y$ |
|---|---|---|
| $J$ | $Q$ | $Y$ |
| $Z$ | 0 | 0 |
| $P$ | 0 | 0 |
| $U$ | 0 | 0 |

| | $Q$ | $Y$ |
|---|---|---|
| $Q$ | $P$ | 0 |
| $Y$ | 0 | 0 |

| | J | Z | P | U |
|---|---|---|---|---|
| J | J | Z | P | U |
| Z | Z | 0 | 0 | P |
| P | P | 0 | 0 | 0 |
| U | U | P | 0 | Z |

| | Q | Y |
|---|---|---|
| J | Q | Y |
| Z | 0 | 0 |
| P | 0 | 0 |
| U | Y | 0 |

| | Q | Y |
|---|---|---|
| Q | P | 0 |
| Y | 0 | 0 |

| | J | Z | P | U |
|---|---|---|---|---|
| J | J | Z | P | U |
| Z | Z | 0 | 0 | P |
| P | P | 0 | 0 | Z |
| U | U | P | Z | J |

| | Q | Y |
|---|---|---|
| J | Q | Y |
| Z | 0 | 0 |
| P | 0 | 0 |
| U | Q | Y |

| | Q | Y |
|---|---|---|
| Q | $P+Z$ | $P+Z$ |
| Y | $P+Z$ | 0 |

| | J | Z | P | U |
|---|---|---|---|---|
| J | J | Z | P | U |
| Z | Z | 0 | 0 | P |
| P | P | 0 | 0 | 0 |
| U | U | P | 0 | Z |

| | Q | Y |
|---|---|---|
| J | Q | Y |
| Z | 0 | 0 |
| P | 0 | 0 |
| U | 0 | 0 |

| | Q | Y |
|---|---|---|
| Q | P | 0 |
| Y | 0 | P |

| | J | Z | P | U |
|---|---|---|---|---|
| J | J | Z | P | U |
| Z | Z | 0 | 0 | P |
| P | P | 0 | 0 | Z |
| U | U | P | Z | J |

| | Q | Y |
|---|---|---|
| J | Q | Y |
| Z | 0 | 0 |
| P | 0 | 0 |
| U | Q | Y |

| | Q | Y |
|---|---|---|
| Q | $P+Z$ | $P+Z$ |
| Y | $P+Z$ | $P+Z$ |

| | J | Z | P | U |
|---|---|---|---|---|
| J | J | Z | P | U |
| Z | Z | 0 | 0 | P |
| P | P | 0 | 0 | 0 |
| U | U | P | 0 | Z |

| | Q | Y |
|---|---|---|
| J | Q | Y |
| Z | 0 | 0 |
| P | 0 | 0 |
| U | 0 | 0 |

| | Q | Y |
|---|---|---|
| Q | P | P |
| Y | P | 0 |

| | J | Z | P | U |
|---|---|---|---|---|
| J | J | Z | P | U |
| Z | Z | 0 | 0 | P |
| P | P | 0 | 0 | Z |
| U | U | P | Z | J |

| | Q | Y |
|---|---|---|
| J | Q | Y |
| Z | 0 | 0 |
| P | 0 | 0 |
| U | Y | Q |

| | Q | Y |
|---|---|---|
| Q | $P+Z$ | $P+Z$ |
| Y | $P+Z$ | $P+Z$ |

| | J | Z | P | U |
|---|---|---|---|---|
| J | J | Z | P | U |
| Z | Z | 0 | 0 | P |
| P | P | 0 | 0 | 0 |
| U | U | P | 0 | Z |

| | Q | Y |
|---|---|---|
| J | Q | Y |
| Z | 0 | 0 |
| P | 0 | 0 |
| U | 0 | 0 |

| | Q | Y |
|---|---|---|
| Q | P | P |
| Y | P | P |

| | J | Z | P | U |
|---|---|---|---|---|
| J | J | Z | P | U |
| Z | Z | 0 | 0 | 0 |
| P | P | 0 | Z | 0 |
| U | U | 0 | 0 | 0 |

| | Q | Y |
|---|---|---|
| J | Q | Y |
| Z | 0 | 0 |
| P | Y | 0 |
| U | 0 | 0 |

| | Q | Y |
|---|---|---|
| Q | P | Z |
| Y | Z | 0 |

| | J | Z | P | U |
|---|---|---|---|---|
| J | J | Z | P | U |
| Z | Z | 0 | 0 | P |
| P | P | 0 | 0 | 0 |
| U | U | P | 0 | Z |

| | Q | Y |
|---|---|---|
| J | Q | Y |
| Z | 0 | 0 |
| P | 0 | 0 |
| U | Y | 0 |

| | Q | Y |
|---|---|---|
| Q | $P+Z$ | P |
| Y | P | 0 |

| | J | Z | P | U |
|---|---|---|---|---|
| J | J | Z | P | U |
| Z | Z | 0 | 0 | 0 |
| P | P | 0 | Z | 0 |
| U | U | 0 | 0 | 0 |

| | Q | Y |
|---|---|---|
| J | Q | Y |
| Z | 0 | 0 |
| P | Y | 0 |
| U | 0 | 0 |

| | Q | Y |
|---|---|---|
| Q | $P+Z$ | Z |
| Y | Z | 0 |

| | J | Z | P | U |
|---|---|---|---|---|
| J | J | Z | P | U |
| Z | Z | 0 | 0 | 0 |
| P | P | 0 | 0 | Z |
| U | U | 0 | Z | 0 |

| | Q | Y |
|---|---|---|
| J | Q | Y |
| Z | 0 | 0 |
| P | 0 | 0 |
| U | Y | 0 |

| | Q | Y |
|---|---|---|
| Q | P | Z |
| Y | Z | 0 |

| | J | Z | P | U |
|---|---|---|---|---|
| J | J | Z | P | U |
| Z | Z | 0 | 0 | 0 |
| P | P | 0 | Z | 0 |
| U | U | 0 | 0 | Z |

| | Q | Y |
|---|---|---|
| J | Q | Y |
| Z | 0 | 0 |
| P | Y | 0 |
| U | 0 | 0 |

| | Q | Y |
|---|---|---|
| Q | P | Z |
| Y | Z | 0 |

| | J | Z | P | U |
|---|---|---|---|---|
| J | J | Z | P | U |
| Z | Z | 0 | 0 | 0 |
| P | P | 0 | 0 | Z |
| U | U | 0 | Z | 0 |

| | Q | Y |
|---|---|---|
| J | Q | Y |
| Z | 0 | 0 |
| P | 0 | 0 |
| U | Y | 0 |

| | Q | Y |
|---|---|---|
| Q | $P+Z$ | Z |
| Y | Z | 0 |

| | J | Z | P | U |
|---|---|---|---|---|
| J | J | Z | P | U |
| Z | Z | 0 | 0 | 0 |
| P | P | 0 | Z | 0 |
| U | U | 0 | 0 | Z |

| | Q | Y |
|---|---|---|
| J | Q | Y |
| Z | 0 | 0 |
| P | Y | 0 |
| U | 0 | 0 |

| | Q | Y |
|---|---|---|
| Q | $P+Z$ | Z |
| Y | Z | 0 |

| | J | Z | P | U |
|---|---|---|---|---|
| J | J | Z | P | U |
| Z | Z | 0 | 0 | 0 |
| P | P | 0 | 0 | Z |
| U | U | 0 | Z | Z |

| | Q | Y |
|---|---|---|
| J | Q | Y |
| Z | 0 | 0 |
| P | 0 | 0 |
| U | Y | 0 |

| | Q | Y |
|---|---|---|
| Q | P | Z |
| Y | Z | 0 |

| | J | Z | P | U |
|---|---|---|---|---|
| J | J | Z | P | U |
| Z | Z | 0 | 0 | 0 |
| P | P | 0 | Z | Z |
| U | U | 0 | Z | 0 |

| | Q | Y |
|---|---|---|
| J | Q | Y |
| Z | 0 | 0 |
| P | Y | 0 |
| U | Y | 0 |

| | Q | Y |
|---|---|---|
| Q | P | Z |
| Y | Z | 0 |

| | J | Z | P | U |
|---|---|---|---|---|
| J | J | Z | P | U |
| Z | Z | 0 | 0 | 0 |
| P | P | 0 | 0 | Z |
| U | U | 0 | Z | Z |

| | Q | Y |
|---|---|---|
| J | Q | Y |
| Z | 0 | 0 |
| P | 0 | 0 |
| U | Y | 0 |

| | Q | Y |
|---|---|---|
| Q | $P+Z$ | Z |
| Y | Z | 0 |

| | J | Z | P | U |
|---|---|---|---|---|
| J | J | Z | P | U |
| Z | Z | 0 | 0 | 0 |
| P | P | 0 | Z | Z |
| U | U | 0 | Z | 0 |

| | Q | Y |
|---|---|---|
| J | Q | Y |
| Z | 0 | 0 |
| P | Y | 0 |
| U | Y | 0 |

| | Q | Y |
|---|---|---|
| Q | $P+Z$ | Z |
| Y | Z | 0 |

| | J | Z | P | U |
|---|---|---|---|---|
| J | J | Z | P | U |
| Z | Z | 0 | 0 | P |
| P | P | 0 | 0 | Z |
| U | U | P | Z | J |

| | Q | Y |
|---|---|---|
| J | Q | Y |
| Z | 0 | 0 |
| P | 0 | 0 |
| U | Y | Q |

| | Q | Y |
|---|---|---|
| Q | P | Z |
| Y | Z | P |

| | J | Z | P | U |
|---|---|---|---|---|
| J | J | Z | P | U |
| Z | Z | 0 | 0 | 0 |
| P | P | 0 | Z | Z |
| U | U | 0 | Z | Z |

| | Q | Y |
|---|---|---|
| J | Q | Y |
| Z | 0 | 0 |
| P | Y | 0 |
| U | Y | 0 |

| | Q | Y |
|---|---|---|
| Q | P | Z |
| Y | Z | 0 |

| | J | Z | P | U |
|---|---|---|---|---|
| J | J | Z | P | U |
| Z | Z | 0 | 0 | P |
| P | P | 0 | 0 | Z |
| U | U | P | Z | J |

| | Q | Y |
|---|---|---|
| J | Q | Y |
| Z | 0 | 0 |
| P | 0 | 0 |
| U | Q | Y |

| | Q | Y |
|---|---|---|
| Q | $P+Z$ | 0 |
| Y | 0 | 0 |

| | J | Z | P | U |
|---|---|---|---|---|
| J | J | Z | P | U |
| Z | Z | 0 | 0 | 0 |
| P | P | 0 | Z | Z |
| U | U | 0 | Z | Z |

| | Q | Y |
|---|---|---|
| J | Q | Y |
| Z | 0 | 0 |
| P | Y | 0 |
| U | Y | 0 |

| | Q | Y |
|---|---|---|
| Q | $P+Z$ | Z |
| Y | Z | 0 |

| | J | Z | P | U |
|---|---|---|---|---|
| J | J | Z | P | U |
| Z | Z | 0 | 0 | P |
| P | P | 0 | 0 | Z |
| U | U | P | Z | J |

| | Q | Y |
|---|---|---|
| J | Q | Y |
| Z | Y | 0 |
| P | Y | 0 |
| U | Q | Y |

| | Q | Y |
|---|---|---|
| Q | $P+Z$ | 0 |
| Y | 0 | 0 |

| | J | Z | P | U |
|---|---|---|---|---|
| J | J | Z | P | U |
| Z | Z | 0 | U | 0 |
| P | P | U | J | Z |
| U | U | 0 | Z | 0 |

| | Q | Y |
|---|---|---|
| J | Q | Y |
| Z | Y | 0 |
| P | Q | Y |
| U | Y | 0 |

| | Q | Y |
|---|---|---|
| Q | $J+P$ | $U+Z$ |
| Y | $U+Z$ | 0 |

| | J | Z | P | U |
|---|---|---|---|---|
| J | J | Z | P | U |
| Z | Z | 0 | 0 | P |
| P | P | 0 | 0 | Z |
| U | U | P | Z | J |

| | Q | Y |
|---|---|---|
| J | Q | Y |
| Z | 0 | 0 |
| P | 0 | 0 |
| U | Q | Y |

| | Q | Y |
|---|---|---|
| Q | $P+Z$ | 0 |
| Y | 0 | $P+Z$ |

| | J | Z | P | U |
|---|---|---|---|---|
| J | J | Z | P | U |
| Z | Z | Z | 0 | 0 |
| P | P | 0 | 0 | 0 |
| U | U | 0 | 0 | 0 |

| | Q | Y |
|---|---|---|
| J | Q | Y |
| Z | 0 | 0 |
| P | 0 | 0 |
| U | 0 | 0 |

| | Q | Y |
|---|---|---|
| Q | P | 0 |
| Y | 0 | 0 |

| | J | Z | P | U |
|---|---|---|---|---|
| J | J | Z | P | U |
| Z | Z | Z | 0 | 0 |
| P | P | 0 | 0 | 0 |
| U | U | 0 | 0 | 0 |

| | Q | Y |
|---|---|---|
| J | Q | Y |
| Z | 0 | Y |
| P | 0 | 0 |
| U | 0 | 0 |

| | Q | Y |
|---|---|---|
| Q | P | 0 |
| Y | 0 | 0 |

| | J | Z | P | U |
|---|---|---|---|---|
| J | J | Z | P | U |
| Z | Z | Z | 0 | 0 |
| P | P | 0 | 0 | 0 |
| U | U | 0 | 0 | 0 |

| | Q | Y |
|---|---|---|
| J | Q | Y |
| Z | 0 | 0 |
| P | 0 | 0 |
| U | 0 | 0 |

| | Q | Y |
|---|---|---|
| Q | P | U |
| Y | U | U |

| | J | Z | P | U |
|---|---|---|---|---|
| J | J | Z | P | U |
| Z | Z | Z | 0 | 0 |
| P | P | 0 | 0 | 0 |
| U | U | 0 | 0 | 0 |

| | Q | Y |
|---|---|---|
| J | Q | Y |
| Z | Y | Y |
| P | 0 | 0 |
| U | 0 | 0 |

| | Q | Y |
|---|---|---|
| Q | P | 0 |
| Y | 0 | 0 |

| | J | Z | P | U |
|---|---|---|---|---|
| J | J | Z | P | U |
| Z | Z | Z | 0 | 0 |
| P | P | 0 | 0 | 0 |
| U | U | 0 | 0 | 0 |

| | Q | Y |
|---|---|---|
| J | Q | Y |
| Z | Y | Y |
| P | 0 | 0 |
| U | 0 | 0 |

| | Q | Y |
|---|---|---|
| Q | $P+Z$ | Z |
| Y | Z | Z |

| | J | Z | P | U |
|---|---|---|---|---|
| J | J | Z | P | U |
| Z | Z | Z | 0 | 0 |
| P | P | 0 | 0 | 0 |
| U | U | 0 | 0 | 0 |

| | Q | Y |
|---|---|---|
| J | Q | Y |
| Z | 0 | 0 |
| P | 0 | 0 |
| U | Y | 0 |

| | Q | Y |
|---|---|---|
| Q | P | 0 |
| Y | 0 | 0 |

| | J | Z | P | U |
|---|---|---|---|---|
| J | J | Z | P | U |
| Z | Z | Z | 0 | U |
| P | P | 0 | 0 | 0 |
| U | U | U | 0 | 0 |

| | Q | Y |
|---|---|---|
| J | Q | Y |
| Z | 0 | 0 |
| P | 0 | 0 |
| U | 0 | 0 |

| | Q | Y |
|---|---|---|
| Q | P | 0 |
| Y | 0 | 0 |

| | J | Z | P | U |
|---|---|---|---|---|
| J | J | Z | P | U |
| Z | Z | Z | 0 | 0 |
| P | P | 0 | 0 | 0 |
| U | U | 0 | 0 | 0 |

| | Q | Y |
|---|---|---|
| J | Q | Y |
| Z | 0 | 0 |
| P | Y | 0 |
| U | 0 | 0 |

| | Q | Y |
|---|---|---|
| Q | P | 0 |
| Y | 0 | 0 |

| | J | Z | P | U |
|---|---|---|---|---|
| J | J | Z | P | U |
| Z | Z | Z | 0 | U |
| P | P | 0 | 0 | 0 |
| U | U | U | 0 | 0 |

| | Q | Y |
|---|---|---|
| J | Q | Y |
| Z | 0 | Y |
| P | 0 | 0 |
| U | 0 | 0 |

| | Q | Y |
|---|---|---|
| Q | P | 0 |
| Y | 0 | 0 |

| | J | Z | P | U |
|---|---|---|---|---|
| J | J | Z | P | U |
| Z | Z | Z | 0 | 0 |
| P | P | 0 | 0 | 0 |
| U | U | 0 | 0 | 0 |

| | Q | Y |
|---|---|---|
| J | Q | Y |
| Z | 0 | 0 |
| P | Y | 0 |
| U | Y | 0 |

| | Q | Y |
|---|---|---|
| Q | P | 0 |
| Y | 0 | 0 |

| | J | Z | P | U |
|---|---|---|---|---|
| J | J | Z | P | U |
| Z | Z | Z | 0 | U |
| P | P | 0 | 0 | 0 |
| U | U | U | 0 | 0 |

| | Q | Y |
|---|---|---|
| J | Q | Y |
| Z | Y | Y |
| P | 0 | 0 |
| U | 0 | 0 |

| | Q | Y |
|---|---|---|
| Q | P | 0 |
| Y | 0 | 0 |

| | J | Z | P | U |
|---|---|---|---|---|
| J | J | Z | P | U |
| Z | Z | Z | 0 | 0 |
| P | P | 0 | 0 | 0 |
| U | U | 0 | 0 | 0 |

| | Q | Y |
|---|---|---|
| J | Q | Y |
| Z | 0 | 0 |
| P | 0 | 0 |
| U | 0 | 0 |

| | Q | Y |
|---|---|---|
| Q | P | 0 |
| Y | 0 | P |

| | J | Z | P | U |
|---|---|---|---|---|
| J | J | Z | P | U |
| Z | Z | Z | 0 | U |
| P | P | 0 | 0 | 0 |
| U | U | U | 0 | 0 |

| | Q | Y |
|---|---|---|
| J | Q | Y |
| Z | 0 | 0 |
| P | Y | 0 |
| U | 0 | 0 |

| | Q | Y |
|---|---|---|
| Q | P | 0 |
| Y | 0 | 0 |

| | J | Z | P | U |
|---|---|---|---|---|
| J | J | Z | P | U |
| Z | Z | Z | 0 | 0 |
| P | P | 0 | 0 | 0 |
| U | U | 0 | 0 | 0 |

| | Q | Y |
|---|---|---|
| J | Q | Y |
| Z | 0 | 0 |
| P | 0 | 0 |
| U | 0 | 0 |

| | Q | Y |
|---|---|---|
| Q | P | 0 |
| Y | 0 | U |

| | J | Z | P | U |
|---|---|---|---|---|
| J | J | Z | P | U |
| Z | Z | Z | 0 | U |
| P | P | 0 | 0 | 0 |
| U | U | U | 0 | 0 |

| | Q | Y |
|---|---|---|
| J | Q | Y |
| Z | 0 | 0 |
| P | 0 | 0 |
| U | 0 | 0 |

| | Q | Y |
|---|---|---|
| Q | P | 0 |
| Y | 0 | P |

| | J | Z | P | U |
|---|---|---|---|---|
| J | J | Z | P | U |
| Z | Z | Z | 0 | 0 |
| P | P | 0 | 0 | 0 |
| U | U | 0 | 0 | 0 |

| | Q | Y |
|---|---|---|
| J | Q | Y |
| Z | 0 | Y |
| P | 0 | 0 |
| U | 0 | 0 |

| | Q | Y |
|---|---|---|
| Q | P | 0 |
| Y | 0 | Z |

| | J | Z | P | U |
|---|---|---|---|---|
| J | J | Z | P | U |
| Z | Z | Z | 0 | U |
| P | P | 0 | 0 | 0 |
| U | U | U | 0 | 0 |

| | Q | Y |
|---|---|---|
| J | Q | Y |
| Z | 0 | Y |
| P | 0 | 0 |
| U | 0 | 0 |

| | Q | Y |
|---|---|---|
| Q | P | 0 |
| Y | 0 | U |

| | J | Z | P | U |
|---|---|---|---|---|
| J | J | Z | P | U |
| Z | Z | Z | 0 | 0 |
| P | P | 0 | 0 | 0 |
| U | U | 0 | 0 | 0 |

| | Q | Y |
|---|---|---|
| J | Q | Y |
| Z | 0 | 0 |
| P | 0 | 0 |
| U | 0 | 0 |

| | Q | Y |
|---|---|---|
| Q | P | P |
| Y | P | 0 |

| | J | Z | P | U |
|---|---|---|---|---|
| J | J | Z | P | U |
| Z | Z | Z | 0 | U |
| P | P | 0 | 0 | 0 |
| U | U | U | 0 | 0 |

| | Q | Y |
|---|---|---|
| J | Q | Y |
| Z | 0 | 0 |
| P | 0 | 0 |
| U | 0 | 0 |

| | Q | Y |
|---|---|---|
| Q | P | P |
| Y | P | 0 |

| | J | Z | P | U |
|---|---|---|---|---|
| J | J | Z | P | U |
| Z | Z | Z | 0 | 0 |
| P | P | 0 | 0 | 0 |
| U | U | 0 | 0 | 0 |

| | Q | Y |
|---|---|---|
| J | Q | Y |
| Z | 0 | 0 |
| P | 0 | 0 |
| U | 0 | 0 |

| | Q | Y |
|---|---|---|
| Q | P | P |
| Y | P | P |

| | J | Z | P | U |
|---|---|---|---|---|
| J | J | Z | P | U |
| Z | Z | Z | 0 | U |
| P | P | 0 | 0 | 0 |
| U | U | U | 0 | 0 |

| | Q | Y |
|---|---|---|
| J | Q | Y |
| Z | 0 | 0 |
| P | 0 | 0 |
| U | 0 | 0 |

| | Q | Y |
|---|---|---|
| Q | P | P |
| Y | P | P |

| | J | Z | P | U |
|---|---|---|---|---|
| J | J | Z | P | U |
| Z | Z | Z | 0 | 0 |
| P | P | 0 | 0 | 0 |
| U | U | 0 | 0 | 0 |

| | Q | Y |
|---|---|---|
| J | Q | Y |
| Z | 0 | 0 |
| P | 0 | 0 |
| U | 0 | 0 |

| | Q | Y |
|---|---|---|
| Q | P | P |
| Y | P | U |

| | J | Z | P | U |
|---|---|---|---|---|
| J | J | Z | P | U |
| Z | Z | Z | P | 0 |
| P | P | P | 0 | 0 |
| U | U | 0 | 0 | 0 |

| | Q | Y |
|---|---|---|
| J | Q | Y |
| Z | Q | 0 |
| P | 0 | 0 |
| U | 0 | 0 |

| | Q | Y |
|---|---|---|
| Q | P | 0 |
| Y | 0 | 0 |

| | J | Z | P | U |
|---|---|---|---|---|
| J | J | Z | P | U |
| Z | Z | Z | 0 | 0 |
| P | P | 0 | 0 | 0 |
| U | U | 0 | 0 | 0 |

| | Q | Y |
|---|---|---|
| J | Q | Y |
| Z | 0 | 0 |
| P | 0 | 0 |
| U | 0 | 0 |

| | Q | Y |
|---|---|---|
| Q | P | U |
| Y | U | 0 |

| | J | Z | P | U |
|---|---|---|---|---|
| J | J | Z | P | U |
| Z | Z | Z | P | 0 |
| P | P | P | 0 | 0 |
| U | U | 0 | 0 | 0 |

| | Q | Y |
|---|---|---|
| J | Q | Y |
| Z | Q | Y |
| P | 0 | 0 |
| U | 0 | 0 |

| | Q | Y |
|---|---|---|
| Q | P | 0 |
| Y | 0 | 0 |

| | J | Z | P | U |
|---|---|---|---|---|
| J | J | Z | P | U |
| Z | Z | Z | 0 | 0 |
| P | P | 0 | 0 | 0 |
| U | U | 0 | 0 | 0 |

| | Q | Y |
|---|---|---|
| J | Q | Y |
| Z | 0 | 0 |
| P | 0 | 0 |
| U | 0 | 0 |

| | Q | Y |
|---|---|---|
| Q | P | U |
| Y | U | P |

| | J | Z | P | U |
|---|---|---|---|---|
| J | J | Z | P | U |
| Z | Z | Z | P | 0 |
| P | P | P | 0 | 0 |
| U | U | 0 | 0 | 0 |

| | Q | Y |
|---|---|---|
| J | Q | Y |
| Z | Q | Y |
| P | Y | 0 |
| U | 0 | 0 |

| | Q | Y |
|---|---|---|
| Q | P | 0 |
| Y | 0 | 0 |

| | J | Z | P | U |
|---|---|---|---|---|
| J | J | Z | P | U |
| Z | Z | Z | P | 0 |
| P | P | P | 0 | 0 |
| U | U | 0 | 0 | 0 |

| | Q | Y |
|---|---|---|
| J | Q | Y |
| Z | Q | Y |
| P | 0 | 0 |
| U | 0 | 0 |

| | Q | Y |
|---|---|---|
| Q | P | 0 |
| Y | 0 | P |

| | J | Z | P | U |
|---|---|---|---|---|
| J | J | Z | P | U |
| Z | Z | Z | P | 0 |
| P | P | P | 0 | 0 |
| U | U | 0 | 0 | 0 |

| | Q | Y |
|---|---|---|
| J | Q | Y |
| Z | Q | 0 |
| P | 0 | 0 |
| U | 0 | 0 |

| | Q | Y |
|---|---|---|
| Q | P | 0 |
| Y | 0 | U |

| | J | Z | P | U |
|---|---|---|---|---|
| J | J | Z | P | U |
| Z | Z | Z | P | 0 |
| P | P | P | 0 | 0 |
| U | U | 0 | 0 | 0 |

| | Q | Y |
|---|---|---|
| J | Q | Y |
| Z | Q | Y |
| P | 0 | 0 |
| U | 0 | 0 |

| | Q | Y |
|---|---|---|
| Q | P | P |
| Y | P | 0 |

| | J | Z | P | U |
|---|---|---|---|---|
| J | J | Z | P | U |
| Z | Z | Z | P | 0 |
| P | P | P | 0 | 0 |
| U | U | 0 | 0 | 0 |

| | Q | Y |
|---|---|---|
| J | Q | Y |
| Z | Q | Q |
| P | 0 | 0 |
| U | 0 | 0 |

| | Q | Y |
|---|---|---|
| Q | P | P |
| Y | P | P |

| | J | Z | P | U |
|---|---|---|---|---|
| J | J | Z | P | U |
| Z | Z | Z | P | 0 |
| P | P | P | 0 | 0 |
| U | U | 0 | 0 | 0 |

| | Q | Y |
|---|---|---|
| J | Q | Y |
| Z | Q | Y |
| P | 0 | 0 |
| U | 0 | 0 |

| | Q | Y |
|---|---|---|
| Q | P | P |
| Y | P | P |

| | J | Z | P | U |
|---|---|---|---|---|
| J | J | Z | P | U |
| Z | Z | Z | P | 0 |
| P | P | P | 0 | 0 |
| U | U | 0 | 0 | 0 |

| | Q | Y |
|---|---|---|
| J | Q | Y |
| Z | Y | Y |
| P | 0 | 0 |
| U | 0 | 0 |

| | Q | Y |
|---|---|---|
| Q | P | P |
| Y | P | P |

| | J | Z | P | U |
|---|---|---|---|---|
| J | J | Z | P | U |
| Z | Z | Z | P | 0 |
| P | P | P | 0 | 0 |
| U | U | 0 | 0 | 0 |

| | Q | Y |
|---|---|---|
| J | Q | Y |
| Z | Q | Y |
| P | Y | 0 |
| U | 0 | 0 |

| | Q | Y |
|---|---|---|
| Q | $P+Z$ | P |
| Y | P | 0 |

| | J | Z | P | U |
|---|---|---|---|---|
| J | J | Z | P | U |
| Z | Z | Z | P | P |
| P | P | P | 0 | 0 |
| U | U | P | 0 | 0 |

| | Q | Y |
|---|---|---|
| J | Q | Y |
| Z | Q | 0 |
| P | 0 | 0 |
| U | 0 | 0 |

| | Q | Y |
|---|---|---|
| Q | P | 0 |
| Y | 0 | 0 |

| | J | Z | P | U |
|---|---|---|---|---|
| J | J | Z | P | U |
| Z | Z | Z | P | P |
| P | P | P | 0 | 0 |
| U | U | P | 0 | 0 |

| | Q | Y |
|---|---|---|
| J | Q | Y |
| Z | Q | Y |
| P | 0 | 0 |
| U | 0 | 0 |

| | Q | Y |
|---|---|---|
| Q | P | 0 |
| Y | 0 | 0 |

| | J | Z | P | U |
|---|---|---|---|---|
| J | J | Z | P | U |
| Z | Z | Z | P | P |
| P | P | P | 0 | 0 |
| U | U | P | 0 | 0 |

| | Q | Y |
|---|---|---|
| J | Q | Y |
| Z | Q | Y |
| P | Y | 0 |
| U | Y | 0 |

| | Q | Y |
|---|---|---|
| Q | P | 0 |
| Y | 0 | 0 |

| | J | Z | P | U |
|---|---|---|---|---|
| J | J | Z | P | U |
| Z | Z | Z | P | P |
| P | P | P | 0 | 0 |
| U | U | P | 0 | 0 |

| | Q | Y |
|---|---|---|
| J | Q | Y |
| Z | Q | Y |
| P | 0 | 0 |
| U | 0 | 0 |

| | Q | Y |
|---|---|---|
| Q | P | 0 |
| Y | 0 | P |

| | J | Z | P | U |
|---|---|---|---|---|
| J | J | Z | P | U |
| Z | Z | Z | P | P |
| P | P | P | 0 | 0 |
| U | U | P | 0 | 0 |

| | Q | Y |
|---|---|---|
| J | Q | Y |
| Z | Q | Y |
| P | 0 | 0 |
| U | 0 | 0 |

| | Q | Y |
|---|---|---|
| Q | P | P |
| Y | P | 0 |

| | J | Z | P | U |
|---|---|---|---|---|
| J | J | Z | P | U |
| Z | Z | Z | P | P |
| P | P | P | 0 | 0 |
| U | U | P | 0 | 0 |

| | Q | Y |
|---|---|---|
| J | Q | Y |
| Z | Q | Q |
| P | 0 | 0 |
| U | 0 | 0 |

| | Q | Y |
|---|---|---|
| Q | P | P |
| Y | P | P |

| | J | Z | P | U |
|---|---|---|---|---|
| J | J | Z | P | U |
| Z | Z | Z | P | P |
| P | P | P | 0 | 0 |
| U | U | P | 0 | 0 |

| | Q | Y |
|---|---|---|
| J | Q | Y |
| Z | Q | Y |
| P | 0 | 0 |
| U | 0 | 0 |

| | Q | Y |
|---|---|---|
| Q | P | P |
| Y | P | P |

| | J | Z | P | U |
|---|---|---|---|---|
| J | J | Z | P | U |
| Z | Z | Z | P | P |
| P | P | P | 0 | 0 |
| U | U | P | 0 | 0 |

| | Q | Y |
|---|---|---|
| J | Q | Y |
| Z | Y | Y |
| P | 0 | 0 |
| U | 0 | 0 |

| | Q | Y |
|---|---|---|
| Q | P | P |
| Y | P | P |

| | J | Z | P | U |
|---|---|---|---|---|
| J | J | Z | P | U |
| Z | Z | Z | P | P |
| P | P | P | 0 | 0 |
| U | U | P | 0 | 0 |

| | Q | Y |
|---|---|---|
| J | Q | Y |
| Z | Q | Q |
| P | 0 | 0 |
| U | 0 | 0 |

| | Q | Y |
|---|---|---|
| Q | P | P |
| Y | P | U |

| | J | Z | P | U |
|---|---|---|---|---|
| J | J | Z | P | U |
| Z | Z | Z | P | P |
| P | P | P | 0 | 0 |
| U | U | P | 0 | 0 |

| | Q | Y |
|---|---|---|
| J | Q | Y |
| Z | Q | Y |
| P | Y | 0 |
| U | Y | 0 |

| | Q | Y |
|---|---|---|
| Q | $P+Z$ | P |
| Y | P | 0 |

| | J | Z | P | U |
|---|---|---|---|---|
| J | J | Z | P | U |
| Z | Z | Z | P | U |
| P | P | P | 0 | 0 |
| U | U | U | 0 | 0 |

| | Q | Y |
|---|---|---|
| J | Q | Y |
| Z | Q | 0 |
| P | 0 | 0 |
| U | 0 | 0 |

| | Q | Y |
|---|---|---|
| Q | P | 0 |
| Y | 0 | 0 |

| | J | Z | P | U |
|---|---|---|---|---|
| J | J | Z | P | U |
| Z | Z | Z | P | U |
| P | P | P | 0 | 0 |
| U | U | U | 0 | 0 |

| | Q | Y |
|---|---|---|
| J | Q | Y |
| Z | Q | Y |
| P | 0 | 0 |
| U | 0 | 0 |

| | Q | Y |
|---|---|---|
| Q | P | 0 |
| Y | 0 | 0 |

| | J | Z | P | U |
|---|---|---|---|---|
| J | J | Z | P | U |
| Z | Z | Z | P | U |
| P | P | P | 0 | 0 |
| U | U | U | 0 | 0 |

| | Q | Y |
|---|---|---|
| J | Q | Y |
| Z | Q | Y |
| P | 0 | 0 |
| U | Y | 0 |

| | Q | Y |
|---|---|---|
| Q | P | 0 |
| Y | 0 | 0 |

| | J | Z | P | U |
|---|---|---|---|---|
| J | J | Z | P | U |
| Z | Z | Z | P | U |
| P | P | P | 0 | 0 |
| U | U | U | 0 | 0 |

| | Q | Y |
|---|---|---|
| J | Q | Y |
| Z | Q | Y |
| P | Y | 0 |
| U | 0 | 0 |

| | Q | Y |
|---|---|---|
| Q | P | 0 |
| Y | 0 | 0 |

| | J | Z | P | U |
|---|---|---|---|---|
| J | J | Z | P | U |
| Z | Z | Z | P | U |
| P | P | P | 0 | 0 |
| U | U | U | 0 | 0 |

| | Q | Y |
|---|---|---|
| J | Q | Y |
| Z | Q | Y |
| P | Y | 0 |
| U | Y | 0 |

| | Q | Y |
|---|---|---|
| Q | P | 0 |
| Y | 0 | 0 |

| | J | Z | P | U |
|---|---|---|---|---|
| J | J | Z | P | U |
| Z | Z | Z | P | U |
| P | P | P | 0 | 0 |
| U | U | U | 0 | 0 |

| | Q | Y |
|---|---|---|
| J | Q | Y |
| Z | Q | Y |
| P | 0 | 0 |
| U | 0 | 0 |

| | Q | Y |
|---|---|---|
| Q | P | 0 |
| Y | 0 | P |

| | J | Z | P | U |
|---|---|---|---|---|
| J | J | Z | P | U |
| Z | Z | Z | P | U |
| P | P | P | 0 | 0 |
| U | U | U | 0 | 0 |

| | Q | Y |
|---|---|---|
| J | Q | Y |
| Z | Q | Y |
| P | 0 | 0 |
| U | 0 | 0 |

| | Q | Y |
|---|---|---|
| Q | P | 0 |
| Y | 0 | U |

| | J | Z | P | U |
|---|---|---|---|---|
| J | J | Z | P | U |
| Z | Z | Z | P | U |
| P | P | P | 0 | 0 |
| U | U | U | 0 | 0 |

| | Q | Y |
|---|---|---|
| J | Q | Y |
| Z | Q | Y |
| P | 0 | 0 |
| U | 0 | 0 |

| | Q | Y |
|---|---|---|
| Q | P | P |
| Y | P | 0 |

| | J | Z | P | U |
|---|---|---|---|---|
| J | J | Z | P | U |
| Z | Z | Z | P | U |
| P | P | P | 0 | 0 |
| U | U | U | 0 | 0 |

| | Q | Y |
|---|---|---|
| J | Q | Y |
| Z | Q | Q |
| P | 0 | 0 |
| U | 0 | 0 |

| | Q | Y |
|---|---|---|
| Q | P | P |
| Y | P | P |

| | J | Z | P | U |
|---|---|---|---|---|
| J | J | Z | P | U |
| Z | Z | Z | P | U |
| P | P | P | 0 | 0 |
| U | U | U | 0 | 0 |

| | Q | Y |
|---|---|---|
| J | Q | Y |
| Z | Q | Y |
| P | 0 | 0 |
| U | 0 | 0 |

| | Q | Y |
|---|---|---|
| Q | P | P |
| Y | P | P |

| | J | Z | P | U |
|---|---|---|---|---|
| J | J | Z | P | U |
| Z | Z | Z | 0 | U |
| P | P | 0 | 0 | 0 |
| U | U | U | 0 | Z |

| | Q | Y |
|---|---|---|
| J | Q | Y |
| Z | 0 | 0 |
| P | 0 | 0 |
| U | 0 | 0 |

| | Q | Y |
|---|---|---|
| Q | P | P |
| Y | P | 0 |

| | J | Z | P | U |
|---|---|---|---|---|
| J | J | Z | P | U |
| Z | Z | Z | P | U |
| P | P | P | 0 | 0 |
| U | U | U | 0 | 0 |

| | Q | Y |
|---|---|---|
| J | Q | Y |
| Z | Y | Y |
| P | 0 | 0 |
| U | 0 | 0 |

| | Q | Y |
|---|---|---|
| Q | P | P |
| Y | P | P |

| | J | Z | P | U |
|---|---|---|---|---|
| J | J | Z | P | U |
| Z | Z | Z | 0 | U |
| P | P | 0 | 0 | 0 |
| U | U | U | 0 | Z |

| | Q | Y |
|---|---|---|
| J | Q | Y |
| Z | 0 | 0 |
| P | 0 | 0 |
| U | 0 | 0 |

| | Q | Y |
|---|---|---|
| Q | P | P |
| Y | P | P |

| | J | Z | P | U |
|---|---|---|---|---|
| J | J | Z | P | U |
| Z | Z | Z | P | U |
| P | P | P | 0 | 0 |
| U | U | U | 0 | 0 |

| | Q | Y |
|---|---|---|
| J | Q | Y |
| Z | Q | Y |
| P | 0 | 0 |
| U | 0 | 0 |

| | Q | Y |
|---|---|---|
| Q | P | P |
| Y | P | U |

| | J | Z | P | U |
|---|---|---|---|---|
| J | J | Z | P | U |
| Z | Z | Z | P | 0 |
| P | P | P | Z | 0 |
| U | U | 0 | 0 | 0 |

| | Q | Y |
|---|---|---|
| J | Q | Y |
| Z | Q | Y |
| P | Y | Q |
| U | 0 | 0 |

| | Q | Y |
|---|---|---|
| Q | P | Z |
| Y | Z | P |

| | J | Z | P | U |
|---|---|---|---|---|
| J | J | Z | P | U |
| Z | Z | Z | P | U |
| P | P | P | 0 | 0 |
| U | U | U | 0 | 0 |

| | Q | Y |
|---|---|---|
| J | Q | Y |
| Z | Q | Y |
| P | 0 | 0 |
| U | 0 | 0 |

| | Q | Y |
|---|---|---|
| Q | P | U |
| Y | U | 0 |

| | J | Z | P | U |
|---|---|---|---|---|
| J | J | Z | P | U |
| Z | Z | Z | P | 0 |
| P | P | P | Z | 0 |
| U | U | 0 | 0 | 0 |

| | Q | Y |
|---|---|---|
| J | Q | Y |
| Z | Q | 0 |
| P | Q | 0 |
| U | 0 | 0 |

| | Q | Y |
|---|---|---|
| Q | $P+Z$ | 0 |
| Y | 0 | 0 |

| | J | Z | P | U |
|---|---|---|---|---|
| J | J | Z | P | U |
| Z | Z | Z | P | U |
| P | P | P | 0 | 0 |
| U | U | U | 0 | 0 |

| | Q | Y |
|---|---|---|
| J | Q | Y |
| Z | Q | Y |
| P | 0 | 0 |
| U | 0 | 0 |

| | Q | Y |
|---|---|---|
| Q | P | U |
| Y | U | P |

| | J | Z | P | U |
|---|---|---|---|---|
| J | J | Z | P | U |
| Z | Z | Z | P | 0 |
| P | P | P | Z | 0 |
| U | U | 0 | 0 | 0 |

| | Q | Y |
|---|---|---|
| J | Q | Y |
| Z | Q | 0 |
| P | Q | 0 |
| U | 0 | 0 |

| | Q | Y |
|---|---|---|
| Q | $P+Z$ | 0 |
| Y | 0 | U |

| | J | Z | P | U |
|---|---|---|---|---|
| J | J | Z | P | U |
| Z | Z | Z | P | U |
| P | P | P | 0 | 0 |
| U | U | U | 0 | 0 |

| | Q | Y |
|---|---|---|
| J | Q | Y |
| Z | Q | Y |
| P | 0 | 0 |
| U | 0 | 0 |

| | Q | Y |
|---|---|---|
| Q | P | U |
| Y | U | U |

| | J | Z | P | U |
|---|---|---|---|---|
| J | J | Z | P | U |
| Z | Z | Z | P | 0 |
| P | P | P | Z | 0 |
| U | U | 0 | 0 | 0 |

| | Q | Y |
|---|---|---|
| J | Q | Y |
| Z | Q | Q |
| P | Q | Q |
| U | 0 | 0 |

| | Q | Y |
|---|---|---|
| Q | $P+Z$ | $P+Z$ |
| Y | $P+Z$ | $P+Z$ |

| | J | Z | P | U |
|---|---|---|---|---|
| J | J | Z | P | U |
| Z | Z | Z | U | U |
| P | P | U | 0 | 0 |
| U | U | U | 0 | 0 |

| | Q | Y |
|---|---|---|
| J | Q | Y |
| Z | Y | Y |
| P | 0 | 0 |
| U | 0 | 0 |

| | Q | Y |
|---|---|---|
| Q | P | U |
| Y | U | U |

| | J | Z | P | U |
|---|---|---|---|---|
| J | J | Z | P | U |
| Z | Z | Z | P | 0 |
| P | P | P | Z | 0 |
| U | U | 0 | 0 | 0 |

| | Q | Y |
|---|---|---|
| J | Q | Y |
| Z | Q | Y |
| P | Y | Q |
| U | 0 | 0 |

| | Q | Y |
|---|---|---|
| Q | $P+Z$ | $P+Z$ |
| Y | $P+Z$ | $P+Z$ |

| | J | Z | P | U |
|---|---|---|---|---|
| J | J | Z | P | U |
| Z | Z | Z | 0 | U |
| P | P | 0 | 0 | 0 |
| U | U | U | 0 | Z |

| | Q | Y |
|---|---|---|
| J | Q | Y |
| Z | 0 | 0 |
| P | 0 | 0 |
| U | 0 | 0 |

| | Q | Y |
|---|---|---|
| Q | P | 0 |
| Y | 0 | 0 |

| | J | Z | P | U |
|---|---|---|---|---|
| J | J | Z | P | U |
| Z | Z | Z | P | 0 |
| P | P | P | Z | 0 |
| U | U | 0 | 0 | 0 |

| | Q | Y |
|---|---|---|
| J | Q | Y |
| Z | Y | Y |
| P | Y | Y |
| U | 0 | 0 |

| | Q | Y |
|---|---|---|
| Q | $P+Z$ | $P+Z$ |
| Y | $P+Z$ | $P+Z$ |

| | J | Z | P | U |
|---|---|---|---|---|
| J | J | Z | P | U |
| Z | Z | Z | 0 | U |
| P | P | 0 | 0 | 0 |
| U | U | U | 0 | Z |

| | Q | Y |
|---|---|---|
| J | Q | Y |
| Z | 0 | Y |
| P | 0 | 0 |
| U | 0 | Y |

| | Q | Y |
|---|---|---|
| Q | P | 0 |
| Y | 0 | 0 |

| | J | Z | P | U |
|---|---|---|---|---|
| J | J | Z | P | U |
| Z | Z | Z | P | P |
| P | P | P | Z | Z |
| U | U | P | Z | Z |

| | Q | Y |
|---|---|---|
| J | Q | Y |
| Z | Q | Y |
| P | Y | Q |
| U | Y | Q |

| | Q | Y |
|---|---|---|
| Q | P | Z |
| Y | Z | P |

| | J | Z | P | U |
|---|---|---|---|---|
| J | J | Z | P | U |
| Z | Z | Z | 0 | U |
| P | P | 0 | 0 | 0 |
| U | U | U | 0 | Z |

| | Q | Y |
|---|---|---|
| J | Q | Y |
| Z | Y | Y |
| P | 0 | 0 |
| U | Y | Y |

| | Q | Y |
|---|---|---|
| Q | P | 0 |
| Y | 0 | 0 |

| | J | Z | P | U |
|---|---|---|---|---|
| J | J | Z | P | U |
| Z | Z | Z | P | P |
| P | P | P | Z | Z |
| U | U | P | Z | Z |

| | Q | Y |
|---|---|---|
| J | Q | Y |
| Z | Q | 0 |
| P | Q | 0 |
| U | Q | 0 |

| | Q | Y |
|---|---|---|
| Q | $P+Z$ | 0 |
| Y | 0 | 0 |

| | J | Z | P | U |
|---|---|---|---|---|
| J | J | Z | P | U |
| Z | Z | Z | 0 | U |
| P | P | 0 | 0 | 0 |
| U | U | U | 0 | Z |

| | Q | Y |
|---|---|---|
| J | Q | Y |
| Z | 0 | 0 |
| P | Y | 0 |
| U | 0 | 0 |

| | Q | Y |
|---|---|---|
| Q | P | 0 |
| Y | 0 | 0 |

| | J | Z | P | U |
|---|---|---|---|---|
| J | J | Z | P | U |
| Z | Z | Z | P | P |
| P | P | P | Z | Z |
| U | U | P | Z | Z |

| | Q | Y |
|---|---|---|
| J | Q | Y |
| Z | Q | Q |
| P | Q | Q |
| U | Q | Q |

| | Q | Y |
|---|---|---|
| Q | $P+Z$ | $P+Z$ |
| Y | $P+Z$ | $P+Z$ |

| | J | Z | P | U |
|---|---|---|---|---|
| J | J | Z | P | U |
| Z | Z | Z | 0 | U |
| P | P | 0 | 0 | 0 |
| U | U | U | 0 | Z |

| | Q | Y |
|---|---|---|
| J | Q | Y |
| Z | 0 | 0 |
| P | 0 | 0 |
| U | 0 | 0 |

| | Q | Y |
|---|---|---|
| Q | P | 0 |
| Y | 0 | P |

| | J | Z | P | U |
|---|---|---|---|---|
| J | J | Z | P | U |
| Z | Z | Z | P | P |
| P | P | P | Z | Z |
| U | U | P | Z | Z |

| | Q | Y |
|---|---|---|
| J | Q | Y |
| Z | Q | Y |
| P | Y | Q |
| U | Y | Q |

| | Q | Y |
|---|---|---|
| Q | $P+Z$ | $P+Z$ |
| Y | $P+Z$ | $P+Z$ |

| | J | Z | P | U |
|---|---|---|---|---|
| J | J | Z | P | U |
| Z | Z | Z | 0 | U |
| P | P | 0 | 0 | 0 |
| U | U | U | 0 | Z |

| | Q | Y |
|---|---|---|
| J | Q | Y |
| Z | 0 | Y |
| P | 0 | 0 |
| U | 0 | Y |

| | Q | Y |
|---|---|---|
| Q | P | 0 |
| Y | 0 | $U+Z$ |

| | J | Z | P | U |
|---|---|---|---|---|
| J | J | Z | P | U |
| Z | Z | Z | P | P |
| P | P | P | Z | Z |
| U | U | P | Z | Z |

| | Q | Y |
|---|---|---|
| J | Q | Y |
| Z | Y | Y |
| P | Y | Y |
| U | Y | Y |

| | Q | Y |
|---|---|---|
| Q | $P+Z$ | $P+Z$ |
| Y | $P+Z$ | $P+Z$ |

| | J | Z | P | U |
|---|---|---|---|---|
| J | J | Z | P | U |
| Z | Z | Z | P | P |
| P | P | P | Z | Z |
| U | U | P | Z | Z |

| | Q | Y |
|---|---|---|
| J | Q | Y |
| Z | Q | Q |
| P | Q | Q |
| U | Q | Q |

| | Q | Y |
|---|---|---|
| Q | $P+Z$ | $P+Z$ |
| Y | $P+Z$ | $U+Z$ |

| | J | Z | P | U |
|---|---|---|---|---|
| J | J | Z | P | U |
| Z | Z | Z | U | U |
| P | P | U | Z | Z |
| U | U | U | Z | Z |

| | Q | Y |
|---|---|---|
| J | Q | Y |
| Z | Y | Y |
| P | Y | Y |
| U | Y | Y |

| | Q | Y |
|---|---|---|
| Q | $P+Z$ | $U+Z$ |
| Y | $U+Z$ | $U+Z$ |

| | J | Z | P | U |
|---|---|---|---|---|
| J | J | Z | P | U |
| Z | Z | Z | P | P |
| P | P | P | Z | Z |
| U | U | P | Z | J |

| | Q | Y |
|---|---|---|
| J | Q | Y |
| Z | Q | Y |
| P | Y | Q |
| U | Y | Q |

| | Q | Y |
|---|---|---|
| Q | P | Z |
| Y | Z | P |

| | J | Z | P | U |
|---|---|---|---|---|
| J | J | Z | P | U |
| Z | Z | Z | P | P |
| P | P | P | Z | Z |
| U | U | P | Z | J |

| | Q | Y |
|---|---|---|
| J | Q | Y |
| Z | Q | 0 |
| P | Q | 0 |
| U | Q | Y |

| | Q | Y |
|---|---|---|
| Q | $P+Z$ | 0 |
| Y | 0 | 0 |

| | J | Z | P | U |
|---|---|---|---|---|
| J | J | Z | P | U |
| Z | Z | Z | P | P |
| P | P | P | Z | Z |
| U | U | P | Z | J |

| | Q | Y |
|---|---|---|
| J | Q | Y |
| Z | Q | Q |
| P | Q | Q |
| U | Q | Y |

| | Q | Y |
|---|---|---|
| Q | $P+Z$ | $P+Z$ |
| Y | $P+Z$ | $P+Z$ |

| | J | Z | P | U |
|---|---|---|---|---|
| J | J | Z | P | U |
| Z | Z | Z | P | P |
| P | P | P | Z | Z |
| U | U | P | Z | J |

| | Q | Y |
|---|---|---|
| J | Q | Y |
| Z | Q | Y |
| P | Y | Q |
| U | Y | Q |

| | Q | Y |
|---|---|---|
| Q | $P+Z$ | $P+Z$ |
| Y | $P+Z$ | $P+Z$ |

| | J | Z | P | U |
|---|---|---|---|---|
| J | J | Z | P | U |
| Z | Z | Z | P | P |
| P | P | P | Z | Z |
| U | U | P | Z | J |

| | Q | Y |
|---|---|---|
| J | Q | Y |
| Z | Y | Y |
| P | Y | Y |
| U | Q | Y |

| | Q | Y |
|---|---|---|
| Q | $P+Z$ | $P+Z$ |
| Y | $P+Z$ | $P+Z$ |

| | J | Z | P | U |
|---|---|---|---|---|
| J | J | Z | P | U |
| Z | Z | Z | P | P |
| P | P | P | Z | Z |
| U | U | P | Z | J |

| | Q | Y |
|---|---|---|
| J | Q | Y |
| Z | Q | Q |
| P | Q | Q |
| U | Q | Y |

| | Q | Y |
|---|---|---|
| Q | $P+Z$ | $P+Z$ |
| Y | $P+Z$ | $J+U$ |

| | J | Z | P | U |
|---|---|---|---|---|
| J | J | Z | P | U |
| Z | Z | Z | U | U |
| P | P | U | J | Z |
| U | U | U | Z | Z |

| | Q | Y |
|---|---|---|
| J | Q | Y |
| Z | Y | Y |
| P | Q | Y |
| U | Y | Y |

| | Q | Y |
|---|---|---|
| Q | $J+P$ | $U+Z$ |
| Y | $U+Z$ | $U+Z$ |

| | J | Z | P | U |
|---|---|---|---|---|
| J | J | Z | P | U |
| Z | Z | J | P | U |
| P | P | P | 0 | 0 |
| U | U | U | 0 | 0 |

| | Q | Y |
|---|---|---|
| J | Q | Y |
| Z | Q | Y |
| P | 0 | 0 |
| U | 0 | 0 |

| | Q | Y |
|---|---|---|
| Q | P | 0 |
| Y | 0 | 0 |

| | J | Z | P | U |
|---|---|---|---|---|
| J | J | Z | P | U |
| Z | Z | J | P | U |
| P | P | P | 0 | 0 |
| U | U | U | 0 | 0 |

| | Q | Y |
|---|---|---|
| J | Q | Y |
| Z | Q | Y |
| P | 0 | 0 |
| U | Y | 0 |

| | Q | Y |
|---|---|---|
| Q | P | 0 |
| Y | 0 | 0 |

| | J | Z | P | U |
|---|---|---|---|---|
| J | J | Z | P | U |
| Z | Z | J | P | U |
| P | P | P | 0 | 0 |
| U | U | U | 0 | 0 |

| | Q | Y |
|---|---|---|
| J | Q | Y |
| Z | Q | Y |
| P | Y | 0 |
| U | 0 | 0 |

| | Q | Y |
|---|---|---|
| Q | P | 0 |
| Y | 0 | 0 |

| | J | Z | P | U |
|---|---|---|---|---|
| J | J | Z | P | U |
| Z | Z | J | P | U |
| P | P | P | 0 | 0 |
| U | U | U | 0 | 0 |

| | Q | Y |
|---|---|---|
| J | Q | Y |
| Z | Q | Y |
| P | Y | 0 |
| U | Y | 0 |

| | Q | Y |
|---|---|---|
| Q | P | 0 |
| Y | 0 | 0 |

| | J | Z | P | U |
|---|---|---|---|---|
| J | J | Z | P | U |
| Z | Z | J | P | U |
| P | P | P | 0 | 0 |
| U | U | U | 0 | 0 |

| | Q | Y |
|---|---|---|
| J | Q | Y |
| Z | Q | Y |
| P | 0 | 0 |
| U | 0 | 0 |

| | Q | Y |
|---|---|---|
| Q | P | 0 |
| Y | 0 | P |

| | J | Z | P | U |
|---|---|---|---|---|
| J | J | Z | P | U |
| Z | Z | J | P | U |
| P | P | P | 0 | 0 |
| U | U | U | 0 | 0 |

| | Q | Y |
|---|---|---|
| J | Q | Y |
| Z | Q | Y |
| P | 0 | 0 |
| U | 0 | 0 |

| | Q | Y |
|---|---|---|
| Q | P | 0 |
| Y | 0 | U |

| | J | Z | P | U |
|---|---|---|---|---|
| J | J | Z | P | U |
| Z | Z | J | P | U |
| P | P | P | 0 | 0 |
| U | U | U | 0 | 0 |

| | Q | Y |
|---|---|---|
| J | Q | Y |
| Z | Q | Y |
| P | 0 | 0 |
| U | 0 | 0 |

| | Q | Y |
|---|---|---|
| Q | P | P |
| Y | P | 0 |

| | J | Z | P | U |
|---|---|---|---|---|
| J | J | Z | P | U |
| Z | Z | J | P | U |
| P | P | P | 0 | 0 |
| U | U | U | 0 | 0 |

| | Q | Y |
|---|---|---|
| J | Q | Y |
| Z | Q | Y |
| P | 0 | 0 |
| U | 0 | 0 |

| | Q | Y |
|---|---|---|
| Q | P | P |
| Y | P | P |

| | J | Z | P | U |
|---|---|---|---|---|
| J | J | Z | P | U |
| Z | Z | J | P | U |
| P | P | P | 0 | 0 |
| U | U | U | 0 | 0 |

| | Q | Y |
|---|---|---|
| J | Q | Y |
| Z | Y | Q |
| P | 0 | 0 |
| U | 0 | 0 |

| | Q | Y |
|---|---|---|
| Q | P | P |
| Y | P | P |

| | J | Z | P | U |
|---|---|---|---|---|
| J | J | Z | P | U |
| Z | Z | J | P | U |
| P | P | P | 0 | 0 |
| U | U | U | 0 | 0 |

| | Q | Y |
|---|---|---|
| J | Q | Y |
| Z | Q | Y |
| P | 0 | 0 |
| U | 0 | 0 |

| | Q | Y |
|---|---|---|
| Q | P | P |
| Y | P | U |

| | J | Z | P | U |
|---|---|---|---|---|
| J | J | Z | P | U |
| Z | Z | J | P | U |
| P | P | P | 0 | 0 |
| U | U | U | 0 | 0 |

| | Q | Y |
|---|---|---|
| J | Q | Y |
| Z | Q | Y |
| P | 0 | 0 |
| U | 0 | 0 |

| | Q | Y |
|---|---|---|
| Q | P | U |
| Y | U | 0 |

| | J | Z | P | U |
|---|---|---|---|---|
| J | J | Z | P | U |
| Z | Z | J | P | U |
| P | P | P | 0 | 0 |
| U | U | U | 0 | 0 |

| | Q | Y |
|---|---|---|
| J | Q | Y |
| Z | Q | Y |
| P | 0 | 0 |
| U | 0 | 0 |

| | Q | Y |
|---|---|---|
| Q | P | U |
| Y | U | P |

| | J | Z | P | U |
|---|---|---|---|---|
| J | J | Z | P | U |
| Z | Z | J | P | U |
| P | P | P | 0 | 0 |
| U | U | U | 0 | 0 |

| | Q | Y |
|---|---|---|
| J | Q | Y |
| Z | Q | Y |
| P | 0 | 0 |
| U | 0 | 0 |

| | Q | Y |
|---|---|---|
| Q | P | U |
| Y | U | U |

| | J | Z | P | U |
|---|---|---|---|---|
| J | J | Z | P | U |
| Z | Z | J | U | P |
| P | P | U | 0 | 0 |
| U | U | P | 0 | 0 |

| | Q | Y |
|---|---|---|
| J | Q | Y |
| Z | Y | Q |
| P | 0 | 0 |
| U | 0 | 0 |

| | Q | Y |
|---|---|---|
| Q | P | U |
| Y | U | P |

| | J | Z | P | U |
|---|---|---|---|---|
| J | J | Z | P | U |
| Z | Z | J | U | P |
| P | P | U | J | Z |
| U | U | P | Z | J |

| | Q | Y |
|---|---|---|
| J | Q | Y |
| Z | Y | Q |
| P | Y | Q |
| U | Q | Y |

| | Q | Y |
|---|---|---|
| Q | $P+Z$ | $J+U$ |
| Y | $J+U$ | $P+Z$ |

| | J | Z | P | U |
|---|---|---|---|---|
| J | J | Z | P | U |
| Z | Z | J | U | P |
| P | P | U | J | Z |
| U | U | P | Z | J |

| | Q | Y |
|---|---|---|
| J | Q | Y |
| Z | Y | Q |
| P | Q | Y |
| U | Y | Q |

| | Q | Y |
|---|---|---|
| Q | $J+P$ | $U+Z$ |
| Y | $U+Z$ | $J+P$ |

Total number of resonant non-standard cases: 403.

| | $J$ | $Z$ | $P$ | $U$ |
|---|---|---|---|---|
| $J$ | $J$ | $Z$ | $P$ | $U$ |
| $Z$ | $Z$ | 0 | 0 | 0 |
| $P$ | $P$ | 0 | 0 | 0 |
| $U$ | $U$ | 0 | 0 | 0 |

| | $Q$ | $Y$ |
|---|---|---|
| $J$ | $Q$ | $Y$ |
| $Z$ | 0 | 0 |
| $P$ | 0 | 0 |
| $U$ | 0 | 0 |

| | $Q$ | $Y$ |
|---|---|---|
| $Q$ | $U$ | 0 |
| $Y$ | 0 | 0 |

| | $J$ | $Z$ | $P$ | $U$ |
|---|---|---|---|---|
| $J$ | $J$ | $Z$ | $P$ | $U$ |
| $Z$ | $Z$ | 0 | 0 | 0 |
| $P$ | $P$ | 0 | 0 | 0 |
| $U$ | $U$ | 0 | 0 | 0 |

| | $Q$ | $Y$ |
|---|---|---|
| $J$ | $Q$ | $Y$ |
| $Z$ | $Y$ | 0 |
| $P$ | 0 | 0 |
| $U$ | 0 | 0 |

| | $Q$ | $Y$ |
|---|---|---|
| $Q$ | $U$ | 0 |
| $Y$ | 0 | 0 |

| | $J$ | $Z$ | $P$ | $U$ |
|---|---|---|---|---|
| $J$ | $J$ | $Z$ | $P$ | $U$ |
| $Z$ | $Z$ | 0 | 0 | 0 |
| $P$ | $P$ | 0 | 0 | 0 |
| $U$ | $U$ | 0 | 0 | 0 |

| | $Q$ | $Y$ |
|---|---|---|
| $J$ | $Q$ | $Y$ |
| $Z$ | 0 | 0 |
| $P$ | 0 | 0 |
| $U$ | $Y$ | 0 |

| | $Q$ | $Y$ |
|---|---|---|
| $Q$ | $U$ | 0 |
| $Y$ | 0 | 0 |

| | $J$ | $Z$ | $P$ | $U$ |
|---|---|---|---|---|
| $J$ | $J$ | $Z$ | $P$ | $U$ |
| $Z$ | $Z$ | 0 | 0 | 0 |
| $P$ | $P$ | 0 | 0 | 0 |
| $U$ | $U$ | 0 | 0 | 0 |

| | $Q$ | $Y$ |
|---|---|---|
| $J$ | $Q$ | $Y$ |
| $Z$ | $Y$ | 0 |
| $P$ | 0 | 0 |
| $U$ | $Y$ | 0 |

| | $Q$ | $Y$ |
|---|---|---|
| $Q$ | $U$ | 0 |
| $Y$ | 0 | 0 |

| | $J$ | $Z$ | $P$ | $U$ |
|---|---|---|---|---|
| $J$ | $J$ | $Z$ | $P$ | $U$ |
| $Z$ | $Z$ | 0 | 0 | 0 |
| $P$ | $P$ | 0 | 0 | 0 |
| $U$ | $U$ | 0 | 0 | 0 |

| | $Q$ | $Y$ |
|---|---|---|
| $J$ | $Q$ | $Y$ |
| $Z$ | 0 | 0 |
| $P$ | $Y$ | 0 |
| $U$ | 0 | 0 |

| | $Q$ | $Y$ |
|---|---|---|
| $Q$ | $U$ | 0 |
| $Y$ | 0 | 0 |

| | $J$ | $Z$ | $P$ | $U$ |
|---|---|---|---|---|
| $J$ | $J$ | $Z$ | $P$ | $U$ |
| $Z$ | $Z$ | 0 | 0 | 0 |
| $P$ | $P$ | 0 | 0 | 0 |
| $U$ | $U$ | 0 | 0 | 0 |

| | $Q$ | $Y$ |
|---|---|---|
| $J$ | $Q$ | $Y$ |
| $Z$ | $Y$ | 0 |
| $P$ | $Y$ | 0 |
| $U$ | 0 | 0 |

| | $Q$ | $Y$ |
|---|---|---|
| $Q$ | $U$ | 0 |
| $Y$ | 0 | 0 |

| | $J$ | $Z$ | $P$ | $U$ |
|---|---|---|---|---|
| $J$ | $J$ | $Z$ | $P$ | $U$ |
| $Z$ | $Z$ | 0 | 0 | 0 |
| $P$ | $P$ | 0 | 0 | 0 |
| $U$ | $U$ | 0 | 0 | 0 |

| | $Q$ | $Y$ |
|---|---|---|
| $J$ | $Q$ | $Y$ |
| $Z$ | 0 | 0 |
| $P$ | $Y$ | 0 |
| $U$ | $Y$ | 0 |

| | $Q$ | $Y$ |
|---|---|---|
| $Q$ | $U$ | 0 |
| $Y$ | 0 | 0 |

| | $J$ | $Z$ | $P$ | $U$ |
|---|---|---|---|---|
| $J$ | $J$ | $Z$ | $P$ | $U$ |
| $Z$ | $Z$ | 0 | 0 | 0 |
| $P$ | $P$ | 0 | 0 | 0 |
| $U$ | $U$ | 0 | 0 | 0 |

| | $Q$ | $Y$ |
|---|---|---|
| $J$ | $Q$ | $Y$ |
| $Z$ | $Y$ | 0 |
| $P$ | $Y$ | 0 |
| $U$ | $Y$ | 0 |

| | $Q$ | $Y$ |
|---|---|---|
| $Q$ | $U$ | 0 |
| $Y$ | 0 | 0 |

| | $J$ | $Z$ | $P$ | $U$ |
|---|---|---|---|---|
| $J$ | $J$ | $Z$ | $P$ | $U$ |
| $Z$ | $Z$ | 0 | 0 | 0 |
| $P$ | $P$ | 0 | 0 | 0 |
| $U$ | $U$ | 0 | 0 | 0 |

| | $Q$ | $Y$ |
|---|---|---|
| $J$ | $Q$ | $Y$ |
| $Z$ | 0 | 0 |
| $P$ | 0 | 0 |
| $U$ | 0 | 0 |

| | $Q$ | $Y$ |
|---|---|---|
| $Q$ | $U$ | 0 |
| $Y$ | 0 | $P$ |

| | $J$ | $Z$ | $P$ | $U$ |
|---|---|---|---|---|
| $J$ | $J$ | $Z$ | $P$ | $U$ |
| $Z$ | $Z$ | 0 | 0 | 0 |
| $P$ | $P$ | 0 | 0 | 0 |
| $U$ | $U$ | 0 | 0 | 0 |

| | $Q$ | $Y$ |
|---|---|---|
| $J$ | $Q$ | $Y$ |
| $Z$ | 0 | 0 |
| $P$ | 0 | 0 |
| $U$ | 0 | 0 |

| | $Q$ | $Y$ |
|---|---|---|
| $Q$ | $U$ | 0 |
| $Y$ | 0 | $U$ |

| | $J$ | $Z$ | $P$ | $U$ |
|---|---|---|---|---|
| $J$ | $J$ | $Z$ | $P$ | $U$ |
| $Z$ | $Z$ | 0 | 0 | 0 |
| $P$ | $P$ | 0 | 0 | 0 |
| $U$ | $U$ | 0 | 0 | 0 |

| | $Q$ | $Y$ |
|---|---|---|
| $J$ | $Q$ | $Y$ |
| $Z$ | 0 | 0 |
| $P$ | 0 | 0 |
| $U$ | 0 | 0 |

| | $Q$ | $Y$ |
|---|---|---|
| $Q$ | $U$ | 0 |
| $Y$ | 0 | $Z$ |

| | $J$ | $Z$ | $P$ | $U$ |
|---|---|---|---|---|
| $J$ | $J$ | $Z$ | $P$ | $U$ |
| $Z$ | $Z$ | 0 | 0 | 0 |
| $P$ | $P$ | 0 | 0 | 0 |
| $U$ | $U$ | 0 | 0 | 0 |

| | $Q$ | $Y$ |
|---|---|---|
| $J$ | $Q$ | $Y$ |
| $Z$ | 0 | 0 |
| $P$ | 0 | 0 |
| $U$ | 0 | 0 |

| | $Q$ | $Y$ |
|---|---|---|
| $Q$ | $U$ | 0 |
| $Y$ | 0 | $P+Z$ |

| | $J$ | $Z$ | $P$ | $U$ |
|---|---|---|---|---|
| $J$ | $J$ | $Z$ | $P$ | $U$ |
| $Z$ | $Z$ | 0 | 0 | 0 |
| $P$ | $P$ | 0 | 0 | 0 |
| $U$ | $U$ | 0 | 0 | 0 |

| | $Q$ | $Y$ |
|---|---|---|
| $J$ | $Q$ | $Y$ |
| $Z$ | 0 | 0 |
| $P$ | 0 | 0 |
| $U$ | 0 | 0 |

| | $Q$ | $Y$ |
|---|---|---|
| $Q$ | $U$ | 0 |
| $Y$ | 0 | $U+Z$ |

| | $J$ | $Z$ | $P$ | $U$ |
|---|---|---|---|---|
| $J$ | $J$ | $Z$ | $P$ | $U$ |
| $Z$ | $Z$ | 0 | 0 | 0 |
| $P$ | $P$ | 0 | 0 | 0 |
| $U$ | $U$ | 0 | 0 | 0 |

| | $Q$ | $Y$ |
|---|---|---|
| $J$ | $Q$ | $Y$ |
| $Z$ | 0 | 0 |
| $P$ | 0 | 0 |
| $U$ | 0 | 0 |

| | $Q$ | $Y$ |
|---|---|---|
| $Q$ | $U$ | $P$ |
| $Y$ | $P$ | 0 |

| | $J$ | $Z$ | $P$ | $U$ |
|---|---|---|---|---|
| $J$ | $J$ | $Z$ | $P$ | $U$ |
| $Z$ | $Z$ | 0 | 0 | 0 |
| $P$ | $P$ | 0 | 0 | 0 |
| $U$ | $U$ | 0 | 0 | 0 |

| | $Q$ | $Y$ |
|---|---|---|
| $J$ | $Q$ | $Y$ |
| $Z$ | 0 | 0 |
| $P$ | 0 | 0 |
| $U$ | 0 | 0 |

| | $Q$ | $Y$ |
|---|---|---|
| $Q$ | $U$ | $P$ |
| $Y$ | $P$ | $P$ |

| | $J$ | $Z$ | $P$ | $U$ |
|---|---|---|---|---|
| $J$ | $J$ | $Z$ | $P$ | $U$ |
| $Z$ | $Z$ | 0 | 0 | 0 |
| $P$ | $P$ | 0 | 0 | 0 |
| $U$ | $U$ | 0 | 0 | 0 |

| | $Q$ | $Y$ |
|---|---|---|
| $J$ | $Q$ | $Y$ |
| $Z$ | 0 | 0 |
| $P$ | 0 | 0 |
| $U$ | 0 | 0 |

| | $Q$ | $Y$ |
|---|---|---|
| $Q$ | $U$ | $P$ |
| $Y$ | $P$ | $U$ |

| | $J$ | $Z$ | $P$ | $U$ |
|---|---|---|---|---|
| $J$ | $J$ | $Z$ | $P$ | $U$ |
| $Z$ | $Z$ | 0 | 0 | 0 |
| $P$ | $P$ | 0 | 0 | 0 |
| $U$ | $U$ | 0 | 0 | 0 |

| | $Q$ | $Y$ |
|---|---|---|
| $J$ | $Q$ | $Y$ |
| $Z$ | 0 | 0 |
| $P$ | 0 | 0 |
| $U$ | 0 | 0 |

| | $Q$ | $Y$ |
|---|---|---|
| $Q$ | $U$ | $P$ |
| $Y$ | $P$ | $Z$ |

| | $J$ | $Z$ | $P$ | $U$ |
|---|---|---|---|---|
| $J$ | $J$ | $Z$ | $P$ | $U$ |
| $Z$ | $Z$ | 0 | 0 | 0 |
| $P$ | $P$ | 0 | 0 | 0 |
| $U$ | $U$ | 0 | 0 | 0 |

| | $Q$ | $Y$ |
|---|---|---|
| $J$ | $Q$ | $Y$ |
| $Z$ | 0 | 0 |
| $P$ | 0 | 0 |
| $U$ | 0 | 0 |

| | $Q$ | $Y$ |
|---|---|---|
| $Q$ | $U$ | $P$ |
| $Y$ | $P$ | $P+Z$ |

| | $J$ | $Z$ | $P$ | $U$ |
|---|---|---|---|---|
| $J$ | $J$ | $Z$ | $P$ | $U$ |
| $Z$ | $Z$ | 0 | 0 | 0 |
| $P$ | $P$ | 0 | 0 | 0 |
| $U$ | $U$ | 0 | 0 | 0 |

| | $Q$ | $Y$ |
|---|---|---|
| $J$ | $Q$ | $Y$ |
| $Z$ | 0 | 0 |
| $P$ | 0 | 0 |
| $U$ | 0 | 0 |

| | $Q$ | $Y$ |
|---|---|---|
| $Q$ | $U$ | $P$ |
| $Y$ | $P$ | $U+Z$ |

| | $J$ | $Z$ | $P$ | $U$ |
|---|---|---|---|---|
| $J$ | $J$ | $Z$ | $P$ | $U$ |
| $Z$ | $Z$ | 0 | 0 | 0 |
| $P$ | $P$ | 0 | 0 | 0 |
| $U$ | $U$ | 0 | 0 | 0 |

| | $Q$ | $Y$ |
|---|---|---|
| $J$ | $Q$ | $Y$ |
| $Z$ | 0 | 0 |
| $P$ | 0 | 0 |
| $U$ | 0 | 0 |

| | $Q$ | $Y$ |
|---|---|---|
| $Q$ | $U$ | $U$ |
| $Y$ | $U$ | 0 |

| | $J$ | $Z$ | $P$ | $U$ |
|---|---|---|---|---|
| $J$ | $J$ | $Z$ | $P$ | $U$ |
| $Z$ | $Z$ | 0 | 0 | 0 |
| $P$ | $P$ | 0 | 0 | 0 |
| $U$ | $U$ | 0 | 0 | 0 |

| | $Q$ | $Y$ |
|---|---|---|
| $J$ | $Q$ | $Y$ |
| $Z$ | 0 | 0 |
| $P$ | 0 | 0 |
| $U$ | 0 | 0 |

| | $Q$ | $Y$ |
|---|---|---|
| $Q$ | $U$ | $U$ |
| $Y$ | $U$ | $P$ |

| | $J$ | $Z$ | $P$ | $U$ |
|---|---|---|---|---|
| $J$ | $J$ | $Z$ | $P$ | $U$ |
| $Z$ | $Z$ | 0 | 0 | 0 |
| $P$ | $P$ | 0 | 0 | 0 |
| $U$ | $U$ | 0 | 0 | 0 |

| | $Q$ | $Y$ |
|---|---|---|
| $J$ | $Q$ | $Y$ |
| $Z$ | 0 | 0 |
| $P$ | 0 | 0 |
| $U$ | 0 | 0 |

| | $Q$ | $Y$ |
|---|---|---|
| $Q$ | $U$ | $U$ |
| $Y$ | $U$ | $U$ |

| | $J$ | $Z$ | $P$ | $U$ |
|---|---|---|---|---|
| $J$ | $J$ | $Z$ | $P$ | $U$ |
| $Z$ | $Z$ | 0 | 0 | 0 |
| $P$ | $P$ | 0 | 0 | 0 |
| $U$ | $U$ | 0 | 0 | 0 |

| | $Q$ | $Y$ |
|---|---|---|
| $J$ | $Q$ | $Y$ |
| $Z$ | 0 | 0 |
| $P$ | 0 | 0 |
| $U$ | 0 | 0 |

| | $Q$ | $Y$ |
|---|---|---|
| $Q$ | $U$ | $U$ |
| $Y$ | $U$ | $Z$ |

| | $J$ | $Z$ | $P$ | $U$ |
|---|---|---|---|---|
| $J$ | $J$ | $Z$ | $P$ | $U$ |
| $Z$ | $Z$ | 0 | 0 | 0 |
| $P$ | $P$ | 0 | 0 | 0 |
| $U$ | $U$ | 0 | 0 | 0 |

| | $Q$ | $Y$ |
|---|---|---|
| $J$ | $Q$ | $Y$ |
| $Z$ | 0 | 0 |
| $P$ | 0 | 0 |
| $U$ | 0 | 0 |

| | $Q$ | $Y$ |
|---|---|---|
| $Q$ | $U$ | $U$ |
| $Y$ | $U$ | $P+Z$ |

| | $J$ | $Z$ | $P$ | $U$ |
|---|---|---|---|---|
| $J$ | $J$ | $Z$ | $P$ | $U$ |
| $Z$ | $Z$ | 0 | 0 | 0 |
| $P$ | $P$ | 0 | 0 | 0 |
| $U$ | $U$ | 0 | 0 | 0 |

| | $Q$ | $Y$ |
|---|---|---|
| $J$ | $Q$ | $Y$ |
| $Z$ | 0 | 0 |
| $P$ | 0 | 0 |
| $U$ | 0 | 0 |

| | $Q$ | $Y$ |
|---|---|---|
| $Q$ | $U$ | $U$ |
| $Y$ | $U$ | $U+Z$ |

| | J | Z | P | U |
|---|---|---|---|---|
| J | J | Z | P | U |
| Z | Z | 0 | 0 | 0 |
| P | P | 0 | 0 | 0 |
| U | U | 0 | 0 | 0 |

| | Q | Y |
|---|---|---|
| J | Q | Y |
| Z | 0 | 0 |
| P | 0 | 0 |
| U | 0 | 0 |

| | Q | Y |
|---|---|---|
| Q | U | Z |
| Y | Z | 0 |

| | J | Z | P | U |
|---|---|---|---|---|
| J | J | Z | P | U |
| Z | Z | 0 | 0 | 0 |
| P | P | 0 | 0 | 0 |
| U | U | 0 | 0 | 0 |

| | Q | Y |
|---|---|---|
| J | Q | Y |
| Z | 0 | 0 |
| P | 0 | 0 |
| U | 0 | 0 |

| | Q | Y |
|---|---|---|
| Q | U | $U+Z$ |
| Y | $U+Z$ | P |

| | J | Z | P | U |
|---|---|---|---|---|
| J | J | Z | P | U |
| Z | Z | 0 | 0 | 0 |
| P | P | 0 | 0 | 0 |
| U | U | 0 | 0 | 0 |

| | Q | Y |
|---|---|---|
| J | Q | Y |
| Z | 0 | 0 |
| P | 0 | 0 |
| U | 0 | 0 |

| | Q | Y |
|---|---|---|
| Q | U | Z |
| Y | Z | P |

| | J | Z | P | U |
|---|---|---|---|---|
| J | J | Z | P | U |
| Z | Z | 0 | 0 | 0 |
| P | P | 0 | 0 | 0 |
| U | U | 0 | 0 | 0 |

| | Q | Y |
|---|---|---|
| J | Q | Y |
| Z | 0 | 0 |
| P | 0 | 0 |
| U | 0 | 0 |

| | Q | Y |
|---|---|---|
| Q | U | $U+Z$ |
| Y | $U+Z$ | U |

| | J | Z | P | U |
|---|---|---|---|---|
| J | J | Z | P | U |
| Z | Z | 0 | 0 | 0 |
| P | P | 0 | 0 | 0 |
| U | U | 0 | 0 | 0 |

| | Q | Y |
|---|---|---|
| J | Q | Y |
| Z | 0 | 0 |
| P | 0 | 0 |
| U | 0 | 0 |

| | Q | Y |
|---|---|---|
| Q | U | Z |
| Y | Z | U |

| | J | Z | P | U |
|---|---|---|---|---|
| J | J | Z | P | U |
| Z | Z | 0 | 0 | 0 |
| P | P | 0 | 0 | 0 |
| U | U | 0 | 0 | 0 |

| | Q | Y |
|---|---|---|
| J | Q | Y |
| Z | 0 | 0 |
| P | 0 | 0 |
| U | 0 | 0 |

| | Q | Y |
|---|---|---|
| Q | U | $U+Z$ |
| Y | $U+Z$ | Z |

| | J | Z | P | U |
|---|---|---|---|---|
| J | J | Z | P | U |
| Z | Z | 0 | 0 | 0 |
| P | P | 0 | 0 | 0 |
| U | U | 0 | 0 | 0 |

| | Q | Y |
|---|---|---|
| J | Q | Y |
| Z | 0 | 0 |
| P | 0 | 0 |
| U | 0 | 0 |

| | Q | Y |
|---|---|---|
| Q | U | Z |
| Y | Z | Z |

| | J | Z | P | U |
|---|---|---|---|---|
| J | J | Z | P | U |
| Z | Z | 0 | 0 | 0 |
| P | P | 0 | 0 | 0 |
| U | U | 0 | 0 | 0 |

| | Q | Y |
|---|---|---|
| J | Q | Y |
| Z | 0 | 0 |
| P | 0 | 0 |
| U | 0 | 0 |

| | Q | Y |
|---|---|---|
| Q | U | $U+Z$ |
| Y | $U+Z$ | $P+Z$ |

| | J | Z | P | U |
|---|---|---|---|---|
| J | J | Z | P | U |
| Z | Z | 0 | 0 | 0 |
| P | P | 0 | 0 | 0 |
| U | U | 0 | 0 | 0 |

| | Q | Y |
|---|---|---|
| J | Q | Y |
| Z | 0 | 0 |
| P | 0 | 0 |
| U | 0 | 0 |

| | Q | Y |
|---|---|---|
| Q | U | Z |
| Y | Z | $P+Z$ |

| | J | Z | P | U |
|---|---|---|---|---|
| J | J | Z | P | U |
| Z | Z | 0 | 0 | 0 |
| P | P | 0 | 0 | 0 |
| U | U | 0 | 0 | 0 |

| | Q | Y |
|---|---|---|
| J | Q | Y |
| Z | 0 | 0 |
| P | 0 | 0 |
| U | 0 | 0 |

| | Q | Y |
|---|---|---|
| Q | U | $U+Z$ |
| Y | $U+Z$ | $U+Z$ |

| | J | Z | P | U |
|---|---|---|---|---|
| J | J | Z | P | U |
| Z | Z | 0 | 0 | 0 |
| P | P | 0 | 0 | 0 |
| U | U | 0 | 0 | 0 |

| | Q | Y |
|---|---|---|
| J | Q | Y |
| Z | 0 | 0 |
| P | 0 | 0 |
| U | 0 | 0 |

| | Q | Y |
|---|---|---|
| Q | U | Z |
| Y | Z | $U+Z$ |

| | J | Z | P | U |
|---|---|---|---|---|
| J | J | Z | P | U |
| Z | Z | 0 | 0 | 0 |
| P | P | 0 | 0 | 0 |
| U | U | 0 | 0 | 0 |

| | Q | Y |
|---|---|---|
| J | Q | Y |
| Z | 0 | 0 |
| P | 0 | 0 |
| U | 0 | 0 |

| | Q | Y |
|---|---|---|
| Q | Z | 0 |
| Y | 0 | 0 |

| | J | Z | P | U |
|---|---|---|---|---|
| J | J | Z | P | U |
| Z | Z | 0 | 0 | 0 |
| P | P | 0 | 0 | 0 |
| U | U | 0 | 0 | 0 |

| | Q | Y |
|---|---|---|
| J | Q | Y |
| Z | 0 | 0 |
| P | 0 | 0 |
| U | 0 | 0 |

| | Q | Y |
|---|---|---|
| Q | U | $P+Z$ |
| Y | $P+Z$ | 0 |

| | J | Z | P | U |
|---|---|---|---|---|
| J | J | Z | P | U |
| Z | Z | 0 | 0 | 0 |
| P | P | 0 | 0 | 0 |
| U | U | 0 | 0 | 0 |

| | Q | Y |
|---|---|---|
| J | Q | Y |
| Z | Y | 0 |
| P | 0 | 0 |
| U | 0 | 0 |

| | Q | Y |
|---|---|---|
| Q | Z | 0 |
| Y | 0 | 0 |

| | J | Z | P | U |
|---|---|---|---|---|
| J | J | Z | P | U |
| Z | Z | 0 | 0 | 0 |
| P | P | 0 | 0 | 0 |
| U | U | 0 | 0 | 0 |

| | Q | Y |
|---|---|---|
| J | Q | Y |
| Z | 0 | 0 |
| P | 0 | 0 |
| U | 0 | 0 |

| | Q | Y |
|---|---|---|
| Q | U | $P+Z$ |
| Y | $P+Z$ | P |

| | J | Z | P | U |
|---|---|---|---|---|
| J | J | Z | P | U |
| Z | Z | 0 | 0 | 0 |
| P | P | 0 | 0 | 0 |
| U | U | 0 | 0 | 0 |

| | Q | Y |
|---|---|---|
| J | Q | Y |
| Z | 0 | 0 |
| P | 0 | 0 |
| U | Y | 0 |

| | Q | Y |
|---|---|---|
| Q | Z | 0 |
| Y | 0 | 0 |

| | J | Z | P | U |
|---|---|---|---|---|
| J | J | Z | P | U |
| Z | Z | 0 | 0 | 0 |
| P | P | 0 | 0 | 0 |
| U | U | 0 | 0 | 0 |

| | Q | Y |
|---|---|---|
| J | Q | Y |
| Z | 0 | 0 |
| P | 0 | 0 |
| U | 0 | 0 |

| | Q | Y |
|---|---|---|
| Q | U | $P+Z$ |
| Y | $P+Z$ | U |

| | J | Z | P | U |
|---|---|---|---|---|
| J | J | Z | P | U |
| Z | Z | 0 | 0 | 0 |
| P | P | 0 | 0 | 0 |
| U | U | 0 | 0 | 0 |

| | Q | Y |
|---|---|---|
| J | Q | Y |
| Z | Y | 0 |
| P | 0 | 0 |
| U | Y | 0 |

| | Q | Y |
|---|---|---|
| Q | Z | 0 |
| Y | 0 | 0 |

| | J | Z | P | U |
|---|---|---|---|---|
| J | J | Z | P | U |
| Z | Z | 0 | 0 | 0 |
| P | P | 0 | 0 | 0 |
| U | U | 0 | 0 | 0 |

| | Q | Y |
|---|---|---|
| J | Q | Y |
| Z | 0 | 0 |
| P | 0 | 0 |
| U | 0 | 0 |

| | Q | Y |
|---|---|---|
| Q | U | $P+Z$ |
| Y | $P+Z$ | Z |

| | J | Z | P | U |
|---|---|---|---|---|
| J | J | Z | P | U |
| Z | Z | 0 | 0 | 0 |
| P | P | 0 | 0 | 0 |
| U | U | 0 | 0 | 0 |

| | Q | Y |
|---|---|---|
| J | Q | Y |
| Z | 0 | 0 |
| P | Y | 0 |
| U | 0 | 0 |

| | Q | Y |
|---|---|---|
| Q | Z | 0 |
| Y | 0 | 0 |

| | J | Z | P | U |
|---|---|---|---|---|
| J | J | Z | P | U |
| Z | Z | 0 | 0 | 0 |
| P | P | 0 | 0 | 0 |
| U | U | 0 | 0 | 0 |

| | Q | Y |
|---|---|---|
| J | Q | Y |
| Z | 0 | 0 |
| P | 0 | 0 |
| U | 0 | 0 |

| | Q | Y |
|---|---|---|
| Q | U | $P+Z$ |
| Y | $P+Z$ | $P+Z$ |

| | J | Z | P | U |
|---|---|---|---|---|
| J | J | Z | P | U |
| Z | Z | 0 | 0 | 0 |
| P | P | 0 | 0 | 0 |
| U | U | 0 | 0 | 0 |

| | Q | Y |
|---|---|---|
| J | Q | Y |
| Z | Y | 0 |
| P | Y | 0 |
| U | 0 | 0 |

| | Q | Y |
|---|---|---|
| Q | Z | 0 |
| Y | 0 | 0 |

| | J | Z | P | U |
|---|---|---|---|---|
| J | J | Z | P | U |
| Z | Z | 0 | 0 | 0 |
| P | P | 0 | 0 | 0 |
| U | U | 0 | 0 | 0 |

| | Q | Y |
|---|---|---|
| J | Q | Y |
| Z | 0 | 0 |
| P | 0 | 0 |
| U | 0 | 0 |

| | Q | Y |
|---|---|---|
| Q | U | $P+Z$ |
| Y | $P+Z$ | $U+Z$ |

| | J | Z | P | U |
|---|---|---|---|---|
| J | J | Z | P | U |
| Z | Z | 0 | 0 | 0 |
| P | P | 0 | 0 | 0 |
| U | U | 0 | 0 | 0 |

| | Q | Y |
|---|---|---|
| J | Q | Y |
| Z | 0 | 0 |
| P | Y | 0 |
| U | Y | 0 |

| | Q | Y |
|---|---|---|
| Q | Z | 0 |
| Y | 0 | 0 |

| | J | Z | P | U |
|---|---|---|---|---|
| J | J | Z | P | U |
| Z | Z | 0 | 0 | 0 |
| P | P | 0 | 0 | 0 |
| U | U | 0 | 0 | 0 |

| | Q | Y |
|---|---|---|
| J | Q | Y |
| Z | 0 | 0 |
| P | 0 | 0 |
| U | 0 | 0 |

| | Q | Y |
|---|---|---|
| Q | U | $U+Z$ |
| Y | $U+Z$ | 0 |

| | J | Z | P | U |
|---|---|---|---|---|
| J | J | Z | P | U |
| Z | Z | 0 | 0 | 0 |
| P | P | 0 | 0 | 0 |
| U | U | 0 | 0 | 0 |

| | Q | Y |
|---|---|---|
| J | Q | Y |
| Z | Y | 0 |
| P | Y | 0 |
| U | Y | 0 |

| | Q | Y |
|---|---|---|
| Q | Z | 0 |
| Y | 0 | 0 |

| | J | Z | P | U |
|---|---|---|---|---|
| J | J | Z | P | U |
| Z | Z | 0 | 0 | 0 |
| P | P | 0 | 0 | 0 |
| U | U | 0 | 0 | 0 |

| | Q | Y |
|---|---|---|
| J | Q | Y |
| Z | 0 | 0 |
| P | 0 | 0 |
| U | 0 | 0 |

| | Q | Y |
|---|---|---|
| Q | Z | 0 |
| Y | 0 | P |

| | J | Z | P | U |
|---|---|---|---|---|
| J | J | Z | P | U |
| Z | Z | 0 | 0 | 0 |
| P | P | 0 | 0 | 0 |
| U | U | 0 | 0 | 0 |

| | Q | Y |
|---|---|---|
| J | Q | Y |
| Z | 0 | 0 |
| P | 0 | 0 |
| U | 0 | 0 |

| | Q | Y |
|---|---|---|
| Q | Z | U |
| Y | U | U |

| | J | Z | P | U |
|---|---|---|---|---|
| J | J | Z | P | U |
| Z | Z | 0 | 0 | 0 |
| P | P | 0 | 0 | 0 |
| U | U | 0 | 0 | 0 |

| | Q | Y |
|---|---|---|
| J | Q | Y |
| Z | 0 | 0 |
| P | 0 | 0 |
| U | 0 | 0 |

| | Q | Y |
|---|---|---|
| Q | Z | 0 |
| Y | 0 | U |

| | J | Z | P | U |
|---|---|---|---|---|
| J | J | Z | P | U |
| Z | Z | 0 | 0 | 0 |
| P | P | 0 | 0 | 0 |
| U | U | 0 | 0 | 0 |

| | Q | Y |
|---|---|---|
| J | Q | Y |
| Z | 0 | 0 |
| P | 0 | 0 |
| U | 0 | 0 |

| | Q | Y |
|---|---|---|
| Q | Z | U |
| Y | U | Z |

| | J | Z | P | U |
|---|---|---|---|---|
| J | J | Z | P | U |
| Z | Z | 0 | 0 | 0 |
| P | P | 0 | 0 | 0 |
| U | U | 0 | 0 | 0 |

| | Q | Y |
|---|---|---|
| J | Q | Y |
| Z | 0 | 0 |
| P | 0 | 0 |
| U | 0 | 0 |

| | Q | Y |
|---|---|---|
| Q | Z | 0 |
| Y | 0 | Z |

| | J | Z | P | U |
|---|---|---|---|---|
| J | J | Z | P | U |
| Z | Z | 0 | 0 | 0 |
| P | P | 0 | 0 | 0 |
| U | U | 0 | 0 | 0 |

| | Q | Y |
|---|---|---|
| J | Q | Y |
| Z | 0 | 0 |
| P | 0 | 0 |
| U | 0 | 0 |

| | Q | Y |
|---|---|---|
| Q | Z | U |
| Y | U | P + Z |

| | J | Z | P | U |
|---|---|---|---|---|
| J | J | Z | P | U |
| Z | Z | 0 | 0 | 0 |
| P | P | 0 | 0 | 0 |
| U | U | 0 | 0 | 0 |

| | Q | Y |
|---|---|---|
| J | Q | Y |
| Z | 0 | 0 |
| P | 0 | 0 |
| U | 0 | 0 |

| | Q | Y |
|---|---|---|
| Q | Z | 0 |
| Y | 0 | P + Z |

| | J | Z | P | U |
|---|---|---|---|---|
| J | J | Z | P | U |
| Z | Z | 0 | 0 | 0 |
| P | P | 0 | 0 | 0 |
| U | U | 0 | 0 | 0 |

| | Q | Y |
|---|---|---|
| J | Q | Y |
| Z | 0 | 0 |
| P | 0 | 0 |
| U | 0 | 0 |

| | Q | Y |
|---|---|---|
| Q | Z | U |
| Y | U | U + Z |

| | J | Z | P | U |
|---|---|---|---|---|
| J | J | Z | P | U |
| Z | Z | 0 | 0 | 0 |
| P | P | 0 | 0 | 0 |
| U | U | 0 | 0 | 0 |

| | Q | Y |
|---|---|---|
| J | Q | Y |
| Z | 0 | 0 |
| P | 0 | 0 |
| U | 0 | 0 |

| | Q | Y |
|---|---|---|
| Q | Z | 0 |
| Y | 0 | U + Z |

| | J | Z | P | U |
|---|---|---|---|---|
| J | J | Z | P | U |
| Z | Z | 0 | 0 | 0 |
| P | P | 0 | 0 | 0 |
| U | U | 0 | 0 | 0 |

| | Q | Y |
|---|---|---|
| J | Q | Y |
| Z | 0 | 0 |
| P | 0 | 0 |
| U | 0 | 0 |

| | Q | Y |
|---|---|---|
| Q | Z | Z |
| Y | Z | 0 |

| | J | Z | P | U |
|---|---|---|---|---|
| J | J | Z | P | U |
| Z | Z | 0 | 0 | 0 |
| P | P | 0 | 0 | 0 |
| U | U | 0 | 0 | 0 |

| | Q | Y |
|---|---|---|
| J | Q | Y |
| Z | 0 | 0 |
| P | 0 | 0 |
| U | 0 | 0 |

| | Q | Y |
|---|---|---|
| Q | Z | P |
| Y | P | 0 |

| | J | Z | P | U |
|---|---|---|---|---|
| J | J | Z | P | U |
| Z | Z | 0 | 0 | 0 |
| P | P | 0 | 0 | 0 |
| U | U | 0 | 0 | 0 |

| | Q | Y |
|---|---|---|
| J | Q | Y |
| Z | 0 | 0 |
| P | 0 | 0 |
| U | 0 | 0 |

| | Q | Y |
|---|---|---|
| Q | Z | Z |
| Y | Z | P |

| | J | Z | P | U |
|---|---|---|---|---|
| J | J | Z | P | U |
| Z | Z | 0 | 0 | 0 |
| P | P | 0 | 0 | 0 |
| U | U | 0 | 0 | 0 |

| | Q | Y |
|---|---|---|
| J | Q | Y |
| Z | 0 | 0 |
| P | 0 | 0 |
| U | 0 | 0 |

| | Q | Y |
|---|---|---|
| Q | Z | P |
| Y | P | P |

| | J | Z | P | U |
|---|---|---|---|---|
| J | J | Z | P | U |
| Z | Z | 0 | 0 | 0 |
| P | P | 0 | 0 | 0 |
| U | U | 0 | 0 | 0 |

| | Q | Y |
|---|---|---|
| J | Q | Y |
| Z | 0 | 0 |
| P | 0 | 0 |
| U | 0 | 0 |

| | Q | Y |
|---|---|---|
| Q | Z | Z |
| Y | Z | U |

| | J | Z | P | U |
|---|---|---|---|---|
| J | J | Z | P | U |
| Z | Z | 0 | 0 | 0 |
| P | P | 0 | 0 | 0 |
| U | U | 0 | 0 | 0 |

| | Q | Y |
|---|---|---|
| J | Q | Y |
| Z | 0 | 0 |
| P | 0 | 0 |
| U | 0 | 0 |

| | Q | Y |
|---|---|---|
| Q | Z | P |
| Y | P | U |

| | J | Z | P | U |
|---|---|---|---|---|
| J | J | Z | P | U |
| Z | Z | 0 | 0 | 0 |
| P | P | 0 | 0 | 0 |
| U | U | 0 | 0 | 0 |

| | Q | Y |
|---|---|---|
| J | Q | Y |
| Z | 0 | 0 |
| P | 0 | 0 |
| U | 0 | 0 |

| | Q | Y |
|---|---|---|
| Q | Z | Z |
| Y | Z | Z |

| | J | Z | P | U |
|---|---|---|---|---|
| J | J | Z | P | U |
| Z | Z | 0 | 0 | 0 |
| P | P | 0 | 0 | 0 |
| U | U | 0 | 0 | 0 |

| | Q | Y |
|---|---|---|
| J | Q | Y |
| Z | 0 | 0 |
| P | 0 | 0 |
| U | 0 | 0 |

| | Q | Y |
|---|---|---|
| Q | Z | P |
| Y | P | Z |

| | J | Z | P | U |
|---|---|---|---|---|
| J | J | Z | P | U |
| Z | Z | 0 | 0 | 0 |
| P | P | 0 | 0 | 0 |
| U | U | 0 | 0 | 0 |

| | Q | Y |
|---|---|---|
| J | Q | Y |
| Z | 0 | 0 |
| P | 0 | 0 |
| U | 0 | 0 |

| | Q | Y |
|---|---|---|
| Q | Z | Z |
| Y | Z | P + Z |

| | J | Z | P | U |
|---|---|---|---|---|
| J | J | Z | P | U |
| Z | Z | 0 | 0 | 0 |
| P | P | 0 | 0 | 0 |
| U | U | 0 | 0 | 0 |

| | Q | Y |
|---|---|---|
| J | Q | Y |
| Z | 0 | 0 |
| P | 0 | 0 |
| U | 0 | 0 |

| | Q | Y |
|---|---|---|
| Q | Z | P |
| Y | P | P + Z |

| | J | Z | P | U |
|---|---|---|---|---|
| J | J | Z | P | U |
| Z | Z | 0 | 0 | 0 |
| P | P | 0 | 0 | 0 |
| U | U | 0 | 0 | 0 |

| | Q | Y |
|---|---|---|
| J | Q | Y |
| Z | 0 | 0 |
| P | 0 | 0 |
| U | 0 | 0 |

| | Q | Y |
|---|---|---|
| Q | Z | Z |
| Y | Z | U + Z |

| | J | Z | P | U |
|---|---|---|---|---|
| J | J | Z | P | U |
| Z | Z | 0 | 0 | 0 |
| P | P | 0 | 0 | 0 |
| U | U | 0 | 0 | 0 |

| | Q | Y |
|---|---|---|
| J | Q | Y |
| Z | 0 | 0 |
| P | 0 | 0 |
| U | 0 | 0 |

| | Q | Y |
|---|---|---|
| Q | Z | P |
| Y | P | U + Z |

| | J | Z | P | U |
|---|---|---|---|---|
| J | J | Z | P | U |
| Z | Z | 0 | 0 | 0 |
| P | P | 0 | 0 | 0 |
| U | U | 0 | 0 | 0 |

| | Q | Y |
|---|---|---|
| J | Q | Y |
| Z | 0 | 0 |
| P | 0 | 0 |
| U | 0 | 0 |

| | Q | Y |
|---|---|---|
| Q | Z | P + Z |
| Y | P + Z | 0 |

| | J | Z | P | U |
|---|---|---|---|---|
| J | J | Z | P | U |
| Z | Z | 0 | 0 | 0 |
| P | P | 0 | 0 | 0 |
| U | U | 0 | 0 | 0 |

| | Q | Y |
|---|---|---|
| J | Q | Y |
| Z | 0 | 0 |
| P | 0 | 0 |
| U | 0 | 0 |

| | Q | Y |
|---|---|---|
| Q | Z | U |
| Y | U | 0 |

| | J | Z | P | U |
|---|---|---|---|---|
| J | J | Z | P | U |
| Z | Z | 0 | 0 | 0 |
| P | P | 0 | 0 | 0 |
| U | U | 0 | 0 | 0 |

| | Q | Y |
|---|---|---|
| J | Q | Y |
| Z | 0 | 0 |
| P | 0 | 0 |
| U | 0 | 0 |

| | Q | Y |
|---|---|---|
| Q | Z | P + Z |
| Y | P + Z | P |

| | J | Z | P | U |
|---|---|---|---|---|
| J | J | Z | P | U |
| Z | Z | 0 | 0 | 0 |
| P | P | 0 | 0 | 0 |
| U | U | 0 | 0 | 0 |

| | Q | Y |
|---|---|---|
| J | Q | Y |
| Z | 0 | 0 |
| P | 0 | 0 |
| U | 0 | 0 |

| | Q | Y |
|---|---|---|
| Q | Z | U |
| Y | U | P |

| | J | Z | P | U |
|---|---|---|---|---|
| J | J | Z | P | U |
| Z | Z | 0 | 0 | 0 |
| P | P | 0 | 0 | 0 |
| U | U | 0 | 0 | 0 |

| | Q | Y |
|---|---|---|
| J | Q | Y |
| Z | 0 | 0 |
| P | 0 | 0 |
| U | 0 | 0 |

| | Q | Y |
|---|---|---|
| Q | Z | P + Z |
| Y | P + Z | U |

| | J | Z | P | U |
|---|---|---|---|---|
| J | J | Z | P | U |
| Z | Z | 0 | 0 | 0 |
| P | P | 0 | 0 | 0 |
| U | U | 0 | 0 | 0 |

| | Q | Y |
|---|---|---|
| J | Q | Y |
| Z | 0 | 0 |
| P | 0 | 0 |
| U | 0 | 0 |

| | Q | Y |
|---|---|---|
| Q | Z | P + Z |
| Y | P + Z | Z |

| | J | Z | P | U |
|---|---|---|---|---|
| J | J | Z | P | U |
| Z | Z | 0 | 0 | 0 |
| P | P | 0 | 0 | 0 |
| U | U | 0 | 0 | 0 |

| | Q | Y |
|---|---|---|
| J | Q | Y |
| Z | 0 | 0 |
| P | Y | 0 |
| U | 0 | 0 |

| | Q | Y |
|---|---|---|
| Q | U + Z | 0 |
| Y | 0 | 0 |

| | J | Z | P | U |
|---|---|---|---|---|
| J | J | Z | P | U |
| Z | Z | 0 | 0 | 0 |
| P | P | 0 | 0 | 0 |
| U | U | 0 | 0 | 0 |

| | Q | Y |
|---|---|---|
| J | Q | Y |
| Z | 0 | 0 |
| P | 0 | 0 |
| U | 0 | 0 |

| | Q | Y |
|---|---|---|
| Q | Z | P + Z |
| Y | P + Z | P + Z |

| | J | Z | P | U |
|---|---|---|---|---|
| J | J | Z | P | U |
| Z | Z | 0 | 0 | 0 |
| P | P | 0 | 0 | 0 |
| U | U | 0 | 0 | 0 |

| | Q | Y |
|---|---|---|
| J | Q | Y |
| Z | Y | 0 |
| P | Y | 0 |
| U | 0 | 0 |

| | Q | Y |
|---|---|---|
| Q | U + Z | 0 |
| Y | 0 | 0 |

| | J | Z | P | U |
|---|---|---|---|---|
| J | J | Z | P | U |
| Z | Z | 0 | 0 | 0 |
| P | P | 0 | 0 | 0 |
| U | U | 0 | 0 | 0 |

| | Q | Y |
|---|---|---|
| J | Q | Y |
| Z | 0 | 0 |
| P | 0 | 0 |
| U | 0 | 0 |

| | Q | Y |
|---|---|---|
| Q | Z | P + Z |
| Y | P + Z | U + Z |

| | J | Z | P | U |
|---|---|---|---|---|
| J | J | Z | P | U |
| Z | Z | 0 | 0 | 0 |
| P | P | 0 | 0 | 0 |
| U | U | 0 | 0 | 0 |

| | Q | Y |
|---|---|---|
| J | Q | Y |
| Z | 0 | 0 |
| P | Y | 0 |
| U | Y | 0 |

| | Q | Y |
|---|---|---|
| Q | U + Z | 0 |
| Y | 0 | 0 |

| | J | Z | P | U |
|---|---|---|---|---|
| J | J | Z | P | U |
| Z | Z | 0 | 0 | 0 |
| P | P | 0 | 0 | 0 |
| U | U | 0 | 0 | 0 |

| | Q | Y |
|---|---|---|
| J | Q | Y |
| Z | 0 | 0 |
| P | 0 | 0 |
| U | 0 | 0 |

| | Q | Y |
|---|---|---|
| Q | Z | U + Z |
| Y | U + Z | 0 |

| | J | Z | P | U |
|---|---|---|---|---|
| J | J | Z | P | U |
| Z | Z | 0 | 0 | 0 |
| P | P | 0 | 0 | 0 |
| U | U | 0 | 0 | 0 |

| | Q | Y |
|---|---|---|
| J | Q | Y |
| Z | Y | 0 |
| P | Y | 0 |
| U | Y | 0 |

| | Q | Y |
|---|---|---|
| Q | U + Z | 0 |
| Y | 0 | 0 |

| | J | Z | P | U |
|---|---|---|---|---|
| J | J | Z | P | U |
| Z | Z | 0 | 0 | 0 |
| P | P | 0 | 0 | 0 |
| U | U | 0 | 0 | 0 |

| | Q | Y |
|---|---|---|
| J | Q | Y |
| Z | 0 | 0 |
| P | 0 | 0 |
| U | 0 | 0 |

| | Q | Y |
|---|---|---|
| Q | Z | U + Z |
| Y | U + Z | P |

| | J | Z | P | U |
|---|---|---|---|---|
| J | J | Z | P | U |
| Z | Z | 0 | 0 | 0 |
| P | P | 0 | 0 | 0 |
| U | U | 0 | 0 | 0 |

| | Q | Y |
|---|---|---|
| J | Q | Y |
| Z | 0 | 0 |
| P | 0 | 0 |
| U | 0 | 0 |

| | Q | Y |
|---|---|---|
| Q | U + Z | 0 |
| Y | 0 | P |

| | J | Z | P | U |
|---|---|---|---|---|
| J | J | Z | P | U |
| Z | Z | 0 | 0 | 0 |
| P | P | 0 | 0 | 0 |
| U | U | 0 | 0 | 0 |

| | Q | Y |
|---|---|---|
| J | Q | Y |
| Z | 0 | 0 |
| P | 0 | 0 |
| U | 0 | 0 |

| | Q | Y |
|---|---|---|
| Q | Z | U + Z |
| Y | U + Z | U |

| | J | Z | P | U |
|---|---|---|---|---|
| J | J | Z | P | U |
| Z | Z | 0 | 0 | 0 |
| P | P | 0 | 0 | 0 |
| U | U | 0 | 0 | 0 |

| | Q | Y |
|---|---|---|
| J | Q | Y |
| Z | 0 | 0 |
| P | 0 | 0 |
| U | 0 | 0 |

| | Q | Y |
|---|---|---|
| Q | U + Z | 0 |
| Y | 0 | U |

| | J | Z | P | U |
|---|---|---|---|---|
| J | J | Z | P | U |
| Z | Z | 0 | 0 | 0 |
| P | P | 0 | 0 | 0 |
| U | U | 0 | 0 | 0 |

| | Q | Y |
|---|---|---|
| J | Q | Y |
| Z | 0 | 0 |
| P | 0 | 0 |
| U | 0 | 0 |

| | Q | Y |
|---|---|---|
| Q | Z | U + Z |
| Y | U + Z | Z |

| | J | Z | P | U |
|---|---|---|---|---|
| J | J | Z | P | U |
| Z | Z | 0 | 0 | 0 |
| P | P | 0 | 0 | 0 |
| U | U | 0 | 0 | 0 |

| | Q | Y |
|---|---|---|
| J | Q | Y |
| Z | 0 | 0 |
| P | 0 | 0 |
| U | 0 | 0 |

| | Q | Y |
|---|---|---|
| Q | U + Z | 0 |
| Y | 0 | Z |

| | J | Z | P | U |
|---|---|---|---|---|
| J | J | Z | P | U |
| Z | Z | 0 | 0 | 0 |
| P | P | 0 | 0 | 0 |
| U | U | 0 | 0 | 0 |

| | Q | Y |
|---|---|---|
| J | Q | Y |
| Z | 0 | 0 |
| P | 0 | 0 |
| U | 0 | 0 |

| | Q | Y |
|---|---|---|
| Q | Z | U + Z |
| Y | U + Z | P + Z |

| | J | Z | P | U |
|---|---|---|---|---|
| J | J | Z | P | U |
| Z | Z | 0 | 0 | 0 |
| P | P | 0 | 0 | 0 |
| U | U | 0 | 0 | 0 |

| | Q | Y |
|---|---|---|
| J | Q | Y |
| Z | 0 | 0 |
| P | 0 | 0 |
| U | 0 | 0 |

| | Q | Y |
|---|---|---|
| Q | U + Z | 0 |
| Y | 0 | P + Z |

| | J | Z | P | U |
|---|---|---|---|---|
| J | J | Z | P | U |
| Z | Z | 0 | 0 | 0 |
| P | P | 0 | 0 | 0 |
| U | U | 0 | 0 | 0 |

| | Q | Y |
|---|---|---|
| J | Q | Y |
| Z | 0 | 0 |
| P | 0 | 0 |
| U | 0 | 0 |

| | Q | Y |
|---|---|---|
| Q | Z | U + Z |
| Y | U + Z | U + Z |

| | J | Z | P | U |
|---|---|---|---|---|
| J | J | Z | P | U |
| Z | Z | 0 | 0 | 0 |
| P | P | 0 | 0 | 0 |
| U | U | 0 | 0 | 0 |

| | Q | Y |
|---|---|---|
| J | Q | Y |
| Z | 0 | 0 |
| P | 0 | 0 |
| U | 0 | 0 |

| | Q | Y |
|---|---|---|
| Q | U + Z | 0 |
| Y | 0 | U + Z |

| | J | Z | P | U |
|---|---|---|---|---|
| J | J | Z | P | U |
| Z | Z | 0 | 0 | 0 |
| P | P | 0 | 0 | 0 |
| U | U | 0 | 0 | 0 |

| | Q | Y |
|---|---|---|
| J | Q | Y |
| Z | 0 | 0 |
| P | 0 | 0 |
| U | 0 | 0 |

| | Q | Y |
|---|---|---|
| Q | U + Z | 0 |
| Y | 0 | 0 |

| | J | Z | P | U |
|---|---|---|---|---|
| J | J | Z | P | U |
| Z | Z | 0 | 0 | 0 |
| P | P | 0 | 0 | 0 |
| U | U | 0 | 0 | 0 |

| | Q | Y |
|---|---|---|
| J | Q | Y |
| Z | 0 | 0 |
| P | 0 | 0 |
| U | 0 | 0 |

| | Q | Y |
|---|---|---|
| Q | U + Z | P |
| Y | P | 0 |

| | J | Z | P | U |
|---|---|---|---|---|
| J | J | Z | P | U |
| Z | Z | 0 | 0 | 0 |
| P | P | 0 | 0 | 0 |
| U | U | 0 | 0 | 0 |

| | Q | Y |
|---|---|---|
| J | Q | Y |
| Z | Y | 0 |
| P | 0 | 0 |
| U | 0 | 0 |

| | Q | Y |
|---|---|---|
| Q | U + Z | 0 |
| Y | 0 | 0 |

| | J | Z | P | U |
|---|---|---|---|---|
| J | J | Z | P | U |
| Z | Z | 0 | 0 | 0 |
| P | P | 0 | 0 | 0 |
| U | U | 0 | 0 | 0 |

| | Q | Y |
|---|---|---|
| J | Q | Y |
| Z | 0 | 0 |
| P | 0 | 0 |
| U | 0 | 0 |

| | Q | Y |
|---|---|---|
| Q | U + Z | P |
| Y | P | P |

| | J | Z | P | U |
|---|---|---|---|---|
| J | J | Z | P | U |
| Z | Z | 0 | 0 | 0 |
| P | P | 0 | 0 | 0 |
| U | U | 0 | 0 | 0 |

| | Q | Y |
|---|---|---|
| J | Q | Y |
| Z | 0 | 0 |
| P | 0 | 0 |
| U | Y | 0 |

| | Q | Y |
|---|---|---|
| Q | U + Z | 0 |
| Y | 0 | 0 |

| | J | Z | P | U |
|---|---|---|---|---|
| J | J | Z | P | U |
| Z | Z | 0 | 0 | 0 |
| P | P | 0 | 0 | 0 |
| U | U | 0 | 0 | 0 |

| | Q | Y |
|---|---|---|
| J | Q | Y |
| Z | 0 | 0 |
| P | 0 | 0 |
| U | 0 | 0 |

| | Q | Y |
|---|---|---|
| Q | U + Z | P |
| Y | P | U |

| | J | Z | P | U |
|---|---|---|---|---|
| J | J | Z | P | U |
| Z | Z | 0 | 0 | 0 |
| P | P | 0 | 0 | 0 |
| U | U | 0 | 0 | 0 |

| | Q | Y |
|---|---|---|
| J | Q | Y |
| Z | Y | 0 |
| P | 0 | 0 |
| U | Y | 0 |

| | Q | Y |
|---|---|---|
| Q | U + Z | 0 |
| Y | 0 | 0 |

| | J | Z | P | U |
|---|---|---|---|---|
| J | J | Z | P | U |
| Z | Z | 0 | 0 | 0 |
| P | P | 0 | 0 | 0 |
| U | U | 0 | 0 | 0 |

| | Q | Y |
|---|---|---|
| J | Q | Y |
| Z | 0 | 0 |
| P | 0 | 0 |
| U | 0 | 0 |

| | Q | Y |
|---|---|---|
| Q | U + Z | P |
| Y | P | Z |

| | J | Z | P | U |
|---|---|---|---|---|
| J | J | Z | P | U |
| Z | Z | 0 | 0 | 0 |
| P | P | 0 | 0 | 0 |
| U | U | 0 | 0 | 0 |

| | Q | Y |
|---|---|---|
| J | Q | Y |
| Z | 0 | 0 |
| P | 0 | 0 |
| U | 0 | 0 |

| | Q | Y |
|---|---|---|
| Q | $U+Z$ | $P$ |
| Y | $P$ | $P+Z$ |

| | J | Z | P | U |
|---|---|---|---|---|
| J | J | Z | P | U |
| Z | Z | 0 | 0 | 0 |
| P | P | 0 | 0 | 0 |
| U | U | 0 | 0 | 0 |

| | Q | Y |
|---|---|---|
| J | Q | Y |
| Z | 0 | 0 |
| P | 0 | 0 |
| U | 0 | 0 |

| | Q | Y |
|---|---|---|
| Q | $U+Z$ | $Z$ |
| Y | $Z$ | $U+Z$ |

| | J | Z | P | U |
|---|---|---|---|---|
| J | J | Z | P | U |
| Z | Z | 0 | 0 | 0 |
| P | P | 0 | 0 | 0 |
| U | U | 0 | 0 | 0 |

| | Q | Y |
|---|---|---|
| J | Q | Y |
| Z | 0 | 0 |
| P | 0 | 0 |
| U | 0 | 0 |

| | Q | Y |
|---|---|---|
| Q | $U+Z$ | $P$ |
| Y | $P$ | $U+Z$ |

| | J | Z | P | U |
|---|---|---|---|---|
| J | J | Z | P | U |
| Z | Z | 0 | 0 | 0 |
| P | P | 0 | 0 | 0 |
| U | U | 0 | 0 | 0 |

| | Q | Y |
|---|---|---|
| J | Q | Y |
| Z | 0 | 0 |
| P | 0 | 0 |
| U | 0 | 0 |

| | Q | Y |
|---|---|---|
| Q | $U+Z$ | $P+Z$ |
| Y | $P+Z$ | 0 |

| | J | Z | P | U |
|---|---|---|---|---|
| J | J | Z | P | U |
| Z | Z | 0 | 0 | 0 |
| P | P | 0 | 0 | 0 |
| U | U | 0 | 0 | 0 |

| | Q | Y |
|---|---|---|
| J | Q | Y |
| Z | 0 | 0 |
| P | 0 | 0 |
| U | 0 | 0 |

| | Q | Y |
|---|---|---|
| Q | $U+Z$ | $U$ |
| Y | $U$ | 0 |

| | J | Z | P | U |
|---|---|---|---|---|
| J | J | Z | P | U |
| Z | Z | 0 | 0 | 0 |
| P | P | 0 | 0 | 0 |
| U | U | 0 | 0 | 0 |

| | Q | Y |
|---|---|---|
| J | Q | Y |
| Z | 0 | 0 |
| P | 0 | 0 |
| U | 0 | 0 |

| | Q | Y |
|---|---|---|
| Q | $U+Z$ | $P+Z$ |
| Y | $P+Z$ | $P$ |

| | J | Z | P | U |
|---|---|---|---|---|
| J | J | Z | P | U |
| Z | Z | 0 | 0 | 0 |
| P | P | 0 | 0 | 0 |
| U | U | 0 | 0 | 0 |

| | Q | Y |
|---|---|---|
| J | Q | Y |
| Z | 0 | 0 |
| P | 0 | 0 |
| U | 0 | 0 |

| | Q | Y |
|---|---|---|
| Q | $U+Z$ | $U$ |
| Y | $U$ | $P$ |

| | J | Z | P | U |
|---|---|---|---|---|
| J | J | Z | P | U |
| Z | Z | 0 | 0 | 0 |
| P | P | 0 | 0 | 0 |
| U | U | 0 | 0 | 0 |

| | Q | Y |
|---|---|---|
| J | Q | Y |
| Z | 0 | 0 |
| P | 0 | 0 |
| U | 0 | 0 |

| | Q | Y |
|---|---|---|
| Q | $U+Z$ | $P+Z$ |
| Y | $P+Z$ | $U$ |

| | J | Z | P | U |
|---|---|---|---|---|
| J | J | Z | P | U |
| Z | Z | 0 | 0 | 0 |
| P | P | 0 | 0 | 0 |
| U | U | 0 | 0 | 0 |

| | Q | Y |
|---|---|---|
| J | Q | Y |
| Z | 0 | 0 |
| P | 0 | 0 |
| U | 0 | 0 |

| | Q | Y |
|---|---|---|
| Q | $U+Z$ | $U$ |
| Y | $U$ | $U$ |

| | J | Z | P | U |
|---|---|---|---|---|
| J | J | Z | P | U |
| Z | Z | 0 | 0 | 0 |
| P | P | 0 | 0 | 0 |
| U | U | 0 | 0 | 0 |

| | Q | Y |
|---|---|---|
| J | Q | Y |
| Z | 0 | 0 |
| P | 0 | 0 |
| U | 0 | 0 |

| | Q | Y |
|---|---|---|
| Q | $U+Z$ | $P+Z$ |
| Y | $P+Z$ | $Z$ |

| | J | Z | P | U |
|---|---|---|---|---|
| J | J | Z | P | U |
| Z | Z | 0 | 0 | 0 |
| P | P | 0 | 0 | 0 |
| U | U | 0 | 0 | 0 |

| | Q | Y |
|---|---|---|
| J | Q | Y |
| Z | 0 | 0 |
| P | 0 | 0 |
| U | 0 | 0 |

| | Q | Y |
|---|---|---|
| Q | $U+Z$ | $U$ |
| Y | $U$ | $Z$ |

| | J | Z | P | U |
|---|---|---|---|---|
| J | J | Z | P | U |
| Z | Z | 0 | 0 | 0 |
| P | P | 0 | 0 | 0 |
| U | U | 0 | 0 | 0 |

| | Q | Y |
|---|---|---|
| J | Q | Y |
| Z | 0 | 0 |
| P | 0 | 0 |
| U | 0 | 0 |

| | Q | Y |
|---|---|---|
| Q | $U+Z$ | $P+Z$ |
| Y | $P+Z$ | $P+Z$ |

| | J | Z | P | U |
|---|---|---|---|---|
| J | J | Z | P | U |
| Z | Z | 0 | 0 | 0 |
| P | P | 0 | 0 | 0 |
| U | U | 0 | 0 | 0 |

| | Q | Y |
|---|---|---|
| J | Q | Y |
| Z | 0 | 0 |
| P | 0 | 0 |
| U | 0 | 0 |

| | Q | Y |
|---|---|---|
| Q | $U+Z$ | $U$ |
| Y | $U$ | $P+Z$ |

| | J | Z | P | U |
|---|---|---|---|---|
| J | J | Z | P | U |
| Z | Z | 0 | 0 | 0 |
| P | P | 0 | 0 | 0 |
| U | U | 0 | 0 | 0 |

| | Q | Y |
|---|---|---|
| J | Q | Y |
| Z | 0 | 0 |
| P | 0 | 0 |
| U | 0 | 0 |

| | Q | Y |
|---|---|---|
| Q | $U+Z$ | $P+Z$ |
| Y | $P+Z$ | $U+Z$ |

| | J | Z | P | U |
|---|---|---|---|---|
| J | J | Z | P | U |
| Z | Z | 0 | 0 | 0 |
| P | P | 0 | 0 | 0 |
| U | U | 0 | 0 | 0 |

| | Q | Y |
|---|---|---|
| J | Q | Y |
| Z | 0 | 0 |
| P | 0 | 0 |
| U | 0 | 0 |

| | Q | Y |
|---|---|---|
| Q | $U+Z$ | $U$ |
| Y | $U$ | $U+Z$ |

| | J | Z | P | U |
|---|---|---|---|---|
| J | J | Z | P | U |
| Z | Z | 0 | 0 | 0 |
| P | P | 0 | 0 | 0 |
| U | U | 0 | 0 | 0 |

| | Q | Y |
|---|---|---|
| J | Q | Y |
| Z | 0 | 0 |
| P | 0 | 0 |
| U | 0 | 0 |

| | Q | Y |
|---|---|---|
| Q | $U+Z$ | $U+Z$ |
| Y | $U+Z$ | 0 |

| | J | Z | P | U |
|---|---|---|---|---|
| J | J | Z | P | U |
| Z | Z | 0 | 0 | 0 |
| P | P | 0 | 0 | 0 |
| U | U | 0 | 0 | 0 |

| | Q | Y |
|---|---|---|
| J | Q | Y |
| Z | 0 | 0 |
| P | 0 | 0 |
| U | 0 | 0 |

| | Q | Y |
|---|---|---|
| Q | $U+Z$ | $Z$ |
| Y | $Z$ | 0 |

| | J | Z | P | U |
|---|---|---|---|---|
| J | J | Z | P | U |
| Z | Z | 0 | 0 | 0 |
| P | P | 0 | 0 | 0 |
| U | U | 0 | 0 | 0 |

| | Q | Y |
|---|---|---|
| J | Q | Y |
| Z | 0 | 0 |
| P | 0 | 0 |
| U | 0 | 0 |

| | Q | Y |
|---|---|---|
| Q | $U+Z$ | $U+Z$ |
| Y | $U+Z$ | $P$ |

| | J | Z | P | U |
|---|---|---|---|---|
| J | J | Z | P | U |
| Z | Z | 0 | 0 | 0 |
| P | P | 0 | 0 | 0 |
| U | U | 0 | 0 | 0 |

| | Q | Y |
|---|---|---|
| J | Q | Y |
| Z | 0 | 0 |
| P | 0 | 0 |
| U | 0 | 0 |

| | Q | Y |
|---|---|---|
| Q | $U+Z$ | $Z$ |
| Y | $Z$ | $P$ |

| | J | Z | P | U |
|---|---|---|---|---|
| J | J | Z | P | U |
| Z | Z | 0 | 0 | 0 |
| P | P | 0 | 0 | 0 |
| U | U | 0 | 0 | 0 |

| | Q | Y |
|---|---|---|
| J | Q | Y |
| Z | 0 | 0 |
| P | 0 | 0 |
| U | 0 | 0 |

| | Q | Y |
|---|---|---|
| Q | $U+Z$ | $U+Z$ |
| Y | $U+Z$ | $U$ |

| | J | Z | P | U |
|---|---|---|---|---|
| J | J | Z | P | U |
| Z | Z | 0 | 0 | 0 |
| P | P | 0 | 0 | 0 |
| U | U | 0 | 0 | 0 |

| | Q | Y |
|---|---|---|
| J | Q | Y |
| Z | 0 | 0 |
| P | 0 | 0 |
| U | 0 | 0 |

| | Q | Y |
|---|---|---|
| Q | $U+Z$ | $Z$ |
| Y | $Z$ | $U$ |

| | J | Z | P | U |
|---|---|---|---|---|
| J | J | Z | P | U |
| Z | Z | 0 | 0 | 0 |
| P | P | 0 | 0 | 0 |
| U | U | 0 | 0 | 0 |

| | Q | Y |
|---|---|---|
| J | Q | Y |
| Z | 0 | 0 |
| P | 0 | 0 |
| U | 0 | 0 |

| | Q | Y |
|---|---|---|
| Q | $U+Z$ | $U+Z$ |
| Y | $U+Z$ | $Z$ |

| | J | Z | P | U |
|---|---|---|---|---|
| J | J | Z | P | U |
| Z | Z | 0 | 0 | 0 |
| P | P | 0 | 0 | 0 |
| U | U | 0 | 0 | 0 |

| | Q | Y |
|---|---|---|
| J | Q | Y |
| Z | 0 | 0 |
| P | 0 | 0 |
| U | 0 | 0 |

| | Q | Y |
|---|---|---|
| Q | $U+Z$ | $Z$ |
| Y | $Z$ | $Z$ |

| | J | Z | P | U |
|---|---|---|---|---|
| J | J | Z | P | U |
| Z | Z | 0 | 0 | 0 |
| P | P | 0 | 0 | 0 |
| U | U | 0 | 0 | 0 |

| | Q | Y |
|---|---|---|
| J | Q | Y |
| Z | 0 | 0 |
| P | 0 | 0 |
| U | 0 | 0 |

| | Q | Y |
|---|---|---|
| Q | $U+Z$ | $U+Z$ |
| Y | $U+Z$ | $P+Z$ |

| | J | Z | P | U |
|---|---|---|---|---|
| J | J | Z | P | U |
| Z | Z | 0 | 0 | 0 |
| P | P | 0 | 0 | 0 |
| U | U | 0 | 0 | 0 |

| | Q | Y |
|---|---|---|
| J | Q | Y |
| Z | 0 | 0 |
| P | 0 | 0 |
| U | 0 | 0 |

| | Q | Y |
|---|---|---|
| Q | $U+Z$ | $Z$ |
| Y | $Z$ | $P+Z$ |

| | J | Z | P | U |
|---|---|---|---|---|
| J | J | Z | P | U |
| Z | Z | 0 | 0 | 0 |
| P | P | 0 | 0 | 0 |
| U | U | 0 | 0 | 0 |

| | Q | Y |
|---|---|---|
| J | Q | Y |
| Z | 0 | 0 |
| P | 0 | 0 |
| U | 0 | 0 |

| | Q | Y |
|---|---|---|
| Q | $U+Z$ | $U+Z$ |
| Y | $U+Z$ | $U+Z$ |

| | J | Z | P | U |
|---|---|---|---|---|
| J | J | Z | P | U |
| Z | Z | 0 | 0 | P |
| P | P | 0 | 0 | 0 |
| U | U | P | 0 | 0 |

| | Q | Y |
|---|---|---|
| J | Q | Y |
| Z | Y | 0 |
| P | 0 | 0 |
| U | 0 | 0 |

| | Q | Y |
|---|---|---|
| Q | U | P |
| Y | P | 0 |

| | J | Z | P | U |
|---|---|---|---|---|
| J | J | Z | P | U |
| Z | Z | 0 | 0 | 0 |
| P | P | 0 | 0 | 0 |
| U | U | 0 | 0 | Z |

| | Q | Y |
|---|---|---|
| J | Q | Y |
| Z | 0 | 0 |
| P | 0 | 0 |
| U | 0 | 0 |

| | Q | Y |
|---|---|---|
| Q | Z | 0 |
| Y | 0 | 0 |

| | J | Z | P | U |
|---|---|---|---|---|
| J | J | Z | P | U |
| Z | Z | 0 | 0 | P |
| P | P | 0 | 0 | 0 |
| U | U | P | 0 | 0 |

| | Q | Y |
|---|---|---|
| J | Q | Y |
| Z | 0 | 0 |
| P | 0 | 0 |
| U | Y | 0 |

| | Q | Y |
|---|---|---|
| Q | Z | P |
| Y | P | 0 |

| | J | Z | P | U |
|---|---|---|---|---|
| J | J | Z | P | U |
| Z | Z | 0 | 0 | 0 |
| P | P | 0 | 0 | 0 |
| U | U | 0 | 0 | Z |

| | Q | Y |
|---|---|---|
| J | Q | Y |
| Z | 0 | 0 |
| P | 0 | 0 |
| U | Y | 0 |

| | Q | Y |
|---|---|---|
| Q | Z | 0 |
| Y | 0 | 0 |

| | J | Z | P | U |
|---|---|---|---|---|
| J | J | Z | P | U |
| Z | Z | 0 | 0 | P |
| P | P | 0 | 0 | 0 |
| U | U | P | 0 | 0 |

| | Q | Y |
|---|---|---|
| J | Q | Y |
| Z | Y | 0 |
| P | 0 | 0 |
| U | Y | 0 |

| | Q | Y |
|---|---|---|
| Q | $U+Z$ | P |
| Y | P | 0 |

| | J | Z | P | U |
|---|---|---|---|---|
| J | J | Z | P | U |
| Z | Z | 0 | 0 | 0 |
| P | P | 0 | 0 | 0 |
| U | U | 0 | 0 | Z |

| | Q | Y |
|---|---|---|
| J | Q | Y |
| Z | 0 | 0 |
| P | Y | 0 |
| U | 0 | 0 |

| | Q | Y |
|---|---|---|
| Q | Z | 0 |
| Y | 0 | 0 |

| | J | Z | P | U |
|---|---|---|---|---|
| J | J | Z | P | U |
| Z | Z | 0 | U | 0 |
| P | P | U | 0 | 0 |
| U | U | 0 | 0 | 0 |

| | Q | Y |
|---|---|---|
| J | Q | Y |
| Z | 0 | 0 |
| P | 0 | 0 |
| U | 0 | 0 |

| | Q | Y |
|---|---|---|
| Q | U | 0 |
| Y | 0 | 0 |

| | J | Z | P | U |
|---|---|---|---|---|
| J | J | Z | P | U |
| Z | Z | 0 | 0 | 0 |
| P | P | 0 | 0 | 0 |
| U | U | 0 | 0 | Z |

| | Q | Y |
|---|---|---|
| J | Q | Y |
| Z | 0 | 0 |
| P | Y | 0 |
| U | Y | 0 |

| | Q | Y |
|---|---|---|
| Q | Z | 0 |
| Y | 0 | 0 |

| | J | Z | P | U |
|---|---|---|---|---|
| J | J | Z | P | U |
| Z | Z | 0 | U | 0 |
| P | P | U | 0 | 0 |
| U | U | 0 | 0 | 0 |

| | Q | Y |
|---|---|---|
| J | Q | Y |
| Z | Y | 0 |
| P | 0 | 0 |
| U | 0 | 0 |

| | Q | Y |
|---|---|---|
| Q | U | 0 |
| Y | 0 | 0 |

| | J | Z | P | U |
|---|---|---|---|---|
| J | J | Z | P | U |
| Z | Z | 0 | 0 | 0 |
| P | P | 0 | 0 | 0 |
| U | U | 0 | 0 | Z |

| | Q | Y |
|---|---|---|
| J | Q | Y |
| Z | 0 | 0 |
| P | 0 | 0 |
| U | 0 | 0 |

| | Q | Y |
|---|---|---|
| Q | Z | 0 |
| Y | 0 | P |

| | J | Z | P | U |
|---|---|---|---|---|
| J | J | Z | P | U |
| Z | Z | 0 | U | 0 |
| P | P | U | 0 | 0 |
| U | U | 0 | 0 | 0 |

| | Q | Y |
|---|---|---|
| J | Q | Y |
| Z | 0 | 0 |
| P | Y | 0 |
| U | 0 | 0 |

| | Q | Y |
|---|---|---|
| Q | U | 0 |
| Y | 0 | 0 |

| | J | Z | P | U |
|---|---|---|---|---|
| J | J | Z | P | U |
| Z | Z | 0 | 0 | 0 |
| P | P | 0 | 0 | 0 |
| U | U | 0 | 0 | Z |

| | Q | Y |
|---|---|---|
| J | Q | Y |
| Z | 0 | 0 |
| P | 0 | 0 |
| U | 0 | 0 |

| | Q | Y |
|---|---|---|
| Q | Z | 0 |
| Y | 0 | Z |

| | J | Z | P | U |
|---|---|---|---|---|
| J | J | Z | P | U |
| Z | Z | 0 | U | 0 |
| P | P | U | 0 | 0 |
| U | U | 0 | 0 | 0 |

| | Q | Y |
|---|---|---|
| J | Q | Y |
| Z | Y | 0 |
| P | Y | 0 |
| U | 0 | 0 |

| | Q | Y |
|---|---|---|
| Q | U | 0 |
| Y | 0 | 0 |

| | J | Z | P | U |
|---|---|---|---|---|
| J | J | Z | P | U |
| Z | Z | 0 | 0 | 0 |
| P | P | 0 | 0 | 0 |
| U | U | 0 | 0 | Z |

| | Q | Y |
|---|---|---|
| J | Q | Y |
| Z | 0 | 0 |
| P | 0 | 0 |
| U | 0 | 0 |

| | Q | Y |
|---|---|---|
| Q | Z | 0 |
| Y | 0 | $P+Z$ |

| | J | Z | P | U |
|---|---|---|---|---|
| J | J | Z | P | U |
| Z | Z | 0 | U | 0 |
| P | P | U | 0 | 0 |
| U | U | 0 | 0 | 0 |

| | Q | Y |
|---|---|---|
| J | Q | Y |
| Z | 0 | 0 |
| P | 0 | 0 |
| U | 0 | 0 |

| | Q | Y |
|---|---|---|
| Q | U | 0 |
| Y | 0 | U |

| | J | Z | P | U |
|---|---|---|---|---|
| J | J | Z | P | U |
| Z | Z | 0 | 0 | 0 |
| P | P | 0 | 0 | 0 |
| U | U | 0 | 0 | Z |

| | Q | Y |
|---|---|---|
| J | Q | Y |
| Z | 0 | 0 |
| P | 0 | 0 |
| U | 0 | 0 |

| | Q | Y |
|---|---|---|
| Q | Z | P |
| Y | P | 0 |

| | J | Z | P | U |
|---|---|---|---|---|
| J | J | Z | P | U |
| Z | Z | 0 | U | 0 |
| P | P | U | 0 | 0 |
| U | U | 0 | 0 | 0 |

| | Q | Y |
|---|---|---|
| J | Q | Y |
| Z | 0 | 0 |
| P | 0 | 0 |
| U | 0 | 0 |

| | Q | Y |
|---|---|---|
| Q | U | U |
| Y | U | 0 |

| | J | Z | P | U |
|---|---|---|---|---|
| J | J | Z | P | U |
| Z | Z | 0 | 0 | 0 |
| P | P | 0 | 0 | 0 |
| U | U | 0 | 0 | Z |

| | Q | Y |
|---|---|---|
| J | Q | Y |
| Z | 0 | 0 |
| P | 0 | 0 |
| U | 0 | 0 |

| | Q | Y |
|---|---|---|
| Q | Z | P |
| Y | P | P |

| | J | Z | P | U |
|---|---|---|---|---|
| J | J | Z | P | U |
| Z | Z | 0 | U | 0 |
| P | P | U | 0 | 0 |
| U | U | 0 | 0 | 0 |

| | Q | Y |
|---|---|---|
| J | Q | Y |
| Z | 0 | 0 |
| P | 0 | 0 |
| U | 0 | 0 |

| | Q | Y |
|---|---|---|
| Q | U | U |
| Y | U | U |

| | J | Z | P | U |
|---|---|---|---|---|
| J | J | Z | P | U |
| Z | Z | 0 | 0 | 0 |
| P | P | 0 | 0 | 0 |
| U | U | 0 | 0 | Z |

| | Q | Y |
|---|---|---|
| J | Q | Y |
| Z | 0 | 0 |
| P | 0 | 0 |
| U | 0 | 0 |

| | Q | Y |
|---|---|---|
| Q | Z | P |
| Y | P | Z |

| | J | Z | P | U |
|---|---|---|---|---|
| J | J | Z | P | U |
| Z | Z | 0 | U | 0 |
| P | P | U | 0 | 0 |
| U | U | 0 | 0 | 0 |

| | Q | Y |
|---|---|---|
| J | Q | Y |
| Z | 0 | 0 |
| P | Y | 0 |
| U | 0 | 0 |

| | Q | Y |
|---|---|---|
| Q | Z | U |
| Y | U | 0 |

| | J | Z | P | U |
|---|---|---|---|---|
| J | J | Z | P | U |
| Z | Z | 0 | 0 | 0 |
| P | P | 0 | 0 | 0 |
| U | U | 0 | 0 | Z |

| | Q | Y |
|---|---|---|
| J | Q | Y |
| Z | 0 | 0 |
| P | 0 | 0 |
| U | 0 | 0 |

| | Q | Y |
|---|---|---|
| Q | Z | P |
| Y | P | $P+Z$ |

| | J | Z | P | U |
|---|---|---|---|---|
| J | J | Z | P | U |
| Z | Z | 0 | U | 0 |
| P | P | U | 0 | 0 |
| U | U | 0 | 0 | 0 |

| | Q | Y |
|---|---|---|
| J | Q | Y |
| Z | 0 | 0 |
| P | Y | 0 |
| U | 0 | 0 |

| | Q | Y |
|---|---|---|
| Q | $U+Z$ | U |
| Y | U | 0 |

| | J | Z | P | U |
|---|---|---|---|---|
| J | J | Z | P | U |
| Z | Z | 0 | 0 | 0 |
| P | P | 0 | 0 | 0 |
| U | U | 0 | 0 | Z |

| | Q | Y |
|---|---|---|
| J | Q | Y |
| Z | 0 | 0 |
| P | 0 | 0 |
| U | 0 | 0 |

| | Q | Y |
|---|---|---|
| Q | Z | Z |
| Y | Z | 0 |

| | J | Z | P | U |
|---|---|---|---|---|
| J | J | Z | P | U |
| Z | Z | 0 | 0 | 0 |
| P | P | 0 | 0 | 0 |
| U | U | 0 | 0 | Z |

| | Q | Y |
|---|---|---|
| J | Q | Y |
| Z | 0 | 0 |
| P | 0 | 0 |
| U | Y | 0 |

| | Q | Y |
|---|---|---|
| Q | U | Z |
| Y | Z | 0 |

| | J | Z | P | U |
|---|---|---|---|---|
| J | J | Z | P | U |
| Z | Z | 0 | 0 | 0 |
| P | P | 0 | 0 | 0 |
| U | U | 0 | 0 | Z |

| | Q | Y |
|---|---|---|
| J | Q | Y |
| Z | 0 | 0 |
| P | 0 | 0 |
| U | 0 | 0 |

| | Q | Y |
|---|---|---|
| Q | Z | Z |
| Y | Z | P |

| | J | Z | P | U |
|---|---|---|---|---|
| J | J | Z | P | U |
| Z | Z | 0 | 0 | 0 |
| P | P | 0 | 0 | 0 |
| U | U | 0 | 0 | Z |

| | Q | Y |
|---|---|---|
| J | Q | Y |
| Z | 0 | 0 |
| P | 0 | 0 |
| U | 0 | 0 |

| | Q | Y |
|---|---|---|
| Q | Z | Z |
| Y | Z | Z |

| | J | Z | P | U |
|---|---|---|---|---|
| J | J | Z | P | U |
| Z | Z | 0 | 0 | 0 |
| P | P | 0 | 0 | Z |
| U | U | 0 | Z | 0 |

| | Q | Y |
|---|---|---|
| J | Q | Y |
| Z | 0 | 0 |
| P | 0 | 0 |
| U | 0 | 0 |

| | Q | Y |
|---|---|---|
| Q | Z | 0 |
| Y | 0 | Z |

| | J | Z | P | U |
|---|---|---|---|---|
| J | J | Z | P | U |
| Z | Z | 0 | 0 | 0 |
| P | P | 0 | 0 | 0 |
| U | U | 0 | 0 | Z |

| | Q | Y |
|---|---|---|
| J | Q | Y |
| Z | 0 | 0 |
| P | 0 | 0 |
| U | 0 | 0 |

| | Q | Y |
|---|---|---|
| Q | Z | Z |
| Y | Z | $P+Z$ |

| | J | Z | P | U |
|---|---|---|---|---|
| J | J | Z | P | U |
| Z | Z | 0 | 0 | 0 |
| P | P | 0 | 0 | Z |
| U | U | 0 | Z | 0 |

| | Q | Y |
|---|---|---|
| J | Q | Y |
| Z | 0 | 0 |
| P | 0 | 0 |
| U | 0 | 0 |

| | Q | Y |
|---|---|---|
| Q | Z | Z |
| Y | Z | 0 |

| | J | Z | P | U |
|---|---|---|---|---|
| J | J | Z | P | U |
| Z | Z | 0 | 0 | 0 |
| P | P | 0 | 0 | 0 |
| U | U | 0 | 0 | Z |

| | Q | Y |
|---|---|---|
| J | Q | Y |
| Z | 0 | 0 |
| P | 0 | 0 |
| U | 0 | 0 |

| | Q | Y |
|---|---|---|
| Q | Z | $P+Z$ |
| Y | $P+Z$ | 0 |

| | J | Z | P | U |
|---|---|---|---|---|
| J | J | Z | P | U |
| Z | Z | 0 | 0 | 0 |
| P | P | 0 | 0 | Z |
| U | U | 0 | Z | 0 |

| | Q | Y |
|---|---|---|
| J | Q | Y |
| Z | 0 | 0 |
| P | 0 | 0 |
| U | 0 | 0 |

| | Q | Y |
|---|---|---|
| Q | Z | Z |
| Y | Z | Z |

| | J | Z | P | U |
|---|---|---|---|---|
| J | J | Z | P | U |
| Z | Z | 0 | 0 | 0 |
| P | P | 0 | 0 | 0 |
| U | U | 0 | 0 | Z |

| | Q | Y |
|---|---|---|
| J | Q | Y |
| Z | 0 | 0 |
| P | 0 | 0 |
| U | 0 | 0 |

| | Q | Y |
|---|---|---|
| Q | Z | $P+Z$ |
| Y | $P+Z$ | P |

| | J | Z | P | U |
|---|---|---|---|---|
| J | J | Z | P | U |
| Z | Z | 0 | 0 | 0 |
| P | P | 0 | 0 | Z |
| U | U | 0 | Z | 0 |

| | Q | Y |
|---|---|---|
| J | Q | Y |
| Z | 0 | 0 |
| P | Y | 0 |
| U | 0 | 0 |

| | Q | Y |
|---|---|---|
| Q | $U+Z$ | Z |
| Y | Z | 0 |

| | J | Z | P | U |
|---|---|---|---|---|
| J | J | Z | P | U |
| Z | Z | 0 | 0 | 0 |
| P | P | 0 | 0 | 0 |
| U | U | 0 | 0 | Z |

| | Q | Y |
|---|---|---|
| J | Q | Y |
| Z | 0 | 0 |
| P | 0 | 0 |
| U | 0 | 0 |

| | Q | Y |
|---|---|---|
| Q | Z | $P+Z$ |
| Y | $P+Z$ | Z |

| | J | Z | P | U |
|---|---|---|---|---|
| J | J | Z | P | U |
| Z | Z | 0 | 0 | 0 |
| P | P | 0 | 0 | Z |
| U | U | 0 | Z | Z |

| | Q | Y |
|---|---|---|
| J | Q | Y |
| Z | 0 | 0 |
| P | Y | 0 |
| U | Y | 0 |

| | Q | Y |
|---|---|---|
| Q | U | Z |
| Y | Z | 0 |

| | J | Z | P | U |
|---|---|---|---|---|
| J | J | Z | P | U |
| Z | Z | 0 | 0 | 0 |
| P | P | 0 | 0 | 0 |
| U | U | 0 | 0 | Z |

| | Q | Y |
|---|---|---|
| J | Q | Y |
| Z | 0 | 0 |
| P | 0 | 0 |
| U | 0 | 0 |

| | Q | Y |
|---|---|---|
| Q | Z | $P+Z$ |
| Y | $P+Z$ | $P+Z$ |

| | J | Z | P | U |
|---|---|---|---|---|
| J | J | Z | P | U |
| Z | Z | 0 | 0 | 0 |
| P | P | 0 | 0 | Z |
| U | U | 0 | Z | Z |

| | Q | Y |
|---|---|---|
| J | Q | Y |
| Z | 0 | 0 |
| P | 0 | 0 |
| U | 0 | 0 |

| | Q | Y |
|---|---|---|
| Q | Z | 0 |
| Y | 0 | 0 |

| | J | Z | P | U |
|---|---|---|---|---|
| J | J | Z | P | U |
| Z | Z | 0 | 0 | 0 |
| P | P | 0 | 0 | 0 |
| U | U | 0 | 0 | Z |

| | Q | Y |
|---|---|---|
| J | Q | Y |
| Z | 0 | 0 |
| P | 0 | 0 |
| U | Y | 0 |

| | Q | Y |
|---|---|---|
| Q | $U+Z$ | Z |
| Y | Z | 0 |

| | J | Z | P | U |
|---|---|---|---|---|
| J | J | Z | P | U |
| Z | Z | 0 | 0 | 0 |
| P | P | 0 | 0 | Z |
| U | U | 0 | Z | Z |

| | Q | Y |
|---|---|---|
| J | Q | Y |
| Z | 0 | 0 |
| P | 0 | 0 |
| U | Y | 0 |

| | Q | Y |
|---|---|---|
| Q | Z | 0 |
| Y | 0 | 0 |

| | J | Z | P | U |
|---|---|---|---|---|
| J | J | Z | P | U |
| Z | Z | 0 | 0 | P |
| P | P | 0 | 0 | 0 |
| U | U | P | 0 | Z |

| | Q | Y |
|---|---|---|
| J | Q | Y |
| Z | 0 | 0 |
| P | 0 | 0 |
| U | Y | 0 |

| | Q | Y |
|---|---|---|
| Q | Z | P |
| Y | P | 0 |

| | J | Z | P | U |
|---|---|---|---|---|
| J | J | Z | P | U |
| Z | Z | 0 | 0 | 0 |
| P | P | 0 | 0 | Z |
| U | U | 0 | Z | Z |

| | Q | Y |
|---|---|---|
| J | Q | Y |
| Z | 0 | 0 |
| P | Y | 0 |
| U | 0 | 0 |

| | Q | Y |
|---|---|---|
| Q | Z | 0 |
| Y | 0 | 0 |

| | J | Z | P | U |
|---|---|---|---|---|
| J | J | Z | P | U |
| Z | Z | 0 | 0 | 0 |
| P | P | 0 | 0 | Z |
| U | U | 0 | Z | 0 |

| | Q | Y |
|---|---|---|
| J | Q | Y |
| Z | 0 | 0 |
| P | Y | 0 |
| U | 0 | 0 |

| | Q | Y |
|---|---|---|
| Q | U | Z |
| Y | Z | 0 |

| | J | Z | P | U |
|---|---|---|---|---|
| J | J | Z | P | U |
| Z | Z | 0 | 0 | 0 |
| P | P | 0 | 0 | Z |
| U | U | 0 | Z | Z |

| | Q | Y |
|---|---|---|
| J | Q | Y |
| Z | 0 | 0 |
| P | Y | 0 |
| U | Y | 0 |

| | Q | Y |
|---|---|---|
| Q | Z | 0 |
| Y | 0 | 0 |

| | J | Z | P | U |
|---|---|---|---|---|
| J | J | Z | P | U |
| Z | Z | 0 | 0 | 0 |
| P | P | 0 | 0 | Z |
| U | U | 0 | Z | 0 |

| | Q | Y |
|---|---|---|
| J | Q | Y |
| Z | 0 | 0 |
| P | 0 | 0 |
| U | 0 | 0 |

| | Q | Y |
|---|---|---|
| Q | Z | 0 |
| Y | 0 | 0 |

| | J | Z | P | U |
|---|---|---|---|---|
| J | J | Z | P | U |
| Z | Z | 0 | 0 | 0 |
| P | P | 0 | 0 | Z |
| U | U | 0 | Z | Z |

| | Q | Y |
|---|---|---|
| J | Q | Y |
| Z | 0 | 0 |
| P | 0 | 0 |
| U | 0 | 0 |

| | Q | Y |
|---|---|---|
| Q | Z | 0 |
| Y | 0 | Z |

| | J | Z | P | U |
|---|---|---|---|---|
| J | J | Z | P | U |
| Z | Z | 0 | 0 | 0 |
| P | P | 0 | 0 | Z |
| U | U | 0 | Z | 0 |

| | Q | Y |
|---|---|---|
| J | Q | Y |
| Z | 0 | 0 |
| P | 0 | 0 |
| U | Y | 0 |

| | Q | Y |
|---|---|---|
| Q | Z | 0 |
| Y | 0 | 0 |

| | J | Z | P | U |
|---|---|---|---|---|
| J | J | Z | P | U |
| Z | Z | 0 | 0 | 0 |
| P | P | 0 | 0 | Z |
| U | U | 0 | Z | Z |

| | Q | Y |
|---|---|---|
| J | Q | Y |
| Z | 0 | 0 |
| P | 0 | 0 |
| U | 0 | 0 |

| | Q | Y |
|---|---|---|
| Q | Z | Z |
| Y | Z | 0 |

| | J | Z | P | U |
|---|---|---|---|---|
| J | J | Z | P | U |
| Z | Z | 0 | 0 | 0 |
| P | P | 0 | 0 | Z |
| U | U | 0 | Z | 0 |

| | Q | Y |
|---|---|---|
| J | Q | Y |
| Z | 0 | 0 |
| P | Y | 0 |
| U | 0 | 0 |

| | Q | Y |
|---|---|---|
| Q | Z | 0 |
| Y | 0 | 0 |

| | J | Z | P | U |
|---|---|---|---|---|
| J | J | Z | P | U |
| Z | Z | 0 | 0 | 0 |
| P | P | 0 | 0 | Z |
| U | U | 0 | Z | Z |

| | Q | Y |
|---|---|---|
| J | Q | Y |
| Z | 0 | 0 |
| P | 0 | 0 |
| U | 0 | 0 |

| | Q | Y |
|---|---|---|
| Q | Z | Z |
| Y | Z | Z |

| | J | Z | P | U |
|---|---|---|---|---|
| J | J | Z | P | U |
| Z | Z | 0 | 0 | 0 |
| P | P | 0 | 0 | Z |
| U | U | 0 | Z | 0 |

| | Q | Y |
|---|---|---|
| J | Q | Y |
| Z | 0 | 0 |
| P | Y | 0 |
| U | Y | 0 |

| | Q | Y |
|---|---|---|
| Q | Z | 0 |
| Y | 0 | 0 |

| | J | Z | P | U |
|---|---|---|---|---|
| J | J | Z | P | U |
| Z | Z | 0 | 0 | 0 |
| P | P | 0 | 0 | Z |
| U | U | 0 | Z | Z |

| | Q | Y |
|---|---|---|
| J | Q | Y |
| Z | 0 | 0 |
| P | Y | 0 |
| U | Y | 0 |

| | Q | Y |
|---|---|---|
| Q | $U+Z$ | Z |
| Y | Z | 0 |

| | J | Z | P | U |
|---|---|---|---|---|
| J | J | Z | P | U |
| Z | Z | 0 | 0 | P |
| P | P | 0 | 0 | Z |
| U | U | P | Z | J |

| | Q | Y |
|---|---|---|
| J | Q | Y |
| Z | 0 | 0 |
| P | 0 | 0 |
| U | Y | Q |

| | Q | Y |
|---|---|---|
| Q | Z | P |
| Y | P | Z |

| | J | Z | P | U |
|---|---|---|---|---|
| J | J | Z | P | U |
| Z | Z | 0 | 0 | 0 |
| P | P | 0 | Z | 0 |
| U | U | 0 | 0 | 0 |

| | Q | Y |
|---|---|---|
| J | Q | Y |
| Z | 0 | 0 |
| P | 0 | 0 |
| U | 0 | 0 |

| | Q | Y |
|---|---|---|
| Q | U | Z |
| Y | Z | 0 |

| | J | Z | P | U |
|---|---|---|---|---|
| J | J | Z | P | U |
| Z | Z | 0 | 0 | P |
| P | P | 0 | 0 | Z |
| U | U | P | Z | J |

| | Q | Y |
|---|---|---|
| J | Q | Y |
| Z | Y | 0 |
| P | Y | 0 |
| U | Q | Y |

| | Q | Y |
|---|---|---|
| Q | $J+U$ | $P+Z$ |
| Y | $P+Z$ | 0 |

| | J | Z | P | U |
|---|---|---|---|---|
| J | J | Z | P | U |
| Z | Z | 0 | 0 | 0 |
| P | P | 0 | Z | 0 |
| U | U | 0 | 0 | 0 |

| | Q | Y |
|---|---|---|
| J | Q | Y |
| Z | 0 | 0 |
| P | 0 | 0 |
| U | 0 | 0 |

| | Q | Y |
|---|---|---|
| Q | U | Z |
| Y | Z | U |

| | J | Z | P | U |
|---|---|---|---|---|
| J | J | Z | P | U |
| Z | Z | 0 | 0 | 0 |
| P | P | 0 | Z | 0 |
| U | U | 0 | 0 | 0 |

| | Q | Y |
|---|---|---|
| J | Q | Y |
| Z | 0 | 0 |
| P | 0 | 0 |
| U | 0 | 0 |

| | Q | Y |
|---|---|---|
| Q | U | 0 |
| Y | 0 | 0 |

| | J | Z | P | U |
|---|---|---|---|---|
| J | J | Z | P | U |
| Z | Z | 0 | 0 | 0 |
| P | P | 0 | Z | 0 |
| U | U | 0 | 0 | 0 |

| | Q | Y |
|---|---|---|
| J | Q | Y |
| Z | 0 | 0 |
| P | 0 | 0 |
| U | 0 | 0 |

| | Q | Y |
|---|---|---|
| Q | U | Z |
| Y | Z | Z |

| | J | Z | P | U |
|---|---|---|---|---|
| J | J | Z | P | U |
| Z | Z | 0 | 0 | 0 |
| P | P | 0 | Z | 0 |
| U | U | 0 | 0 | 0 |

| | Q | Y |
|---|---|---|
| J | Q | Y |
| Z | 0 | 0 |
| P | 0 | 0 |
| U | Y | 0 |

| | Q | Y |
|---|---|---|
| Q | U | 0 |
| Y | 0 | 0 |

| | J | Z | P | U |
|---|---|---|---|---|
| J | J | Z | P | U |
| Z | Z | 0 | 0 | 0 |
| P | P | 0 | Z | 0 |
| U | U | 0 | 0 | 0 |

| | Q | Y |
|---|---|---|
| J | Q | Y |
| Z | 0 | 0 |
| P | 0 | 0 |
| U | 0 | 0 |

| | Q | Y |
|---|---|---|
| Q | U | Z |
| Y | Z | $U+Z$ |

| | J | Z | P | U |
|---|---|---|---|---|
| J | J | Z | P | U |
| Z | Z | 0 | 0 | 0 |
| P | P | 0 | Z | 0 |
| U | U | 0 | 0 | 0 |

| | Q | Y |
|---|---|---|
| J | Q | Y |
| Z | 0 | 0 |
| P | Y | 0 |
| U | 0 | 0 |

| | Q | Y |
|---|---|---|
| Q | U | 0 |
| Y | 0 | 0 |

| | J | Z | P | U |
|---|---|---|---|---|
| J | J | Z | P | U |
| Z | Z | 0 | 0 | 0 |
| P | P | 0 | Z | 0 |
| U | U | 0 | 0 | 0 |

| | Q | Y |
|---|---|---|
| J | Q | Y |
| Z | 0 | 0 |
| P | 0 | 0 |
| U | 0 | 0 |

| | Q | Y |
|---|---|---|
| Q | U | $U+Z$ |
| Y | $U+Z$ | 0 |

| | J | Z | P | U |
|---|---|---|---|---|
| J | J | Z | P | U |
| Z | Z | 0 | 0 | 0 |
| P | P | 0 | Z | 0 |
| U | U | 0 | 0 | 0 |

| | Q | Y |
|---|---|---|
| J | Q | Y |
| Z | 0 | 0 |
| P | Y | 0 |
| U | Y | 0 |

| | Q | Y |
|---|---|---|
| Q | U | 0 |
| Y | 0 | 0 |

| | J | Z | P | U |
|---|---|---|---|---|
| J | J | Z | P | U |
| Z | Z | 0 | 0 | 0 |
| P | P | 0 | Z | 0 |
| U | U | 0 | 0 | 0 |

| | Q | Y |
|---|---|---|
| J | Q | Y |
| Z | 0 | 0 |
| P | 0 | 0 |
| U | 0 | 0 |

| | Q | Y |
|---|---|---|
| Q | U | $U+Z$ |
| Y | $U+Z$ | U |

| | J | Z | P | U |
|---|---|---|---|---|
| J | J | Z | P | U |
| Z | Z | 0 | 0 | 0 |
| P | P | 0 | Z | 0 |
| U | U | 0 | 0 | 0 |

| | Q | Y |
|---|---|---|
| J | Q | Y |
| Z | 0 | 0 |
| P | 0 | 0 |
| U | 0 | 0 |

| | Q | Y |
|---|---|---|
| Q | U | 0 |
| Y | 0 | U |

| | J | Z | P | U |
|---|---|---|---|---|
| J | J | Z | P | U |
| Z | Z | 0 | 0 | 0 |
| P | P | 0 | Z | 0 |
| U | U | 0 | 0 | 0 |

| | Q | Y |
|---|---|---|
| J | Q | Y |
| Z | 0 | 0 |
| P | 0 | 0 |
| U | 0 | 0 |

| | Q | Y |
|---|---|---|
| Q | U | $U+Z$ |
| Y | $U+Z$ | Z |

| | J | Z | P | U |
|---|---|---|---|---|
| J | J | Z | P | U |
| Z | Z | 0 | 0 | 0 |
| P | P | 0 | Z | 0 |
| U | U | 0 | 0 | 0 |

| | Q | Y |
|---|---|---|
| J | Q | Y |
| Z | 0 | 0 |
| P | 0 | 0 |
| U | 0 | 0 |

| | Q | Y |
|---|---|---|
| Q | U | 0 |
| Y | 0 | Z |

| | J | Z | P | U |
|---|---|---|---|---|
| J | J | Z | P | U |
| Z | Z | 0 | 0 | 0 |
| P | P | 0 | Z | 0 |
| U | U | 0 | 0 | 0 |

| | Q | Y |
|---|---|---|
| J | Q | Y |
| Z | 0 | 0 |
| P | 0 | 0 |
| U | 0 | 0 |

| | Q | Y |
|---|---|---|
| Q | U | $U+Z$ |
| Y | $U+Z$ | $U+Z$ |

| | J | Z | P | U |
|---|---|---|---|---|
| J | J | Z | P | U |
| Z | Z | 0 | 0 | 0 |
| P | P | 0 | Z | 0 |
| U | U | 0 | 0 | 0 |

| | Q | Y |
|---|---|---|
| J | Q | Y |
| Z | 0 | 0 |
| P | 0 | 0 |
| U | 0 | 0 |

| | Q | Y |
|---|---|---|
| Q | U | 0 |
| Y | 0 | $U+Z$ |

| | J | Z | P | U |
|---|---|---|---|---|
| J | J | Z | P | U |
| Z | Z | 0 | 0 | 0 |
| P | P | 0 | Z | 0 |
| U | U | 0 | 0 | 0 |

| | Q | Y |
|---|---|---|
| J | Q | Y |
| Z | 0 | 0 |
| P | 0 | 0 |
| U | 0 | 0 |

| | Q | Y |
|---|---|---|
| Q | Z | 0 |
| Y | 0 | 0 |

| | J | Z | P | U |
|---|---|---|---|---|
| J | J | Z | P | U |
| Z | Z | 0 | 0 | 0 |
| P | P | 0 | Z | 0 |
| U | U | 0 | 0 | 0 |

| | Q | Y |
|---|---|---|
| J | Q | Y |
| Z | 0 | 0 |
| P | 0 | 0 |
| U | 0 | 0 |

| | Q | Y |
|---|---|---|
| Q | U | U |
| Y | U | 0 |

| | J | Z | P | U |
|---|---|---|---|---|
| J | J | Z | P | U |
| Z | Z | 0 | 0 | 0 |
| P | P | 0 | Z | 0 |
| U | U | 0 | 0 | 0 |

| | Q | Y |
|---|---|---|
| J | Q | Y |
| Z | 0 | 0 |
| P | 0 | 0 |
| U | Y | 0 |

| | Q | Y |
|---|---|---|
| Q | Z | 0 |
| Y | 0 | 0 |

| | J | Z | P | U |
|---|---|---|---|---|
| J | J | Z | P | U |
| Z | Z | 0 | 0 | 0 |
| P | P | 0 | Z | 0 |
| U | U | 0 | 0 | 0 |

| | Q | Y |
|---|---|---|
| J | Q | Y |
| Z | 0 | 0 |
| P | 0 | 0 |
| U | 0 | 0 |

| | Q | Y |
|---|---|---|
| Q | U | U |
| Y | U | U |

| | J | Z | P | U |
|---|---|---|---|---|
| J | J | Z | P | U |
| Z | Z | 0 | 0 | 0 |
| P | P | 0 | Z | 0 |
| U | U | 0 | 0 | 0 |

| | Q | Y |
|---|---|---|
| J | Q | Y |
| Z | 0 | 0 |
| P | Y | 0 |
| U | 0 | 0 |

| | Q | Y |
|---|---|---|
| Q | Z | 0 |
| Y | 0 | 0 |

| | J | Z | P | U |
|---|---|---|---|---|
| J | J | Z | P | U |
| Z | Z | 0 | 0 | 0 |
| P | P | 0 | Z | 0 |
| U | U | 0 | 0 | 0 |

| | Q | Y |
|---|---|---|
| J | Q | Y |
| Z | 0 | 0 |
| P | 0 | 0 |
| U | 0 | 0 |

| | Q | Y |
|---|---|---|
| Q | U | U |
| Y | U | Z |

| | J | Z | P | U |
|---|---|---|---|---|
| J | J | Z | P | U |
| Z | Z | 0 | 0 | 0 |
| P | P | 0 | Z | 0 |
| U | U | 0 | 0 | 0 |

| | Q | Y |
|---|---|---|
| J | Q | Y |
| Z | 0 | 0 |
| P | Y | 0 |
| U | Y | 0 |

| | Q | Y |
|---|---|---|
| Q | Z | 0 |
| Y | 0 | 0 |

| | J | Z | P | U |
|---|---|---|---|---|
| J | J | Z | P | U |
| Z | Z | 0 | 0 | 0 |
| P | P | 0 | Z | 0 |
| U | U | 0 | 0 | 0 |

| | Q | Y |
|---|---|---|
| J | Q | Y |
| Z | 0 | 0 |
| P | 0 | 0 |
| U | 0 | 0 |

| | Q | Y |
|---|---|---|
| Q | U | U |
| Y | U | $U+Z$ |

| | J | Z | P | U |
|---|---|---|---|---|
| J | J | Z | P | U |
| Z | Z | 0 | 0 | 0 |
| P | P | 0 | Z | 0 |
| U | U | 0 | 0 | 0 |

| | Q | Y |
|---|---|---|
| J | Q | Y |
| Z | 0 | 0 |
| P | 0 | 0 |
| U | 0 | 0 |

| | Q | Y |
|---|---|---|
| Q | Z | 0 |
| Y | 0 | U |

| | $J$ | $Z$ | $P$ | $U$ |
|---|---|---|---|---|
| $J$ | $J$ | $Z$ | $P$ | $U$ |
| $Z$ | $Z$ | 0 | 0 | 0 |
| $P$ | $P$ | 0 | $Z$ | 0 |
| $U$ | $U$ | 0 | 0 | 0 |

| | $Q$ | $Y$ |
|---|---|---|
| $J$ | $Q$ | $Y$ |
| $Z$ | 0 | 0 |
| $P$ | 0 | 0 |
| $U$ | 0 | 0 |

| | $Q$ | $Y$ |
|---|---|---|
| $Q$ | $Z$ | 0 |
| $Y$ | 0 | $Z$ |

| | $J$ | $Z$ | $P$ | $U$ |
|---|---|---|---|---|
| $J$ | $J$ | $Z$ | $P$ | $U$ |
| $Z$ | $Z$ | 0 | 0 | 0 |
| $P$ | $P$ | 0 | $Z$ | 0 |
| $U$ | $U$ | 0 | 0 | 0 |

| | $Q$ | $Y$ |
|---|---|---|
| $J$ | $Q$ | $Y$ |
| $Z$ | 0 | 0 |
| $P$ | 0 | 0 |
| $U$ | 0 | 0 |

| | $Q$ | $Y$ |
|---|---|---|
| $Q$ | $Z$ | $U+Z$ |
| $Y$ | $U+Z$ | $U+Z$ |

| | $J$ | $Z$ | $P$ | $U$ |
|---|---|---|---|---|
| $J$ | $J$ | $Z$ | $P$ | $U$ |
| $Z$ | $Z$ | 0 | 0 | 0 |
| $P$ | $P$ | 0 | $Z$ | 0 |
| $U$ | $U$ | 0 | 0 | 0 |

| | $Q$ | $Y$ |
|---|---|---|
| $J$ | $Q$ | $Y$ |
| $Z$ | 0 | 0 |
| $P$ | 0 | 0 |
| $U$ | 0 | 0 |

| | $Q$ | $Y$ |
|---|---|---|
| $Q$ | $Z$ | 0 |
| $Y$ | 0 | $U+Z$ |

| | $J$ | $Z$ | $P$ | $U$ |
|---|---|---|---|---|
| $J$ | $J$ | $Z$ | $P$ | $U$ |
| $Z$ | $Z$ | 0 | 0 | 0 |
| $P$ | $P$ | 0 | $Z$ | 0 |
| $U$ | $U$ | 0 | 0 | 0 |

| | $Q$ | $Y$ |
|---|---|---|
| $J$ | $Q$ | $Y$ |
| $Z$ | 0 | 0 |
| $P$ | 0 | 0 |
| $U$ | 0 | 0 |

| | $Q$ | $Y$ |
|---|---|---|
| $Q$ | $U+Z$ | 0 |
| $Y$ | 0 | 0 |

| | $J$ | $Z$ | $P$ | $U$ |
|---|---|---|---|---|
| $J$ | $J$ | $Z$ | $P$ | $U$ |
| $Z$ | $Z$ | 0 | 0 | 0 |
| $P$ | $P$ | 0 | $Z$ | 0 |
| $U$ | $U$ | 0 | 0 | 0 |

| | $Q$ | $Y$ |
|---|---|---|
| $J$ | $Q$ | $Y$ |
| $Z$ | 0 | 0 |
| $P$ | 0 | 0 |
| $U$ | 0 | 0 |

| | $Q$ | $Y$ |
|---|---|---|
| $Q$ | $Z$ | $U$ |
| $Y$ | $U$ | 0 |

| | $J$ | $Z$ | $P$ | $U$ |
|---|---|---|---|---|
| $J$ | $J$ | $Z$ | $P$ | $U$ |
| $Z$ | $Z$ | 0 | 0 | 0 |
| $P$ | $P$ | 0 | $Z$ | 0 |
| $U$ | $U$ | 0 | 0 | 0 |

| | $Q$ | $Y$ |
|---|---|---|
| $J$ | $Q$ | $Y$ |
| $Z$ | 0 | 0 |
| $P$ | 0 | 0 |
| $U$ | $Y$ | 0 |

| | $Q$ | $Y$ |
|---|---|---|
| $Q$ | $U+Z$ | 0 |
| $Y$ | 0 | 0 |

| | $J$ | $Z$ | $P$ | $U$ |
|---|---|---|---|---|
| $J$ | $J$ | $Z$ | $P$ | $U$ |
| $Z$ | $Z$ | 0 | 0 | 0 |
| $P$ | $P$ | 0 | $Z$ | 0 |
| $U$ | $U$ | 0 | 0 | 0 |

| | $Q$ | $Y$ |
|---|---|---|
| $J$ | $Q$ | $Y$ |
| $Z$ | 0 | 0 |
| $P$ | 0 | 0 |
| $U$ | 0 | 0 |

| | $Q$ | $Y$ |
|---|---|---|
| $Q$ | $Z$ | $U$ |
| $Y$ | $U$ | $U$ |

| | $J$ | $Z$ | $P$ | $U$ |
|---|---|---|---|---|
| $J$ | $J$ | $Z$ | $P$ | $U$ |
| $Z$ | $Z$ | 0 | 0 | 0 |
| $P$ | $P$ | 0 | $Z$ | 0 |
| $U$ | $U$ | 0 | 0 | 0 |

| | $Q$ | $Y$ |
|---|---|---|
| $J$ | $Q$ | $Y$ |
| $Z$ | 0 | 0 |
| $P$ | $Y$ | 0 |
| $U$ | 0 | 0 |

| | $Q$ | $Y$ |
|---|---|---|
| $Q$ | $U+Z$ | 0 |
| $Y$ | 0 | 0 |

| | $J$ | $Z$ | $P$ | $U$ |
|---|---|---|---|---|
| $J$ | $J$ | $Z$ | $P$ | $U$ |
| $Z$ | $Z$ | 0 | 0 | 0 |
| $P$ | $P$ | 0 | $Z$ | 0 |
| $U$ | $U$ | 0 | 0 | 0 |

| | $Q$ | $Y$ |
|---|---|---|
| $J$ | $Q$ | $Y$ |
| $Z$ | 0 | 0 |
| $P$ | 0 | 0 |
| $U$ | 0 | 0 |

| | $Q$ | $Y$ |
|---|---|---|
| $Q$ | $Z$ | $U$ |
| $Y$ | $U$ | $Z$ |

| | $J$ | $Z$ | $P$ | $U$ |
|---|---|---|---|---|
| $J$ | $J$ | $Z$ | $P$ | $U$ |
| $Z$ | $Z$ | 0 | 0 | 0 |
| $P$ | $P$ | 0 | $Z$ | 0 |
| $U$ | $U$ | 0 | 0 | 0 |

| | $Q$ | $Y$ |
|---|---|---|
| $J$ | $Q$ | $Y$ |
| $Z$ | 0 | 0 |
| $P$ | $Y$ | 0 |
| $U$ | $Y$ | 0 |

| | $Q$ | $Y$ |
|---|---|---|
| $Q$ | $U+Z$ | 0 |
| $Y$ | 0 | 0 |

| | $J$ | $Z$ | $P$ | $U$ |
|---|---|---|---|---|
| $J$ | $J$ | $Z$ | $P$ | $U$ |
| $Z$ | $Z$ | 0 | 0 | 0 |
| $P$ | $P$ | 0 | $Z$ | 0 |
| $U$ | $U$ | 0 | 0 | 0 |

| | $Q$ | $Y$ |
|---|---|---|
| $J$ | $Q$ | $Y$ |
| $Z$ | 0 | 0 |
| $P$ | 0 | 0 |
| $U$ | 0 | 0 |

| | $Q$ | $Y$ |
|---|---|---|
| $Q$ | $Z$ | $U$ |
| $Y$ | $U$ | $U+Z$ |

| | $J$ | $Z$ | $P$ | $U$ |
|---|---|---|---|---|
| $J$ | $J$ | $Z$ | $P$ | $U$ |
| $Z$ | $Z$ | 0 | 0 | 0 |
| $P$ | $P$ | 0 | $Z$ | 0 |
| $U$ | $U$ | 0 | 0 | 0 |

| | $Q$ | $Y$ |
|---|---|---|
| $J$ | $Q$ | $Y$ |
| $Z$ | 0 | 0 |
| $P$ | 0 | 0 |
| $U$ | 0 | 0 |

| | $Q$ | $Y$ |
|---|---|---|
| $Q$ | $U+Z$ | 0 |
| $Y$ | 0 | $U$ |

| | $J$ | $Z$ | $P$ | $U$ |
|---|---|---|---|---|
| $J$ | $J$ | $Z$ | $P$ | $U$ |
| $Z$ | $Z$ | 0 | 0 | 0 |
| $P$ | $P$ | 0 | $Z$ | 0 |
| $U$ | $U$ | 0 | 0 | 0 |

| | $Q$ | $Y$ |
|---|---|---|
| $J$ | $Q$ | $Y$ |
| $Z$ | 0 | 0 |
| $P$ | 0 | 0 |
| $U$ | 0 | 0 |

| | $Q$ | $Y$ |
|---|---|---|
| $Q$ | $Z$ | $Z$ |
| $Y$ | $Z$ | 0 |

| | $J$ | $Z$ | $P$ | $U$ |
|---|---|---|---|---|
| $J$ | $J$ | $Z$ | $P$ | $U$ |
| $Z$ | $Z$ | 0 | 0 | 0 |
| $P$ | $P$ | 0 | $Z$ | 0 |
| $U$ | $U$ | 0 | 0 | 0 |

| | $Q$ | $Y$ |
|---|---|---|
| $J$ | $Q$ | $Y$ |
| $Z$ | 0 | 0 |
| $P$ | 0 | 0 |
| $U$ | 0 | 0 |

| | $Q$ | $Y$ |
|---|---|---|
| $Q$ | $U+Z$ | 0 |
| $Y$ | 0 | $Z$ |

| | $J$ | $Z$ | $P$ | $U$ |
|---|---|---|---|---|
| $J$ | $J$ | $Z$ | $P$ | $U$ |
| $Z$ | $Z$ | 0 | 0 | 0 |
| $P$ | $P$ | 0 | $Z$ | 0 |
| $U$ | $U$ | 0 | 0 | 0 |

| | $Q$ | $Y$ |
|---|---|---|
| $J$ | $Q$ | $Y$ |
| $Z$ | 0 | 0 |
| $P$ | 0 | 0 |
| $U$ | 0 | 0 |

| | $Q$ | $Y$ |
|---|---|---|
| $Q$ | $Z$ | $Z$ |
| $Y$ | $Z$ | $U$ |

| | $J$ | $Z$ | $P$ | $U$ |
|---|---|---|---|---|
| $J$ | $J$ | $Z$ | $P$ | $U$ |
| $Z$ | $Z$ | 0 | 0 | 0 |
| $P$ | $P$ | 0 | $Z$ | 0 |
| $U$ | $U$ | 0 | 0 | 0 |

| | $Q$ | $Y$ |
|---|---|---|
| $J$ | $Q$ | $Y$ |
| $Z$ | 0 | 0 |
| $P$ | 0 | 0 |
| $U$ | 0 | 0 |

| | $Q$ | $Y$ |
|---|---|---|
| $Q$ | $U+Z$ | 0 |
| $Y$ | 0 | $U+Z$ |

| | $J$ | $Z$ | $P$ | $U$ |
|---|---|---|---|---|
| $J$ | $J$ | $Z$ | $P$ | $U$ |
| $Z$ | $Z$ | 0 | 0 | 0 |
| $P$ | $P$ | 0 | $Z$ | 0 |
| $U$ | $U$ | 0 | 0 | 0 |

| | $Q$ | $Y$ |
|---|---|---|
| $J$ | $Q$ | $Y$ |
| $Z$ | 0 | 0 |
| $P$ | 0 | 0 |
| $U$ | 0 | 0 |

| | $Q$ | $Y$ |
|---|---|---|
| $Q$ | $Z$ | $Z$ |
| $Y$ | $Z$ | $Z$ |

| | $J$ | $Z$ | $P$ | $U$ |
|---|---|---|---|---|
| $J$ | $J$ | $Z$ | $P$ | $U$ |
| $Z$ | $Z$ | 0 | 0 | 0 |
| $P$ | $P$ | 0 | $Z$ | 0 |
| $U$ | $U$ | 0 | 0 | 0 |

| | $Q$ | $Y$ |
|---|---|---|
| $J$ | $Q$ | $Y$ |
| $Z$ | 0 | 0 |
| $P$ | 0 | 0 |
| $U$ | 0 | 0 |

| | $Q$ | $Y$ |
|---|---|---|
| $Q$ | $U+Z$ | $U$ |
| $Y$ | $U$ | 0 |

| | $J$ | $Z$ | $P$ | $U$ |
|---|---|---|---|---|
| $J$ | $J$ | $Z$ | $P$ | $U$ |
| $Z$ | $Z$ | 0 | 0 | 0 |
| $P$ | $P$ | 0 | $Z$ | 0 |
| $U$ | $U$ | 0 | 0 | 0 |

| | $Q$ | $Y$ |
|---|---|---|
| $J$ | $Q$ | $Y$ |
| $Z$ | 0 | 0 |
| $P$ | 0 | 0 |
| $U$ | 0 | 0 |

| | $Q$ | $Y$ |
|---|---|---|
| $Q$ | $Z$ | $Z$ |
| $Y$ | $Z$ | $U+Z$ |

| | $J$ | $Z$ | $P$ | $U$ |
|---|---|---|---|---|
| $J$ | $J$ | $Z$ | $P$ | $U$ |
| $Z$ | $Z$ | 0 | 0 | 0 |
| $P$ | $P$ | 0 | $Z$ | 0 |
| $U$ | $U$ | 0 | 0 | 0 |

| | $Q$ | $Y$ |
|---|---|---|
| $J$ | $Q$ | $Y$ |
| $Z$ | 0 | 0 |
| $P$ | 0 | 0 |
| $U$ | 0 | 0 |

| | $Q$ | $Y$ |
|---|---|---|
| $Q$ | $U+Z$ | $U$ |
| $Y$ | $U$ | $U$ |

| | $J$ | $Z$ | $P$ | $U$ |
|---|---|---|---|---|
| $J$ | $J$ | $Z$ | $P$ | $U$ |
| $Z$ | $Z$ | 0 | 0 | 0 |
| $P$ | $P$ | 0 | $Z$ | 0 |
| $U$ | $U$ | 0 | 0 | 0 |

| | $Q$ | $Y$ |
|---|---|---|
| $J$ | $Q$ | $Y$ |
| $Z$ | 0 | 0 |
| $P$ | 0 | 0 |
| $U$ | 0 | 0 |

| | $Q$ | $Y$ |
|---|---|---|
| $Q$ | $Z$ | $U+Z$ |
| $Y$ | $U+Z$ | 0 |

| | $J$ | $Z$ | $P$ | $U$ |
|---|---|---|---|---|
| $J$ | $J$ | $Z$ | $P$ | $U$ |
| $Z$ | $Z$ | 0 | 0 | 0 |
| $P$ | $P$ | 0 | $Z$ | 0 |
| $U$ | $U$ | 0 | 0 | 0 |

| | $Q$ | $Y$ |
|---|---|---|
| $J$ | $Q$ | $Y$ |
| $Z$ | 0 | 0 |
| $P$ | 0 | 0 |
| $U$ | 0 | 0 |

| | $Q$ | $Y$ |
|---|---|---|
| $Q$ | $U+Z$ | $U$ |
| $Y$ | $U$ | $Z$ |

| | $J$ | $Z$ | $P$ | $U$ |
|---|---|---|---|---|
| $J$ | $J$ | $Z$ | $P$ | $U$ |
| $Z$ | $Z$ | 0 | 0 | 0 |
| $P$ | $P$ | 0 | $Z$ | 0 |
| $U$ | $U$ | 0 | 0 | 0 |

| | $Q$ | $Y$ |
|---|---|---|
| $J$ | $Q$ | $Y$ |
| $Z$ | 0 | 0 |
| $P$ | 0 | 0 |
| $U$ | 0 | 0 |

| | $Q$ | $Y$ |
|---|---|---|
| $Q$ | $Z$ | $U+Z$ |
| $Y$ | $U+Z$ | $U$ |

| | $J$ | $Z$ | $P$ | $U$ |
|---|---|---|---|---|
| $J$ | $J$ | $Z$ | $P$ | $U$ |
| $Z$ | $Z$ | 0 | 0 | 0 |
| $P$ | $P$ | 0 | $Z$ | 0 |
| $U$ | $U$ | 0 | 0 | 0 |

| | $Q$ | $Y$ |
|---|---|---|
| $J$ | $Q$ | $Y$ |
| $Z$ | 0 | 0 |
| $P$ | 0 | 0 |
| $U$ | 0 | 0 |

| | $Q$ | $Y$ |
|---|---|---|
| $Q$ | $U+Z$ | $U$ |
| $Y$ | $U$ | $U+Z$ |

| | $J$ | $Z$ | $P$ | $U$ |
|---|---|---|---|---|
| $J$ | $J$ | $Z$ | $P$ | $U$ |
| $Z$ | $Z$ | 0 | 0 | 0 |
| $P$ | $P$ | 0 | $Z$ | 0 |
| $U$ | $U$ | 0 | 0 | 0 |

| | $Q$ | $Y$ |
|---|---|---|
| $J$ | $Q$ | $Y$ |
| $Z$ | 0 | 0 |
| $P$ | 0 | 0 |
| $U$ | 0 | 0 |

| | $Q$ | $Y$ |
|---|---|---|
| $Q$ | $Z$ | $U+Z$ |
| $Y$ | $U+Z$ | $Z$ |

| | $J$ | $Z$ | $P$ | $U$ |
|---|---|---|---|---|
| $J$ | $J$ | $Z$ | $P$ | $U$ |
| $Z$ | $Z$ | 0 | 0 | 0 |
| $P$ | $P$ | 0 | $Z$ | 0 |
| $U$ | $U$ | 0 | 0 | 0 |

| | $Q$ | $Y$ |
|---|---|---|
| $J$ | $Q$ | $Y$ |
| $Z$ | 0 | 0 |
| $P$ | 0 | 0 |
| $U$ | 0 | 0 |

| | $Q$ | $Y$ |
|---|---|---|
| $Q$ | $U+Z$ | $Z$ |
| $Y$ | $Z$ | 0 |

| | J | Z | P | U |
|---|---|---|---|---|
| J | J | Z | P | U |
| Z | Z | 0 | 0 | 0 |
| P | P | 0 | Z | 0 |
| U | U | 0 | 0 | 0 |

| | Q | Y |
|---|---|---|
| J | Q | Y |
| Z | 0 | 0 |
| P | 0 | 0 |
| U | 0 | 0 |

| | Q | Y |
|---|---|---|
| Q | U + Z | Z |
| Y | Z | U |

| | J | Z | P | U |
|---|---|---|---|---|
| J | J | Z | P | U |
| Z | Z | 0 | U | 0 |
| P | P | U | Z | 0 |
| U | U | 0 | 0 | 0 |

| | Q | Y |
|---|---|---|
| J | Q | Y |
| Z | 0 | 0 |
| P | Y | 0 |
| U | 0 | 0 |

| | Q | Y |
|---|---|---|
| Q | U + Z | U |
| Y | U | 0 |

| | J | Z | P | U |
|---|---|---|---|---|
| J | J | Z | P | U |
| Z | Z | 0 | 0 | 0 |
| P | P | 0 | Z | 0 |
| U | U | 0 | 0 | 0 |

| | Q | Y |
|---|---|---|
| J | Q | Y |
| Z | 0 | 0 |
| P | 0 | 0 |
| U | 0 | 0 |

| | Q | Y |
|---|---|---|
| Q | U + Z | Z |
| Y | Z | Z |

| | J | Z | P | U |
|---|---|---|---|---|
| J | J | Z | P | U |
| Z | Z | 0 | 0 | 0 |
| P | P | 0 | Z | 0 |
| U | U | 0 | 0 | Z |

| | Q | Y |
|---|---|---|
| J | Q | Y |
| Z | 0 | 0 |
| P | 0 | 0 |
| U | Y | 0 |

| | Q | Y |
|---|---|---|
| Q | U | Z |
| Y | Z | 0 |

| | J | Z | P | U |
|---|---|---|---|---|
| J | J | Z | P | U |
| Z | Z | 0 | 0 | 0 |
| P | P | 0 | Z | 0 |
| U | U | 0 | 0 | 0 |

| | Q | Y |
|---|---|---|
| J | Q | Y |
| Z | 0 | 0 |
| P | 0 | 0 |
| U | 0 | 0 |

| | Q | Y |
|---|---|---|
| Q | U + Z | Z |
| Y | Z | U + Z |

| | J | Z | P | U |
|---|---|---|---|---|
| J | J | Z | P | U |
| Z | Z | 0 | 0 | 0 |
| P | P | 0 | Z | 0 |
| U | U | 0 | 0 | Z |

| | Q | Y |
|---|---|---|
| J | Q | Y |
| Z | 0 | 0 |
| P | 0 | 0 |
| U | 0 | 0 |

| | Q | Y |
|---|---|---|
| Q | Z | 0 |
| Y | 0 | 0 |

| | J | Z | P | U |
|---|---|---|---|---|
| J | J | Z | P | U |
| Z | Z | 0 | 0 | 0 |
| P | P | 0 | Z | 0 |
| U | U | 0 | 0 | 0 |

| | Q | Y |
|---|---|---|
| J | Q | Y |
| Z | 0 | 0 |
| P | 0 | 0 |
| U | 0 | 0 |

| | Q | Y |
|---|---|---|
| Q | U + Z | U + Z |
| Y | U + Z | 0 |

| | J | Z | P | U |
|---|---|---|---|---|
| J | J | Z | P | U |
| Z | Z | 0 | 0 | 0 |
| P | P | 0 | Z | 0 |
| U | U | 0 | 0 | Z |

| | Q | Y |
|---|---|---|
| J | Q | Y |
| Z | 0 | 0 |
| P | 0 | 0 |
| U | Y | 0 |

| | Q | Y |
|---|---|---|
| Q | Z | 0 |
| Y | 0 | 0 |

| | J | Z | P | U |
|---|---|---|---|---|
| J | J | Z | P | U |
| Z | Z | 0 | 0 | 0 |
| P | P | 0 | Z | 0 |
| U | U | 0 | 0 | 0 |

| | Q | Y |
|---|---|---|
| J | Q | Y |
| Z | 0 | 0 |
| P | 0 | 0 |
| U | 0 | 0 |

| | Q | Y |
|---|---|---|
| Q | U + Z | U + Z |
| Y | U + Z | U |

| | J | Z | P | U |
|---|---|---|---|---|
| J | J | Z | P | U |
| Z | Z | 0 | 0 | 0 |
| P | P | 0 | Z | 0 |
| U | U | 0 | 0 | Z |

| | Q | Y |
|---|---|---|
| J | Q | Y |
| Z | 0 | 0 |
| P | Y | 0 |
| U | 0 | 0 |

| | Q | Y |
|---|---|---|
| Q | Z | 0 |
| Y | 0 | 0 |

| | J | Z | P | U |
|---|---|---|---|---|
| J | J | Z | P | U |
| Z | Z | 0 | 0 | 0 |
| P | P | 0 | Z | 0 |
| U | U | 0 | 0 | 0 |

| | Q | Y |
|---|---|---|
| J | Q | Y |
| Z | 0 | 0 |
| P | 0 | 0 |
| U | 0 | 0 |

| | Q | Y |
|---|---|---|
| Q | U + Z | U + Z |
| Y | U + Z | Z |

| | J | Z | P | U |
|---|---|---|---|---|
| J | J | Z | P | U |
| Z | Z | 0 | 0 | 0 |
| P | P | 0 | Z | 0 |
| U | U | 0 | 0 | Z |

| | Q | Y |
|---|---|---|
| J | Q | Y |
| Z | 0 | 0 |
| P | Y | 0 |
| U | Y | 0 |

| | Q | Y |
|---|---|---|
| Q | Z | 0 |
| Y | 0 | 0 |

| | J | Z | P | U |
|---|---|---|---|---|
| J | J | Z | P | U |
| Z | Z | 0 | 0 | 0 |
| P | P | 0 | Z | 0 |
| U | U | 0 | 0 | 0 |

| | Q | Y |
|---|---|---|
| J | Q | Y |
| Z | 0 | 0 |
| P | 0 | 0 |
| U | 0 | 0 |

| | Q | Y |
|---|---|---|
| Q | U + Z | U + Z |
| Y | U + Z | U + Z |

| | J | Z | P | U |
|---|---|---|---|---|
| J | J | Z | P | U |
| Z | Z | 0 | 0 | 0 |
| P | P | 0 | Z | 0 |
| U | U | 0 | 0 | Z |

| | Q | Y |
|---|---|---|
| J | Q | Y |
| Z | 0 | 0 |
| P | 0 | 0 |
| U | 0 | 0 |

| | Q | Y |
|---|---|---|
| Q | Z | 0 |
| Y | 0 | Z |

| | J | Z | P | U |
|---|---|---|---|---|
| J | J | Z | P | U |
| Z | Z | 0 | U | 0 |
| P | P | U | Z | 0 |
| U | U | 0 | 0 | 0 |

| | Q | Y |
|---|---|---|
| J | Q | Y |
| Z | 0 | 0 |
| P | 0 | 0 |
| U | 0 | 0 |

| | Q | Y |
|---|---|---|
| Q | U | 0 |
| Y | 0 | 0 |

| | J | Z | P | U |
|---|---|---|---|---|
| J | J | Z | P | U |
| Z | Z | 0 | 0 | 0 |
| P | P | 0 | Z | 0 |
| U | U | 0 | 0 | Z |

| | Q | Y |
|---|---|---|
| J | Q | Y |
| Z | 0 | 0 |
| P | 0 | 0 |
| U | 0 | 0 |

| | Q | Y |
|---|---|---|
| Q | Z | Z |
| Y | Z | 0 |

| | J | Z | P | U |
|---|---|---|---|---|
| J | J | Z | P | U |
| Z | Z | 0 | U | 0 |
| P | P | U | Z | 0 |
| U | U | 0 | 0 | 0 |

| | Q | Y |
|---|---|---|
| J | Q | Y |
| Z | 0 | 0 |
| P | Y | 0 |
| U | 0 | 0 |

| | Q | Y |
|---|---|---|
| Q | U | 0 |
| Y | 0 | 0 |

| | J | Z | P | U |
|---|---|---|---|---|
| J | J | Z | P | U |
| Z | Z | 0 | 0 | 0 |
| P | P | 0 | Z | 0 |
| U | U | 0 | 0 | Z |

| | Q | Y |
|---|---|---|
| J | Q | Y |
| Z | 0 | 0 |
| P | 0 | 0 |
| U | 0 | 0 |

| | Q | Y |
|---|---|---|
| Q | Z | Z |
| Y | Z | Z |

| | J | Z | P | U |
|---|---|---|---|---|
| J | J | Z | P | U |
| Z | Z | 0 | U | 0 |
| P | P | U | Z | 0 |
| U | U | 0 | 0 | 0 |

| | Q | Y |
|---|---|---|
| J | Q | Y |
| Z | 0 | 0 |
| P | 0 | 0 |
| U | 0 | 0 |

| | Q | Y |
|---|---|---|
| Q | U | 0 |
| Y | 0 | U |

| | J | Z | P | U |
|---|---|---|---|---|
| J | J | Z | P | U |
| Z | Z | 0 | 0 | 0 |
| P | P | 0 | Z | 0 |
| U | U | 0 | 0 | Z |

| | Q | Y |
|---|---|---|
| J | Q | Y |
| Z | 0 | 0 |
| P | 0 | 0 |
| U | Y | 0 |

| | Q | Y |
|---|---|---|
| Q | U + Z | Z |
| Y | Z | 0 |

| | J | Z | P | U |
|---|---|---|---|---|
| J | J | Z | P | U |
| Z | Z | 0 | U | 0 |
| P | P | U | Z | 0 |
| U | U | 0 | 0 | 0 |

| | Q | Y |
|---|---|---|
| J | Q | Y |
| Z | 0 | 0 |
| P | 0 | 0 |
| U | 0 | 0 |

| | Q | Y |
|---|---|---|
| Q | U | U |
| Y | U | 0 |

| | J | Z | P | U |
|---|---|---|---|---|
| J | J | Z | P | U |
| Z | Z | 0 | 0 | 0 |
| P | P | 0 | Z | Z |
| U | U | 0 | Z | 0 |

| | Q | Y |
|---|---|---|
| J | Q | Y |
| Z | 0 | 0 |
| P | Y | 0 |
| U | 0 | 0 |

| | Q | Y |
|---|---|---|
| Q | U | Z |
| Y | Z | 0 |

| | J | Z | P | U |
|---|---|---|---|---|
| J | J | Z | P | U |
| Z | Z | 0 | U | 0 |
| P | P | U | Z | 0 |
| U | U | 0 | 0 | 0 |

| | Q | Y |
|---|---|---|
| J | Q | Y |
| Z | 0 | 0 |
| P | 0 | 0 |
| U | 0 | 0 |

| | Q | Y |
|---|---|---|
| Q | U | U |
| Y | U | U |

| | J | Z | P | U |
|---|---|---|---|---|
| J | J | Z | P | U |
| Z | Z | 0 | 0 | 0 |
| P | P | 0 | Z | Z |
| U | U | 0 | Z | 0 |

| | Q | Y |
|---|---|---|
| J | Q | Y |
| Z | 0 | 0 |
| P | 0 | 0 |
| U | 0 | 0 |

| | Q | Y |
|---|---|---|
| Q | Z | 0 |
| Y | 0 | 0 |

| | J | Z | P | U |
|---|---|---|---|---|
| J | J | Z | P | U |
| Z | Z | 0 | U | 0 |
| P | P | U | Z | 0 |
| U | U | 0 | 0 | 0 |

| | Q | Y |
|---|---|---|
| J | Q | Y |
| Z | 0 | 0 |
| P | Y | 0 |
| U | 0 | 0 |

| | Q | Y |
|---|---|---|
| Q | Z | U |
| Y | U | 0 |

| | J | Z | P | U |
|---|---|---|---|---|
| J | J | Z | P | U |
| Z | Z | 0 | 0 | 0 |
| P | P | 0 | Z | Z |
| U | U | 0 | Z | 0 |

| | Q | Y |
|---|---|---|
| J | Q | Y |
| Z | 0 | 0 |
| P | 0 | 0 |
| U | Y | 0 |

| | Q | Y |
|---|---|---|
| Q | Z | 0 |
| Y | 0 | 0 |

| | J | Z | P | U |
|---|---|---|---|---|
| J | J | Z | P | U |
| Z | Z | 0 | 0 | 0 |
| P | P | 0 | Z | Z |
| U | U | 0 | Z | 0 |

| | Q | Y |
|---|---|---|
| J | Q | Y |
| Z | 0 | 0 |
| P | Y | 0 |
| U | 0 | 0 |

| | Q | Y |
|---|---|---|
| Q | Z | 0 |
| Y | 0 | 0 |

| | J | Z | P | U |
|---|---|---|---|---|
| J | J | Z | P | U |
| Z | Z | 0 | 0 | 0 |
| P | P | 0 | Z | Z |
| U | U | 0 | Z | 0 |

| | Q | Y |
|---|---|---|
| J | Q | Y |
| Z | 0 | 0 |
| P | Y | 0 |
| U | Y | 0 |

| | Q | Y |
|---|---|---|
| Q | Z | 0 |
| Y | 0 | 0 |

| | J | Z | P | U |
|---|---|---|---|---|
| J | J | Z | P | U |
| Z | Z | 0 | 0 | 0 |
| P | P | 0 | Z | Z |
| U | U | 0 | Z | 0 |

| | Q | Y |
|---|---|---|
| J | Q | Y |
| Z | 0 | 0 |
| P | 0 | 0 |
| U | 0 | 0 |

| | Q | Y |
|---|---|---|
| Q | Z | 0 |
| Y | 0 | Z |

| | J | Z | P | U |
|---|---|---|---|---|
| J | J | Z | P | U |
| Z | Z | 0 | 0 | 0 |
| P | P | 0 | Z | Z |
| U | U | 0 | Z | 0 |

| | Q | Y |
|---|---|---|
| J | Q | Y |
| Z | 0 | 0 |
| P | 0 | 0 |
| U | 0 | 0 |

| | Q | Y |
|---|---|---|
| Q | Z | Z |
| Y | Z | 0 |

| | J | Z | P | U |
|---|---|---|---|---|
| J | J | Z | P | U |
| Z | Z | 0 | 0 | 0 |
| P | P | 0 | Z | Z |
| U | U | 0 | Z | 0 |

| | Q | Y |
|---|---|---|
| J | Q | Y |
| Z | 0 | 0 |
| P | 0 | 0 |
| U | 0 | 0 |

| | Q | Y |
|---|---|---|
| Q | Z | Z |
| Y | Z | Z |

| | J | Z | P | U |
|---|---|---|---|---|
| J | J | Z | P | U |
| Z | Z | 0 | 0 | 0 |
| P | P | 0 | Z | Z |
| U | U | 0 | Z | 0 |

| | Q | Y |
|---|---|---|
| J | Q | Y |
| Z | 0 | 0 |
| P | Y | 0 |
| U | 0 | 0 |

| | Q | Y |
|---|---|---|
| Q | U+Z | Z |
| Y | Z | 0 |

| | J | Z | P | U |
|---|---|---|---|---|
| J | J | Z | P | U |
| Z | Z | 0 | 0 | 0 |
| P | P | 0 | Z | Z |
| U | U | 0 | Z | Z |

| | Q | Y |
|---|---|---|
| J | Q | Y |
| Z | 0 | 0 |
| P | Y | 0 |
| U | Y | 0 |

| | Q | Y |
|---|---|---|
| Q | U | Z |
| Y | Z | 0 |

| | J | Z | P | U |
|---|---|---|---|---|
| J | J | Z | P | U |
| Z | Z | 0 | 0 | 0 |
| P | P | 0 | Z | Z |
| U | U | 0 | Z | Z |

| | Q | Y |
|---|---|---|
| J | Q | Y |
| Z | 0 | 0 |
| P | 0 | 0 |
| U | 0 | 0 |

| | Q | Y |
|---|---|---|
| Q | Z | 0 |
| Y | 0 | 0 |

| | J | Z | P | U |
|---|---|---|---|---|
| J | J | Z | P | U |
| Z | Z | 0 | 0 | 0 |
| P | P | 0 | Z | Z |
| U | U | 0 | Z | Z |

| | Q | Y |
|---|---|---|
| J | Q | Y |
| Z | 0 | 0 |
| P | 0 | 0 |
| U | Y | 0 |

| | Q | Y |
|---|---|---|
| Q | Z | 0 |
| Y | 0 | 0 |

| | J | Z | P | U |
|---|---|---|---|---|
| J | J | Z | P | U |
| Z | Z | 0 | 0 | 0 |
| P | P | 0 | Z | Z |
| U | U | 0 | Z | Z |

| | Q | Y |
|---|---|---|
| J | Q | Y |
| Z | 0 | 0 |
| P | Y | 0 |
| U | 0 | 0 |

| | Q | Y |
|---|---|---|
| Q | Z | 0 |
| Y | 0 | 0 |

| | J | Z | P | U |
|---|---|---|---|---|
| J | J | Z | P | U |
| Z | Z | 0 | 0 | 0 |
| P | P | 0 | Z | Z |
| U | U | 0 | Z | Z |

| | Q | Y |
|---|---|---|
| J | Q | Y |
| Z | 0 | 0 |
| P | Y | 0 |
| U | Y | 0 |

| | Q | Y |
|---|---|---|
| Q | Z | 0 |
| Y | 0 | 0 |

| | J | Z | P | U |
|---|---|---|---|---|
| J | J | Z | P | U |
| Z | Z | 0 | 0 | 0 |
| P | P | 0 | Z | Z |
| U | U | 0 | Z | Z |

| | Q | Y |
|---|---|---|
| J | Q | Y |
| Z | 0 | 0 |
| P | 0 | 0 |
| U | 0 | 0 |

| | Q | Y |
|---|---|---|
| Q | Z | 0 |
| Y | 0 | Z |

| | J | Z | P | U |
|---|---|---|---|---|
| J | J | Z | P | U |
| Z | Z | 0 | 0 | 0 |
| P | P | 0 | Z | Z |
| U | U | 0 | Z | Z |

| | Q | Y |
|---|---|---|
| J | Q | Y |
| Z | 0 | 0 |
| P | 0 | 0 |
| U | 0 | 0 |

| | Q | Y |
|---|---|---|
| Q | Z | Z |
| Y | Z | 0 |

| | J | Z | P | U |
|---|---|---|---|---|
| J | J | Z | P | U |
| Z | Z | 0 | 0 | 0 |
| P | P | 0 | Z | Z |
| U | U | 0 | Z | Z |

| | Q | Y |
|---|---|---|
| J | Q | Y |
| Z | 0 | 0 |
| P | 0 | 0 |
| U | 0 | 0 |

| | Q | Y |
|---|---|---|
| Q | Z | Z |
| Y | Z | Z |

| | J | Z | P | U |
|---|---|---|---|---|
| J | J | Z | P | U |
| Z | Z | 0 | 0 | 0 |
| P | P | 0 | Z | Z |
| U | U | 0 | Z | Z |

| | Q | Y |
|---|---|---|
| J | Q | Y |
| Z | 0 | 0 |
| P | Y | 0 |
| U | Y | 0 |

| | Q | Y |
|---|---|---|
| Q | U+Z | Z |
| Y | Z | 0 |

| | J | Z | P | U |
|---|---|---|---|---|
| J | J | Z | P | U |
| Z | Z | 0 | U | 0 |
| P | P | U | J | Z |
| U | U | 0 | Z | 0 |

| | Q | Y |
|---|---|---|
| J | Q | Y |
| Z | 0 | 0 |
| P | Y | Q |
| U | 0 | 0 |

| | Q | Y |
|---|---|---|
| Q | U | Z |
| Y | Z | U |

| | J | Z | P | U |
|---|---|---|---|---|
| J | J | Z | P | U |
| Z | Z | 0 | U | 0 |
| P | P | U | J | Z |
| U | U | 0 | Z | 0 |

| | Q | Y |
|---|---|---|
| J | Q | Y |
| Z | 0 | 0 |
| P | Y | Q |
| U | 0 | 0 |

| | Q | Y |
|---|---|---|
| Q | Z | U |
| Y | U | Z |

| | J | Z | P | U |
|---|---|---|---|---|
| J | J | Z | P | U |
| Z | Z | 0 | U | 0 |
| P | P | U | J | Z |
| U | U | 0 | Z | 0 |

| | Q | Y |
|---|---|---|
| J | Q | Y |
| Z | 0 | 0 |
| P | Q | Y |
| U | 0 | 0 |

| | Q | Y |
|---|---|---|
| Q | U+Z | 0 |
| Y | 0 | 0 |

| | J | Z | P | U |
|---|---|---|---|---|
| J | J | Z | P | U |
| Z | Z | 0 | U | 0 |
| P | P | U | J | Z |
| U | U | 0 | Z | 0 |

| | Q | Y |
|---|---|---|
| J | Q | Y |
| Z | Y | 0 |
| P | Q | Y |
| U | Y | 0 |

| | Q | Y |
|---|---|---|
| Q | U+Z | 0 |
| Y | 0 | 0 |

| | J | Z | P | U |
|---|---|---|---|---|
| J | J | Z | P | U |
| Z | Z | 0 | U | 0 |
| P | P | U | J | Z |
| U | U | 0 | Z | 0 |

| | Q | Y |
|---|---|---|
| J | Q | Y |
| Z | 0 | 0 |
| P | Q | Y |
| U | 0 | 0 |

| | Q | Y |
|---|---|---|
| Q | U+Z | 0 |
| Y | 0 | U+Z |

| | J | Z | P | U |
|---|---|---|---|---|
| J | J | Z | P | U |
| Z | Z | 0 | U | 0 |
| P | P | U | J | Z |
| U | U | 0 | Z | 0 |

| | Q | Y |
|---|---|---|
| J | Q | Y |
| Z | 0 | 0 |
| P | Q | Y |
| U | 0 | 0 |

| | Q | Y |
|---|---|---|
| Q | U+Z | U+Z |
| Y | U+Z | 0 |

| | J | Z | P | U |
|---|---|---|---|---|
| J | J | Z | P | U |
| Z | Z | 0 | U | 0 |
| P | P | U | J | Z |
| U | U | 0 | Z | 0 |

| | Q | Y |
|---|---|---|
| J | Q | Y |
| Z | 0 | 0 |
| P | Q | Y |
| U | 0 | 0 |

| | Q | Y |
|---|---|---|
| Q | U+Z | U+Z |
| Y | U+Z | U+Z |

| | J | Z | P | U |
|---|---|---|---|---|
| J | J | Z | P | U |
| Z | Z | 0 | U | 0 |
| P | P | U | J | Z |
| U | U | 0 | Z | 0 |

| | Q | Y |
|---|---|---|
| J | Q | Y |
| Z | 0 | 0 |
| P | Y | Q |
| U | 0 | 0 |

| | Q | Y |
|---|---|---|
| Q | U+Z | U+Z |
| Y | U+Z | U+Z |

| | J | Z | P | U |
|---|---|---|---|---|
| J | J | Z | P | U |
| Z | Z | Z | 0 | 0 |
| P | P | 0 | 0 | 0 |
| U | U | 0 | 0 | 0 |

| | Q | Y |
|---|---|---|
| J | Q | Y |
| Z | 0 | 0 |
| P | 0 | 0 |
| U | 0 | 0 |

| | Q | Y |
|---|---|---|
| Q | U | 0 |
| Y | 0 | 0 |

| | J | Z | P | U |
|---|---|---|---|---|
| J | J | Z | P | U |
| Z | Z | Z | 0 | 0 |
| P | P | 0 | 0 | 0 |
| U | U | 0 | 0 | 0 |

| | Q | Y |
|---|---|---|
| J | Q | Y |
| Z | 0 | Y |
| P | 0 | 0 |
| U | 0 | 0 |

| | Q | Y |
|---|---|---|
| Q | U | 0 |
| Y | 0 | 0 |

| | J | Z | P | U |
|---|---|---|---|---|
| J | J | Z | P | U |
| Z | Z | Z | 0 | 0 |
| P | P | 0 | 0 | 0 |
| U | U | 0 | 0 | 0 |

| | Q | Y |
|---|---|---|
| J | Q | Y |
| Z | Y | Y |
| P | 0 | 0 |
| U | 0 | 0 |

| | Q | Y |
|---|---|---|
| Q | U | 0 |
| Y | 0 | 0 |

| | $J$ | $Z$ | $P$ | $U$ |
|---|---|---|---|---|
| $J$ | $J$ | $Z$ | $P$ | $U$ |
| $Z$ | $Z$ | $Z$ | 0 | 0 |
| $P$ | $P$ | 0 | 0 | 0 |
| $U$ | $U$ | 0 | 0 | 0 |

| | $Q$ | $Y$ |
|---|---|---|
| $J$ | $Q$ | $Y$ |
| $Z$ | 0 | 0 |
| $P$ | 0 | 0 |
| $U$ | $Y$ | 0 |

| | $Q$ | $Y$ |
|---|---|---|
| $Q$ | $U$ | 0 |
| $Y$ | 0 | 0 |

| | $J$ | $Z$ | $P$ | $U$ |
|---|---|---|---|---|
| $J$ | $J$ | $Z$ | $P$ | $U$ |
| $Z$ | $Z$ | $Z$ | 0 | 0 |
| $P$ | $P$ | 0 | 0 | 0 |
| $U$ | $U$ | 0 | 0 | 0 |

| | $Q$ | $Y$ |
|---|---|---|
| $J$ | $Q$ | $Y$ |
| $Z$ | 0 | 0 |
| $P$ | $Y$ | 0 |
| $U$ | 0 | 0 |

| | $Q$ | $Y$ |
|---|---|---|
| $Q$ | $U$ | 0 |
| $Y$ | 0 | 0 |

| | $J$ | $Z$ | $P$ | $U$ |
|---|---|---|---|---|
| $J$ | $J$ | $Z$ | $P$ | $U$ |
| $Z$ | $Z$ | $Z$ | 0 | 0 |
| $P$ | $P$ | 0 | 0 | 0 |
| $U$ | $U$ | 0 | 0 | 0 |

| | $Q$ | $Y$ |
|---|---|---|
| $J$ | $Q$ | $Y$ |
| $Z$ | 0 | 0 |
| $P$ | $Y$ | 0 |
| $U$ | $Y$ | 0 |

| | $Q$ | $Y$ |
|---|---|---|
| $Q$ | $U$ | 0 |
| $Y$ | 0 | 0 |

| | $J$ | $Z$ | $P$ | $U$ |
|---|---|---|---|---|
| $J$ | $J$ | $Z$ | $P$ | $U$ |
| $Z$ | $Z$ | $Z$ | 0 | 0 |
| $P$ | $P$ | 0 | 0 | 0 |
| $U$ | $U$ | 0 | 0 | 0 |

| | $Q$ | $Y$ |
|---|---|---|
| $J$ | $Q$ | $Y$ |
| $Z$ | 0 | 0 |
| $P$ | 0 | 0 |
| $U$ | 0 | 0 |

| | $Q$ | $Y$ |
|---|---|---|
| $Q$ | $U$ | 0 |
| $Y$ | 0 | $P$ |

| | $J$ | $Z$ | $P$ | $U$ |
|---|---|---|---|---|
| $J$ | $J$ | $Z$ | $P$ | $U$ |
| $Z$ | $Z$ | $Z$ | 0 | 0 |
| $P$ | $P$ | 0 | 0 | 0 |
| $U$ | $U$ | 0 | 0 | 0 |

| | $Q$ | $Y$ |
|---|---|---|
| $J$ | $Q$ | $Y$ |
| $Z$ | 0 | 0 |
| $P$ | 0 | 0 |
| $U$ | 0 | 0 |

| | $Q$ | $Y$ |
|---|---|---|
| $Q$ | $U$ | 0 |
| $Y$ | 0 | $U$ |

| | $J$ | $Z$ | $P$ | $U$ |
|---|---|---|---|---|
| $J$ | $J$ | $Z$ | $P$ | $U$ |
| $Z$ | $Z$ | $Z$ | 0 | 0 |
| $P$ | $P$ | 0 | 0 | 0 |
| $U$ | $U$ | 0 | 0 | 0 |

| | $Q$ | $Y$ |
|---|---|---|
| $J$ | $Q$ | $Y$ |
| $Z$ | 0 | $Y$ |
| $P$ | 0 | 0 |
| $U$ | 0 | 0 |

| | $Q$ | $Y$ |
|---|---|---|
| $Q$ | $U$ | 0 |
| $Y$ | 0 | $Z$ |

| | $J$ | $Z$ | $P$ | $U$ |
|---|---|---|---|---|
| $J$ | $J$ | $Z$ | $P$ | $U$ |
| $Z$ | $Z$ | $Z$ | 0 | 0 |
| $P$ | $P$ | 0 | 0 | 0 |
| $U$ | $U$ | 0 | 0 | 0 |

| | $Q$ | $Y$ |
|---|---|---|
| $J$ | $Q$ | $Y$ |
| $Z$ | 0 | 0 |
| $P$ | 0 | 0 |
| $U$ | 0 | 0 |

| | $Q$ | $Y$ |
|---|---|---|
| $Q$ | $U$ | $P$ |
| $Y$ | $P$ | 0 |

| | $J$ | $Z$ | $P$ | $U$ |
|---|---|---|---|---|
| $J$ | $J$ | $Z$ | $P$ | $U$ |
| $Z$ | $Z$ | $Z$ | 0 | 0 |
| $P$ | $P$ | 0 | 0 | 0 |
| $U$ | $U$ | 0 | 0 | 0 |

| | $Q$ | $Y$ |
|---|---|---|
| $J$ | $Q$ | $Y$ |
| $Z$ | 0 | 0 |
| $P$ | 0 | 0 |
| $U$ | 0 | 0 |

| | $Q$ | $Y$ |
|---|---|---|
| $Q$ | $U$ | $P$ |
| $Y$ | $P$ | $P$ |

| | $J$ | $Z$ | $P$ | $U$ |
|---|---|---|---|---|
| $J$ | $J$ | $Z$ | $P$ | $U$ |
| $Z$ | $Z$ | $Z$ | 0 | 0 |
| $P$ | $P$ | 0 | 0 | 0 |
| $U$ | $U$ | 0 | 0 | 0 |

| | $Q$ | $Y$ |
|---|---|---|
| $J$ | $Q$ | $Y$ |
| $Z$ | 0 | 0 |
| $P$ | 0 | 0 |
| $U$ | 0 | 0 |

| | $Q$ | $Y$ |
|---|---|---|
| $Q$ | $U$ | $P$ |
| $Y$ | $P$ | $U$ |

| | $J$ | $Z$ | $P$ | $U$ |
|---|---|---|---|---|
| $J$ | $J$ | $Z$ | $P$ | $U$ |
| $Z$ | $Z$ | $Z$ | 0 | 0 |
| $P$ | $P$ | 0 | 0 | 0 |
| $U$ | $U$ | 0 | 0 | 0 |

| | $Q$ | $Y$ |
|---|---|---|
| $J$ | $Q$ | $Y$ |
| $Z$ | 0 | 0 |
| $P$ | 0 | 0 |
| $U$ | 0 | 0 |

| | $Q$ | $Y$ |
|---|---|---|
| $Q$ | $U$ | $U$ |
| $Y$ | $U$ | 0 |

| | $J$ | $Z$ | $P$ | $U$ |
|---|---|---|---|---|
| $J$ | $J$ | $Z$ | $P$ | $U$ |
| $Z$ | $Z$ | $Z$ | 0 | 0 |
| $P$ | $P$ | 0 | 0 | 0 |
| $U$ | $U$ | 0 | 0 | 0 |

| | $Q$ | $Y$ |
|---|---|---|
| $J$ | $Q$ | $Y$ |
| $Z$ | 0 | 0 |
| $P$ | 0 | 0 |
| $U$ | 0 | 0 |

| | $Q$ | $Y$ |
|---|---|---|
| $Q$ | $U$ | $U$ |
| $Y$ | $U$ | $P$ |

| | $J$ | $Z$ | $P$ | $U$ |
|---|---|---|---|---|
| $J$ | $J$ | $Z$ | $P$ | $U$ |
| $Z$ | $Z$ | $Z$ | 0 | 0 |
| $P$ | $P$ | 0 | 0 | 0 |
| $U$ | $U$ | 0 | 0 | 0 |

| | $Q$ | $Y$ |
|---|---|---|
| $J$ | $Q$ | $Y$ |
| $Z$ | 0 | 0 |
| $P$ | 0 | 0 |
| $U$ | 0 | 0 |

| | $Q$ | $Y$ |
|---|---|---|
| $Q$ | $U$ | $U$ |
| $Y$ | $U$ | $U$ |

| | $J$ | $Z$ | $P$ | $U$ |
|---|---|---|---|---|
| $J$ | $J$ | $Z$ | $P$ | $U$ |
| $Z$ | $Z$ | $Z$ | 0 | 0 |
| $P$ | $P$ | 0 | 0 | 0 |
| $U$ | $U$ | 0 | 0 | 0 |

| | $Q$ | $Y$ |
|---|---|---|
| $J$ | $Q$ | $Y$ |
| $Z$ | $Q$ | 0 |
| $P$ | 0 | 0 |
| $U$ | 0 | 0 |

| | $Q$ | $Y$ |
|---|---|---|
| $Q$ | $Z$ | 0 |
| $Y$ | 0 | 0 |

| | $J$ | $Z$ | $P$ | $U$ |
|---|---|---|---|---|
| $J$ | $J$ | $Z$ | $P$ | $U$ |
| $Z$ | $Z$ | $Z$ | 0 | 0 |
| $P$ | $P$ | 0 | 0 | 0 |
| $U$ | $U$ | 0 | 0 | 0 |

| | $Q$ | $Y$ |
|---|---|---|
| $J$ | $Q$ | $Y$ |
| $Z$ | $Q$ | 0 |
| $P$ | 0 | 0 |
| $U$ | 0 | 0 |

| | $Q$ | $Y$ |
|---|---|---|
| $Q$ | $Z$ | 0 |
| $Y$ | 0 | $P$ |

| | $J$ | $Z$ | $P$ | $U$ |
|---|---|---|---|---|
| $J$ | $J$ | $Z$ | $P$ | $U$ |
| $Z$ | $Z$ | $Z$ | 0 | 0 |
| $P$ | $P$ | 0 | 0 | 0 |
| $U$ | $U$ | 0 | 0 | 0 |

| | $Q$ | $Y$ |
|---|---|---|
| $J$ | $Q$ | $Y$ |
| $Z$ | $Q$ | 0 |
| $P$ | 0 | 0 |
| $U$ | 0 | 0 |

| | $Q$ | $Y$ |
|---|---|---|
| $Q$ | $Z$ | 0 |
| $Y$ | 0 | $U$ |

| | $J$ | $Z$ | $P$ | $U$ |
|---|---|---|---|---|
| $J$ | $J$ | $Z$ | $P$ | $U$ |
| $Z$ | $Z$ | $Z$ | 0 | 0 |
| $P$ | $P$ | 0 | 0 | 0 |
| $U$ | $U$ | 0 | 0 | 0 |

| | $Q$ | $Y$ |
|---|---|---|
| $J$ | $Q$ | $Y$ |
| $Z$ | $Q$ | $Q$ |
| $P$ | 0 | 0 |
| $U$ | 0 | 0 |

| | $Q$ | $Y$ |
|---|---|---|
| $Q$ | $Z$ | $Z$ |
| $Y$ | $Z$ | $Z$ |

| | $J$ | $Z$ | $P$ | $U$ |
|---|---|---|---|---|
| $J$ | $J$ | $Z$ | $P$ | $U$ |
| $Z$ | $Z$ | $Z$ | 0 | 0 |
| $P$ | $P$ | 0 | 0 | 0 |
| $U$ | $U$ | 0 | 0 | 0 |

| | $Q$ | $Y$ |
|---|---|---|
| $J$ | $Q$ | $Y$ |
| $Z$ | $Y$ | $Y$ |
| $P$ | 0 | 0 |
| $U$ | 0 | 0 |

| | $Q$ | $Y$ |
|---|---|---|
| $Q$ | $Z$ | $Z$ |
| $Y$ | $Z$ | $Z$ |

| | $J$ | $Z$ | $P$ | $U$ |
|---|---|---|---|---|
| $J$ | $J$ | $Z$ | $P$ | $U$ |
| $Z$ | $Z$ | $Z$ | 0 | 0 |
| $P$ | $P$ | 0 | 0 | 0 |
| $U$ | $U$ | 0 | 0 | 0 |

| | $Q$ | $Y$ |
|---|---|---|
| $J$ | $Q$ | $Y$ |
| $Z$ | $Q$ | $Q$ |
| $P$ | 0 | 0 |
| $U$ | 0 | 0 |

| | $Q$ | $Y$ |
|---|---|---|
| $Q$ | $Z$ | $Z$ |
| $Y$ | $Z$ | $P+Z$ |

| | $J$ | $Z$ | $P$ | $U$ |
|---|---|---|---|---|
| $J$ | $J$ | $Z$ | $P$ | $U$ |
| $Z$ | $Z$ | $Z$ | 0 | 0 |
| $P$ | $P$ | 0 | 0 | 0 |
| $U$ | $U$ | 0 | 0 | 0 |

| | $Q$ | $Y$ |
|---|---|---|
| $J$ | $Q$ | $Y$ |
| $Z$ | $Q$ | $Q$ |
| $P$ | 0 | 0 |
| $U$ | 0 | 0 |

| | $Q$ | $Y$ |
|---|---|---|
| $Q$ | $Z$ | $Z$ |
| $Y$ | $Z$ | $U+Z$ |

| | $J$ | $Z$ | $P$ | $U$ |
|---|---|---|---|---|
| $J$ | $J$ | $Z$ | $P$ | $U$ |
| $Z$ | $Z$ | $Z$ | 0 | 0 |
| $P$ | $P$ | 0 | 0 | 0 |
| $U$ | $U$ | 0 | 0 | 0 |

| | $Q$ | $Y$ |
|---|---|---|
| $J$ | $Q$ | $Y$ |
| $Z$ | $Y$ | $Y$ |
| $P$ | 0 | 0 |
| $U$ | 0 | 0 |

| | $Q$ | $Y$ |
|---|---|---|
| $Q$ | $U+Z$ | $Z$ |
| $Y$ | $Z$ | $Z$ |

| | $J$ | $Z$ | $P$ | $U$ |
|---|---|---|---|---|
| $J$ | $J$ | $Z$ | $P$ | $U$ |
| $Z$ | $Z$ | $Z$ | 0 | $U$ |
| $P$ | $P$ | 0 | 0 | 0 |
| $U$ | $U$ | $U$ | 0 | 0 |

| | $Q$ | $Y$ |
|---|---|---|
| $J$ | $Q$ | $Y$ |
| $Z$ | $Q$ | 0 |
| $P$ | 0 | 0 |
| $U$ | 0 | 0 |

| | $Q$ | $Y$ |
|---|---|---|
| $Q$ | $U$ | 0 |
| $Y$ | 0 | 0 |

| | $J$ | $Z$ | $P$ | $U$ |
|---|---|---|---|---|
| $J$ | $J$ | $Z$ | $P$ | $U$ |
| $Z$ | $Z$ | $Z$ | 0 | $U$ |
| $P$ | $P$ | 0 | 0 | 0 |
| $U$ | $U$ | $U$ | 0 | 0 |

| | $Q$ | $Y$ |
|---|---|---|
| $J$ | $Q$ | $Y$ |
| $Z$ | $Q$ | $Y$ |
| $P$ | 0 | 0 |
| $U$ | 0 | 0 |

| | $Q$ | $Y$ |
|---|---|---|
| $Q$ | $U$ | 0 |
| $Y$ | 0 | 0 |

| | $J$ | $Z$ | $P$ | $U$ |
|---|---|---|---|---|
| $J$ | $J$ | $Z$ | $P$ | $U$ |
| $Z$ | $Z$ | $Z$ | 0 | $U$ |
| $P$ | $P$ | 0 | 0 | 0 |
| $U$ | $U$ | $U$ | 0 | 0 |

| | $Q$ | $Y$ |
|---|---|---|
| $J$ | $Q$ | $Y$ |
| $Z$ | $Q$ | $Y$ |
| $P$ | 0 | 0 |
| $U$ | $Y$ | 0 |

| | $Q$ | $Y$ |
|---|---|---|
| $Q$ | $U$ | 0 |
| $Y$ | 0 | 0 |

| | $J$ | $Z$ | $P$ | $U$ |
|---|---|---|---|---|
| $J$ | $J$ | $Z$ | $P$ | $U$ |
| $Z$ | $Z$ | $Z$ | 0 | $U$ |
| $P$ | $P$ | 0 | 0 | 0 |
| $U$ | $U$ | $U$ | 0 | 0 |

| | $Q$ | $Y$ |
|---|---|---|
| $J$ | $Q$ | $Y$ |
| $Z$ | $Q$ | 0 |
| $P$ | 0 | 0 |
| $U$ | 0 | 0 |

| | $Q$ | $Y$ |
|---|---|---|
| $Q$ | $U$ | 0 |
| $Y$ | 0 | $P$ |

| | $J$ | $Z$ | $P$ | $U$ |
|---|---|---|---|---|
| $J$ | $J$ | $Z$ | $P$ | $U$ |
| $Z$ | $Z$ | $Z$ | 0 | $U$ |
| $P$ | $P$ | 0 | 0 | 0 |
| $U$ | $U$ | $U$ | 0 | 0 |

| | $Q$ | $Y$ |
|---|---|---|
| $J$ | $Q$ | $Y$ |
| $Z$ | $Q$ | $Y$ |
| $P$ | 0 | 0 |
| $U$ | 0 | 0 |

| | $Q$ | $Y$ |
|---|---|---|
| $Q$ | $U$ | 0 |
| $Y$ | 0 | $U$ |

| | $J$ | $Z$ | $P$ | $U$ |
|---|---|---|---|---|
| $J$ | $J$ | $Z$ | $P$ | $U$ |
| $Z$ | $Z$ | $Z$ | 0 | $U$ |
| $P$ | $P$ | 0 | 0 | 0 |
| $U$ | $U$ | $U$ | 0 | 0 |

| | $Q$ | $Y$ |
|---|---|---|
| $J$ | $Q$ | $Y$ |
| $Z$ | $Q$ | $Y$ |
| $P$ | 0 | 0 |
| $U$ | 0 | 0 |

| | $Q$ | $Y$ |
|---|---|---|
| $Q$ | $U$ | $U$ |
| $Y$ | $U$ | 0 |

| | J | Z | P | U |
|---|---|---|---|---|
| J | J | Z | P | U |
| Z | Z | Z | 0 | U |
| P | P | 0 | 0 | 0 |
| U | U | U | 0 | 0 |

| | Q | Y |
|---|---|---|
| J | Q | Y |
| Z | Q | Q |
| P | 0 | 0 |
| U | 0 | 0 |

| | Q | Y |
|---|---|---|
| Q | U | U |
| Y | U | U |

| | J | Z | P | U |
|---|---|---|---|---|
| J | J | Z | P | U |
| Z | Z | Z | 0 | U |
| P | P | 0 | 0 | 0 |
| U | U | U | 0 | 0 |

| | Q | Y |
|---|---|---|
| J | Q | Y |
| Z | Q | Y |
| P | 0 | 0 |
| U | 0 | 0 |

| | Q | Y |
|---|---|---|
| Q | U | U |
| Y | U | U |

| | J | Z | P | U |
|---|---|---|---|---|
| J | J | Z | P | U |
| Z | Z | Z | 0 | U |
| P | P | 0 | 0 | 0 |
| U | U | U | 0 | 0 |

| | Q | Y |
|---|---|---|
| J | Q | Y |
| Z | Y | Y |
| P | 0 | 0 |
| U | 0 | 0 |

| | Q | Y |
|---|---|---|
| Q | U | U |
| Y | U | U |

| | J | Z | P | U |
|---|---|---|---|---|
| J | J | Z | P | U |
| Z | Z | Z | 0 | U |
| P | P | 0 | 0 | 0 |
| U | U | U | 0 | 0 |

| | Q | Y |
|---|---|---|
| J | Q | Y |
| Z | Q | Y |
| P | 0 | 0 |
| U | Y | 0 |

| | Q | Y |
|---|---|---|
| Q | Z | U |
| Y | U | 0 |

| | J | Z | P | U |
|---|---|---|---|---|
| J | J | Z | P | U |
| Z | Z | Z | 0 | U |
| P | P | 0 | 0 | 0 |
| U | U | U | 0 | 0 |

| | Q | Y |
|---|---|---|
| J | Q | Y |
| Z | Q | Y |
| P | 0 | 0 |
| U | Y | 0 |

| | Q | Y |
|---|---|---|
| Q | $U+Z$ | U |
| Y | U | 0 |

| | J | Z | P | U |
|---|---|---|---|---|
| J | J | Z | P | U |
| Z | Z | Z | P | 0 |
| P | P | P | 0 | 0 |
| U | U | 0 | 0 | 0 |

| | Q | Y |
|---|---|---|
| J | Q | Y |
| Z | 0 | 0 |
| P | 0 | 0 |
| U | 0 | 0 |

| | Q | Y |
|---|---|---|
| Q | U | 0 |
| Y | 0 | 0 |

| | J | Z | P | U |
|---|---|---|---|---|
| J | J | Z | P | U |
| Z | Z | Z | P | 0 |
| P | P | P | 0 | 0 |
| U | U | 0 | 0 | 0 |

| | Q | Y |
|---|---|---|
| J | Q | Y |
| Z | 0 | Y |
| P | 0 | 0 |
| U | 0 | 0 |

| | Q | Y |
|---|---|---|
| Q | U | 0 |
| Y | 0 | 0 |

| | J | Z | P | U |
|---|---|---|---|---|
| J | J | Z | P | U |
| Z | Z | Z | P | 0 |
| P | P | P | 0 | 0 |
| U | U | 0 | 0 | 0 |

| | Q | Y |
|---|---|---|
| J | Q | Y |
| Z | Y | Y |
| P | 0 | 0 |
| U | 0 | 0 |

| | Q | Y |
|---|---|---|
| Q | U | 0 |
| Y | 0 | 0 |

| | J | Z | P | U |
|---|---|---|---|---|
| J | J | Z | P | U |
| Z | Z | Z | P | 0 |
| P | P | P | 0 | 0 |
| U | U | 0 | 0 | 0 |

| | Q | Y |
|---|---|---|
| J | Q | Y |
| Z | 0 | 0 |
| P | 0 | 0 |
| U | Y | 0 |

| | Q | Y |
|---|---|---|
| Q | U | 0 |
| Y | 0 | 0 |

| | J | Z | P | U |
|---|---|---|---|---|
| J | J | Z | P | U |
| Z | Z | Z | P | 0 |
| P | P | P | 0 | 0 |
| U | U | 0 | 0 | 0 |

| | Q | Y |
|---|---|---|
| J | Q | Y |
| Z | 0 | Y |
| P | 0 | 0 |
| U | 0 | 0 |

| | Q | Y |
|---|---|---|
| Q | U | 0 |
| Y | 0 | P |

| | J | Z | P | U |
|---|---|---|---|---|
| J | J | Z | P | U |
| Z | Z | Z | P | 0 |
| P | P | P | 0 | 0 |
| U | U | 0 | 0 | 0 |

| | Q | Y |
|---|---|---|
| J | Q | Y |
| Z | 0 | 0 |
| P | 0 | 0 |
| U | 0 | 0 |

| | Q | Y |
|---|---|---|
| Q | U | 0 |
| Y | 0 | U |

| | J | Z | P | U |
|---|---|---|---|---|
| J | J | Z | P | U |
| Z | Z | Z | P | 0 |
| P | P | P | 0 | 0 |
| U | U | 0 | 0 | 0 |

| | Q | Y |
|---|---|---|
| J | Q | Y |
| Z | 0 | 0 |
| P | 0 | 0 |
| U | 0 | 0 |

| | Q | Y |
|---|---|---|
| Q | U | U |
| Y | U | 0 |

| | J | Z | P | U |
|---|---|---|---|---|
| J | J | Z | P | U |
| Z | Z | Z | P | 0 |
| P | P | P | 0 | 0 |
| U | U | 0 | 0 | 0 |

| | Q | Y |
|---|---|---|
| J | Q | Y |
| Z | 0 | 0 |
| P | 0 | 0 |
| U | 0 | 0 |

| | Q | Y |
|---|---|---|
| Q | U | U |
| Y | U | U |

| | J | Z | P | U |
|---|---|---|---|---|
| J | J | Z | P | U |
| Z | Z | Z | P | 0 |
| P | P | P | 0 | 0 |
| U | U | 0 | 0 | 0 |

| | Q | Y |
|---|---|---|
| J | Q | Y |
| Z | Q | Y |
| P | Y | 0 |
| U | 0 | 0 |

| | Q | Y |
|---|---|---|
| Q | Z | P |
| Y | P | 0 |

| | J | Z | P | U |
|---|---|---|---|---|
| J | J | Z | P | U |
| Z | Z | Z | P | P |
| P | P | P | 0 | 0 |
| U | U | P | 0 | 0 |

| | Q | Y |
|---|---|---|
| J | Q | Y |
| Z | Y | Y |
| P | 0 | 0 |
| U | 0 | 0 |

| | Q | Y |
|---|---|---|
| Q | U | P |
| Y | P | P |

| | J | Z | P | U |
|---|---|---|---|---|
| J | J | Z | P | U |
| Z | Z | Z | P | P |
| P | P | P | 0 | 0 |
| U | U | P | 0 | 0 |

| | Q | Y |
|---|---|---|
| J | Q | Y |
| Z | Q | Y |
| P | Y | 0 |
| U | Y | 0 |

| | Q | Y |
|---|---|---|
| Q | Z | P |
| Y | P | 0 |

| | J | Z | P | U |
|---|---|---|---|---|
| J | J | Z | P | U |
| Z | Z | Z | P | U |
| P | P | P | 0 | 0 |
| U | U | U | 0 | 0 |

| | Q | Y |
|---|---|---|
| J | Q | Y |
| Z | Q | 0 |
| P | 0 | 0 |
| U | 0 | 0 |

| | Q | Y |
|---|---|---|
| Q | U | 0 |
| Y | 0 | 0 |

| | J | Z | P | U |
|---|---|---|---|---|
| J | J | Z | P | U |
| Z | Z | Z | P | U |
| P | P | P | 0 | 0 |
| U | U | U | 0 | 0 |

| | Q | Y |
|---|---|---|
| J | Q | Y |
| Z | Q | Y |
| P | 0 | 0 |
| U | 0 | 0 |

| | Q | Y |
|---|---|---|
| Q | U | 0 |
| Y | 0 | 0 |

| | J | Z | P | U |
|---|---|---|---|---|
| J | J | Z | P | U |
| Z | Z | Z | P | U |
| P | P | P | 0 | 0 |
| U | U | U | 0 | 0 |

| | Q | Y |
|---|---|---|
| J | Q | Y |
| Z | Q | Y |
| P | 0 | 0 |
| U | Y | 0 |

| | Q | Y |
|---|---|---|
| Q | U | 0 |
| Y | 0 | 0 |

| | J | Z | P | U |
|---|---|---|---|---|
| J | J | Z | P | U |
| Z | Z | Z | P | U |
| P | P | P | 0 | 0 |
| U | U | U | 0 | 0 |

| | Q | Y |
|---|---|---|
| J | Q | Y |
| Z | Q | Y |
| P | Y | 0 |
| U | 0 | 0 |

| | Q | Y |
|---|---|---|
| Q | U | 0 |
| Y | 0 | 0 |

| | J | Z | P | U |
|---|---|---|---|---|
| J | J | Z | P | U |
| Z | Z | Z | P | U |
| P | P | P | 0 | 0 |
| U | U | U | 0 | 0 |

| | Q | Y |
|---|---|---|
| J | Q | Y |
| Z | Q | Y |
| P | Y | 0 |
| U | Y | 0 |

| | Q | Y |
|---|---|---|
| Q | U | 0 |
| Y | 0 | 0 |

| | J | Z | P | U |
|---|---|---|---|---|
| J | J | Z | P | U |
| Z | Z | Z | P | U |
| P | P | P | 0 | 0 |
| U | U | U | 0 | 0 |

| | Q | Y |
|---|---|---|
| J | Q | Y |
| Z | Q | Y |
| P | 0 | 0 |
| U | 0 | 0 |

| | Q | Y |
|---|---|---|
| Q | U | 0 |
| Y | 0 | P |

| | J | Z | P | U |
|---|---|---|---|---|
| J | J | Z | P | U |
| Z | Z | Z | P | U |
| P | P | P | 0 | 0 |
| U | U | U | 0 | 0 |

| | Q | Y |
|---|---|---|
| J | Q | Y |
| Z | Q | Y |
| P | 0 | 0 |
| U | 0 | 0 |

| | Q | Y |
|---|---|---|
| Q | U | 0 |
| Y | 0 | U |

| | J | Z | P | U |
|---|---|---|---|---|
| J | J | Z | P | U |
| Z | Z | Z | P | U |
| P | P | P | 0 | 0 |
| U | U | U | 0 | 0 |

| | Q | Y |
|---|---|---|
| J | Q | Y |
| Z | Q | Y |
| P | 0 | 0 |
| U | 0 | 0 |

| | Q | Y |
|---|---|---|
| Q | U | P |
| Y | P | 0 |

| | J | Z | P | U |
|---|---|---|---|---|
| J | J | Z | P | U |
| Z | Z | Z | P | U |
| P | P | P | 0 | 0 |
| U | U | U | 0 | 0 |

| | Q | Y |
|---|---|---|
| J | Q | Y |
| Z | Q | Y |
| P | 0 | 0 |
| U | 0 | 0 |

| | Q | Y |
|---|---|---|
| Q | U | P |
| Y | P | P |

| | J | Z | P | U |
|---|---|---|---|---|
| J | J | Z | P | U |
| Z | Z | Z | P | U |
| P | P | P | 0 | 0 |
| U | U | U | 0 | 0 |

| | Q | Y |
|---|---|---|
| J | Q | Y |
| Z | Q | Y |
| P | 0 | 0 |
| U | 0 | 0 |

| | Q | Y |
|---|---|---|
| Q | U | P |
| Y | P | U |

| | J | Z | P | U |
|---|---|---|---|---|
| J | J | Z | P | U |
| Z | Z | Z | P | U |
| P | P | P | 0 | 0 |
| U | U | U | 0 | 0 |

| | Q | Y |
|---|---|---|
| J | Q | Y |
| Z | Q | Y |
| P | 0 | 0 |
| U | 0 | 0 |

| | Q | Y |
|---|---|---|
| Q | U | U |
| Y | U | 0 |

| | J | Z | P | U |
|---|---|---|---|---|
| J | J | Z | P | U |
| Z | Z | Z | U | U |
| P | P | U | 0 | 0 |
| U | U | U | 0 | 0 |

| | Q | Y |
|---|---|---|
| J | Q | Y |
| Z | Y | Y |
| P | 0 | 0 |
| U | 0 | 0 |

| | Q | Y |
|---|---|---|
| Q | U | U |
| Y | U | U |

| | J | Z | P | U |
|---|---|---|---|---|
| J | J | Z | P | U |
| Z | Z | Z | P | U |
| P | P | P | 0 | 0 |
| U | U | U | 0 | 0 |

| | Q | Y |
|---|---|---|
| J | Q | Y |
| Z | Q | Y |
| P | 0 | 0 |
| U | 0 | 0 |

| | Q | Y |
|---|---|---|
| Q | U | U |
| Y | U | P |

| | J | Z | P | U |
|---|---|---|---|---|
| J | J | Z | P | U |
| Z | Z | Z | U | U |
| P | P | U | 0 | 0 |
| U | U | U | 0 | 0 |

| | Q | Y |
|---|---|---|
| J | Q | Y |
| Z | Q | Y |
| P | Y | 0 |
| U | Y | 0 |

| | Q | Y |
|---|---|---|
| Q | Z | U |
| Y | U | 0 |

| | J | Z | P | U |
|---|---|---|---|---|
| J | J | Z | P | U |
| Z | Z | Z | P | U |
| P | P | P | 0 | 0 |
| U | U | U | 0 | 0 |

| | Q | Y |
|---|---|---|
| J | Q | Y |
| Z | Q | Q |
| P | 0 | 0 |
| U | 0 | 0 |

| | Q | Y |
|---|---|---|
| Q | U | U |
| Y | U | U |

| | J | Z | P | U |
|---|---|---|---|---|
| J | J | Z | P | U |
| Z | Z | Z | U | U |
| P | P | U | 0 | 0 |
| U | U | U | 0 | 0 |

| | Q | Y |
|---|---|---|
| J | Q | Y |
| Z | Q | Y |
| P | Y | 0 |
| U | Y | 0 |

| | Q | Y |
|---|---|---|
| Q | $U+Z$ | U |
| Y | U | 0 |

| | J | Z | P | U |
|---|---|---|---|---|
| J | J | Z | P | U |
| Z | Z | Z | P | U |
| P | P | P | 0 | 0 |
| U | U | U | 0 | 0 |

| | Q | Y |
|---|---|---|
| J | Q | Y |
| Z | Q | Y |
| P | 0 | 0 |
| U | 0 | 0 |

| | Q | Y |
|---|---|---|
| Q | U | U |
| Y | U | U |

| | J | Z | P | U |
|---|---|---|---|---|
| J | J | Z | P | U |
| Z | Z | Z | 0 | U |
| P | P | 0 | 0 | 0 |
| U | U | U | 0 | Z |

| | Q | Y |
|---|---|---|
| J | Q | Y |
| Z | Q | Y |
| P | 0 | 0 |
| U | Y | Q |

| | Q | Y |
|---|---|---|
| Q | U | Z |
| Y | Z | U |

| | J | Z | P | U |
|---|---|---|---|---|
| J | J | Z | P | U |
| Z | Z | Z | P | U |
| P | P | P | 0 | 0 |
| U | U | U | 0 | 0 |

| | Q | Y |
|---|---|---|
| J | Q | Y |
| Z | Y | Y |
| P | 0 | 0 |
| U | 0 | 0 |

| | Q | Y |
|---|---|---|
| Q | U | U |
| Y | U | U |

| | J | Z | P | U |
|---|---|---|---|---|
| J | J | Z | P | U |
| Z | Z | Z | 0 | U |
| P | P | 0 | 0 | 0 |
| U | U | U | 0 | Z |

| | Q | Y |
|---|---|---|
| J | Q | Y |
| Z | Q | Y |
| P | 0 | 0 |
| U | Y | Q |

| | Q | Y |
|---|---|---|
| Q | Z | U |
| Y | U | Z |

| | J | Z | P | U |
|---|---|---|---|---|
| J | J | Z | P | U |
| Z | Z | Z | U | U |
| P | P | U | 0 | 0 |
| U | U | U | 0 | 0 |

| | Q | Y |
|---|---|---|
| J | Q | Y |
| Z | Q | 0 |
| P | 0 | 0 |
| U | 0 | 0 |

| | Q | Y |
|---|---|---|
| Q | U | 0 |
| Y | 0 | 0 |

| | J | Z | P | U |
|---|---|---|---|---|
| J | J | Z | P | U |
| Z | Z | Z | 0 | U |
| P | P | 0 | 0 | 0 |
| U | U | U | 0 | Z |

| | Q | Y |
|---|---|---|
| J | Q | Y |
| Z | Q | 0 |
| P | 0 | 0 |
| U | Q | 0 |

| | Q | Y |
|---|---|---|
| Q | $U+Z$ | 0 |
| Y | 0 | 0 |

| | J | Z | P | U |
|---|---|---|---|---|
| J | J | Z | P | U |
| Z | Z | Z | U | U |
| P | P | U | 0 | 0 |
| U | U | U | 0 | 0 |

| | Q | Y |
|---|---|---|
| J | Q | Y |
| Z | Q | Y |
| P | 0 | 0 |
| U | 0 | 0 |

| | Q | Y |
|---|---|---|
| Q | U | 0 |
| Y | 0 | 0 |

| | J | Z | P | U |
|---|---|---|---|---|
| J | J | Z | P | U |
| Z | Z | Z | 0 | U |
| P | P | 0 | 0 | 0 |
| U | U | U | 0 | Z |

| | Q | Y |
|---|---|---|
| J | Q | Y |
| Z | Q | 0 |
| P | 0 | 0 |
| U | Q | 0 |

| | Q | Y |
|---|---|---|
| Q | $U+Z$ | 0 |
| Y | 0 | P |

| | J | Z | P | U |
|---|---|---|---|---|
| J | J | Z | P | U |
| Z | Z | Z | U | U |
| P | P | U | 0 | 0 |
| U | U | U | 0 | 0 |

| | Q | Y |
|---|---|---|
| J | Q | Y |
| Z | Q | Y |
| P | Y | 0 |
| U | Y | 0 |

| | Q | Y |
|---|---|---|
| Q | U | 0 |
| Y | 0 | 0 |

| | J | Z | P | U |
|---|---|---|---|---|
| J | J | Z | P | U |
| Z | Z | Z | 0 | U |
| P | P | 0 | 0 | 0 |
| U | U | U | 0 | Z |

| | Q | Y |
|---|---|---|
| J | Q | Y |
| Z | Q | Q |
| P | 0 | 0 |
| U | Q | Q |

| | Q | Y |
|---|---|---|
| Q | $U+Z$ | $U+Z$ |
| Y | $U+Z$ | $U+Z$ |

| | J | Z | P | U |
|---|---|---|---|---|
| J | J | Z | P | U |
| Z | Z | Z | U | U |
| P | P | U | 0 | 0 |
| U | U | U | 0 | 0 |

| | Q | Y |
|---|---|---|
| J | Q | Y |
| Z | Q | Y |
| P | 0 | 0 |
| U | 0 | 0 |

| | Q | Y |
|---|---|---|
| Q | U | 0 |
| Y | 0 | U |

| | J | Z | P | U |
|---|---|---|---|---|
| J | J | Z | P | U |
| Z | Z | Z | 0 | U |
| P | P | 0 | 0 | 0 |
| U | U | U | 0 | Z |

| | Q | Y |
|---|---|---|
| J | Q | Y |
| Z | Q | Y |
| P | 0 | 0 |
| U | Y | Q |

| | Q | Y |
|---|---|---|
| Q | $U+Z$ | $U+Z$ |
| Y | $U+Z$ | $U+Z$ |

| | J | Z | P | U |
|---|---|---|---|---|
| J | J | Z | P | U |
| Z | Z | Z | U | U |
| P | P | U | 0 | 0 |
| U | U | U | 0 | 0 |

| | Q | Y |
|---|---|---|
| J | Q | Y |
| Z | Q | Y |
| P | 0 | 0 |
| U | 0 | 0 |

| | Q | Y |
|---|---|---|
| Q | U | U |
| Y | U | 0 |

| | J | Z | P | U |
|---|---|---|---|---|
| J | J | Z | P | U |
| Z | Z | Z | 0 | U |
| P | P | 0 | 0 | 0 |
| U | U | U | 0 | Z |

| | Q | Y |
|---|---|---|
| J | Q | Y |
| Z | Y | Y |
| P | 0 | 0 |
| U | Y | Y |

| | Q | Y |
|---|---|---|
| Q | $U+Z$ | $U+Z$ |
| Y | $U+Z$ | $U+Z$ |

| | J | Z | P | U |
|---|---|---|---|---|
| J | J | Z | P | U |
| Z | Z | Z | U | U |
| P | P | U | 0 | 0 |
| U | U | U | 0 | 0 |

| | Q | Y |
|---|---|---|
| J | Q | Y |
| Z | Q | Q |
| P | 0 | 0 |
| U | 0 | 0 |

| | Q | Y |
|---|---|---|
| Q | U | U |
| Y | U | P |

| | J | Z | P | U |
|---|---|---|---|---|
| J | J | Z | P | U |
| Z | Z | Z | P | 0 |
| P | P | P | Z | 0 |
| U | U | 0 | 0 | 0 |

| | Q | Y |
|---|---|---|
| J | Q | Y |
| Z | 0 | 0 |
| P | 0 | 0 |
| U | 0 | 0 |

| | Q | Y |
|---|---|---|
| Q | U | 0 |
| Y | 0 | 0 |

| | J | Z | P | U |
|---|---|---|---|---|
| J | J | Z | P | U |
| Z | Z | Z | U | U |
| P | P | U | 0 | 0 |
| U | U | U | 0 | 0 |

| | Q | Y |
|---|---|---|
| J | Q | Y |
| Z | Q | Q |
| P | 0 | 0 |
| U | 0 | 0 |

| | Q | Y |
|---|---|---|
| Q | U | U |
| Y | U | U |

| | J | Z | P | U |
|---|---|---|---|---|
| J | J | Z | P | U |
| Z | Z | Z | P | 0 |
| P | P | P | Z | 0 |
| U | U | 0 | 0 | 0 |

| | Q | Y |
|---|---|---|
| J | Q | Y |
| Z | 0 | 0 |
| P | 0 | 0 |
| U | Y | 0 |

| | Q | Y |
|---|---|---|
| Q | U | 0 |
| Y | 0 | 0 |

| | J | Z | P | U |
|---|---|---|---|---|
| J | J | Z | P | U |
| Z | Z | Z | U | U |
| P | P | U | 0 | 0 |
| U | U | U | 0 | 0 |

| | Q | Y |
|---|---|---|
| J | Q | Y |
| Z | Q | Y |
| P | 0 | 0 |
| U | 0 | 0 |

| | Q | Y |
|---|---|---|
| Q | U | U |
| Y | U | U |

| | J | Z | P | U |
|---|---|---|---|---|
| J | J | Z | P | U |
| Z | Z | Z | P | 0 |
| P | P | P | Z | 0 |
| U | U | 0 | 0 | 0 |

| | Q | Y |
|---|---|---|
| J | Q | Y |
| Z | 0 | Y |
| P | 0 | Y |
| U | 0 | 0 |

| | Q | Y |
|---|---|---|
| Q | U | 0 |
| Y | 0 | 0 |

| | J | Z | P | U |
|---|---|---|---|---|
| J | J | Z | P | U |
| Z | Z | Z | P | 0 |
| P | P | P | Z | 0 |
| U | U | 0 | 0 | 0 |

| | Q | Y |
|---|---|---|
| J | Q | Y |
| Z | Y | Y |
| P | Y | Y |
| U | 0 | 0 |

| | Q | Y |
|---|---|---|
| Q | U | 0 |
| Y | 0 | 0 |

| | J | Z | P | U |
|---|---|---|---|---|
| J | J | Z | P | U |
| Z | Z | Z | U | U |
| P | P | U | Z | Z |
| U | U | U | Z | Z |

| | Q | Y |
|---|---|---|
| J | Q | Y |
| Z | Q | Y |
| P | Y | Q |
| U | Y | Q |

| | Q | Y |
|---|---|---|
| Q | $U+Z$ | $U+Z$ |
| Y | $U+Z$ | $U+Z$ |

| | J | Z | P | U |
|---|---|---|---|---|
| J | J | Z | P | U |
| Z | Z | Z | P | 0 |
| P | P | P | Z | 0 |
| U | U | 0 | 0 | 0 |

| | Q | Y |
|---|---|---|
| J | Q | Y |
| Z | 0 | 0 |
| P | 0 | 0 |
| U | 0 | 0 |

| | Q | Y |
|---|---|---|
| Q | U | 0 |
| Y | 0 | U |

| | J | Z | P | U |
|---|---|---|---|---|
| J | J | Z | P | U |
| Z | Z | Z | U | U |
| P | P | U | Z | Z |
| U | U | U | Z | Z |

| | Q | Y |
|---|---|---|
| J | Q | Y |
| Z | Y | Y |
| P | Y | Y |
| U | Y | Y |

| | Q | Y |
|---|---|---|
| Q | $U+Z$ | $U+Z$ |
| Y | $U+Z$ | $U+Z$ |

| | J | Z | P | U |
|---|---|---|---|---|
| J | J | Z | P | U |
| Z | Z | Z | P | 0 |
| P | P | P | Z | 0 |
| U | U | 0 | 0 | 0 |

| | Q | Y |
|---|---|---|
| J | Q | Y |
| Z | 0 | Y |
| P | 0 | Y |
| U | 0 | 0 |

| | Q | Y |
|---|---|---|
| Q | U | 0 |
| Y | 0 | $P+Z$ |

| | J | Z | P | U |
|---|---|---|---|---|
| J | J | Z | P | U |
| Z | Z | Z | P | P |
| P | P | P | Z | Z |
| U | U | P | Z | J |

| | Q | Y |
|---|---|---|
| J | Q | Y |
| Z | Q | Y |
| P | Y | Q |
| U | Y | Q |

| | Q | Y |
|---|---|---|
| Q | Z | P |
| Y | P | Z |

| | J | Z | P | U |
|---|---|---|---|---|
| J | J | Z | P | U |
| Z | Z | Z | P | 0 |
| P | P | P | Z | 0 |
| U | U | 0 | 0 | 0 |

| | Q | Y |
|---|---|---|
| J | Q | Y |
| Z | 0 | 0 |
| P | 0 | 0 |
| U | 0 | 0 |

| | Q | Y |
|---|---|---|
| Q | U | U |
| Y | U | 0 |

| | J | Z | P | U |
|---|---|---|---|---|
| J | J | Z | P | U |
| Z | Z | Z | P | P |
| P | P | P | Z | Z |
| U | U | P | Z | J |

| | Q | Y |
|---|---|---|
| J | Q | Y |
| Z | Y | Y |
| P | Y | Y |
| U | Q | Y |

| | Q | Y |
|---|---|---|
| Q | $J+U$ | $P+Z$ |
| Y | $P+Z$ | $P+Z$ |

| | J | Z | P | U |
|---|---|---|---|---|
| J | J | Z | P | U |
| Z | Z | Z | P | 0 |
| P | P | P | Z | 0 |
| U | U | 0 | 0 | 0 |

| | Q | Y |
|---|---|---|
| J | Q | Y |
| Z | 0 | 0 |
| P | 0 | 0 |
| U | 0 | 0 |

| | Q | Y |
|---|---|---|
| Q | U | U |
| Y | U | U |

| | J | Z | P | U |
|---|---|---|---|---|
| J | J | Z | P | U |
| Z | Z | Z | U | U |
| P | P | U | J | Z |
| U | U | U | Z | Z |

| | Q | Y |
|---|---|---|
| J | Q | Y |
| Z | Q | Y |
| P | Y | Q |
| U | Y | Q |

| | Q | Y |
|---|---|---|
| Q | U | Z |
| Y | Z | U |

| | J | Z | P | U |
|---|---|---|---|---|
| J | J | Z | P | U |
| Z | Z | Z | P | 0 |
| P | P | P | Z | 0 |
| U | U | 0 | 0 | 0 |

| | Q | Y |
|---|---|---|
| J | Q | Y |
| Z | Q | Y |
| P | Y | Q |
| U | 0 | 0 |

| | Q | Y |
|---|---|---|
| Q | Z | P |
| Y | P | Z |

| | J | Z | P | U |
|---|---|---|---|---|
| J | J | Z | P | U |
| Z | Z | Z | U | U |
| P | P | U | J | Z |
| U | U | U | Z | Z |

| | Q | Y |
|---|---|---|
| J | Q | Y |
| Z | Q | Y |
| P | Y | Q |
| U | Y | Q |

| | Q | Y |
|---|---|---|
| Q | Z | U |
| Y | U | Z |

| | J | Z | P | U |
|---|---|---|---|---|
| J | J | Z | P | U |
| Z | Z | Z | P | P |
| P | P | P | Z | Z |
| U | U | P | Z | Z |

| | Q | Y |
|---|---|---|
| J | Q | Y |
| Z | Q | Y |
| P | Y | Q |
| U | Y | Q |

| | Q | Y |
|---|---|---|
| Q | Z | P |
| Y | P | Z |

| | J | Z | P | U |
|---|---|---|---|---|
| J | J | Z | P | U |
| Z | Z | Z | U | U |
| P | P | U | J | Z |
| U | U | U | Z | Z |

| | Q | Y |
|---|---|---|
| J | Q | Y |
| Z | Q | 0 |
| P | Q | Y |
| U | Q | 0 |

| | Q | Y |
|---|---|---|
| Q | $U+Z$ | 0 |
| Y | 0 | 0 |

| | J | Z | P | U |
|---|---|---|---|---|
| J | J | Z | P | U |
| Z | Z | Z | P | P |
| P | P | P | Z | Z |
| U | U | P | Z | Z |

| | Q | Y |
|---|---|---|
| J | Q | Y |
| Z | Y | Y |
| P | Y | Y |
| U | Y | Y |

| | Q | Y |
|---|---|---|
| Q | $U+Z$ | $P+Z$ |
| Y | $P+Z$ | $P+Z$ |

| | J | Z | P | U |
|---|---|---|---|---|
| J | J | Z | P | U |
| Z | Z | Z | U | U |
| P | P | U | J | Z |
| U | U | U | Z | Z |

| | Q | Y |
|---|---|---|
| J | Q | Y |
| Z | Q | Q |
| P | Q | Y |
| U | Q | Q |

| | Q | Y |
|---|---|---|
| Q | $U+Z$ | $U+Z$ |
| Y | $U+Z$ | $U+Z$ |

| | J | Z | P | U |
|---|---|---|---|---|
| J | J | Z | P | U |
| Z | Z | Z | U | U |
| P | P | U | Z | Z |
| U | U | U | Z | Z |

| | Q | Y |
|---|---|---|
| J | Q | Y |
| Z | Q | Y |
| P | Y | Q |
| U | Y | Q |

| | Q | Y |
|---|---|---|
| Q | U | Z |
| Y | Z | U |

| | J | Z | P | U |
|---|---|---|---|---|
| J | J | Z | P | U |
| Z | Z | Z | U | U |
| P | P | U | J | Z |
| U | U | U | Z | Z |

| | Q | Y |
|---|---|---|
| J | Q | Y |
| Z | Y | Y |
| P | Q | Y |
| U | Y | Y |

| | Q | Y |
|---|---|---|
| Q | $U+Z$ | $U+Z$ |
| Y | $U+Z$ | $U+Z$ |

| | J | Z | P | U |
|---|---|---|---|---|
| J | J | Z | P | U |
| Z | Z | Z | U | U |
| P | P | U | Z | Z |
| U | U | U | Z | Z |

| | Q | Y |
|---|---|---|
| J | Q | Y |
| Z | Q | Y |
| P | Y | Q |
| U | Y | Q |

| | Q | Y |
|---|---|---|
| Q | Z | U |
| Y | U | Z |

| | J | Z | P | U |
|---|---|---|---|---|
| J | J | Z | P | U |
| Z | Z | Z | U | U |
| P | P | U | J | Z |
| U | U | U | Z | Z |

| | Q | Y |
|---|---|---|
| J | Q | Y |
| Z | Q | Y |
| P | Y | Q |
| U | Y | Q |

| | Q | Y |
|---|---|---|
| Q | $U+Z$ | $U+Z$ |
| Y | $U+Z$ | $U+Z$ |

| | J | Z | P | U |
|---|---|---|---|---|
| J | J | Z | P | U |
| Z | Z | Z | U | U |
| P | P | U | Z | Z |
| U | U | U | Z | Z |

| | Q | Y |
|---|---|---|
| J | Q | Y |
| Z | Q | 0 |
| P | Q | 0 |
| U | Q | 0 |

| | Q | Y |
|---|---|---|
| Q | $U+Z$ | 0 |
| Y | 0 | 0 |

| | J | Z | P | U |
|---|---|---|---|---|
| J | J | Z | P | U |
| Z | Z | Z | U | U |
| P | P | U | J | Z |
| U | U | U | Z | Z |

| | Q | Y |
|---|---|---|
| J | Q | Y |
| Z | Q | Q |
| P | Q | Y |
| U | Q | Q |

| | Q | Y |
|---|---|---|
| Q | $U+Z$ | $U+Z$ |
| Y | $U+Z$ | $J+P$ |

| | J | Z | P | U |
|---|---|---|---|---|
| J | J | Z | P | U |
| Z | Z | Z | U | U |
| P | P | U | Z | Z |
| U | U | U | Z | Z |

| | Q | Y |
|---|---|---|
| J | Q | Y |
| Z | Q | Q |
| P | Q | Q |
| U | Q | Q |

| | Q | Y |
|---|---|---|
| Q | $U+Z$ | $U+Z$ |
| Y | $U+Z$ | $P+Z$ |

| | J | Z | P | U |
|---|---|---|---|---|
| J | J | Z | P | U |
| Z | Z | J | P | U |
| P | P | P | 0 | 0 |
| U | U | U | 0 | 0 |

| | Q | Y |
|---|---|---|
| J | Q | Y |
| Z | Q | Y |
| P | 0 | 0 |
| U | 0 | 0 |

| | Q | Y |
|---|---|---|
| Q | U | 0 |
| Y | 0 | 0 |

| | J | Z | P | U |
|---|---|---|---|---|
| J | J | Z | P | U |
| Z | Z | Z | U | U |
| P | P | U | Z | Z |
| U | U | U | Z | Z |

| | Q | Y |
|---|---|---|
| J | Q | Y |
| Z | Q | Q |
| P | Q | Q |
| U | Q | Q |

| | Q | Y |
|---|---|---|
| Q | $U+Z$ | $U+Z$ |
| Y | $U+Z$ | $U+Z$ |

| | J | Z | P | U |
|---|---|---|---|---|
| J | J | Z | P | U |
| Z | Z | J | P | U |
| P | P | P | 0 | 0 |
| U | U | U | 0 | 0 |

| | Q | Y |
|---|---|---|
| J | Q | Y |
| Z | Q | Y |
| P | 0 | 0 |
| U | Y | 0 |

| | Q | Y |
|---|---|---|
| Q | U | 0 |
| Y | 0 | 0 |

| | J | Z | P | U |
|---|---|---|---|---|
| J | J | Z | P | U |
| Z | Z | J | P | U |
| P | P | P | 0 | 0 |
| U | U | U | 0 | 0 |

| | Q | Y |
|---|---|---|
| J | Q | Y |
| Z | Q | Y |
| P | Y | 0 |
| U | 0 | 0 |

| | Q | Y |
|---|---|---|
| Q | U | 0 |
| Y | 0 | 0 |

| | J | Z | P | U |
|---|---|---|---|---|
| J | J | Z | P | U |
| Z | Z | J | U | P |
| P | P | U | J | Z |
| U | U | P | Z | J |

| | Q | Y |
|---|---|---|
| J | Q | Y |
| Z | Y | Q |
| P | Y | Q |
| U | Q | Y |

| | Q | Y |
|---|---|---|
| Q | $J+U$ | $P+Z$ |
| Y | $P+Z$ | $J+U$ |

| | J | Z | P | U |
|---|---|---|---|---|
| J | J | Z | P | U |
| Z | Z | J | P | U |
| P | P | P | 0 | 0 |
| U | U | U | 0 | 0 |

| | Q | Y |
|---|---|---|
| J | Q | Y |
| Z | Q | Y |
| P | Y | 0 |
| U | Y | 0 |

| | Q | Y |
|---|---|---|
| Q | U | 0 |
| Y | 0 | 0 |

| | J | Z | P | U |
|---|---|---|---|---|
| J | J | Z | P | U |
| Z | Z | J | P | U |
| P | P | P | 0 | 0 |
| U | U | U | 0 | 0 |

| | Q | Y |
|---|---|---|
| J | Q | Y |
| Z | Q | Y |
| P | 0 | 0 |
| U | 0 | 0 |

| | Q | Y |
|---|---|---|
| Q | U | 0 |
| Y | 0 | P |

| | J | Z | P | U |
|---|---|---|---|---|
| J | J | Z | P | U |
| Z | Z | J | P | U |
| P | P | P | 0 | 0 |
| U | U | U | 0 | 0 |

| | Q | Y |
|---|---|---|
| J | Q | Y |
| Z | Q | Y |
| P | 0 | 0 |
| U | 0 | 0 |

| | Q | Y |
|---|---|---|
| Q | U | 0 |
| Y | 0 | U |

| | J | Z | P | U |
|---|---|---|---|---|
| J | J | Z | P | U |
| Z | Z | J | P | U |
| P | P | P | 0 | 0 |
| U | U | U | 0 | 0 |

| | Q | Y |
|---|---|---|
| J | Q | Y |
| Z | Q | Y |
| P | 0 | 0 |
| U | 0 | 0 |

| | Q | Y |
|---|---|---|
| Q | U | P |
| Y | P | 0 |

| | J | Z | P | U |
|---|---|---|---|---|
| J | J | Z | P | U |
| Z | Z | J | P | U |
| P | P | P | 0 | 0 |
| U | U | U | 0 | 0 |

| | Q | Y |
|---|---|---|
| J | Q | Y |
| Z | Q | Y |
| P | 0 | 0 |
| U | 0 | 0 |

| | Q | Y |
|---|---|---|
| Q | U | P |
| Y | P | P |

| | J | Z | P | U |
|---|---|---|---|---|
| J | J | Z | P | U |
| Z | Z | J | P | U |
| P | P | P | 0 | 0 |
| U | U | U | 0 | 0 |

| | Q | Y |
|---|---|---|
| J | Q | Y |
| Z | Q | Y |
| P | 0 | 0 |
| U | 0 | 0 |

| | Q | Y |
|---|---|---|
| Q | U | P |
| Y | P | U |

| | J | Z | P | U |
|---|---|---|---|---|
| J | J | Z | P | U |
| Z | Z | J | P | U |
| P | P | P | 0 | 0 |
| U | U | U | 0 | 0 |

| | Q | Y |
|---|---|---|
| J | Q | Y |
| Z | Q | Y |
| P | 0 | 0 |
| U | 0 | 0 |

| | Q | Y |
|---|---|---|
| Q | U | U |
| Y | U | 0 |

| | J | Z | P | U |
|---|---|---|---|---|
| J | J | Z | P | U |
| Z | Z | J | P | U |
| P | P | P | 0 | 0 |
| U | U | U | 0 | 0 |

| | Q | Y |
|---|---|---|
| J | Q | Y |
| Z | Q | Y |
| P | 0 | 0 |
| U | 0 | 0 |

| | Q | Y |
|---|---|---|
| Q | U | U |
| Y | U | P |

| | J | Z | P | U |
|---|---|---|---|---|
| J | J | Z | P | U |
| Z | Z | J | P | U |
| P | P | P | 0 | 0 |
| U | U | U | 0 | 0 |

| | Q | Y |
|---|---|---|
| J | Q | Y |
| Z | Q | Y |
| P | 0 | 0 |
| U | 0 | 0 |

| | Q | Y |
|---|---|---|
| Q | U | U |
| Y | U | U |

| | J | Z | P | U |
|---|---|---|---|---|
| J | J | Z | P | U |
| Z | Z | J | P | U |
| P | P | P | 0 | 0 |
| U | U | U | 0 | 0 |

| | Q | Y |
|---|---|---|
| J | Q | Y |
| Z | Y | Q |
| P | 0 | 0 |
| U | 0 | 0 |

| | Q | Y |
|---|---|---|
| Q | U | U |
| Y | U | U |

| | J | Z | P | U |
|---|---|---|---|---|
| J | J | Z | P | U |
| Z | Z | J | U | P |
| P | P | U | 0 | 0 |
| U | U | P | 0 | 0 |

| | Q | Y |
|---|---|---|
| J | Q | Y |
| Z | Y | Q |
| P | 0 | 0 |
| U | 0 | 0 |

| | Q | Y |
|---|---|---|
| Q | U | P |
| Y | P | U |

| | J | Z | P | U |
|---|---|---|---|---|
| J | J | Z | P | U |
| Z | Z | J | U | P |
| P | P | U | J | Z |
| U | U | P | Z | J |

| | Q | Y |
|---|---|---|
| J | Q | Y |
| Z | Y | Q |
| P | Q | Y |
| U | Y | Q |

| | Q | Y |
|---|---|---|
| Q | $U+Z$ | $J+P$ |
| Y | $J+P$ | $U+Z$ |
